# Supplementary material for: Enhancing Interpretability and Generalizability in Extended Isolation Forests
Source: arXiv:2310.05468 source file (2024-10-09)
Supplement: Supplementary file 1 [file appendix.tex]

\section{}

\begin{definition}[Partial Order]
A binary relation, $\leq$, on a set $\pmb{S}$, is a partial order iff it is reflexive, transitive and antisymmetric, that is:
\begin{itemize}
    \item (Reflexivity): $a \leq a$, $\forall$ $a \in \pmb{S}$.
    \item (Transitivity): If $a \leq b$ and $b \leq c$, then $a \leq c$, $\forall$ $a,b,c \in \pmb{S}$.
    \item (Antisymmetry): If $a \leq b$ and $b \leq a$, then $a=b$, $\forall$ $a,b \in \pmb{S}$.
\end{itemize}
\end{definition}
\vspace{.3cm}
\begin{definition}[Ordered Vector Space]:
A real vector space $X$ equipped with a partial ordering $(X,\leq)$ is a ordered vector space if:
\begin{enumerate}
    \item $x\leq y \implies x+z \leq y+z, \, \forall x,y,z \in X$;
    \item $x\leq y \implies \lambda x \leq \lambda y, \, \forall \lambda \in \mathbb{R}^+:= \{x \in \mathbb{R}|x>0\}$.
\end{enumerate}
\end{definition}
\vspace{.3cm}
\begin{definition}[Infimum (analog. supremum)]
Defined a partial ordered vector space $(X,\geq)$, if $Y \subseteq X$ and $y \in X$ then $y=\inf_{\geq}(Y)$($y=\sup_{\geq}(Y)$), y is the infimum(supremum) of Y w.r.t. $\geq$, iff:
\begin{enumerate}
    \item $\forall x \in Y$: $y \leq x$ ($y \geq x$);
    \item $\forall x \in Y$: $z \leq x \implies z \leq y$ ($z \geq x \implies z \geq y$).
\end{enumerate}
\end{definition}
\vspace{.3cm}
\begin{definition}[Component-Wise Order]\label{Component-Wise Order}
The relation $\leq$ on a vector space $X\subseteq \mathbb{R}^d$ such that $\forall v,w \in X $ if $v_i \leq w_i, \forall i \in \{0,1,\dots,d\} \implies v \leq w$ is a Component wise order for a vector space.
\end{definition}
\vspace{.3cm}
\begin{theorem}
The Component-Wise Order for a vector space is a partial order.
\end{theorem}
