# Supplementary material for: Enhancing Interpretability and Generalizability in Extended Isolation Forests
Source: arXiv:2310.05468 source file (2024-10-09)
Supplement: Supplementary file 2 [file new_appendix.tex]

\appendix
\section{Appendices}
\subsection{Datasets}\label{sec:appendix_datasets}
\subsubsection{Synthetic datasets}\label{sec:appendix-synthetic-data}
The syntethic datasets comprise two distinct categories of data points: one, designated as \textit{inliers}, adheres to the anticipated distribution pattern, while the second category, denoted as \textit{outliers}, consists of points that markedly diverge from the inlier distribution along specific directions.

To accurately replicate the class imbalance prevalent in AD tasks, the proportion of anomalies (outliers) generated is significantly lower than that of inliers. This disparity mirrors real-world conditions, as validated in Section \ref{sec:appendix-real-world-data}, where anomalous instances are infrequent. The datasets are characterized by a \textit{contamination factor}, a metric quantifying the prevalence of outliers relative to the total dataset population. Typical contamination factor values range between 5 to 10\%, although in certain contexts, such as Credit Card Fraud Detection, this percentage can be substantially below 1%.

We considered the following synthetic datasets:

\begin{comment}
    {\ttfamily Bimodal} credo si possa togliere visto che non lo abbiamo più usato 
\end{comment}

\begin{itemize}
    \item The {\ttfamily Bimodal} dataset was exploited also by other researchers like Hariti et. al \cite{8888179}, making it a well-suited synthetic example.
    The resulting point distribution of the {\ttfamily Bimodal} dataset is depicted in the scatter plot in Figure \ref{fig:bimodal-2d-scatter}. The contamination factor used for the {\ttfamily Bimodal} dataset is 2.5\%. 
    \begin{figure}[ht]
      \centering
      \includegraphics[width=0.4\linewidth]{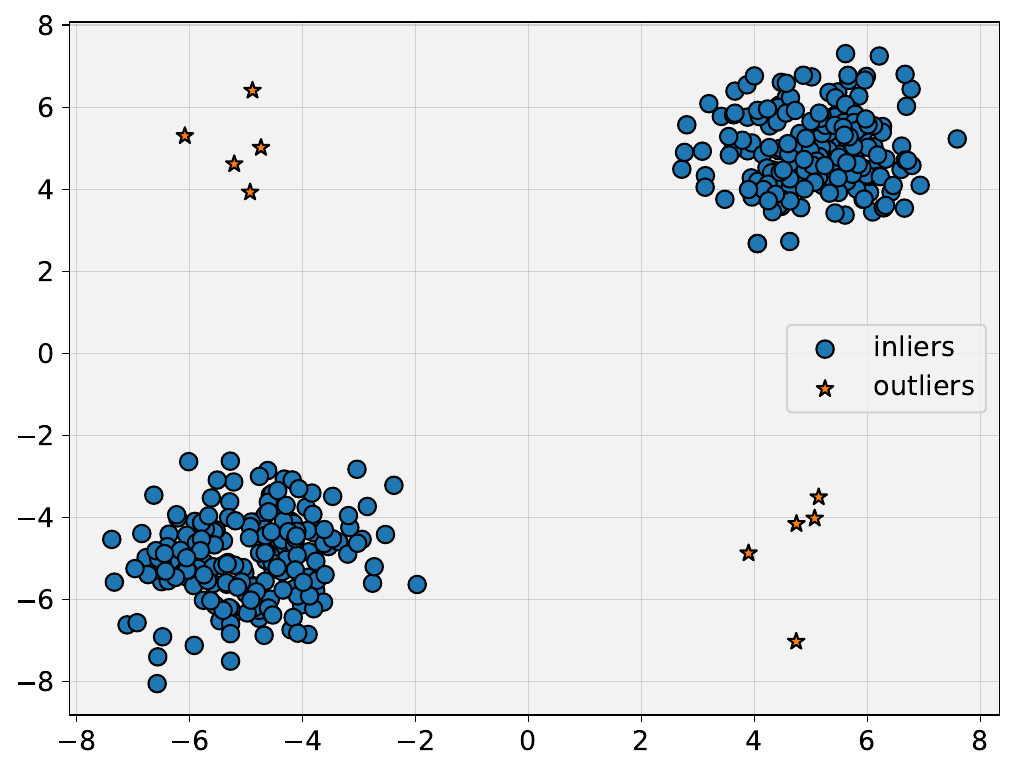}
      \caption{Scatter Plot of the \textbf{bimodal} Dataset}
      \label{fig:bimodal-2d-scatter}
    \end{figure}\hfil % <-- added
    
    In particular, the two clusters of inliers are positioned along the bisector line while the outliers are placed along the anti-bisector line. 
    As it can be noticed from a detailed observation of the scatter plot, there is a significant discrepancy in terms of quantity between inliers and outliers. In fact, the dataset was manipulated in order to ensure the imbalance between normal and anomalous points to replicate a common scenario in the context of Anomaly Detection. 

    \item  The datasets referred to as {\ttfamily Xaxis} and {\ttfamily Yaxis} originate from the research paper authored by Carletti et al. \cite{diffi}. In this particular scenario, inlier points are randomly sampled from a six-dimensional sphere centered at the origin with a radius of 5.
    
    To generate the outlier data, a specific feature is chosen to be associated with anomalous values. In this instance, feature 0 is selected for the {\ttfamily Xaxis} dataset, and feature 1 is chosen for the {\ttfamily Yaxis} dataset. All other features consist of random noise values drawn from a standard normal distribution, denoted as $X \sim N(0,1)$.
    
    Subsequently, outlier points are sampled along these specific features, maintaining a predefined proportion relative to the inliers. In this specific case, there is one outlier for every 10 inliers.

    \item The {\ttfamily Bisect} dataset closely resembles the {\ttfamily Xaxis} and {\ttfamily Yaxis} datasets. In this dataset, the inliers are distributed following a normal distribution pattern within a six-dimensional sphere. Conversely, the anomalies are positioned along the bisector line of the Feature 0 and Feature 1 subspace, equidistant from the origin as the anomalies in the {\ttfamily Xaxis} and {\ttfamily Yaxis} datasets.

    \item As the names suggest, {\ttfamily Bisect3D} and {\ttfamily Bisect6D} datasets are constructed similarly to the {\ttfamily Bisect} dataset. However, in {\ttfamily Bisect3D}, the anomalies are placed along the bisector line of the subspace defined by Feature 0, Feature 1, and Feature 2. In {\ttfamily Bisect6D}, the anomalies are positioned along the bisector line spanning all six dimensions of the dataset.
    The proportion of the outliers remains 1-10 as in the {\ttfamily Xaxis} and {\ttfamily Yaxis} datasets. 

    \item \davide{Finally, the {\ttfamily Bisect3D\_Skewed} dataset shares the same structure of {\ttfamily Bisect3D}, with anomalies distributed along Feature 0,1 and 2, but the width of the bisector lines are different. As a consequence anomalies are unevenly distributed along the three features . In particular, points along Feature 0 are more isolated than those along Feature 1, which in turn are more anomalous than those along Feature 2. This peculiar design is used to test the ability of an interpretability model to not only correctly identify anomalous features but also to correctly rank them in decreasing order of outlyingness.}

\davide{For clarity the pseudocode for the generation of the synthetics datasets employed in this paper are provided in \ref{alg:syn_data_inliers}, \ref{alg:syn_data_outliers_single}, \ref{alg:syn_data_outliers_multi}, \ref{alg:syn_data_outliers_multi_skewed}}. 

\end{itemize}

\begin{algorithm}
\caption{Synthetic Dataset Generation - Inliers Generation} \label{alg:syn_data_inliers}
\SetKwInOut{Input}{Input}
\SetKwInOut{Output}{Output}

\Input{Number of samples to generate $n$, Number of features composing the dataset $p$, Radius of the inliers ball $r$}
\Output{Generated synthetic dataset $\mathcal{D} \in \mathbb{R}^{n \times p}$}

$\mathcal{D} \gets \text{empty list}$\;
\tcp{Initialize an empty list to contain the samples}

\While{$\text{len}(\mathcal{D}) < n$}{
    \tcp{Sample a random $p$-dimensional vector from a Uniform distribution defined in $[-r,r]$ and insert it into $\mathcal{D}$ only if its norm is less than or equal to $r$}
    $\text{point} \sim \mathcal{U}_p([-r,r])$\;
    \If{$(||\text{point}||^2) \leq r$}{
        $\mathcal{D} \gets \mathcal{D} \cup \text{point}$\;
    }
}

\Return{$\mathcal{D}$}\;
\end{algorithm}

\begin{algorithm}
\caption{Synthetic Dataset Generation - Single Dimension Outliers Generation} \label{alg:syn_data_outliers_single}
\SetKwInOut{Input}{Input}
\SetKwInOut{Output}{Output}

\Input{Number of samples to generate $n$, Number of features composing the dataset $p$, Maximum and minimum outlier values: $\text{max} \in \mathbb{R}$, $\text{min} \in \mathbb{R}$}
\Output{Generated synthetic dataset $\mathcal{D} \in \mathbb{R}^{n \times p}$}

$\mathcal{D_O} \gets \mathcal{U}([\text{min},\text{max}])$\;
\tcp{Outliers are scalar values sampled from a Uniform distribution defined in $[\text{min},\text{max}]$}

$\mathcal{D_I} \gets \mathcal{N}_{p-1}([0,1])$\;
\tcp{Samples from the remaining $p-1$ dimensions are sampled from a $\mathcal{N}(0,1)$ distribution}

$\mathcal{D} \gets \text{concatenate}(\mathcal{D_I},\mathcal{D_O})$\;
\tcp{Concatenate $\mathcal{D_I}$ and $\mathcal{D_O}$ column-wise to form the final dataset}

\Return{$\mathcal{D}$}\;

\end{algorithm}

\begin{algorithm}
\caption{Synthetic Dataset Generation - Multiple Dimension Outliers Generation} \label{alg:syn_data_outliers_multi}
\SetKwInOut{Input}{Input}
\SetKwInOut{Output}{Output}

\Input{Number of samples to generate $n$, Number of features composing the dataset $p$, Number of anomalous features $d$ ($d < p$), Maximum and minimum outlier values: $\text{max} \in \mathbb{R}$, $\text{min} \in \mathbb{R}$}
\Output{Generated synthetic dataset $\mathcal{D} \in \mathbb{R}^{n \times p}$}

$\mathcal{D_O}[0] \gets \mathcal{U}([\text{min},\text{max}])$\;
\tcp{Sample the first anomalous feature as done in Algorithm \ref{alg:syn_data_outliers_single}}

\For{$i \gets 1$ \KwTo $d$}{
    \tcp{To sample the remaining $d-1$ anomalous directions, add white noise (i.e., $\mathcal{N}([0,1])$) to the first anomalous direction}
    $\mathcal{D_O}[i] \gets \mathcal{D_O}[0] + \mathcal{N}([0,1])$\;
}

$\mathcal{D_I} \gets \mathcal{N}_{p-d}([0,1])$\;
\tcp{The remaining $p-d$ normal features are sampled from a $\mathcal{N}(0,1)$ distribution}

$\mathcal{D} \gets \text{concatenate}(\mathcal{D_I},\mathcal{D_O})$\;

\Return{$\mathcal{D}$}\;

\end{algorithm}

\davide{
\begin{algorithm}
\caption{Synthetic Dataset Generation - Multiple Dimension Skewed Outliers Generation} \label{alg:syn_data_outliers_multi_skewed}
\SetKwInOut{Input}{Input}
\SetKwInOut{Output}{Output}

\Input{Number of samples to generate $n$, Number of features composing the dataset $p$, Number of anomalous features $d$ ($d < p$), Maximum and minimum outlier values: $\text{max} \in \mathbb{R}$, $\text{min} \in \mathbb{R}$, Distance from the inliers ball $q$, Vector containing the proportion of outlyingness for each feature $v$}
\Output{Generated synthetic dataset $\mathcal{D} \in \mathbb{R}^{n \times p}$}

$x \gets \mathcal{U}([\text{min},\text{max}])$\;
\tcp{Sample some random points as a baseline for the generation}

$u \gets \frac{v}{||v||^2}$\;
\tcp{Define vector $u$ as the normalized version of vector $v$}

\For{$i \gets 1$ \KwTo $d$}{
    \tcp{To construct the anomalous features we create $d$ hyperplanes with inclination dictated by $u$ at distance $q$ from the inliers ball}
    $\mathcal{D_O}[i] \gets d \cdot u[i] + x \cdot u[i])$\;
}

$\mathcal{D_I} \gets \mathcal{N}_{p-d}([0,1])$\;
\tcp{The remaining $p-d$ normal features are sampled from a $\mathcal{N}(0,1)$ distribution}

$\mathcal{D} \gets \text{concatenate}(\mathcal{D_I},\mathcal{D_O})$\;

\Return{$\mathcal{D}$}\;

\end{algorithm}
}

\subsubsection{Real-world Datasets}\label{sec:appendix-real-world-data}
Most of the considered Real-World Datasets are part of the widely used 
Outlier Detection DataSets (ODDS) library introduced in  \cite{Rayana:2016}.
Unlike their computer-generated counterparts, these datasets reflect the complexity present in real world scenarios.
However, it's essential to emphasize the origin of these datasets, as the majority comes from an adaptation to the AD task of datasets originated with a different purpose. In particular, the ODDS datasets are obtained after applying an alteration to datasets that originally came in the form of Multi-Class datasets.
This is due to the fact that, unfortunately, the existing literature lacks dedicated Real-World benchmark Datasets specifically tailored for AD. 
Typically, the applied transformation involves undersampling the least-represented class, designating it as the outlier class, and merging the remaining classes into a single category representing the normal distribution of the data. As we will discuss in our experiments, this approach presents challenges, as an undersampled version of the minority class may not result in abnormally distributed samples. 
The considered AD approaches are designed to identify anomalies defined as isolated samples in an unsupervised manner. Obviously, the detected anomalies may not always align with the provided labels. It is worth noticing that this discrepancy makes it more difficult to evaluate the algorithm interpretability, as will be investigated in Section \ref{sec:real-dataset-experiments}.

Many Real-World Datasets lack detailed information on features and labels, complicating model evaluation and interpretation of Feature Importance scores. Only the {\ttfamily Glass} dataset, detailed by Carletti et al. \cite{carletti2019explainable}, allows us to analyze Feature influence on anomalies, discussed in Section \ref{sec:glass}. This gap in data detail poses significant challenges for complete qualitative model assessment and understanding the real impact of the features to the anomalies.

To overcome these limitations, two new datasets were added to the original list: the {\ttfamily Diabetes} and the {\ttfamily Moodify} datasets. The peculiarity of these two sets of data is that they are provided with highly detailed information on the semantics of the features and labels composing them. Thus, once AD and interpretation results are obtained, is possible to evaluate them by measuring how they are aligned with the provided domain knowledge.

This is the list of considered real-world datasets:
\begin{itemize}
    \item {\ttfamily Annthyroid}: The {\ttfamily Annthyroid} dataset \cite{misc_thyroid_disease_102} is part of the UCI Machine Learning Repository. It is a three-class Classification dataset. The aim of the classification task associated with this dataset is to detect whether a patient is hypothyroid (i.e. the patient has an underactive thyroid) or not. For this scope, the three classes used refer to the functioning conditions of the thyroid that can be\textit{normal} (not hypothyroid), \textit{hyperfunctioning} (overactive thyroid) and \textit{subnormal}. The dataset originally contained 15 categorical and 6 numerical attributes. In order to adapt it to an Anomaly Detection task only the numerical attributes were considered and the \textit{hyperfunctioning} and \textit{subnormal} function classes were considered as part of the outliers while the \textit{normal} functioning samples are used to build the inlier class. 
    The six numerical features represent, respectively, the following quantities: TSH, T3, TT4, T4U, and FTI. 
        \begin{itemize}
            \item \textbf{TSH (Thyroid-Stimulating Hormone}: TSH is an hormone produced by the pituitary gland. An underactive thyroid (hypothyroidism) is associated with high levels of TSH while low levels of TSH are associated with an overactive thyroid (hyperthyroidism). 
            \item \textbf{T3 (Triiodothyronine)}: T3 is one of the thyroid hormones. It plays a crucial role in regulating the metabolism. It is important to measure the levels of this hormone, specifically in cases of hyperthyroidism. 
            \item \textbf{TT4 (Total Thyroxine)}: This quantity represents the total amount of the T4 thyroid hormone in the blood. T4 levels are associated to the overall thyroid hormone production. 
            \item \textbf{T4U (Thyroxine-Binding Globulin}: T4U measures the level of thyroxine-binding globulin, a protein binding to thyroid hormones in the blood. T4U levels are connected to the thyroid hormone availability in the body. 
            \item \textbf{FTI (Free Thyroxine Index}: Taking into account the T4 and T4U levels, the FTI provides an estimate of the amount of free thyroxine (T4) in the blood. It is used to asses the free, active thyroid hormone levels in the body. 
        \end{itemize}
        
    \item {\ttfamily Breast}: The {\ttfamily Breast} dataset \cite{misc_breast_cancer_wisconsin_(original)_15} is a Binary Classification dataset where the target is the presence of breast cancer or not in a patient. The peculiarity of the samples contained in this dataset is that they are formed by categorical features. Normally, the Anomaly Detection models described in this paper are not built to deal with categorical features but in this particular case the high number of levels (e.g. The age variable has nine levels: 10-19, 20-29, \dots; the tumor-size feature has levels equal to 0-4,5-9,10-14, \dots) characterizing the {\ttfamily Breast} dataset's attributes makes it possible to consider them as numerical features.
    A noteworthy consequence to consider is that when the samples of the {\ttfamily Breast} dataset are represented in a scatter plot, as it happens with the Local Importance Scoremap in Figure \ref{fig:Local-Breastw}, they appear to have a grid-like shape.
    The dataset is composed of samples coming from the clinical cases of Dr. Wolberg collected in a time span going from January 1989 to November 1991. 
    The dataset is composed by 9 features representing the following quantities: Clump Thickness, Uniformity of Cell Size, Uniformity of Cell Shape, Marginal Adhesion, Single Epithelial Cell Size, Bare Nuclei, Bland Chromatin, Normal Nucleoli and Mitoses. 
    
    \item {\ttfamily Cardio}: The {\ttfamily Cardio} \cite{misc_cardiotocography_193} dataset is part of the UCI Machine Learning Repository and its complete name is {\ttfamily Cardiotocoraphy} since it contains measurements of fetal heart rate (FHR) and uterine contraction (UC) on cardiotocograms \footnote{A cardiotogram is a medical test monitoring fetal hearth rate and uterine contractions during pregnancy. It is used to assess the health status of the fetus and the progress of labor during pregnancy and childbirth}. This dataset contains 3 classes that were assigned by expert obstetricians: \textit{normal}, \textit{supsect}, and \textit{pathologic}. In order to use this dataset for Anomaly Detection the suspect class was discarded and the pathologic class was downsampled to 176 points to maintain unbalance with respect to the normal class. There are 21 features. \footnote{The complete list of features names can be found at: https://archive.ics.uci.edu/dataset/193/cardiotocography}

    \item {\ttfamily Glass}: \ale{The {\ttfamily Glass} dataset \cite{misc_glass_identification_42} is originally used for multi-class classification to distinguish 7 different types of glasses. There are 9 features: the first one is the Refractive Index while the others measure the concentration of Magnesium (Mg), Silicon (Si), Calcium (Ca), Iron (Fe), Sodium (Na), Aluminum (Al), Potassium (K) and Barium (Ba) in the glass samples. The seven original glass groups were divided into two: Groups 1,2,3 and 4 represent Window Glasses while the remaining ones are non-window glasses: containers glass, tableware glass and headlamp glass. Among the non-window glasses, headlamp glasses were considered as outliers while Window Glasses are labeled as inliers in order to convert this dataset to be used for Anomaly Detection. According to some prior knowledge on the subject the Barium (Ba) and Potassium (K) concentration should be decisive in distinguishing between headlamp and window glasses. In fact Barium is considered the crucial element to perform the distinction between headlamp and window glasses since it is usually added to the category of headlamp glasses in order to improve their optical properties. Another potential key attribute is Potassium (K) that is frequently exploited to enhance strength and thermal resistance of window glasses. For the interested reader a more detailed on this topic is provided in Section \ref{sec:glass-imp-plots}. }

    \item {\ttfamily Ionosphere}: The {\ttfamily Ionosphere} dataset \cite{misc_ionosphere_52} contains measurements collected by a radar in Goose Bay, Labrador. The measurement system consisted of 16 high-frequency antennas with a transmitted power in the order of 6.4 kilowatts. The targets to measure were free electrons in the Ionosphere. Originally this is built as a Binary Classification dataset where the two classes are \textit{good} if the captured electrons show some kind of structure in the ionosphere and \textit{bad} otherwise. The signal is processed with an autocorrelation function depending on the time of a pulse and the pulse number. There are 17 pulse numbers and each of them is identified by a pair of features for a total of 34 features.

    %The task is to recognize the handwritten digit and 16 is the number of numerical features available. Unfortunately, the semantic meaning of these features is not provided. 
    
    \item {\ttfamily Pima}: The {\ttfamily Pima} dataset \footnote{https://www.kaggle.com/datasets/uciml/pima-indians-diabetes-database} comes from the National Institute of Diabetes, Digestive and Kidney Diseases. It is a Binary Classification dataset whose aim is to predict whether a patient has diabetes or not. This dataset is the result of the application of some constraints to a larger dataset. In {\ttfamily Pima}, in fact, the data considered are obtained from female patients of at least 21 years of age coming from the Pima Indian heritage. 
    
    %As it happens with {\ttfamily Ionosphere}, {\ttfamily Glass}, {\ttfamily Breast} a subsampling operation was performed on the dataset before the training of the \approach model to reduce the contamination factor from almost 35\% to 10\%. 
    
    The dataset contains 8 features indicating some typical diagnostic measurements: Number of pregnancies, Plasma Glucose Concentration, Diastolic Blood Pressure, Triceps skin thickness, 2-hour serum if insulin, BMI (Body Mass Index), Diabetes Pedigree function, and Age.

    \item {\ttfamily Pendigits}: The {\ttfamily Pendigits} dataset collects data regarding handwritten digits produced by Forty-four human writers. The task associated with this dataset is the one of recognizing the correct written digit. The dataset is composed of 16 features and the number of objects per class (i.e. per digit) was reduced by a factor of 10 \% to increase the unbalance between classes in order to adapt the dataset as a benchmark for the evaluation of Anomaly Detection models.
    
    \item {\ttfamily Shuttle}: The {\ttfamily Shuttle} dataset \cite{misc_statlog_(shuttle)_148} describes radiator positions in a NASA space shuttle. The samples are characterized by 9 attributes. Originally, the dataset is used for Multi-Class Classification with the target variable containing seven possible classes, which are: Radiator Flow, Fpv Close, Fpv Open, High, Bypass, Bpv Close, and Bpv Open. Besides the normal Radiator Flow class about 20\% of the data points describe anomalous situations. To reduce the amount of anomalies the Radiator Flow class is used to form the inlier class while a stratified sampling procedure was applied to classes 2,3,5,6 and 7. Finally, data coming from class 4 were discarded.
    
    \item {\ttfamily Wine}: The {\ttfamily Wine} dataset \cite{misc_wine_109} is part of the UCI Machine Learning repository and it was originally created as a 3-class classification dataset. In fact, it contains data resulting from a chemical analysis of wines grown in the same region of Italy but obtained from 3 different cultivars. So the aim of a Classification model applied to this dataset would be to correctly predict the original culture of wine given its chemical properties. As it is usually done in these cases the dataset was adapted to test Anomaly Detection models considering the data from two cultures as inliers and the ones beholding to the last culture as the outliers. The dataset is composed by 13 features representing the following quantities: Alcohol, Malic Acid, Ash, Alcalinity of ash, Magnesium, Total phenols, Flavanoids, Nonflavanoid phenols, Proanthocyanins, Color Intensity, Hue, OD280/OD315 \footnote{These codes refers to two measurements of the optical density of a wine sample performed at two different wavelengths: 280 nm and 315 nm. These measurements are typically exploited to assess the protein content and the stability of wine} of diluted wines, and Proline. 
    
\item {\ttfamily Diabetes}: The {\ttfamily Diabetes} dataset \footnote{https://www.kaggle.com/datasets/iammustafatz/diabetes-prediction-dataset} is a Binary Classification dataset with medical data about patients used to predict whether they have diabetes or not. There are 4 categorical and 4 numerical variables. In order to use the \approach model only the numerical variables were considered: 

        \begin{itemize}
            \item Age: The age ranges between 0 and 80 and it can be an important factor since Diabetes is usually diagnosed in older adults.
            \item BMI (Body Mass Index): Measure of body fat based on weight and height. High BMI values are linked to a higher risk of diabetes.
            \item HbA1c-Level: The Hemoglobin A1c Level it's a measure of a person's average blood sugar level over the past 2-3 months. A high level of HbA1c is usually associated with high diabetes risk.
            \item blood-glucose-level: The amount of glucose in the bloodstream at a given time. High glucose levels are a key factor to detect Diabetes.
        \end{itemize}

        Finally, the target variable is a binary variable indicating the presence or absence of diabetes in the patient. Following the usual protocol for Real World Datasets, the inlier group will be represented by healthy patients while the ones affected by diabetes will be placed in the outlier group. 
    
    \item {\ttfamily Moodify}: Moodify is a recommendation app \footnote{More details on the Moodify project can be found at: https://github.com/orzanai/Moodify} that classifies Spotify songs according to the emotions transmitted to the users. The system is trained on the  {\ttfamily Moodify} dataset \footnote{https://www.kaggle.com/datasets/abdullahorzan/moodify-dataset} which contains features regarding the main characteristics of about 278.000 songs and the target is a 4 levels categorical variable with the following coding: 

    \begin{enumerate}
        \item \textit{Sad}
        \item \textit{Happy}
        \item \textit{Energetic}
        \item \textit{Calm}
    \end{enumerate}

    The label with the lowest frequency (15\%) in the dataset is \textit{Calm} so that was used to create the outliers group while the inlier group is formed by the songs that belong to the other three classes. 

    The dataset is composed of 11 numerical features describing different musical attributes of a song. Except for the Loudness variable, which expresses the overall loudness of the track in decibels (dB), all the features have values contained in the [0,1] interval. The variable names are the following: Acousticness, Danceability, Energy, Instrumentalness, Liveness, Loudness, Speechiness, Valence, and Tempo. Other variables are Duration (ms) and spec-rate.
    
\end{itemize}

\subsubsection{Draw-backs of Isolation Forest}\label{sec:IFvsEIF}
Next, we delve deeper into the artifacts of the IF and how the EIF is able to avoid them.
The primary distinction among the mentioned models lies in their approach to determining splitting hyperplanes. In the case of the %iForest 
IF, it operates under the constraint of splitting the feature space along a single dimension. Consequently, the constructed splitting hyperplane is invariably orthogonal to one dimension while remaining parallel to the others.

The EIF model instead relaxes this constraint, it allows multiple splits in the feature space along different dimensions, thus the splitting hyperplane can be oriented differently in each isolation tree. 
This relaxation helps to provide a more expressive way to capture complex data distributions while maintaining performances.
Moreover, as Hariri et al. pointed out in \cite{8888179}, the EIF avoids the creation of regions where the anomaly score is lower only due to the imposed constraints. In Figure \ref{fig:scoremap 2 IF vs EIF} we can observe that the effect of the constraint is twofold: (i) it generates bundles in the hyperplanes orthogonal to the main directions, and (ii) it creates "artifacts", i.e. low anomaly score zones in their intersections, as we can observe in the Scoremap \ref{fig:anomaly scoremap IF}.

\begin{figure}[!ht]
    \centering % <-- added
    \begin{subfigure}{0.45\textwidth}
    \centering
      \includegraphics[width=\linewidth]{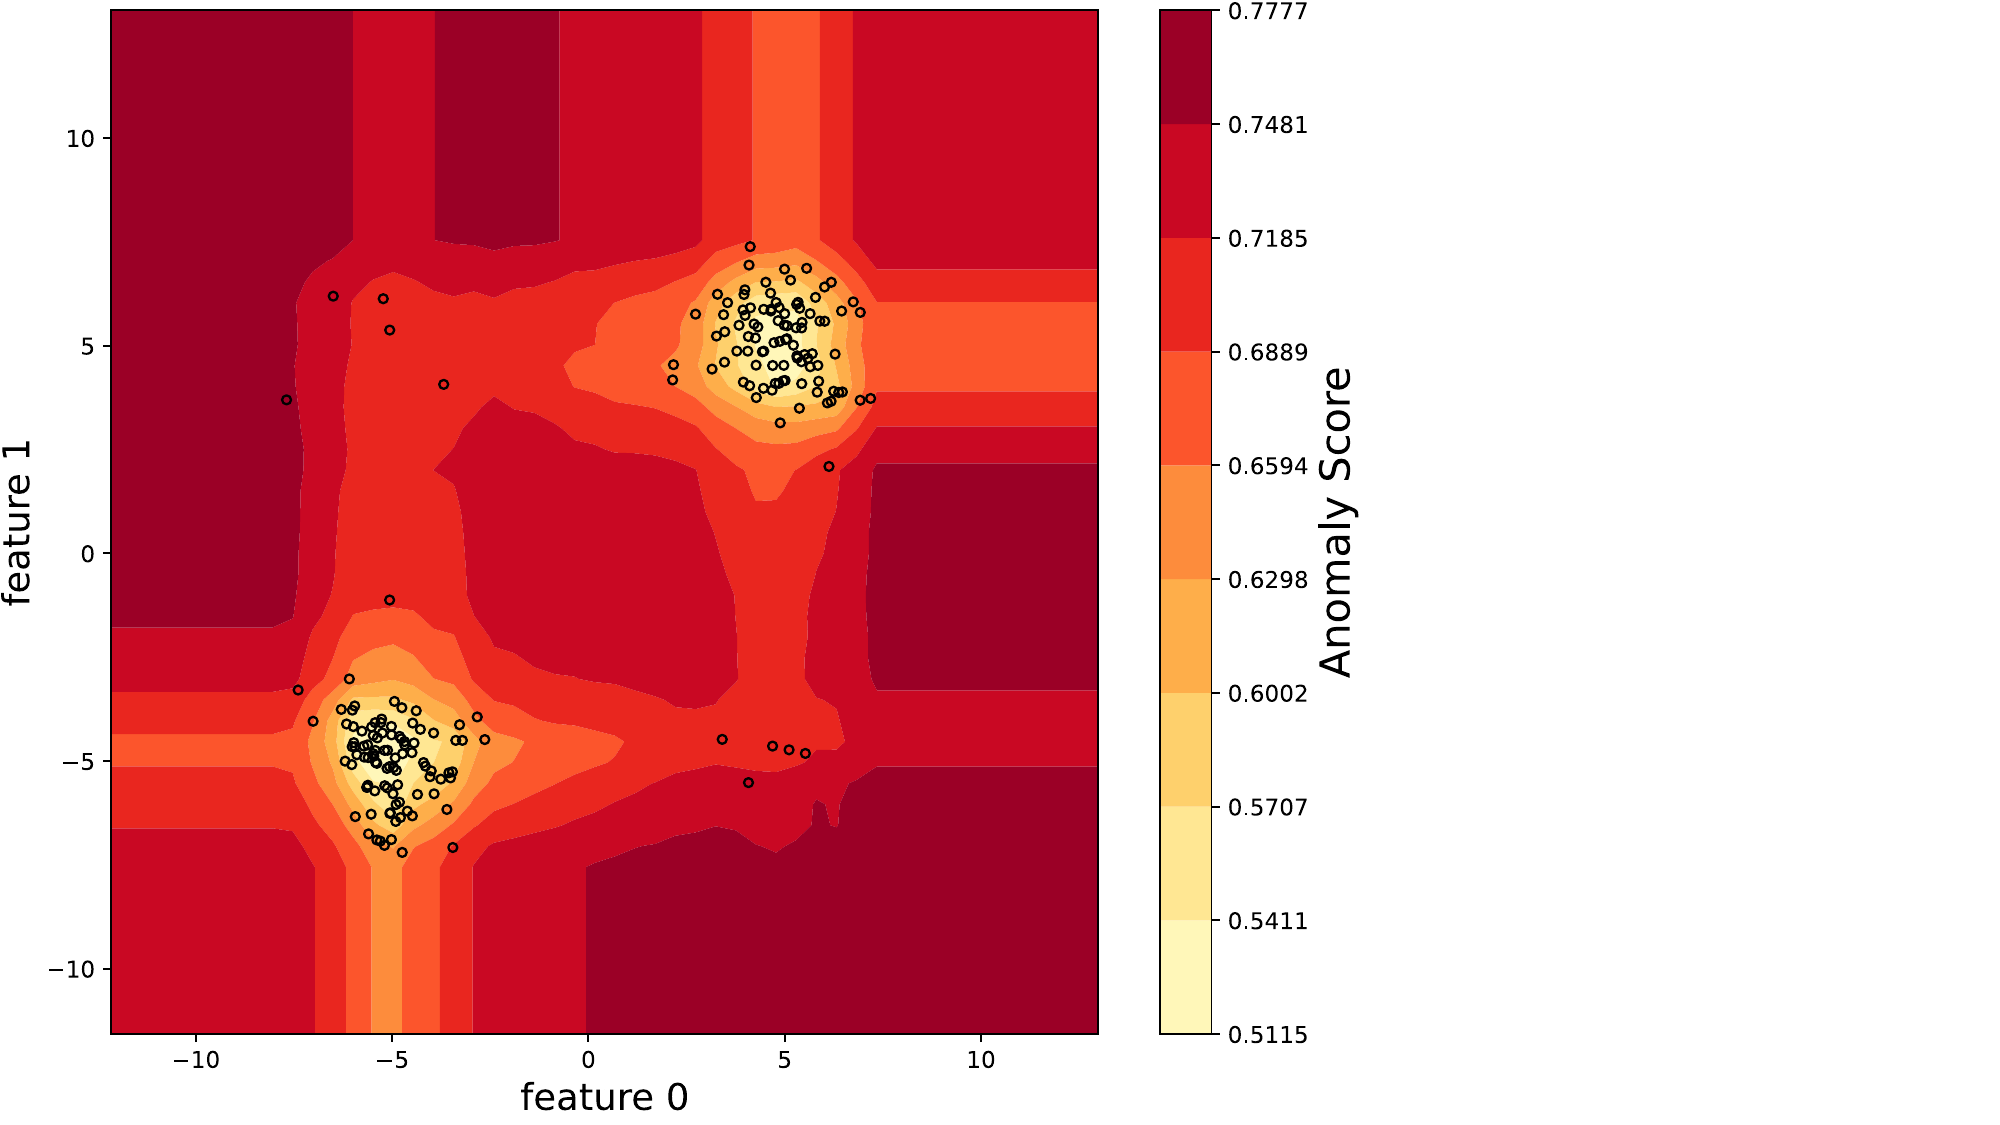}
      \caption{Anomaly Scoremap IF}
      \label{fig:anomaly scoremap IF}
    \end{subfigure}\hfil % <-- added
    \begin{subfigure}{0.45\textwidth}
    \centering
      \includegraphics[width=\linewidth]{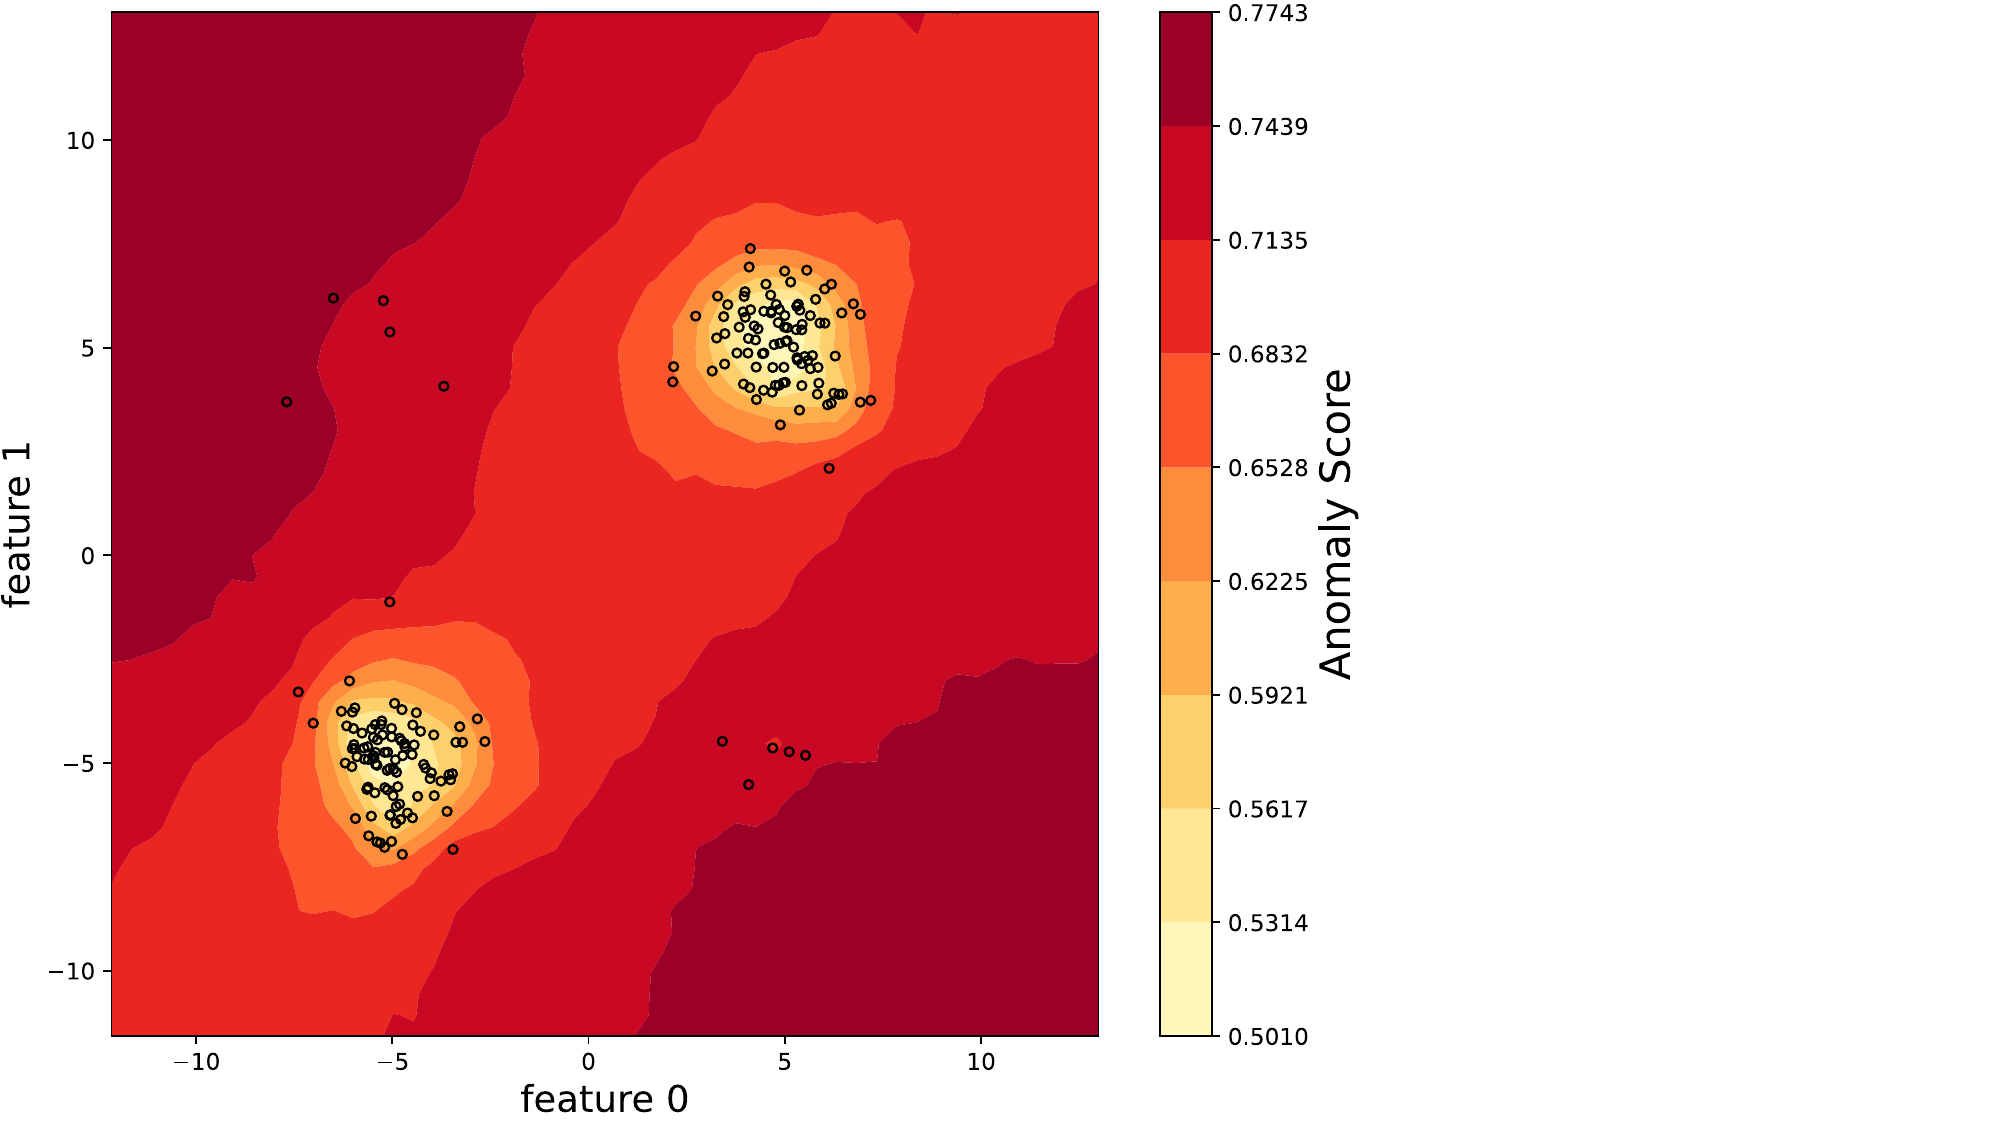}
      \caption{Anomaly Scoremap EIF}
      \label{fig:anomaly scoremap EIF}
    \end{subfigure}\hfil % <-- added
\caption{Scoremap showing the differences between IF and EIF in the two dimensional space dataset {\ttfamily Bimodal} described in Section \ref{sec:appendix-synthetic-data}. Figure inspired from \cite{8888179}.}\label{fig:scoremap 2 IF vs EIF}
\end{figure}

As we progressively relax the IF constraint on splitting directions, these artifacts tend to disappear. We simulated the evolution of the anomaly score surface by allowing the hyperplane to split along a new feature in each step. Figure %\ref{fig:scoremap 6 IF vs EIF} 
vividly demonstrates the gradual elimination of artifact-prone regions.

\begin{figure}[!ht] 
    \centering % <-- added
    \begin{subfigure}{0.33\textwidth}
    \centering
      \includegraphics[trim={0 0 3.5cm 0}, clip, width=\linewidth]{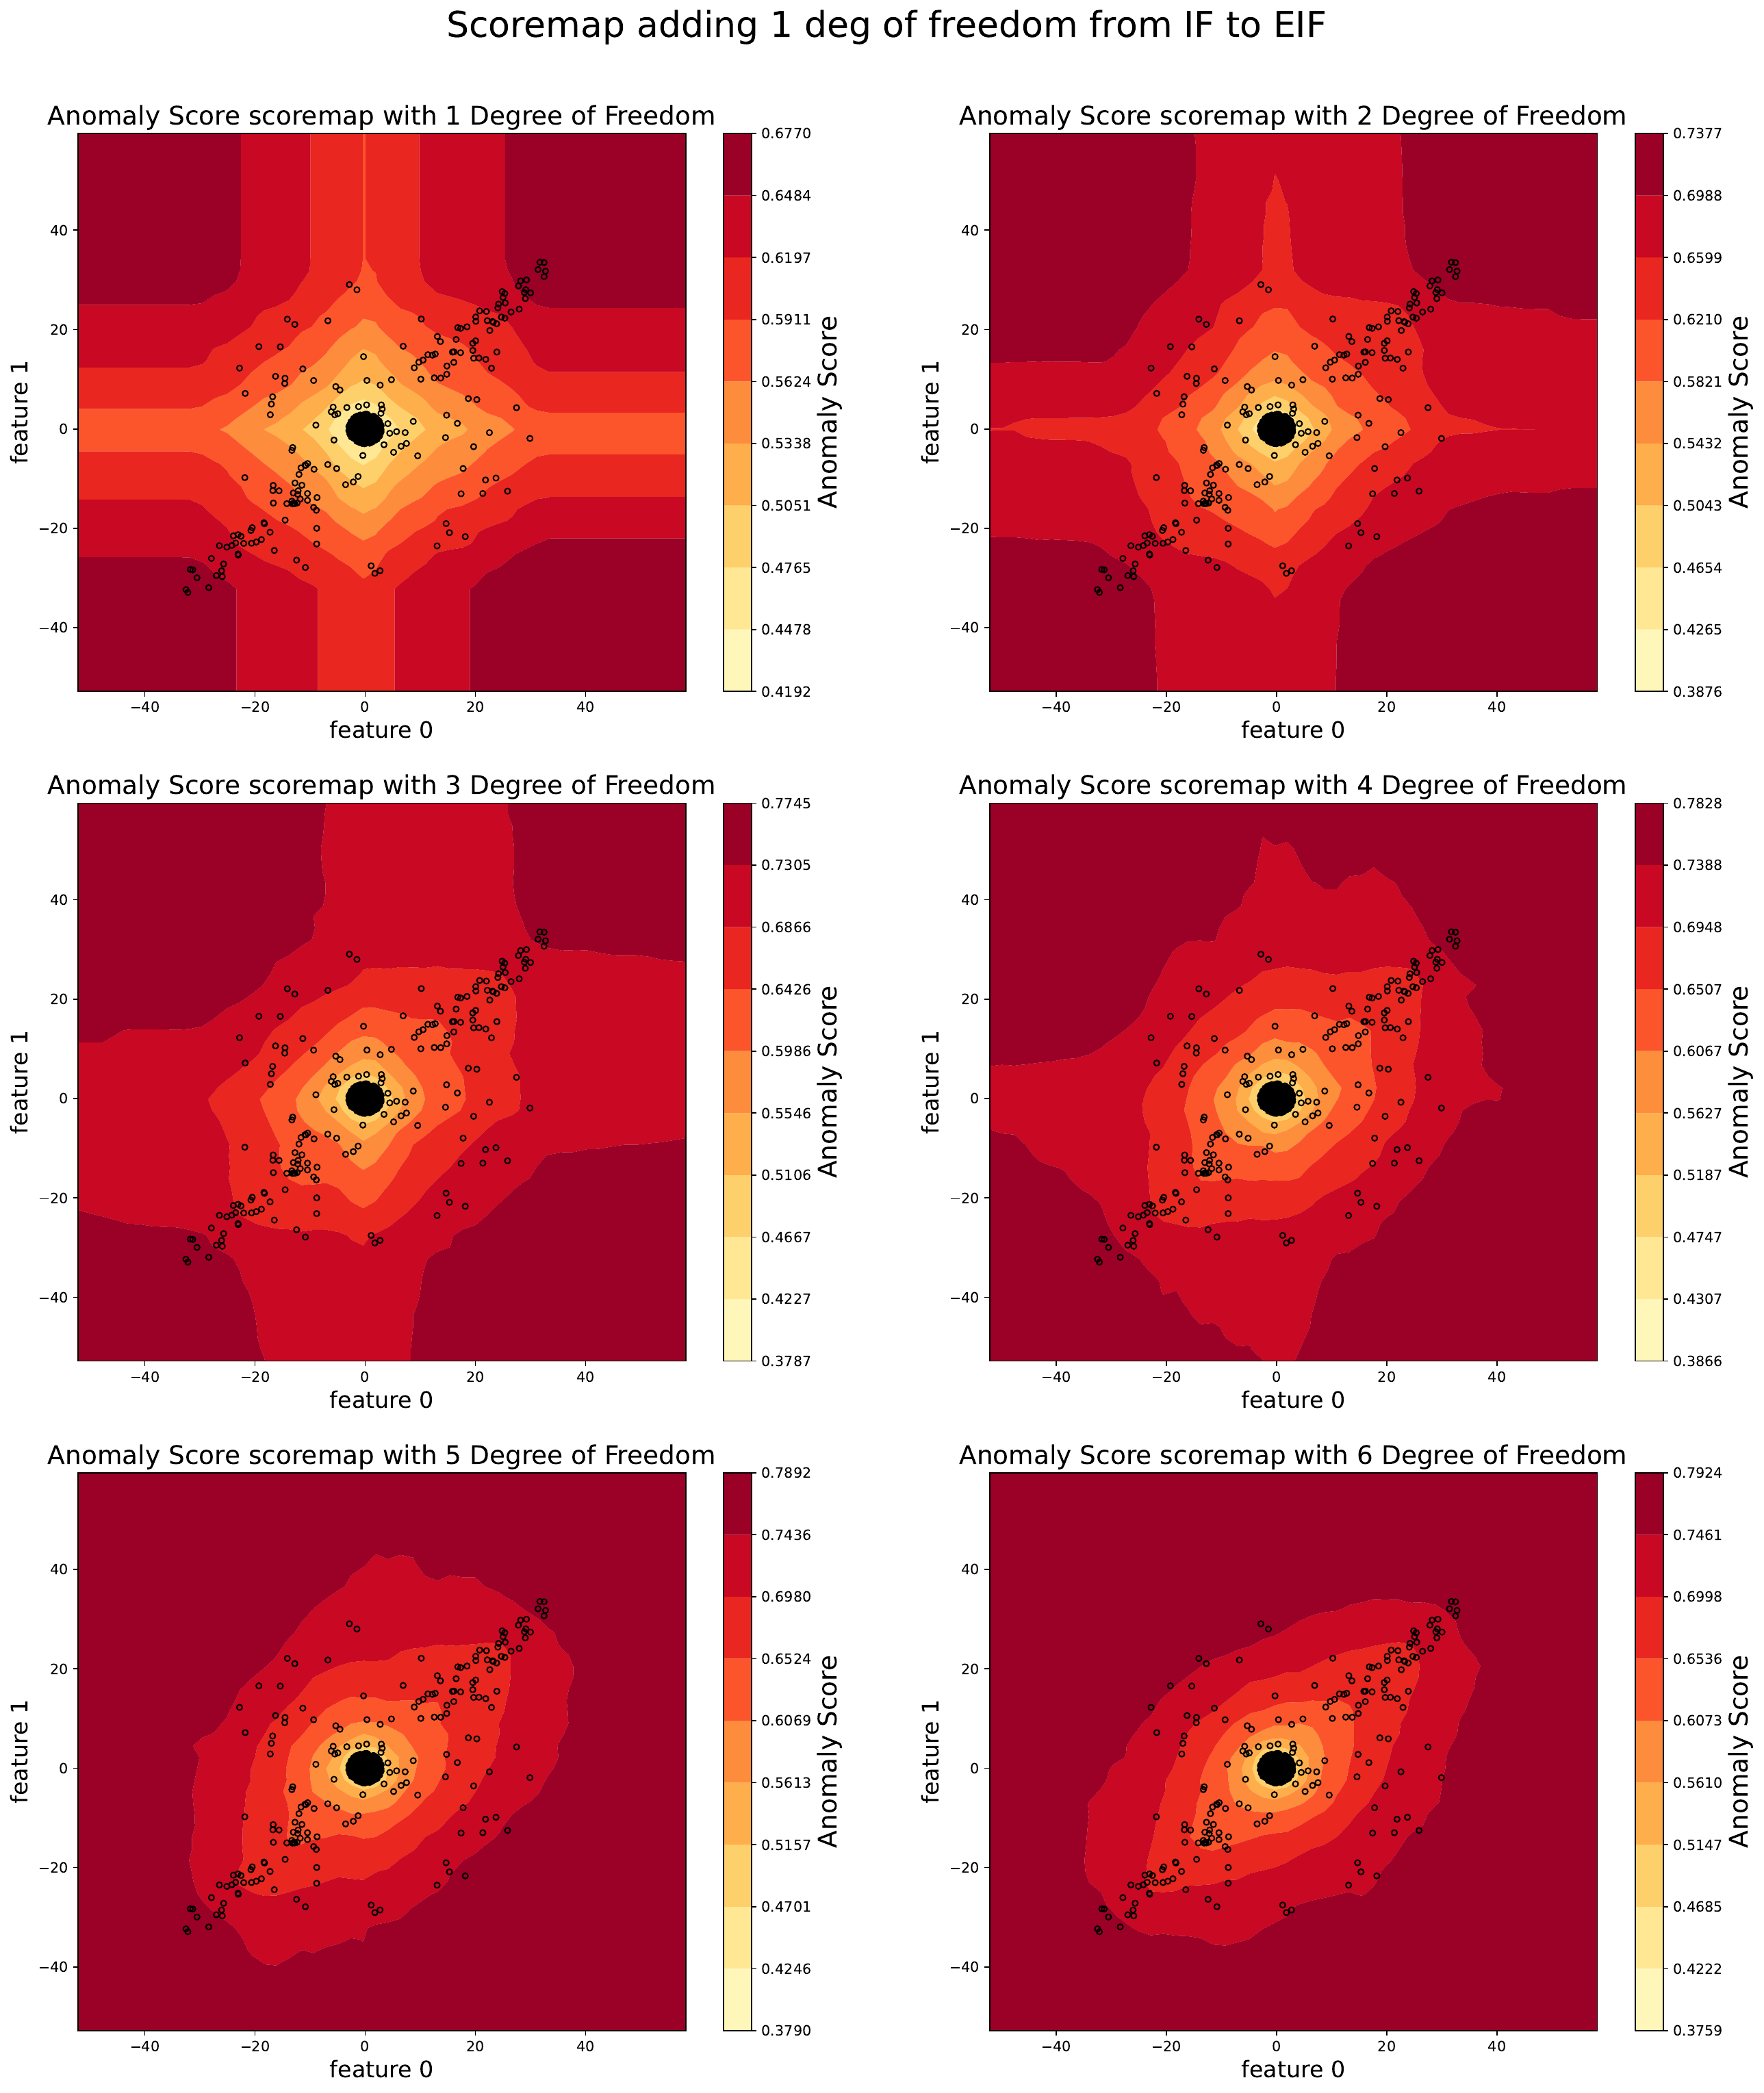}
      \caption{Anomaly Scoremap with 1 degree of freedom}
      \label{fig:scoremap1df}
    \end{subfigure}\hfil % <-- added
    \begin{subfigure}{0.33\textwidth}
    \centering
      \includegraphics[trim={0 0 3.5cm 0}, clip, width=\linewidth]{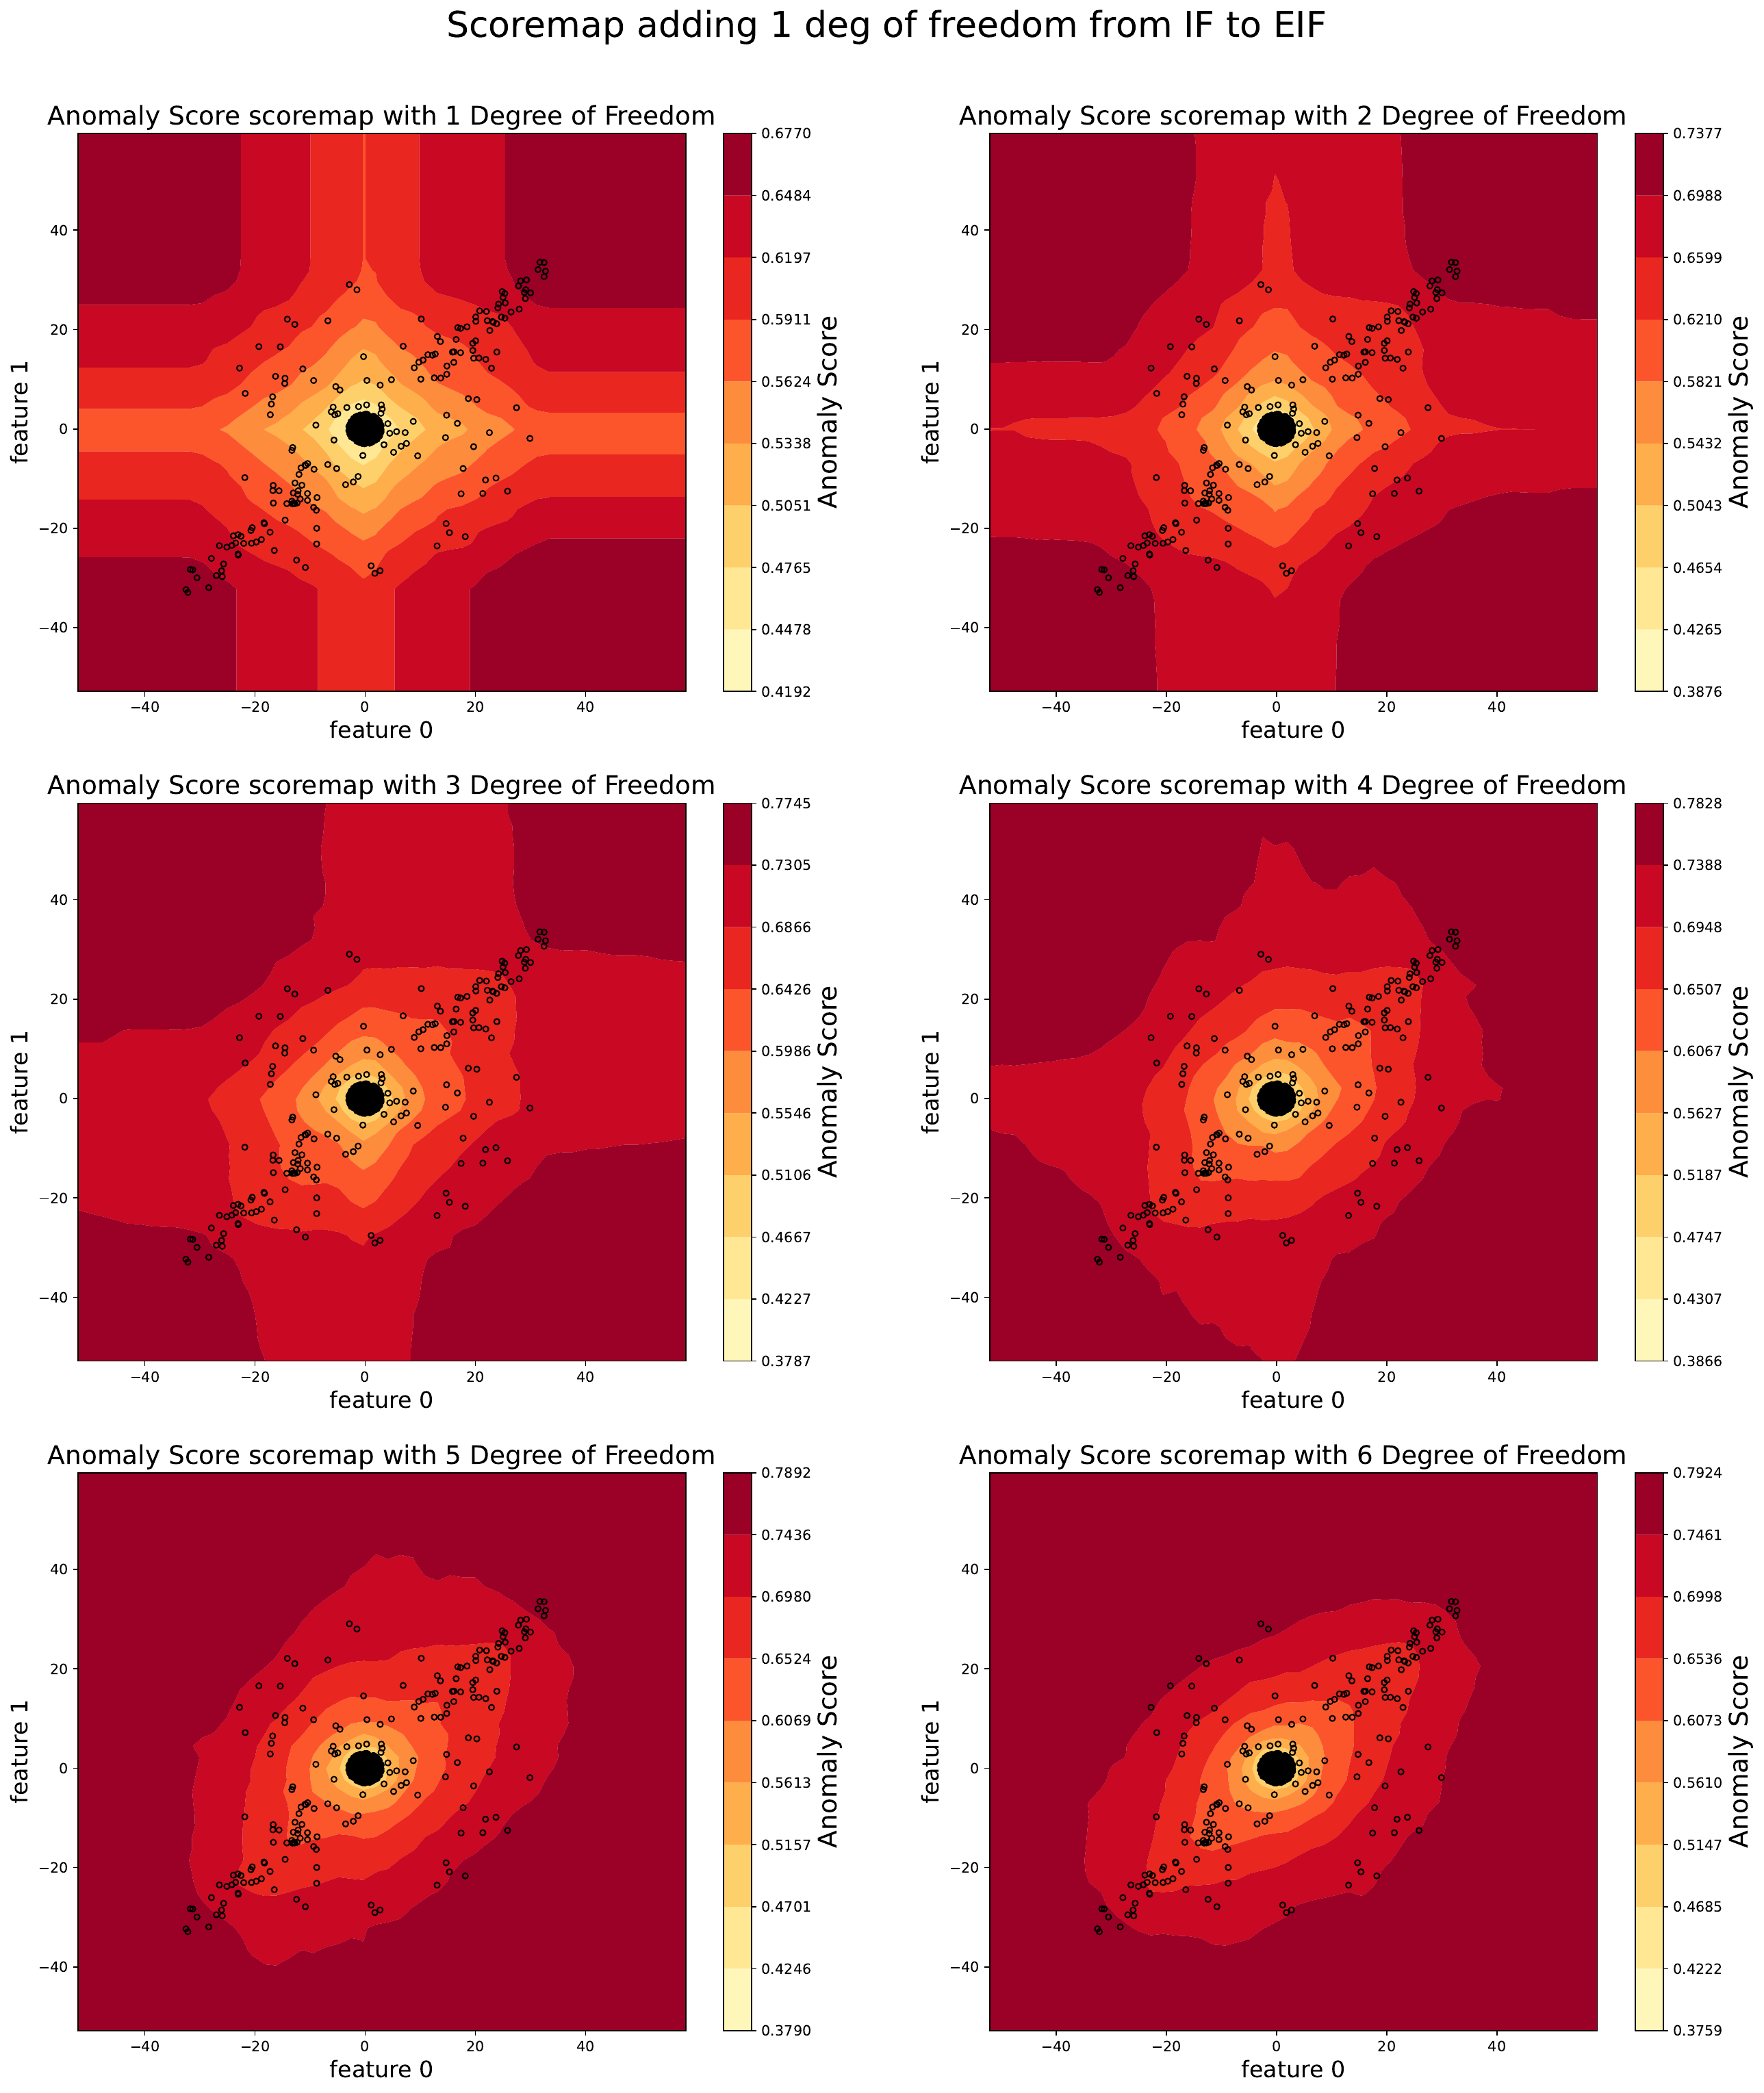}
      \caption{Anomaly Scoremap with 2 degree of freedom}
      \label{fig:scoremap2df}
    \end{subfigure}\hfil % <-- added
    \begin{subfigure}{0.33\textwidth}
    \centering
      \includegraphics[trim={0 0 3.5cm 0}, clip, width=\linewidth]{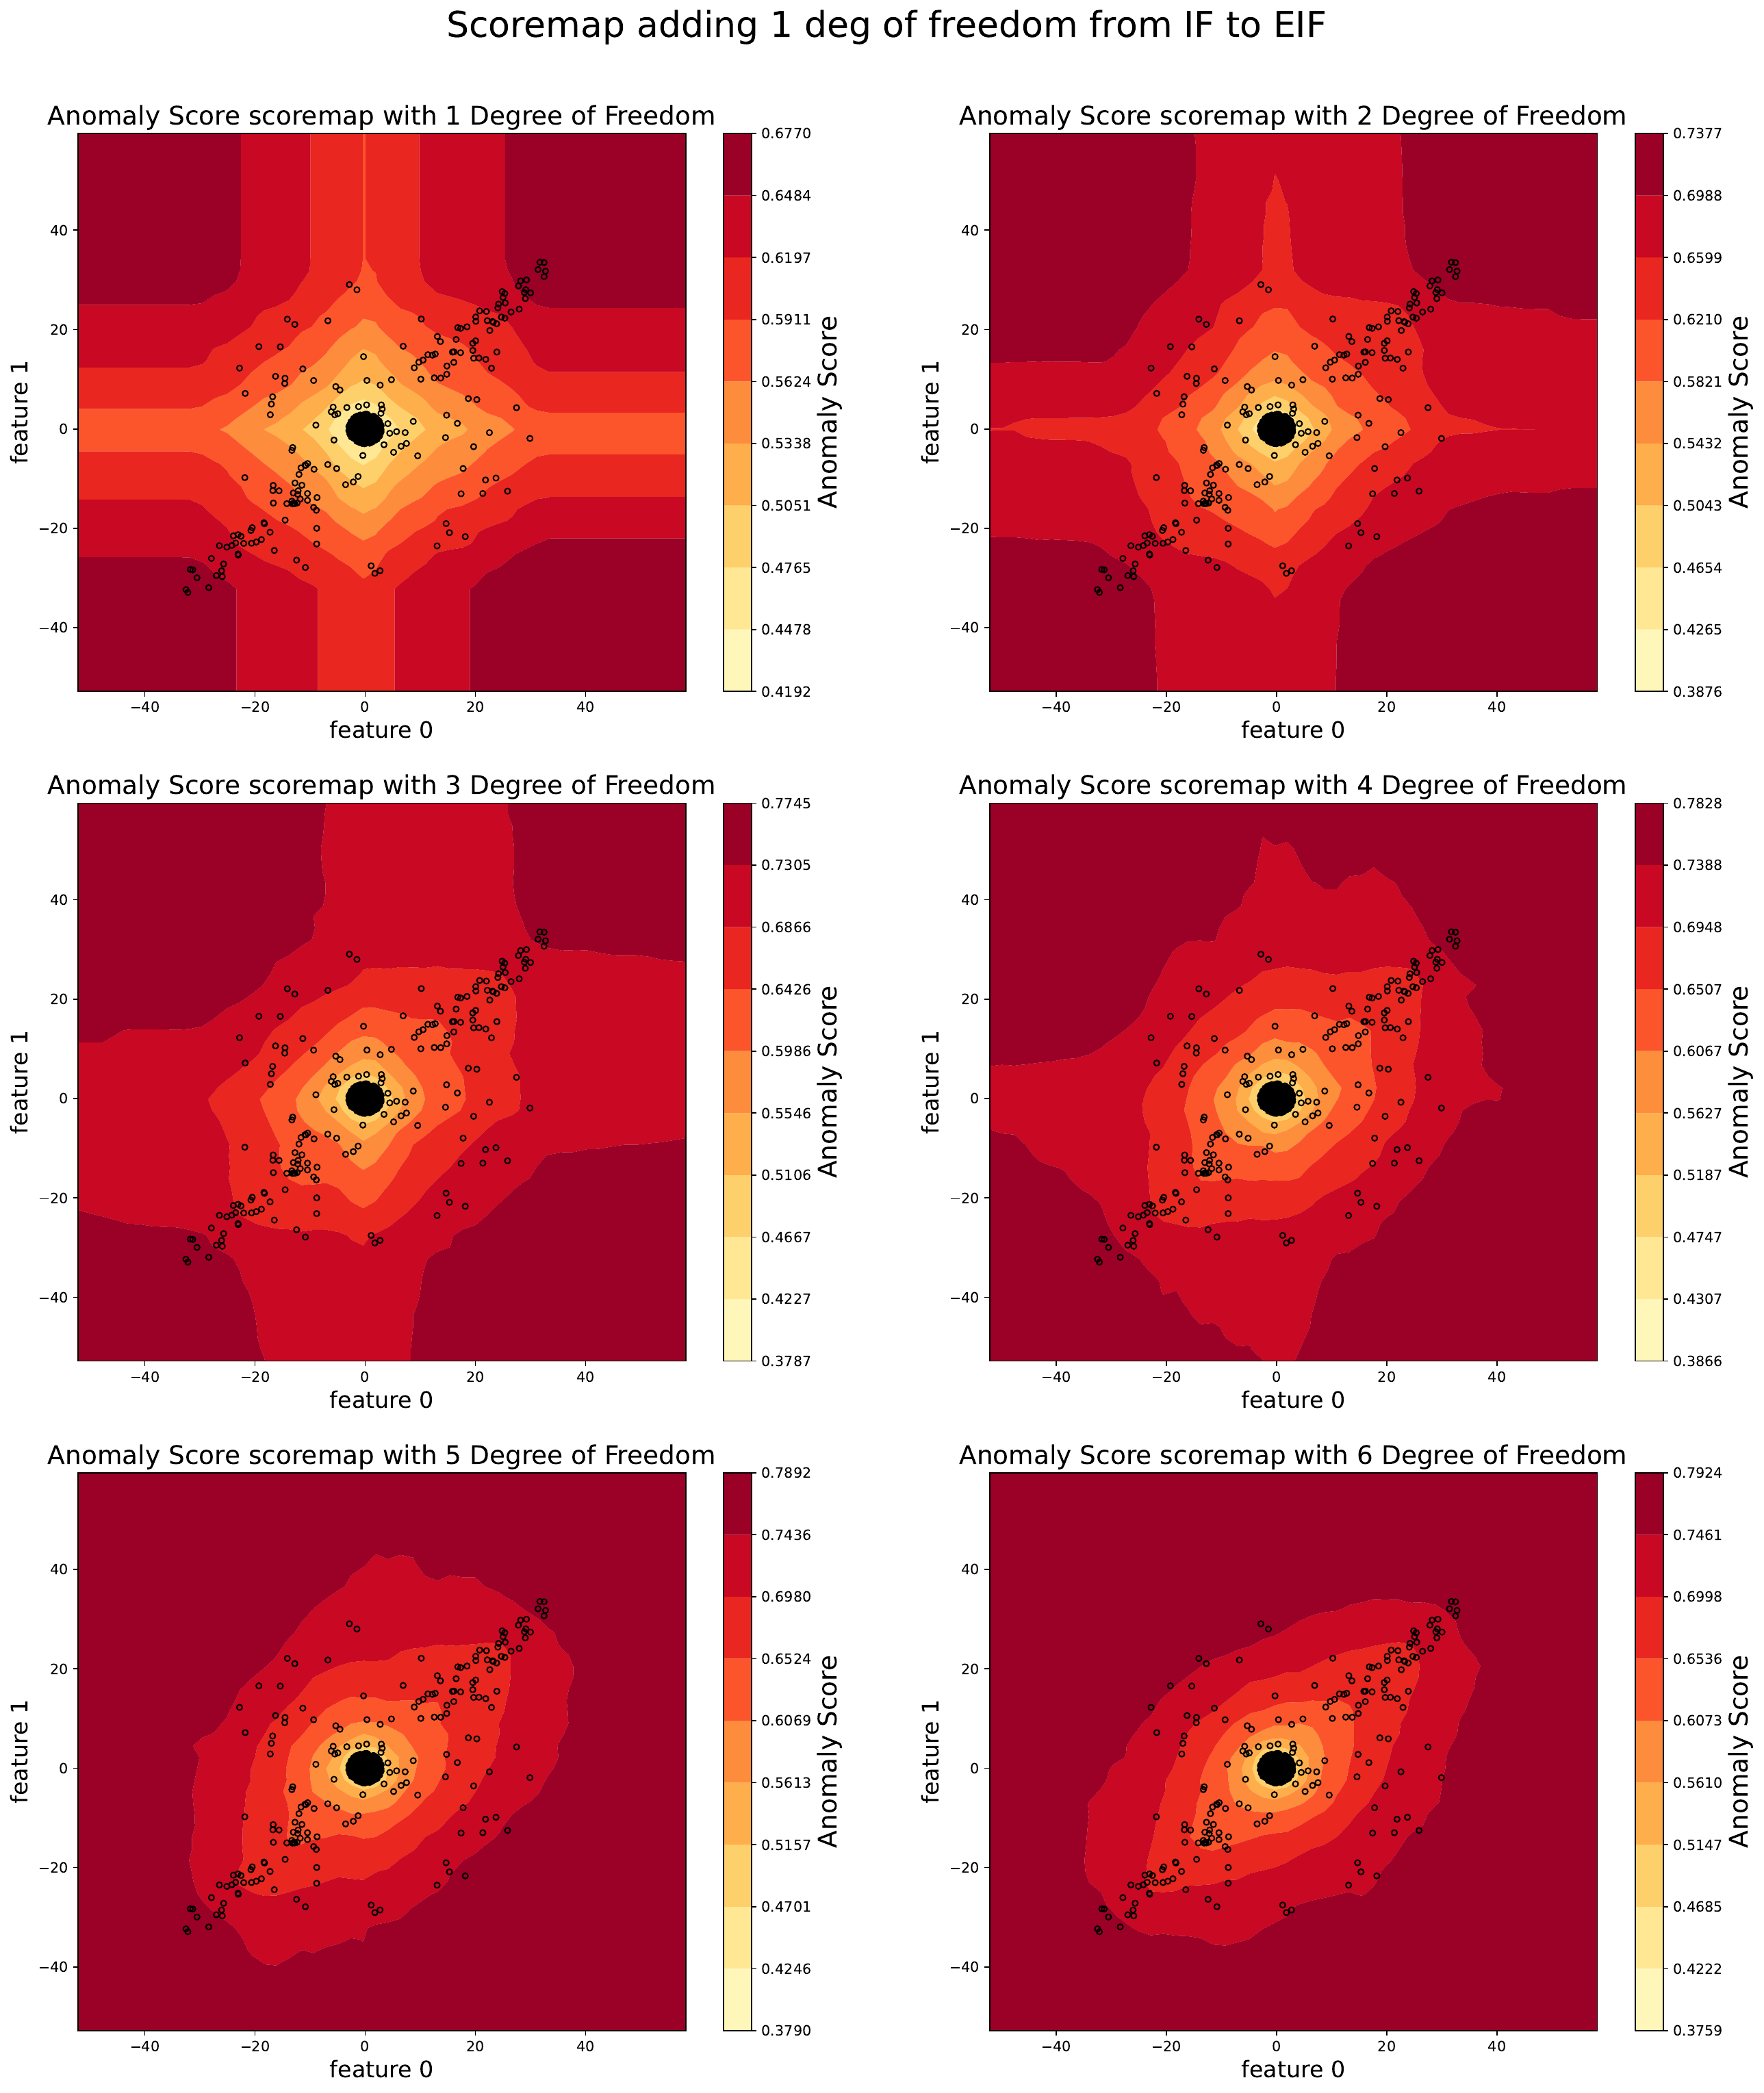}
      \caption{Anomaly Scoremap with 3 degree of freedom}
      \label{fig:scoremap3df}
    \end{subfigure}\hfil % <-- added
    \begin{subfigure}{0.33\textwidth}
    \centering
      \includegraphics[trim={0 0 3.5cm 0}, clip, width=\linewidth]{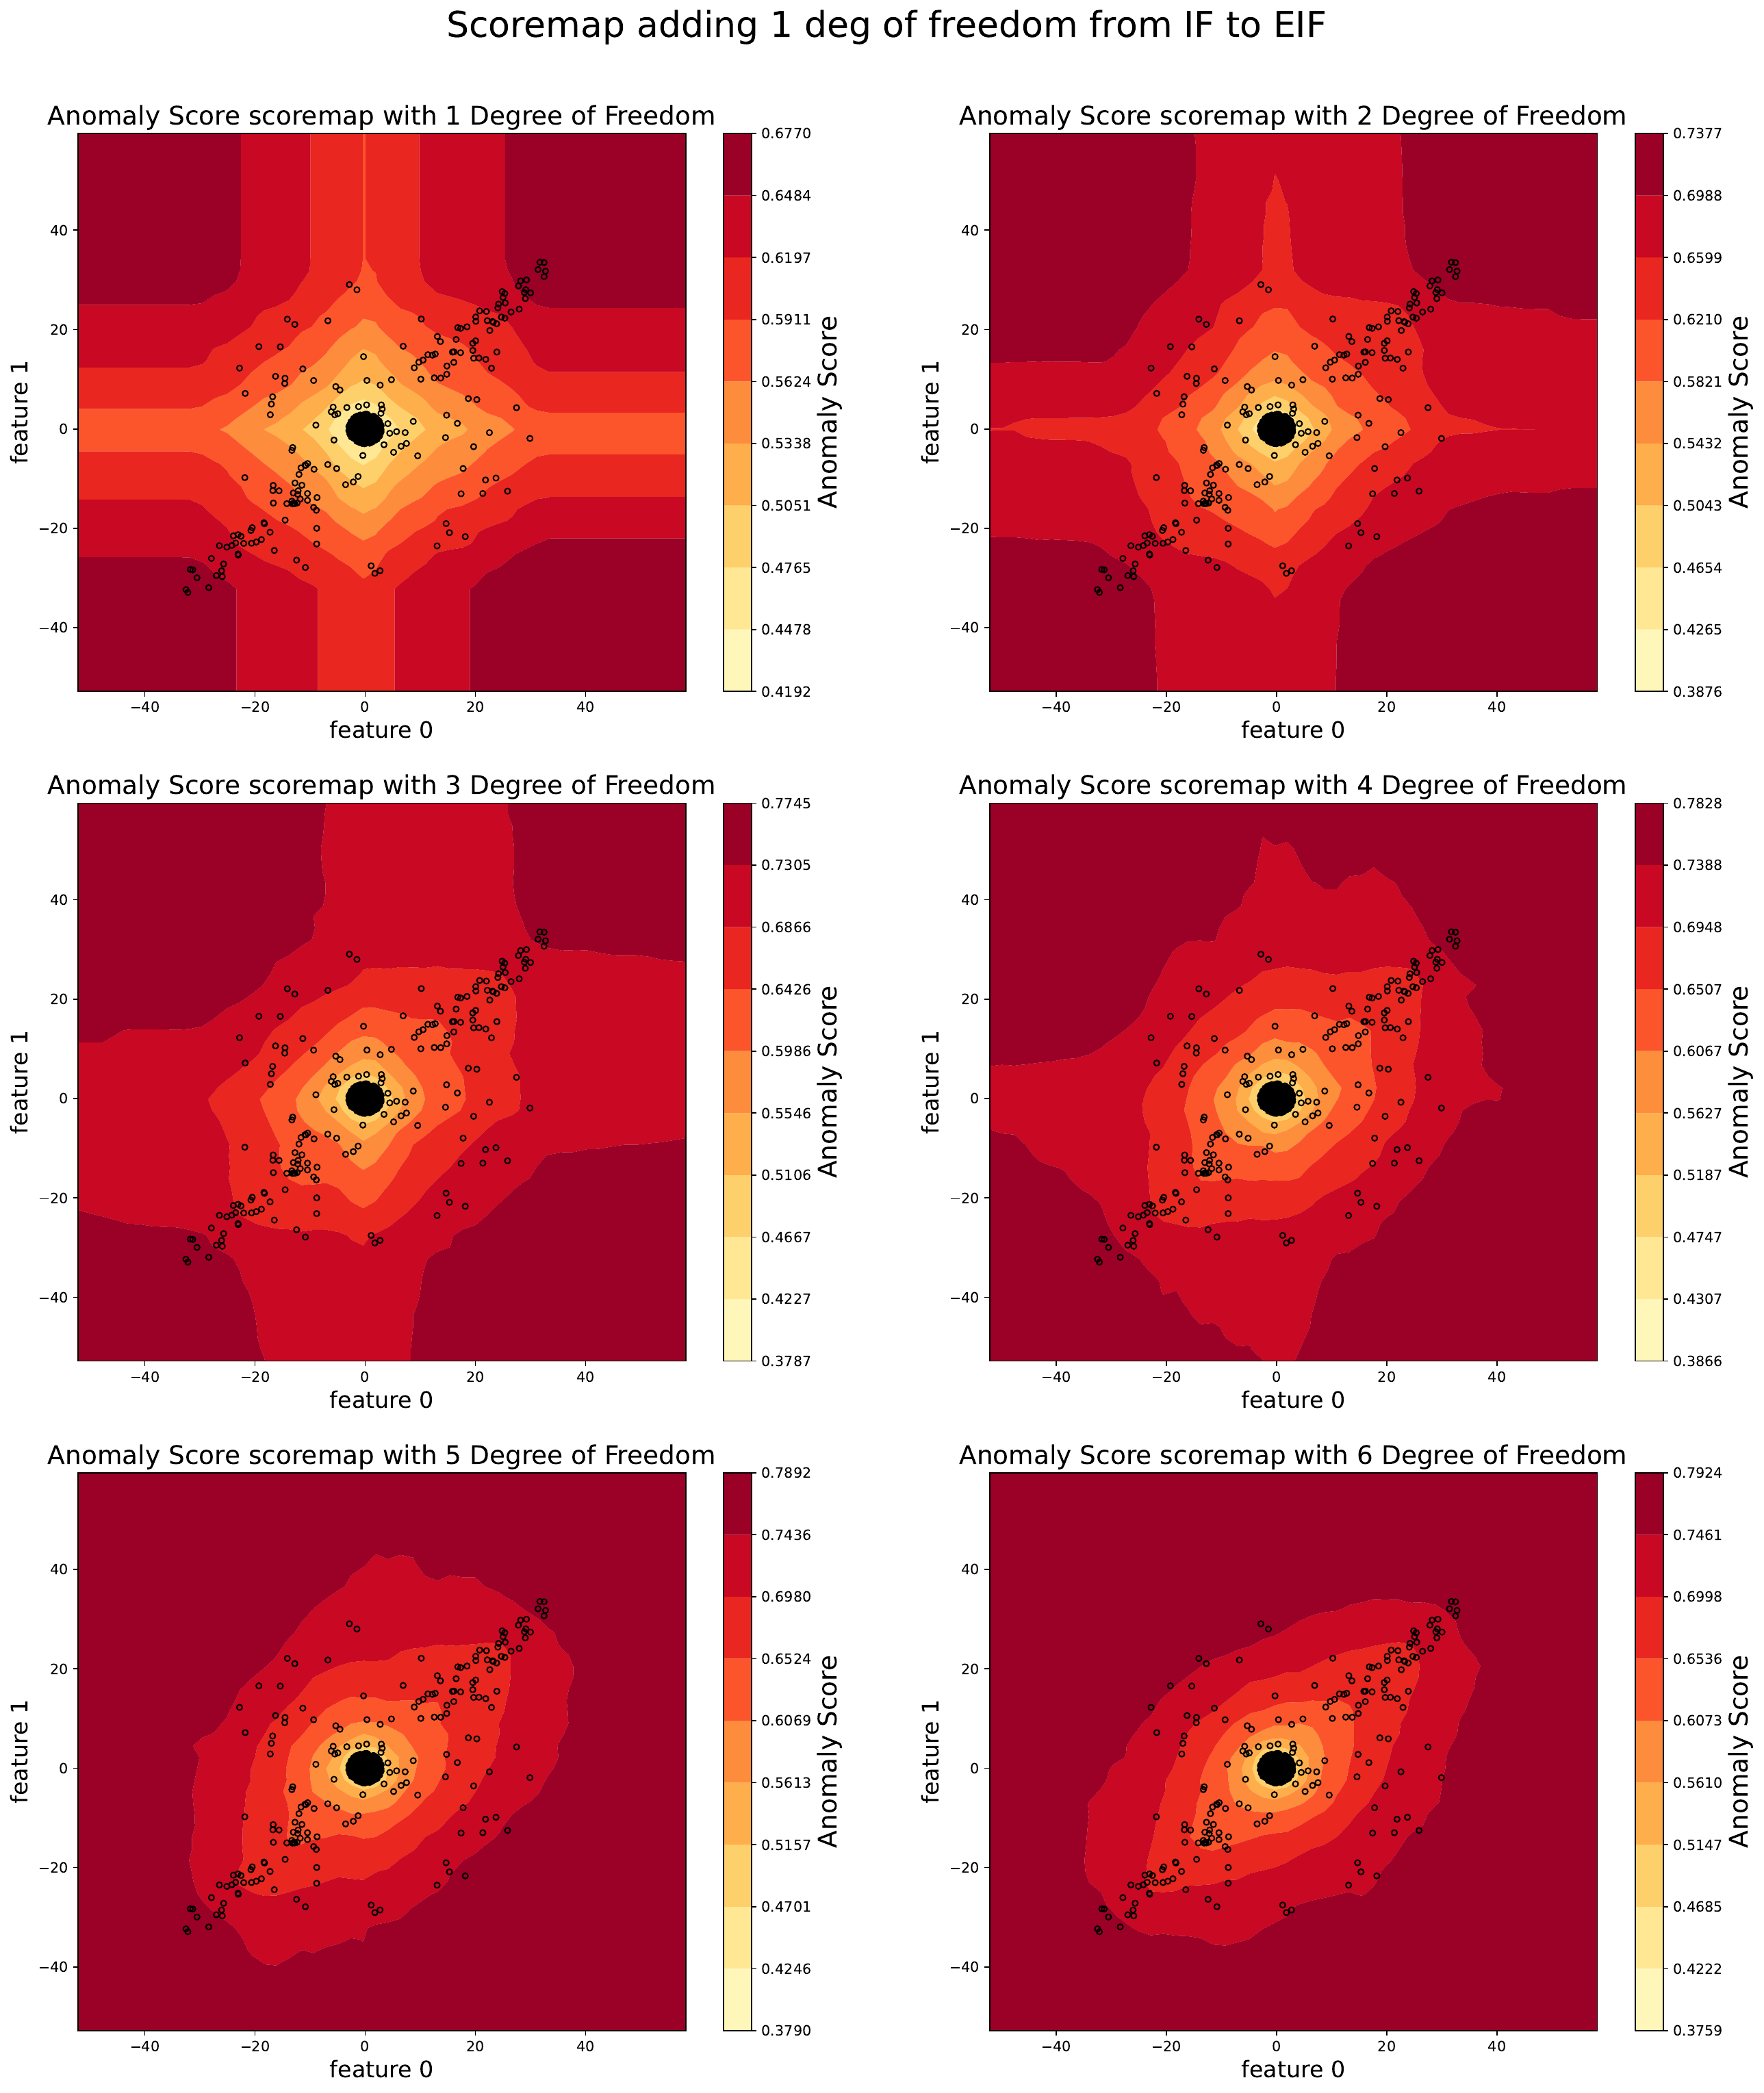}
      \caption{Anomaly Scoremap with 4 degree of freedom}
      \label{fig:scoremap4df}
    \end{subfigure}\hfil % <-- added
    \begin{subfigure}{0.33\textwidth}
    \centering
      \includegraphics[trim={0 0 3.5cm 0}, clip, width=\linewidth]{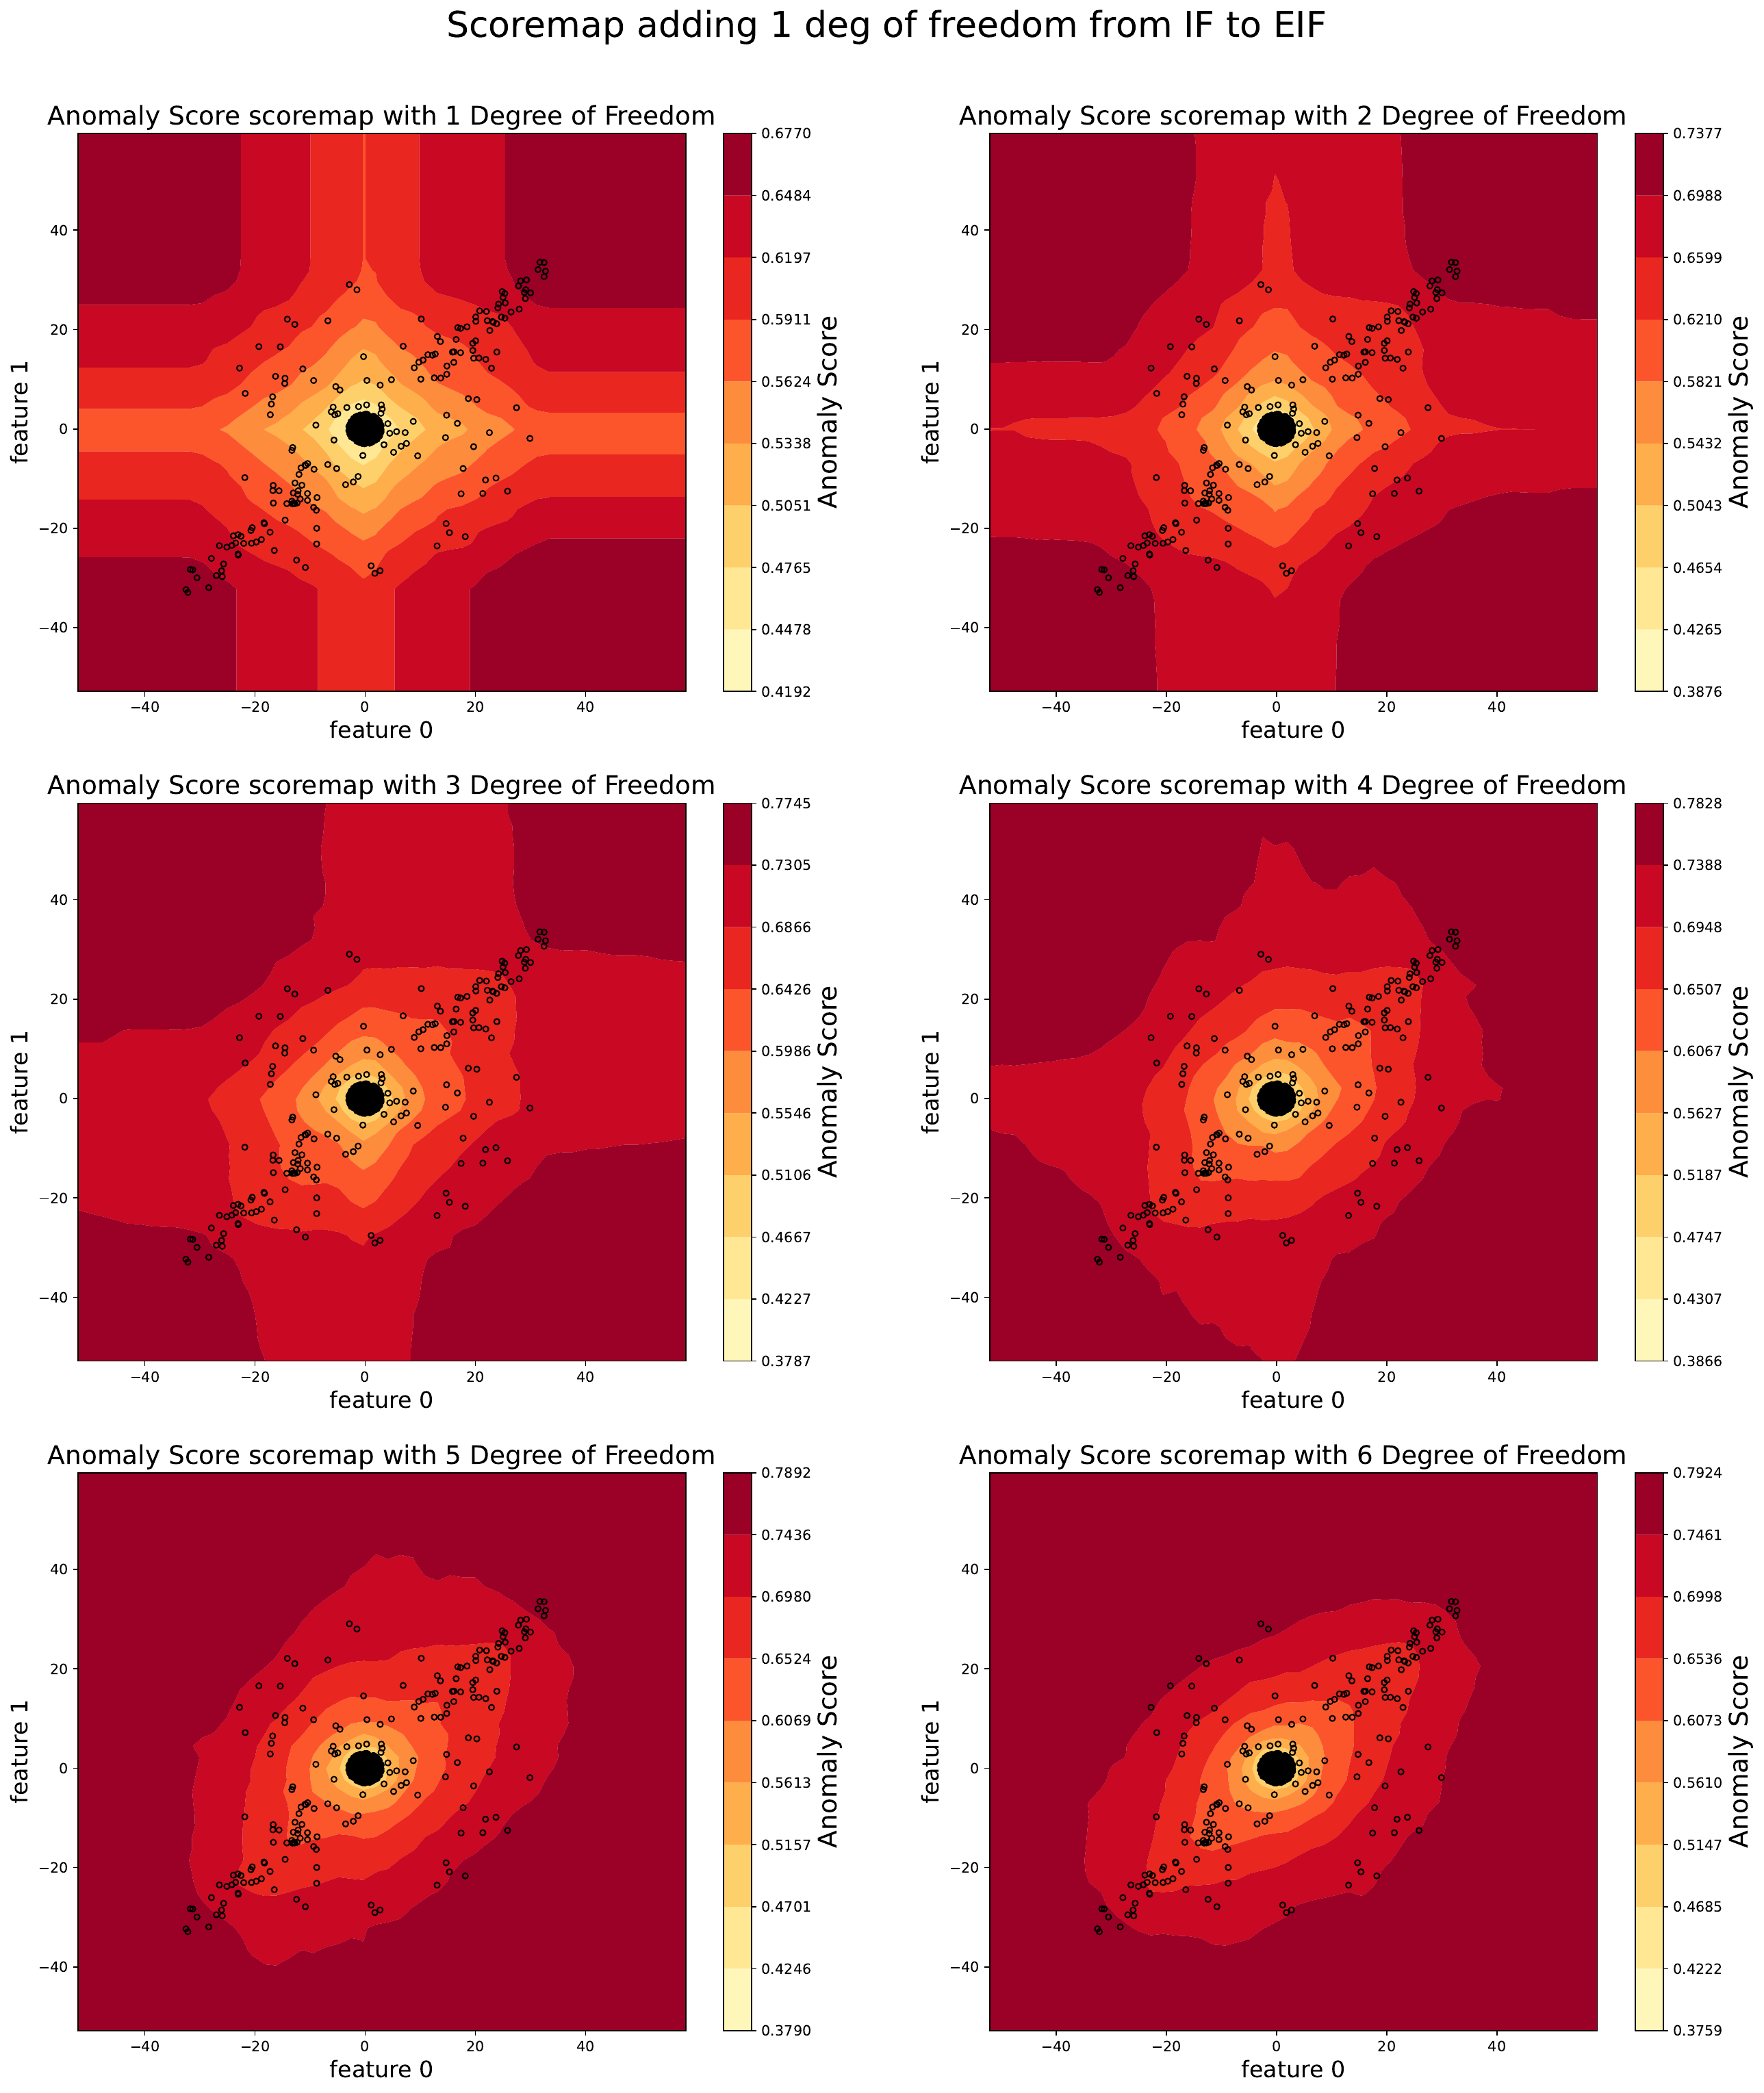}
      \caption{Anomaly Scoremap with 5 degree of freedom}
      \label{fig:scoremap5df}
    \end{subfigure}\hfil % <-- added
    \begin{subfigure}{0.33\textwidth}
    \centering
      \includegraphics[trim={0 0 3.5cm 0}, clip, width=\linewidth]{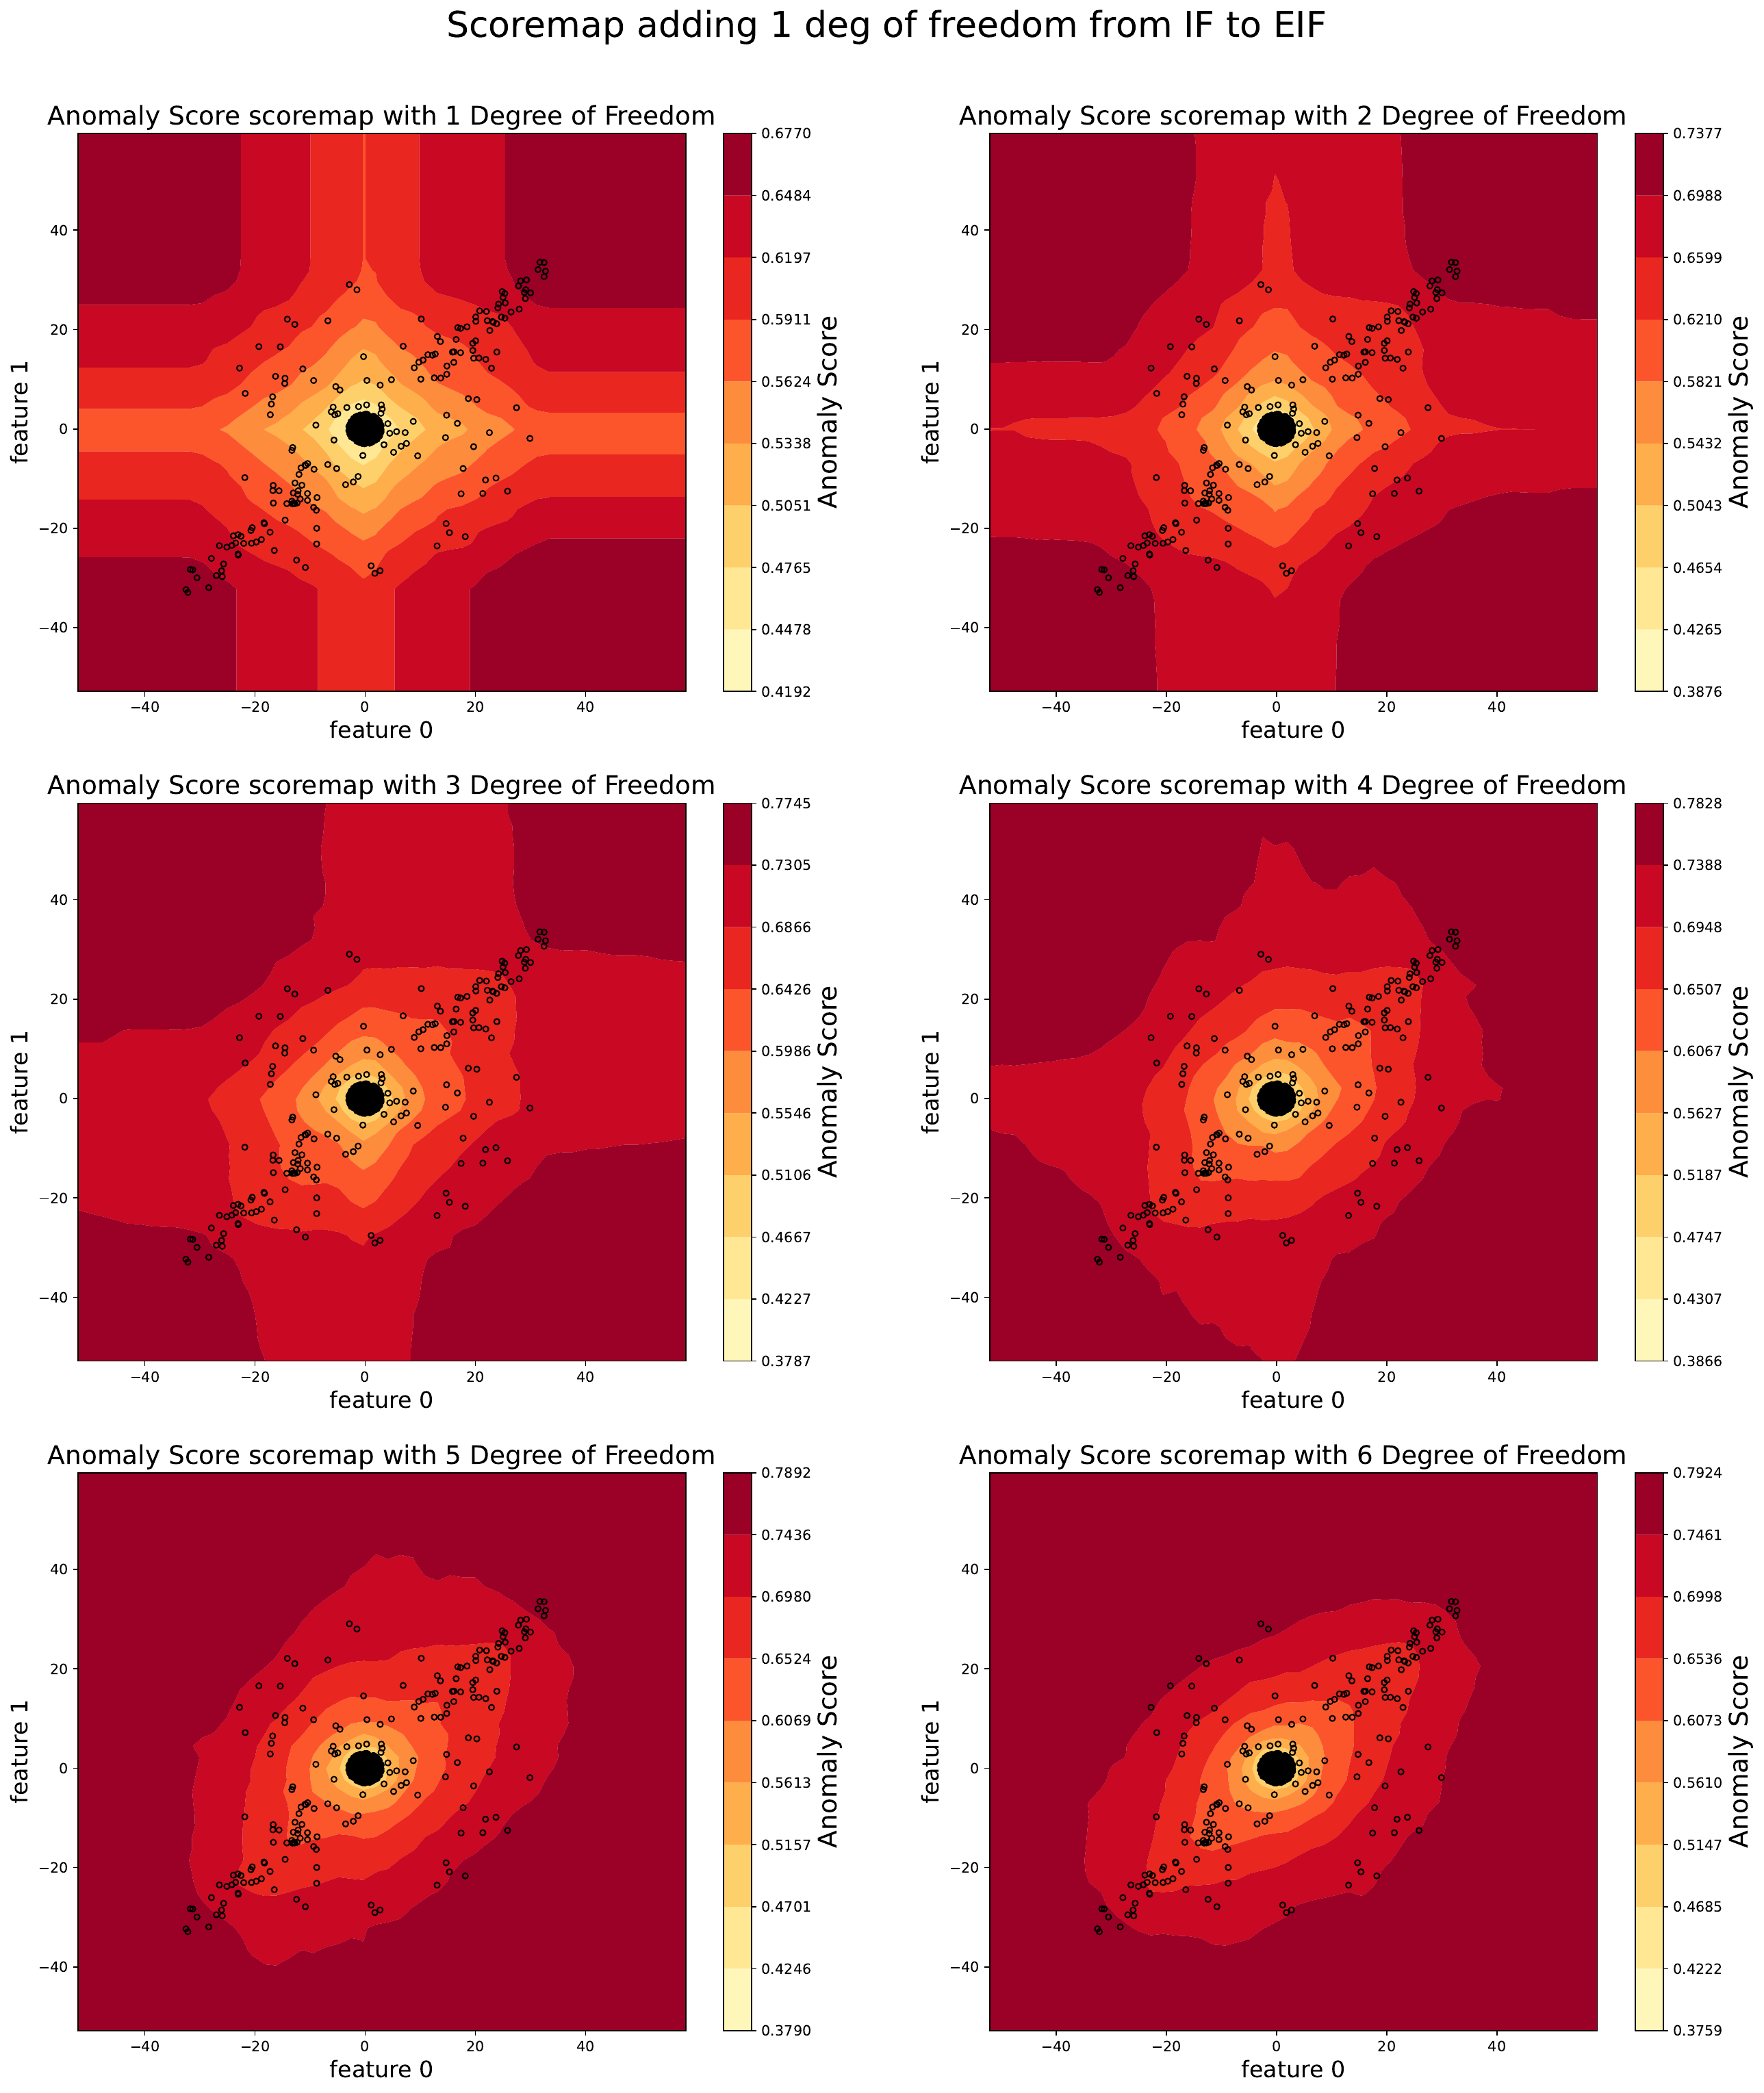}
      \caption{Anomaly Scoremap with 6 degree of freedom}
      \label{fig:scoremap6df}
    \end{subfigure}\hfil % <-- added
\caption{Scoremap resulting from adding one degree of freedom per time while searching for splitting hyperplanes. In this  way we move from the classic IF \ref{fig:scoremap1df} to the EIF \ref{fig:scoremap6df}. {The experiment is performed on the six dimensional space dataset {\ttfamily Bisect} described in Section \ref{sec:appendix-synthetic-data}.}}\label{fig:scoremap 6 IF vs EIF}
\end{figure}
%\feedbackrequired{Vorrei togliere questa immagine enorme e poco interessante per quanto riguarda il paper}
%\todo{sposterei la parte seguente nella sezione successiva lasciando questa solo ad un paragone qualitativo del modello IF vs EIF,EIF+ e dei gradi di libertà}

\begin{comment}
\subsection{Performance Report Table}

This section reports the Performance Report Table (Table \ref{tab:perf-rep-tab-complete}) containing the values of the typical Classification metrics for all the datasets introduced in this study for both Scenario I and Scenario II. 

To obtain the threshold needed for the computation of the Precision, Recall, and F1 Score metrics, we chose it according to the true contamination factor of each dataset.% , computed exploiting the information coming from the labels provided by the dataset, was used to
The result is that these metrics will have the same value. On the other hand, the Average Precision metric is not affected by the contamination factor since it is computed as the Area Under the Curve of the Precision-Recall Curve which considers different classifier thresholds and thus multiple different values for the contamination factor.

\input{tables/score_appendix_table}
 \end{comment}

\subsection{Non Depth-Based importance}
In general, it is accurate to assert that the amount of feature importance attributed by a particular node $k$ to a given sample $x$, provided that the node effectively separates the samples, should be greater if the node is closer to the root of the tree, and the importance score should decrease as the node becomes deeper within the tree. This principle is derived from the same concept used to determine anomaly scores, which are higher for samples that on average are in leafs closer to the root of the tree.

Two distinct approaches exist for assigning importance scores to nodes the one used in the \approach algorithm and the one of which is proposed by the DIFFI algorithm. 
The DIFFI algorithm importance scores are assigned to nodes based on a weighting scheme that inversely relates the score to the depth of the node. This approach is parameterized to ensure that scores decrease as nodes become deeper within the tree.

The \approach algorithm is an alternative approach for assigning importance scores to nodes in a decision tree, which differs from the DIFFI algorithm by not using the inverse of the depth to decrease the score as the node becomes deeper in the tree. This stems from the fact that the maximum acceptable score for a node is directly linked to the number of elements it must partition. As the depth of the node increases, this number inevitably decreases. Therefore, we assert that it is redundant and potentially misleading to incorporate an additional parameter to weigh the importance score.

The underlying idea is that as the node becomes deeper in the tree, it is responsible for splitting fewer and fewer elements, and therefore, it should not be penalized by reducing its importance score because the structure of the algorithm itself decreases the importance on average after every step deeper in the tree. In contrast, a node that splits many elements closer to the root of the tree may be more important because it has a greater impact on the separation of the data, but its importance should not be guaranteed by an external factor.

The EXIFFI algorithm adjusts the maximum score acceptable for a node based on the number of elements it needs to split, which allows for a fair comparison of the importance of nodes across different depths in the tree. This approach can help to avoid overestimating the importance of nodes that are close to the root and underestimating the importance of nodes that are deeper in the tree, risk that the DIFFI algorithm does not take into account.

\begin{figure}[!ht] 
    \centering % <-- added
    \begin{subfigure}{0.45\textwidth}
      \includegraphics[trim={1cm 1cm 1.5cm 1.7cm}, clip, width=\linewidth]{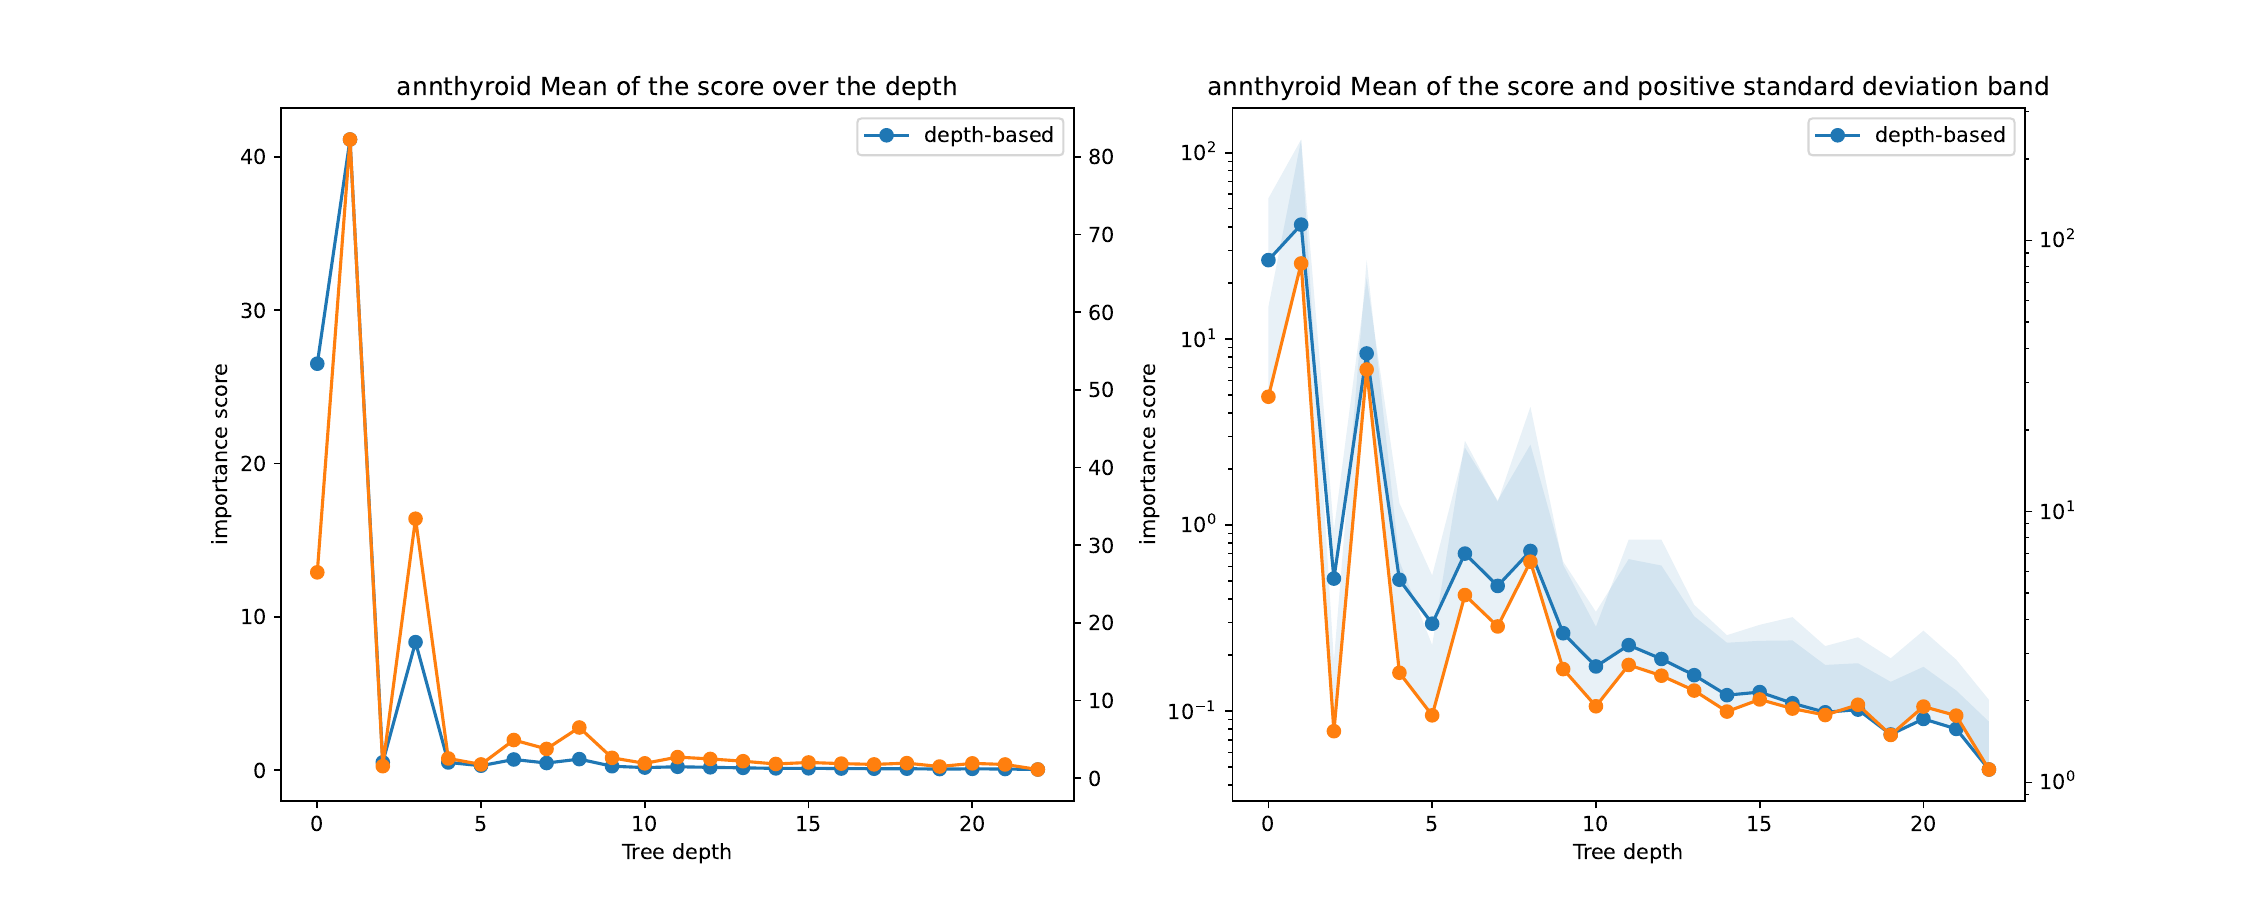}
        \caption{{\ttfamily Annthyroid}}\label{fig:depth_annthyroid}
    \end{subfigure}\hfil % <-- added
    \begin{subfigure}{0.45\textwidth}
      \includegraphics[trim={1cm 1cm 1.5cm 1.7cm}, clip, width=\linewidth]{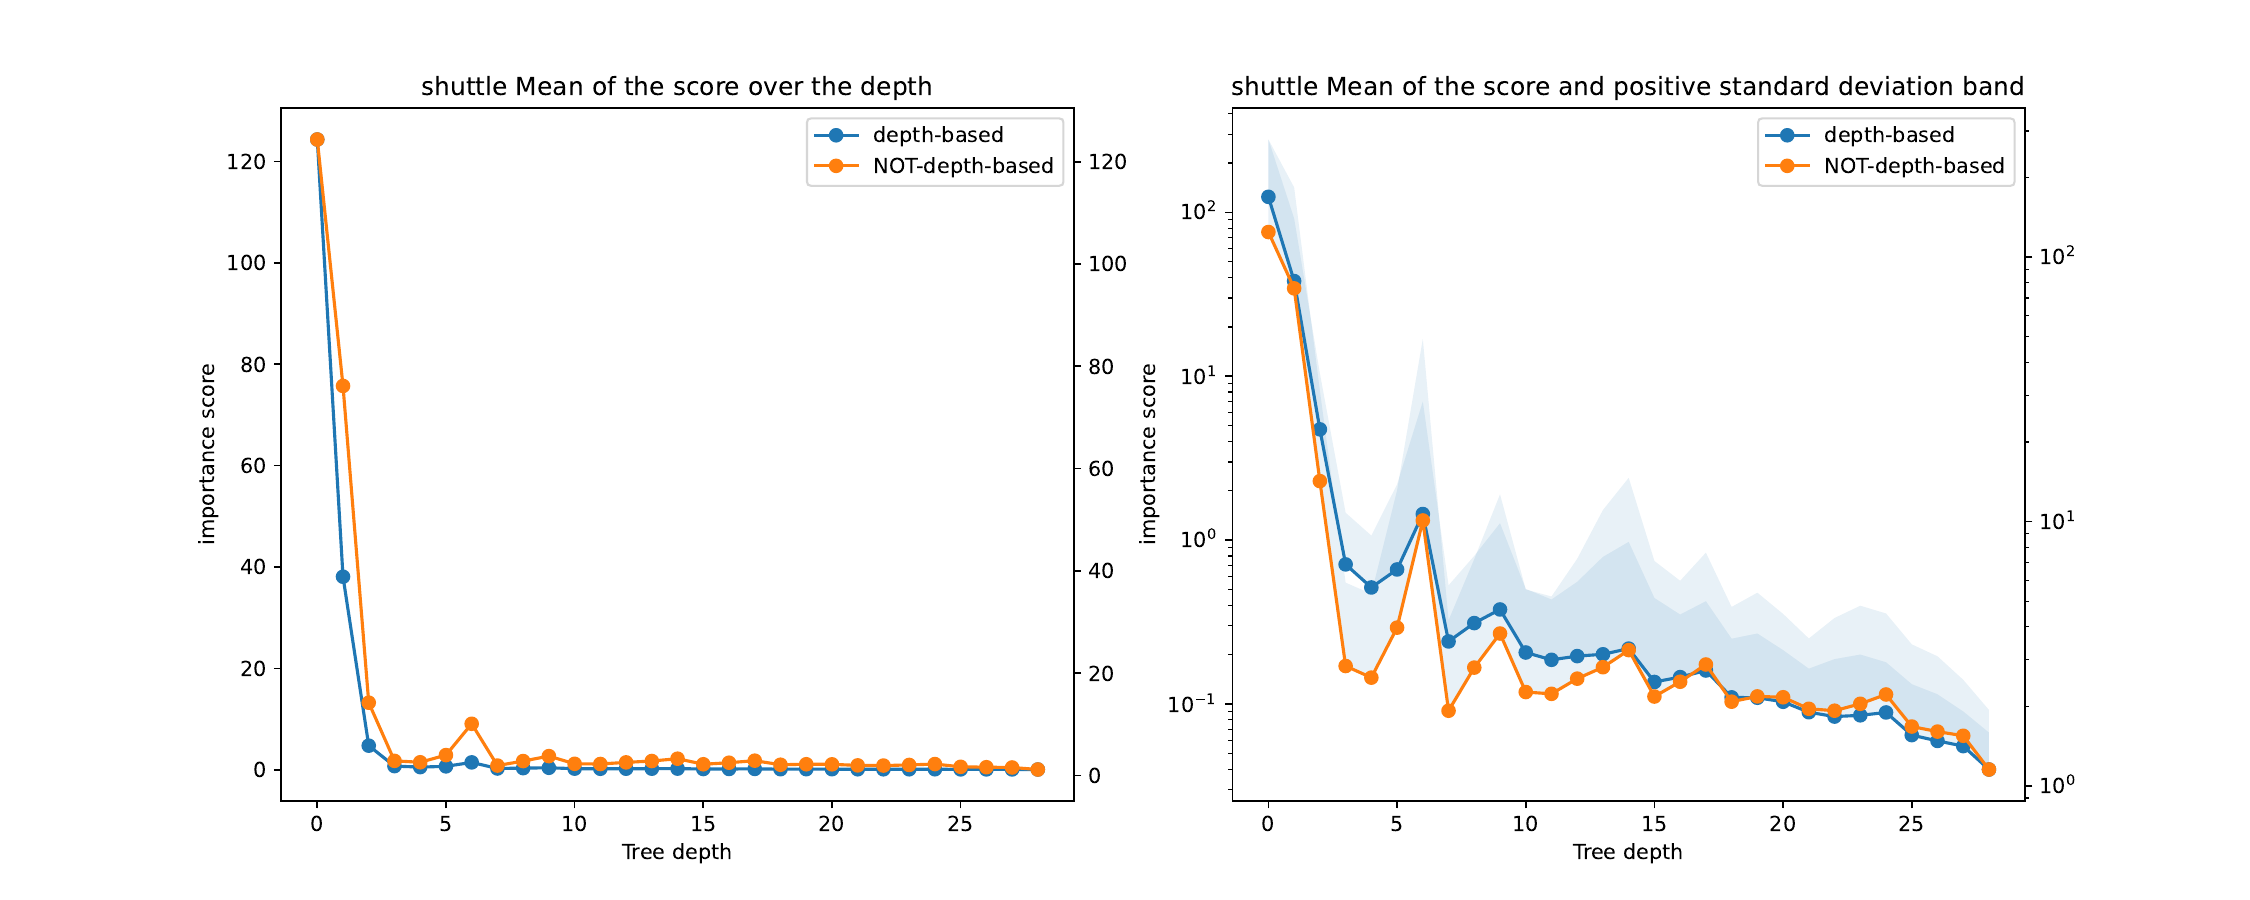}
        \caption{{\ttfamily Shuttle}}\label{fig:depth_shuttle}
    \end{subfigure}\hfil % <-- added
    \begin{subfigure}{0.45\textwidth}
      \includegraphics[trim={1cm 1cm 1.5cm 1.7cm}, clip, width=\linewidth]{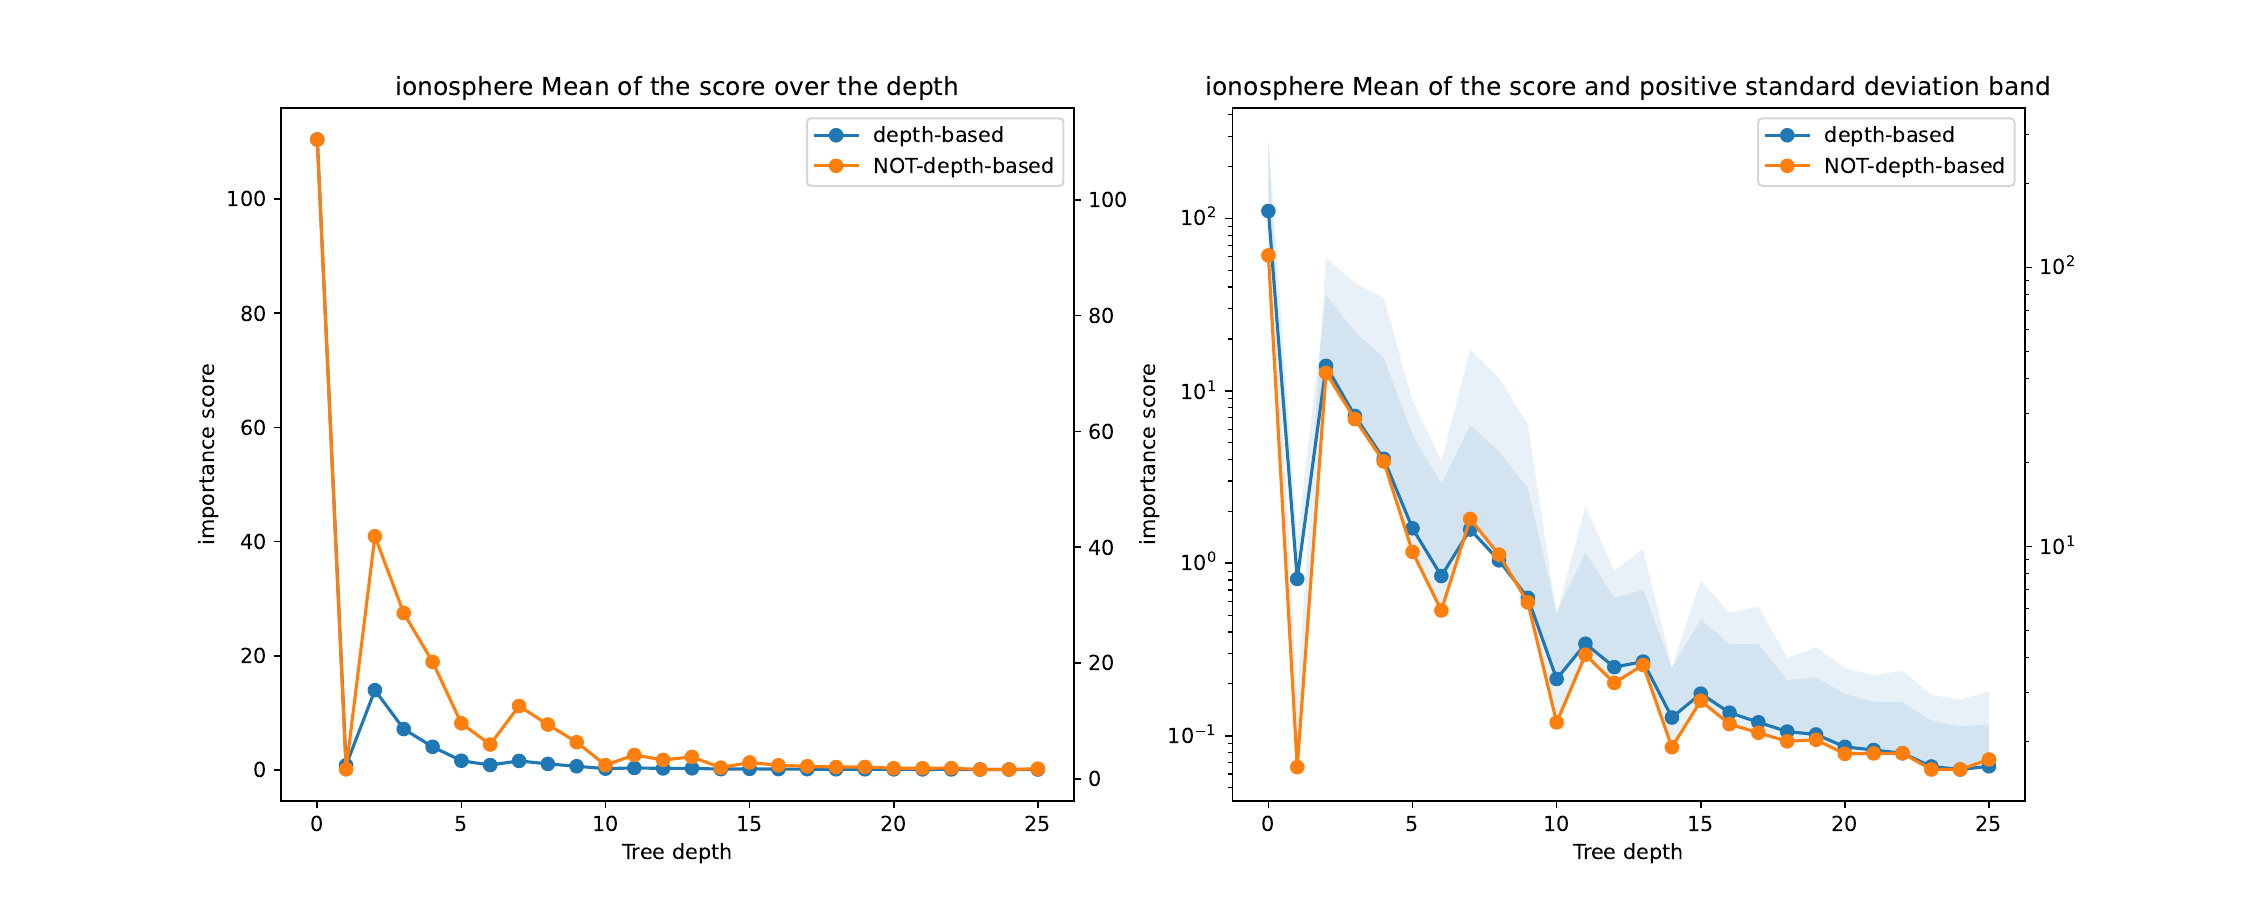}
    \caption{{\ttfamily Ionosphere}}\label{fig:depth_ionosphere}
    \end{subfigure}\hfil % <-- added
        \begin{subfigure}{0.45\textwidth}
      \includegraphics[trim={1cm 1cm 1.5cm 1.7cm}, clip, width=\linewidth]{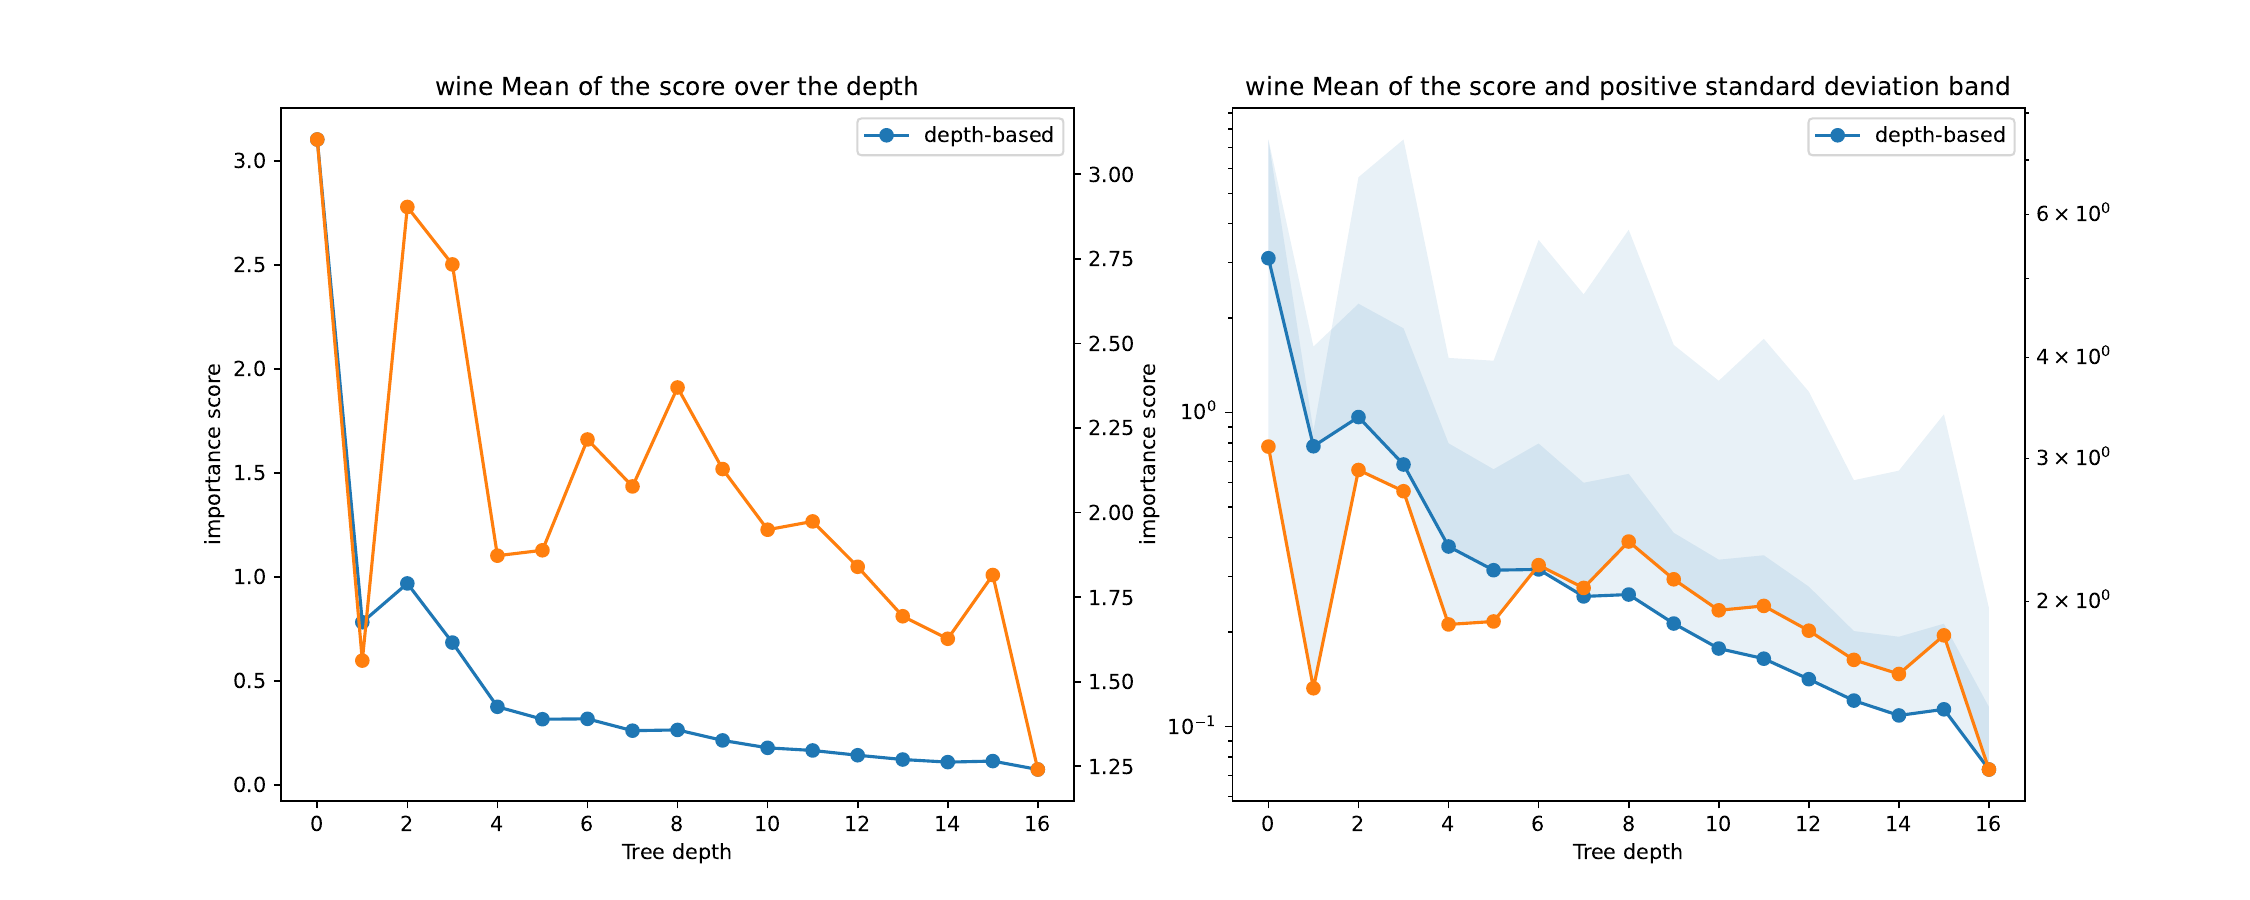}
    \caption{{\ttfamily Wine}}\label{fig:depth_wine}
    \end{subfigure}\hfil % <-- added

\caption{Analysis of the average scores of the nodes related to their depth.}\label{fig:depth}
\end{figure}

We conducted an analysis of the ExIFFI algorithm with and without the depth parameter, in order to identify differences in the evolution of the score at different depths of the trees. To achieve this, we plotted the average score of the nodes at various levels of depth in the forests, as shown in Figure \ref{fig:depth}.

The results of this analysis indicate that the score generally decreases without the use of a depth parameter. Although the ExIFFI algorithm without the depth parameter produced higher scores, the overall shape of the graph is still descending as nodes are evaluated deeper in the tree. This suggests that the ExIFFI algorithm is effective in assigning importance scores to nodes, even when the depth parameter is not utilized.

In summary, our analysis suggests that the ExIFFI algorithm is a robust method for assigning importance scores to nodes in decision trees, with or without the use of a depth parameter.

\subsection{Complete Local Scoremaps}\label{sec:complete-scoremaps}

A useful instrument for the selection of the best pair of features to include in the Local Scoremap is represented by the so-called Complete Local Scoremap. 

In scenarios in which a comprehensive analysis is sought, a more exhaustive study would involve the inspection of Local Importance Scoremaps covering all conceivable pairs of features. By systematically aggregating the acquired scoremaps into a composite "matrix of plots" a lucid comprehension of the hierarchy among the most and least influential features can be derived. 

Furthermore, this additional graphical instrument allows for conducting a profound and detailed graphical analysis of the dataset and its features in order to achieve a qualitative comprehension of the model's output other than just considering the mere Feature importance scores.

For sake of readability, only the Complete Local Scoremap of the {\ttfamily Diabetes} dataset is presented here (Figure \ref{fig:Local-diabetes-complete}. The Complete Scoremaps of the remaining datasets are contained in the GitHub Repository of this study \footnote{The GitHub Repository can be found at: https://github.com/alessioarcudi/ExIFFI}.

\begin{figure}[!ht] 
    \centering 
      \includegraphics[width=0.5\linewidth]{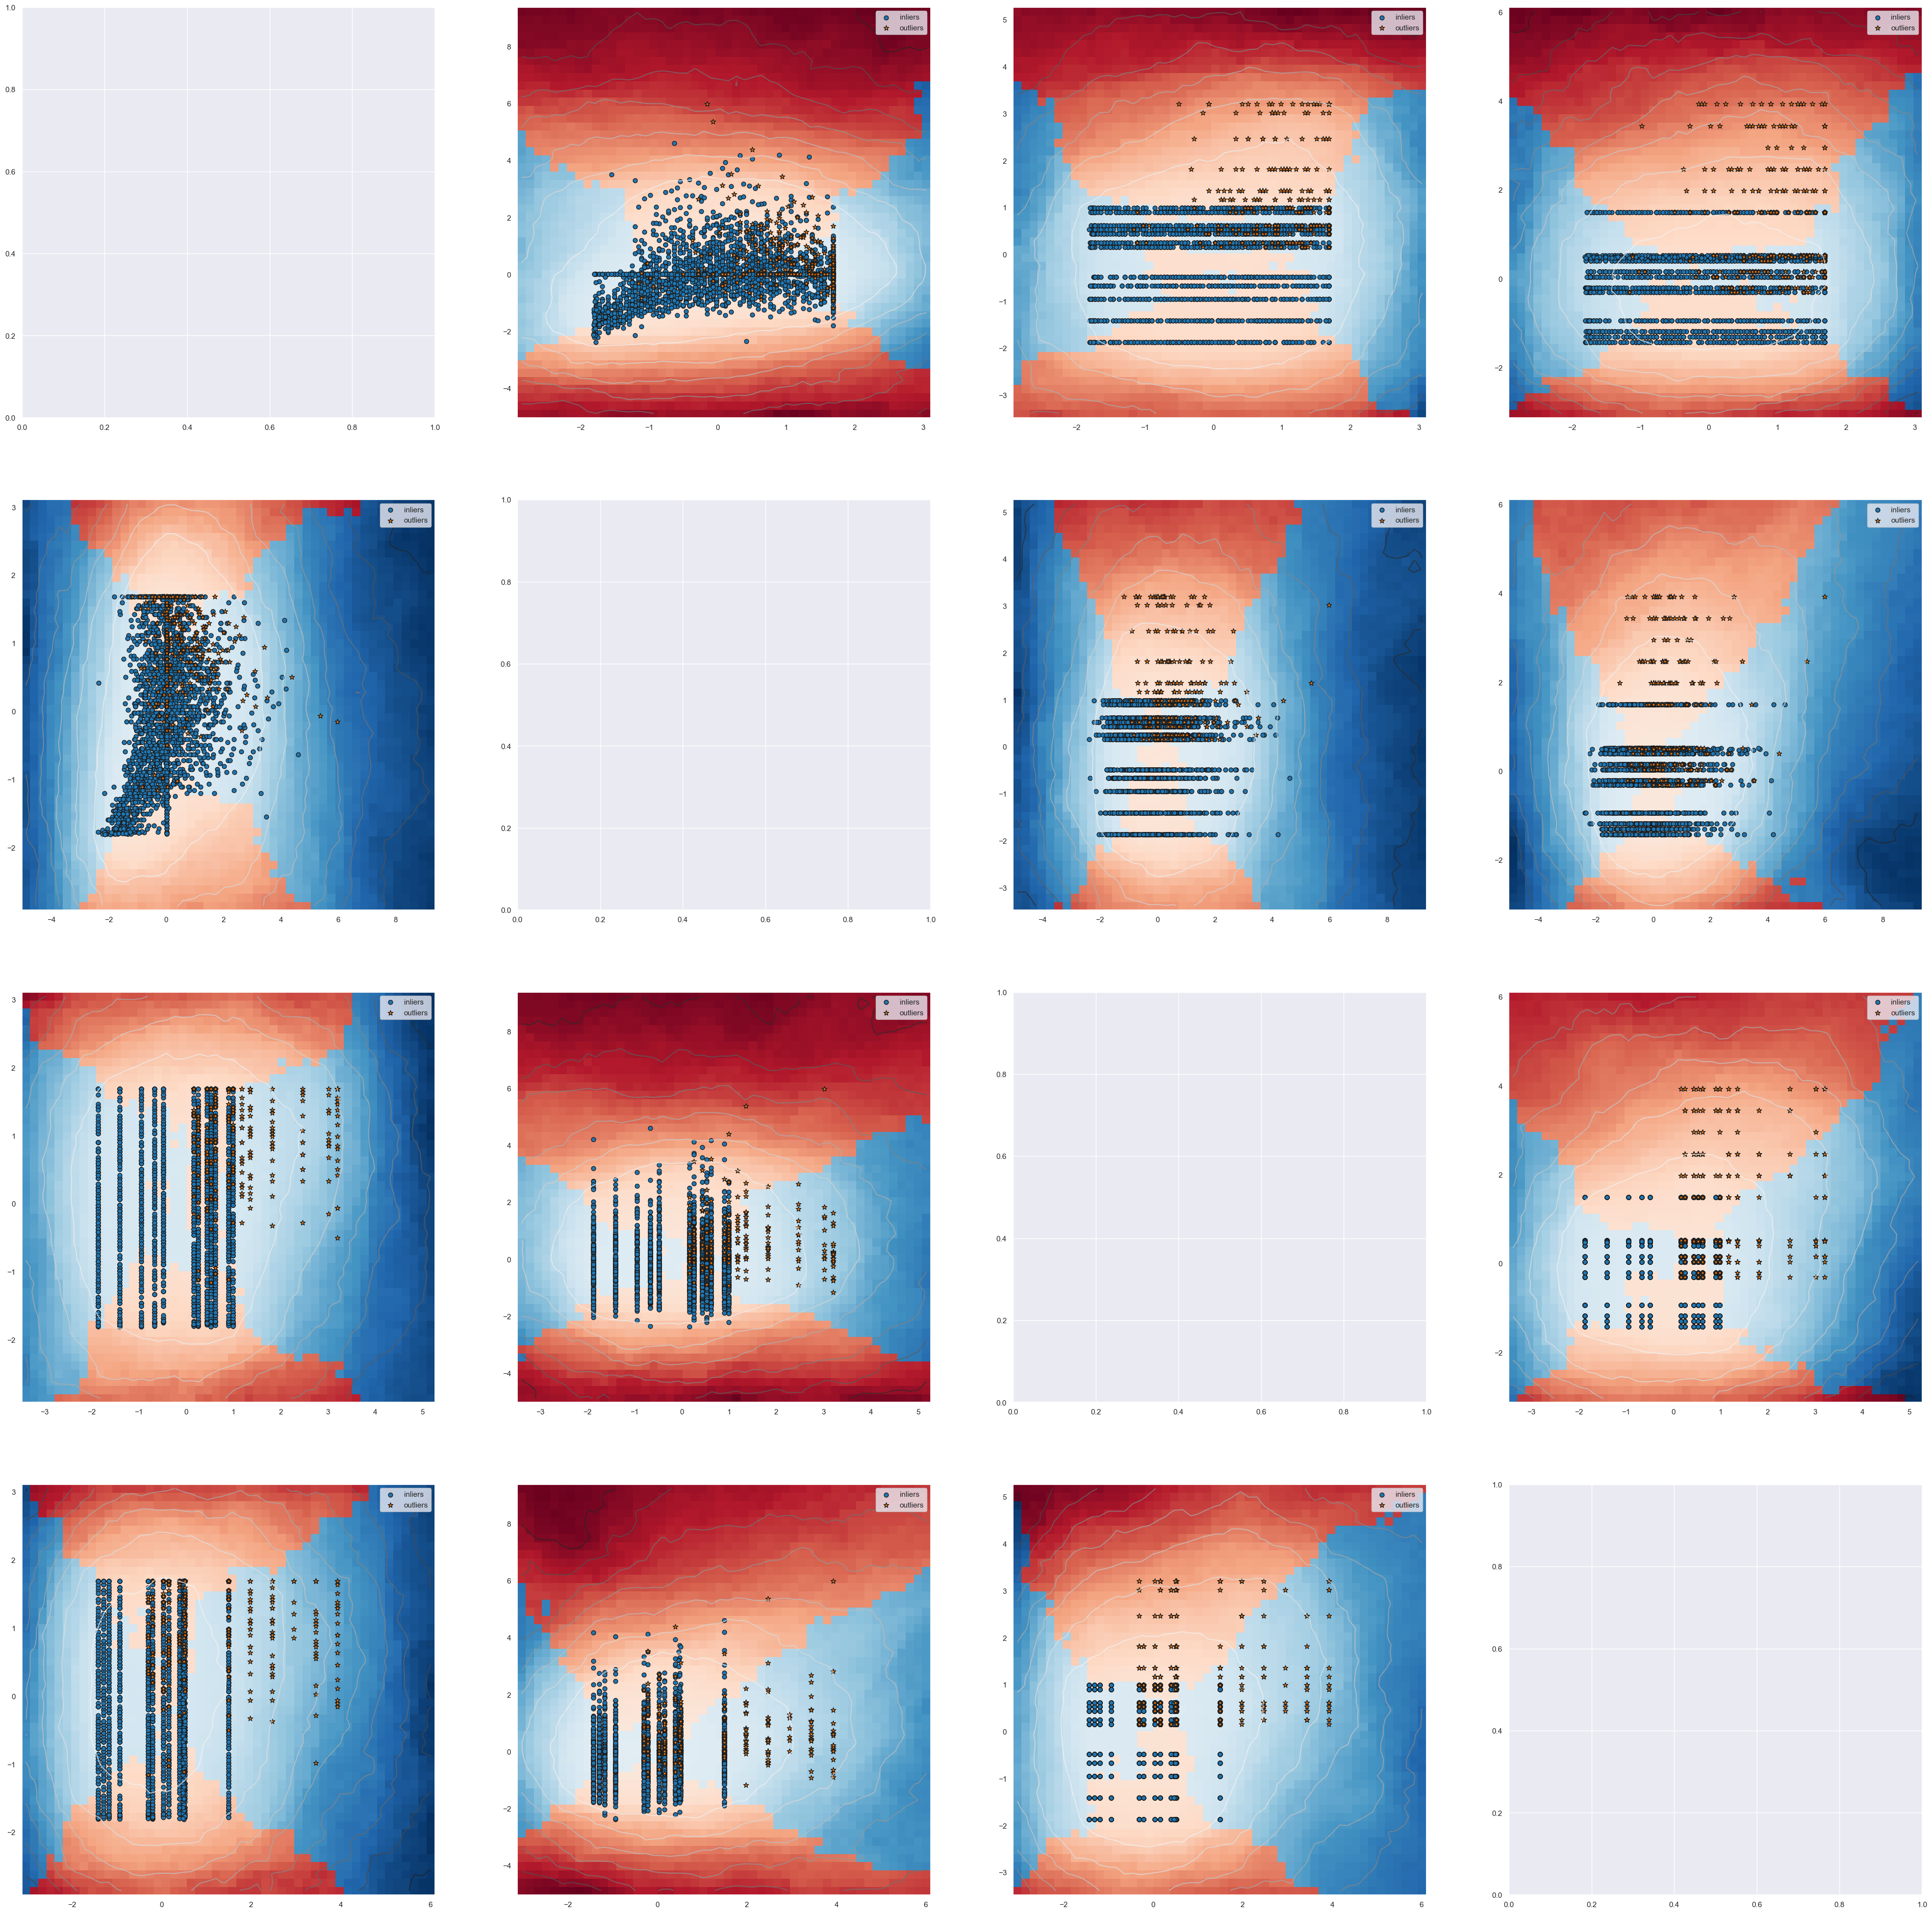}
      \caption{Complete Local Scoremap for the {\ttfamily Diabetes} dataset}
      \label{fig:Local-diabetes-complete}
\end{figure}

\section{}
\subsection{Synthetic Experiments} \label{sec:synt-appendix-experiments}

\subsection*{{\ttfamily Yaxis}}\label{sec:Yaxis}

\ale{Prior to the analysis of the experiment results on the {\ttfamily Yaxis} dataset it is worth noticing how this dataset was produced with the same process used to obtain the {\ttfamily Xaxis} dataset with the only difference that anomalies were distributed along Feature 1 instead of Feature 0. As a consequence the outocomes of the experiments are expected to be very similar, if not coincident, with the ones obtained on {\ttfamily Xaxis} and described in \ref{sec:Xaxis-exp} except for the Importance plots, that will be illustrated in \ref{sec:Yaxis-imp-plots}, where the most relevant feature is expected to be Feature 1, instead of Feature 0. }

\subsubsection{Performance}
 
\ale{Similarly to what was observed for the {\ttfamily Xaxis} dataset in Figure \ref{fig:Yaxis_contamination_full} it is possible to notice how EIF and \EIFplus obtain a perfect Average Precision score of 1 for almost all the contamination values considered and their performances are corresponding as depicted in Figure \ref{fig:Yaxis_contaminationEIFvsEIF+}. Additionally the IF model struggles to detect anomalies in a dataset were the drawbacks of the Isolation Forest model are exposed and the deep learning based approaches considered (i.e. DIF and Autoencoder) are able to achieve similar performances to EIF and \EIFplus only for minimal values of the contamination level. }

\begin{figure}[!ht] 
    \centering % <-- added
    \begin{subfigure}[t]{0.49\textwidth}
      \includegraphics[width=\linewidth]{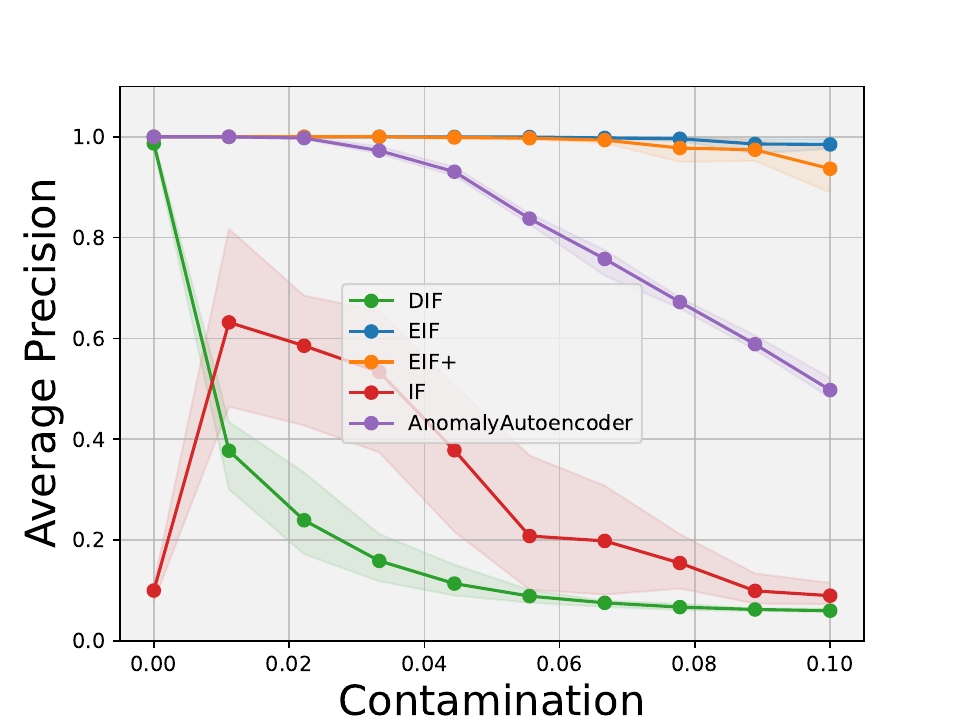}
      \caption{Models evaluation, varying the contamination levels}
      \label{fig:Yaxis_contamination_full}
    \end{subfigure}\hfil % <-- added
    \begin{subfigure}[t]{0.44\textwidth}
      \includegraphics[width=\linewidth]{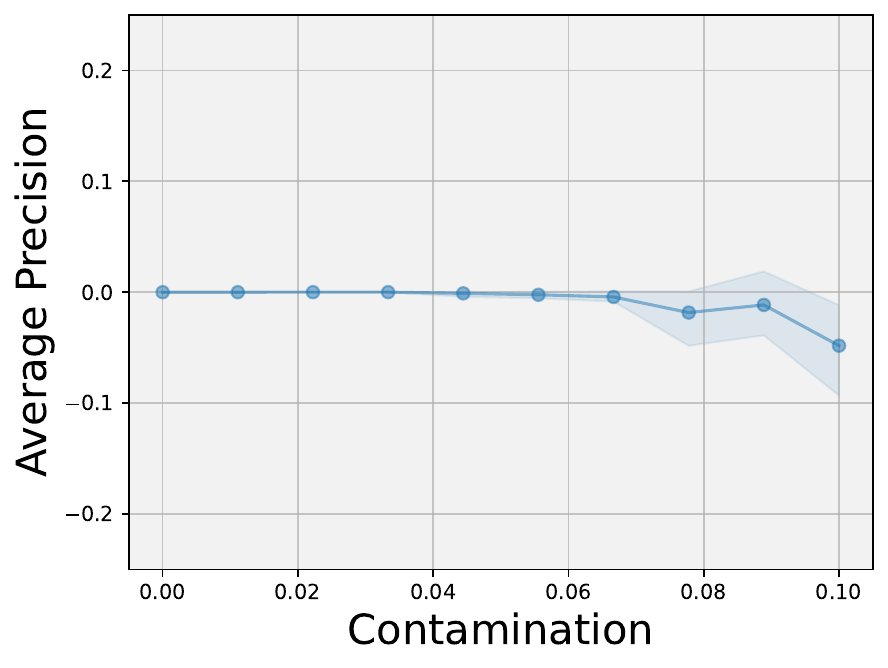}
      \caption{Difference between \EIFplus and EIF average precision}
      \label{fig:Yaxis_contaminationEIFvsEIF+}
    \end{subfigure}\hfil % <-- added
\caption{Figure \ref{fig:Yaxis_contamination_full} illustrates the average precision as the contamination level in the training set increases. Figure \ref{fig:Yaxis_contaminationEIFvsEIF+} compares the performance graphs of EIF and \EIFplus, using the difference of their scores in various contamination levels.}
\label{fig:Yaxis_contamination}
\end{figure}

\ale{A Performance Report of the various AD models explored in this study is reported in Table \ref{tab:Yaxis_perf}  highlighting the difference between Scenario I and Scenario II. The results are very close to the ones presented in \ref{sec:Xaxis-exp} with EIF and \EIFplus being clearly the optimal models both in terms of evaluation metrics and time efficiency. }
\begin{table}[htbp]
\begin{minipage}[t]{0.47\textwidth}
\strut\vspace*{-\baselineskip}\newline
\resizebox{\textwidth}{!}{
\begin{tabular}{|c||ccc|ccc||cc|}
\toprule
\hline
& \multicolumn{3}{c|}{Scenario I} & \multicolumn{3}{c||}{Scenario II} & \multicolumn{2}{c|}{Time} \\
\hline
AD Model& Avg & Prec & ROC & Avg & Prec & ROC & fit & pred \\
 & Prec &  & AUC & Prec &  & AUC &  &  \\
\hline
IF          & 0.1& 0.07& 0.48& 0.12& 0.1&0.5& 0.06& \textbf{0.006}\\
EIF         & \textbf{0.97} & \textbf{0.85}& \textbf{0.91}& \textbf{0.99} & \textbf{1.0} & \textbf{1.0} & \textbf{0.05}& 0.07\\
\EIFplus        & \textbf{0.94}& \textbf{0.9}& \textbf{0.94}& \textbf{0.99} & \textbf{0.99}& \textbf{0.99}& \textbf{0.05}& 0.07\\
DIF         & 0.05& 0.01&0.45& 0.99& 0.97&0.98& 1.65& 1.33\\
AE         & 0.54& 0.49&0.71& 1.0 & 1.0&1.0& 4.07& 0.07 \\
\hline
\end{tabular}
}
\vspace{0.41cm}
\caption{Performances of 5 different Anomaly Detection models over {\ttfamily Yaxis} are compared using classical Classification metrics. Moreover the last two columns contain the average time for a fit and predict operation. The highest metric values and the lowest execution times are highlighted in bold}\label{tab:Yaxis_perf}
\end{minipage}
\hfill
\begin{minipage}[t]{0.47\textwidth}
\strut\vspace*{-\baselineskip}\newline
\resizebox{\textwidth}{!}{
\begin{tabular}{|c||c|c|c|c||c|}
\toprule
\hline
&\multicolumn{2}{c|}{Evaluation with EIF}&\multicolumn{2}{c||}{Evaluation with \EIFplus}&\\
\hline
& Scenario I & Scenario II & Scenario I & Scenario II & Time\\

 Algorithm & $AUC_{FS}$  & $AUC_{FS}$ & $AUC_{FS}$  & $AUC_{FS}$ &  \\
\hline
DIFFI         & 4.726& \textbf{4.740}& \textbf{4.567}& 4.743& 0.36\\
IF\_\approach        & -4.714& 0.952& -4.536& 0.955& \textbf{0.16}\\
EIF\_\approach        & 4.73& 4.729& 4.484& 4.744& \textbf{0.16}\\
\EIFplus\_\approach       & 4.733& 4.73& 4.508& 4.745& \textbf{0.16}\\
IF\_RF        & -2.843& -0.95& -2.669& -0.946& 0.67\\
EIF\_RF       & \textbf{4.734}& 4.733& 4.537& 4.74& 0.67\\
EIF+\_RF      & 4.705& 4.729& 4.506& \textbf{4.746}& 0.67\\
\hline
\end{tabular}
}
\caption{Quantitative evaluation of the effectiveness of 6 different interpretation algorithms on {\ttfamily Yaxis} through the $AUC_{FS}$ metric, introduced in \ref{sec:interpr_evaluat}. In the last column the average time taken by the different models to produce the importance scores is reported. The highest $AUC_{FS}$ and lowest Importance time values are highlighted in bold.}\label{tab:fs-tab-Yaxis}
\end{minipage}
\end{table}

\subsubsection{Importance Plots} \label{sec:Yaxis-imp-plots}

\ale{An evaluation of the proposed interpretation model \approach+ is presented in Figure \ref{fig:interpretation-Yaxis}. As expected the results are symmetrical to the ones obtained in {\ttfamily Xaxis} with Feature 1 being the most relevant feature in both Scenario I and II and the dominance of this variable can also be observed in the Local Scoremaps depicted in Figures \ref{fig:Local-Yaxis-EXIFFI+-1} and \ref{fig:Local-Yaxis-EXIFFI+-2}. }

\begin{figure}[!ht] 
    \centering % <-- added
    \begin{subfigure}[t]{0.33\textwidth}
    \centering
      \includegraphics[width=\linewidth]{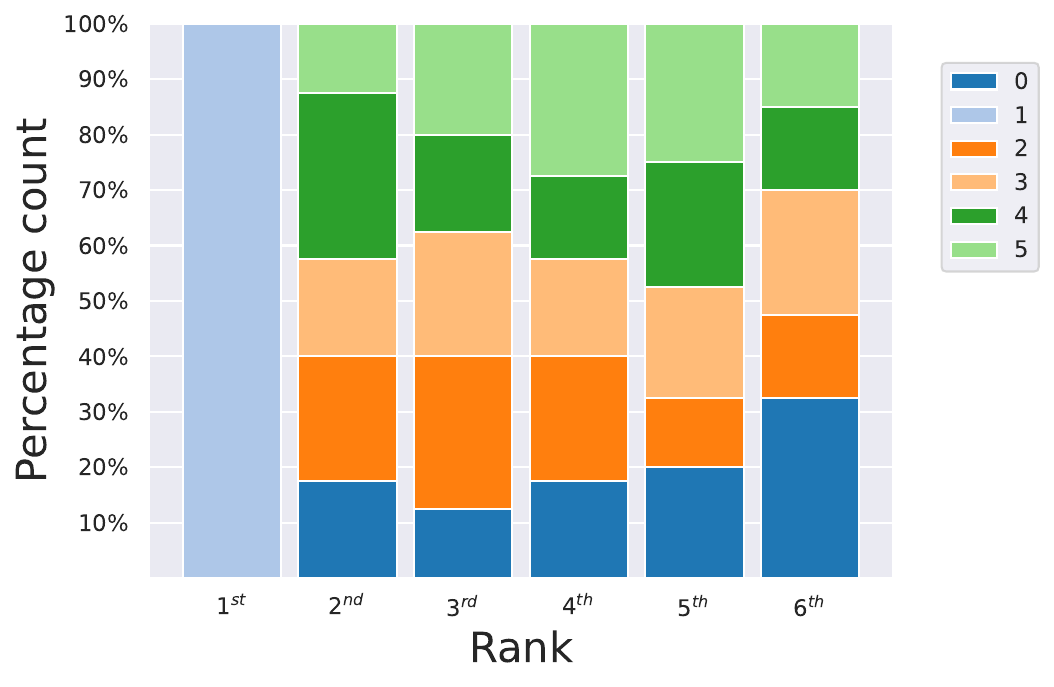}
      \caption{Bar Plot {\ttfamily Yaxis} Scenario I}
      \label{fig:Bar-plot-Yaxis-EXIFFI+-1}
    \end{subfigure}\hfil % <-- added
    \begin{subfigure}[t]{0.27\textwidth}
    \centering
      \includegraphics[width=\linewidth]{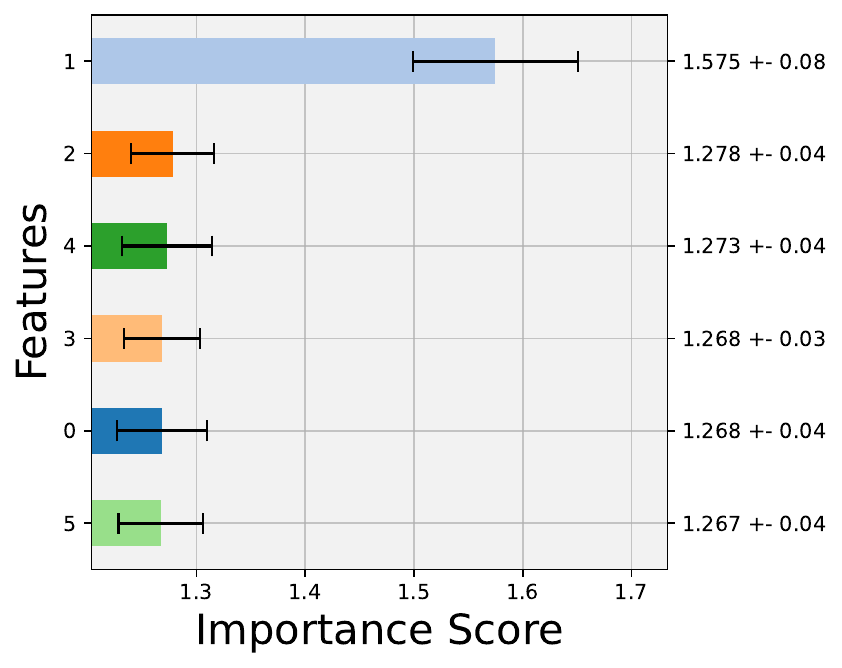}
      \caption{Score Plot {\ttfamily Yaxis} Scenario I}
      \label{fig:Score-plot-Yaxis-EXIFFI+-1}
    \end{subfigure}\hfil % <-- added
    \begin{subfigure}[t]{0.28\textwidth}
    \centering
      \includegraphics[width=\linewidth]{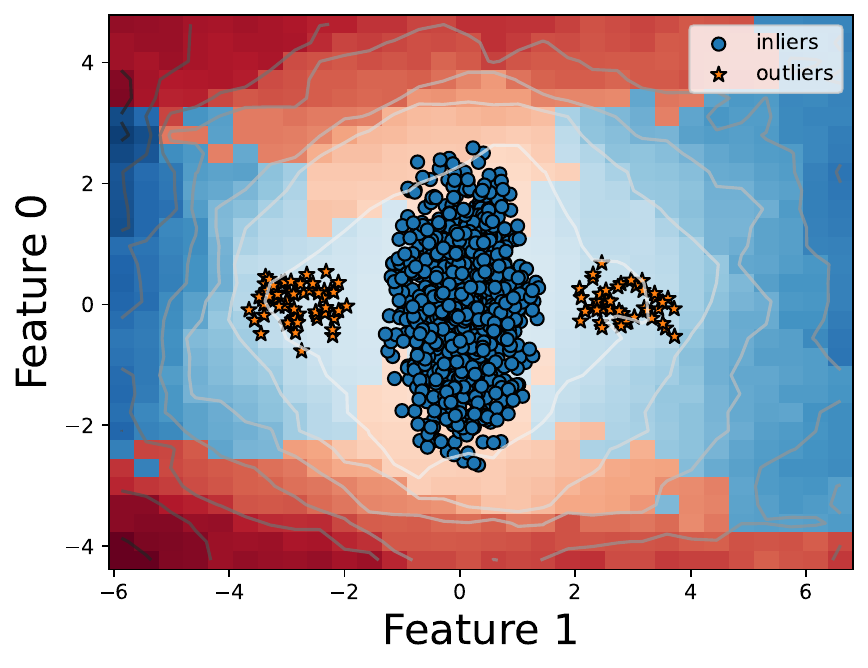}
      \caption{Scoremap {\ttfamily Yaxis} Scenario I}
      \label{fig:Local-Yaxis-EXIFFI+-1}
    \end{subfigure}\hfil % <-- added
    \begin{subfigure}[t]{0.33\textwidth}
    \centering
      \includegraphics[width=\linewidth]{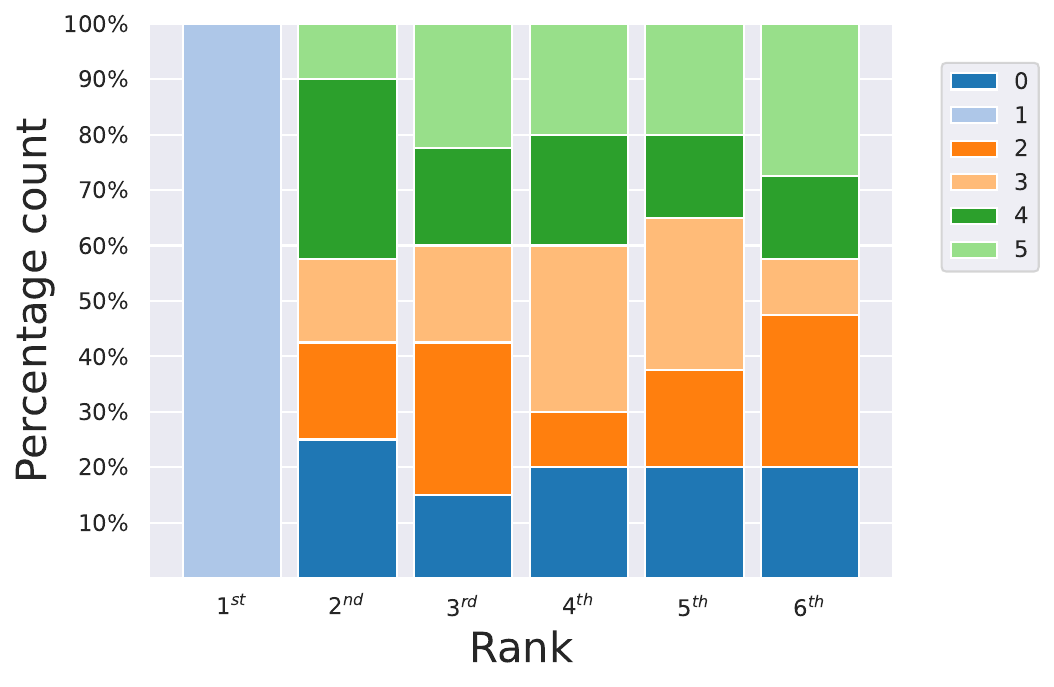}
      \caption{Bar Plot {\ttfamily Yaxis} Scenario II}
      \label{fig:Bar-plot-Yaxis-EXIFFI+-2}
    \end{subfigure}\hfil % <-- added
    \begin{subfigure}[t]{0.27\textwidth}
    \centering
      \includegraphics[width=\linewidth]{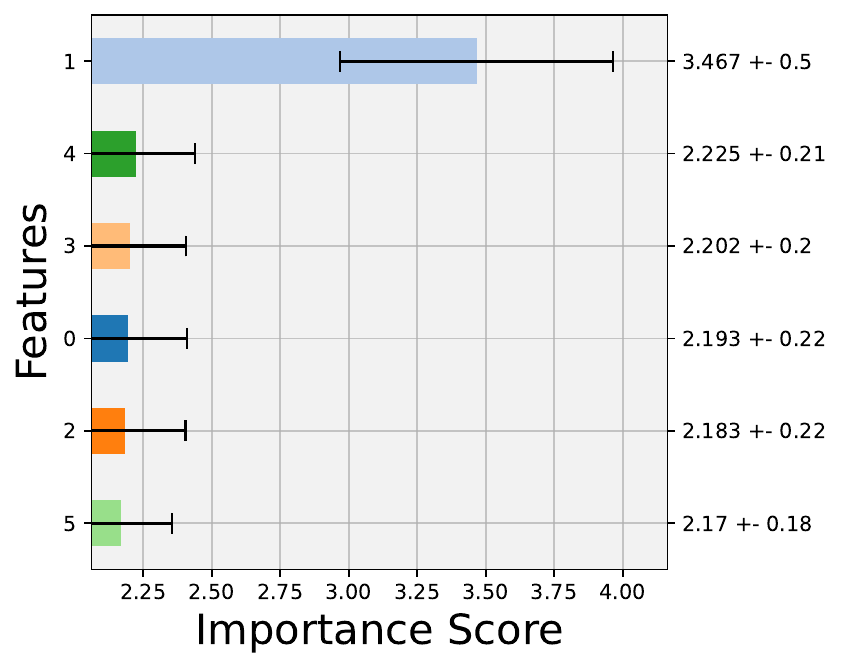}
      \caption{Score Plot {\ttfamily Yaxis} Scenario II}
      \label{fig:Score-plot-Yaxis-EXIFFI+-2}
    \end{subfigure}\hfil % <-- added
    \begin{subfigure}[t]{0.28\textwidth}
    \centering
      \includegraphics[width=\linewidth]{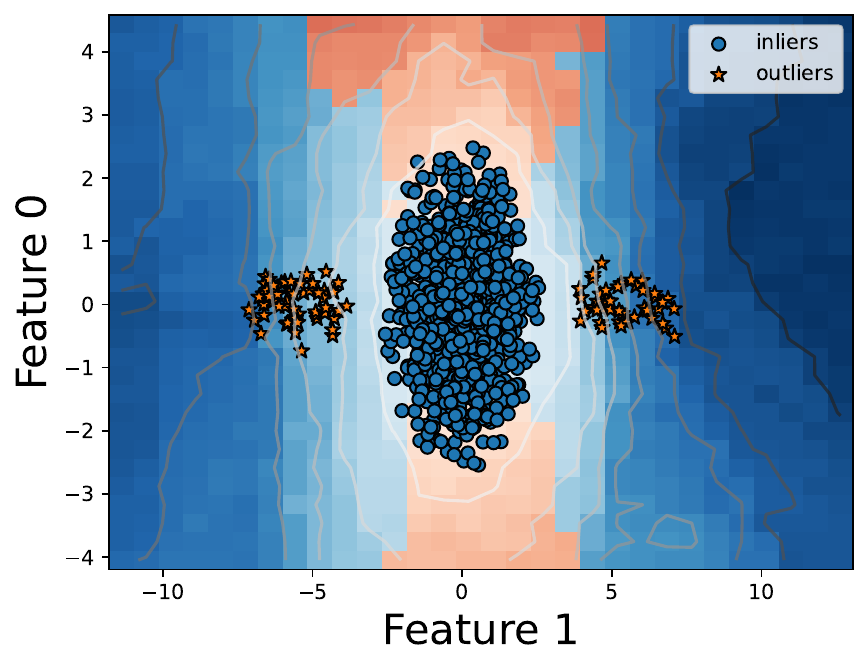}
      \caption{Scoremap {\ttfamily Yaxis} Scenario II}
      \label{fig:Local-Yaxis-EXIFFI+-2}
    \end{subfigure}\hfil % <-- added
\caption{Bar Plot, Score Plot and Scoremap of the dataset {\ttfamily Yaxis} in the two different Scenarios, using the ExIFFI algorithm applied to the \EIFplus model.}\label{fig:interpretation-Yaxis}
\end{figure}

\subsubsection{Feature Selection}

\ale{Also in the Feature Selection Plots, portrayed in Figure \ref{fig:fs-interpretation-Yaxis},  a clear resemblance with the plots displayed in Figure \ref{fig:fs-interpretation-Xaxis} can be observed, except for the peculiar behavior associated to the interpretation of the IF model predictions, shown in Figures \ref{fig:Feat-Sel_Yaxis_valEIF+_DIFFI_2} and \ref{fig:Feat-Sel_Yaxis_valEIF+_IF_RandomForest_2}. As it happens in the {\ttfamily Xaxis} dataset the anomaly score artifacts of IF are exposed in this dataset leading to poor performances of the IF model. However differently from the outcomes described in \ref{sec:feat-sel-Xaxis} the features ranking produced by IF\_\approach and IF\_RandomForest , place Feature 1 (i.e. the most relevant feature for {\ttfamily Yaxis}) in the middle of the ranking, in particular in position 4 and 3 respectively leading to a peculiar parallelogram shape in the Feature Selection plots.}

\begin{comment}
Also for {\ttfamily Yaxis} the newly introduced ad-hoc interpretability methods \approach and \approach+ produce better looking plots than the ones produced by the IF model (\ref{fig:Feat-Sel_Yaxis_valEIF+_DIFFI_2}, \ref{fig:Feat-Sel_Yaxis_valEIF+_IF_RandomForest_2}), in particular, by post-hoc interpretability methods based on the Random Forest surrogate model.
\end{comment} 

\begin{figure}[!ht] 
    \centering
    \hspace{0.05\textwidth}\textbf{IF} \hspace{0.29\textwidth} \textbf{EIF} \hspace{0.29\textwidth} \textbf{EIF+}
    % First row with vertical caption on the left
    \begin{minipage}{\textwidth}
    \rotatebox{90}{\parbox{15mm}{\centering \textbf{Ad-Hoc}}} % Adjust the parbox width as necessary for your caption text
    \begin{minipage}{0.95\textwidth}
        \begin{subfigure}[t]{0.30\textwidth}
            \centering
      \includegraphics[trim={0 0 3.5cm 0}, clip, width=\linewidth]{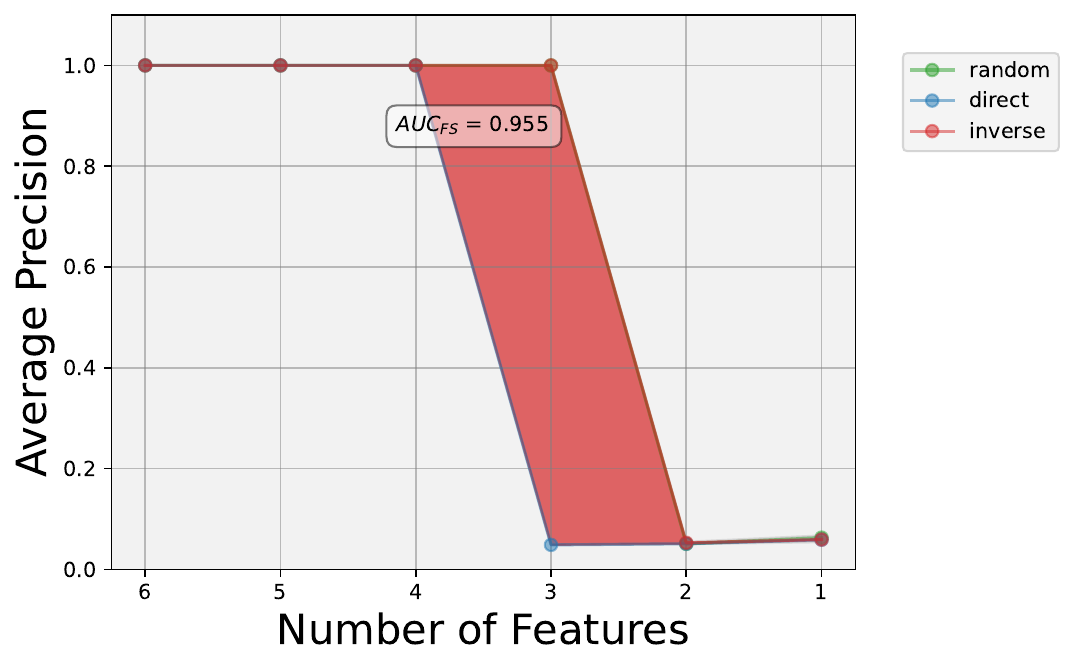}
      \caption{\approach applied to IF}
      \label{fig:Feat-Sel_Yaxis_valEIF+_DIFFI_2}
    \end{subfigure}\hfil % <-- added
    \begin{subfigure}[t]{0.30\textwidth}
    \centering
      \includegraphics[trim={0 0 3.5cm 0}, clip,width=\linewidth]{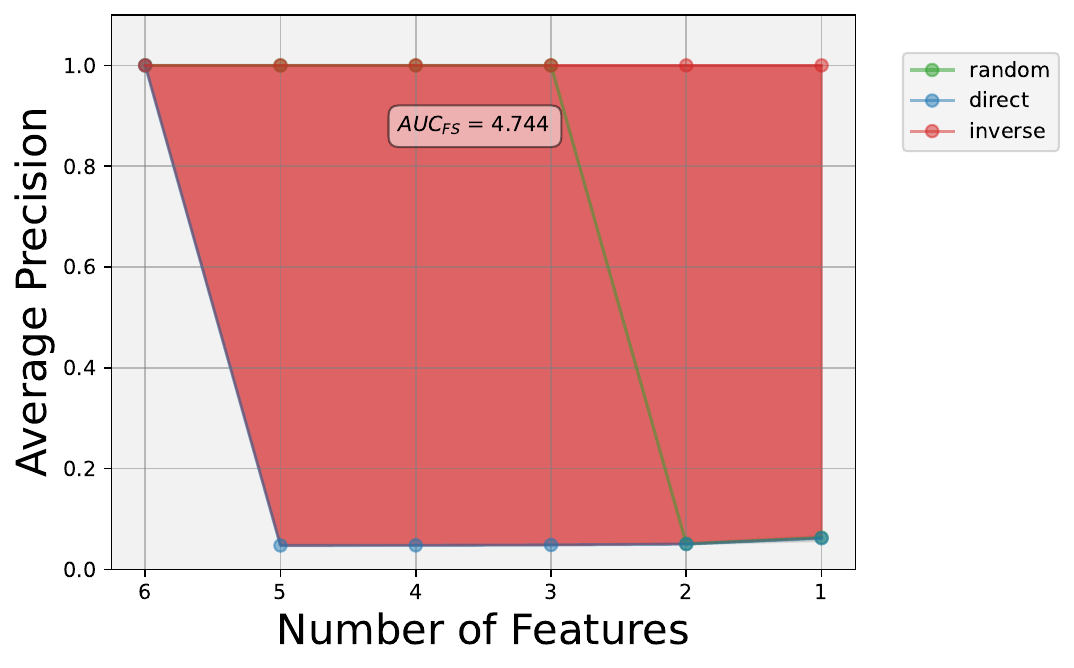}
      \caption{\approach applied to EIF}
      \label{fig:Feat-Sel_Yaxis_valEIF+_EXIFFI_2}
    \end{subfigure}\hfil % <-- added
    \begin{subfigure}[t]{0.30\textwidth}
    \centering
      \includegraphics[trim={0 0 3.5cm 0}, clip,width=\linewidth]{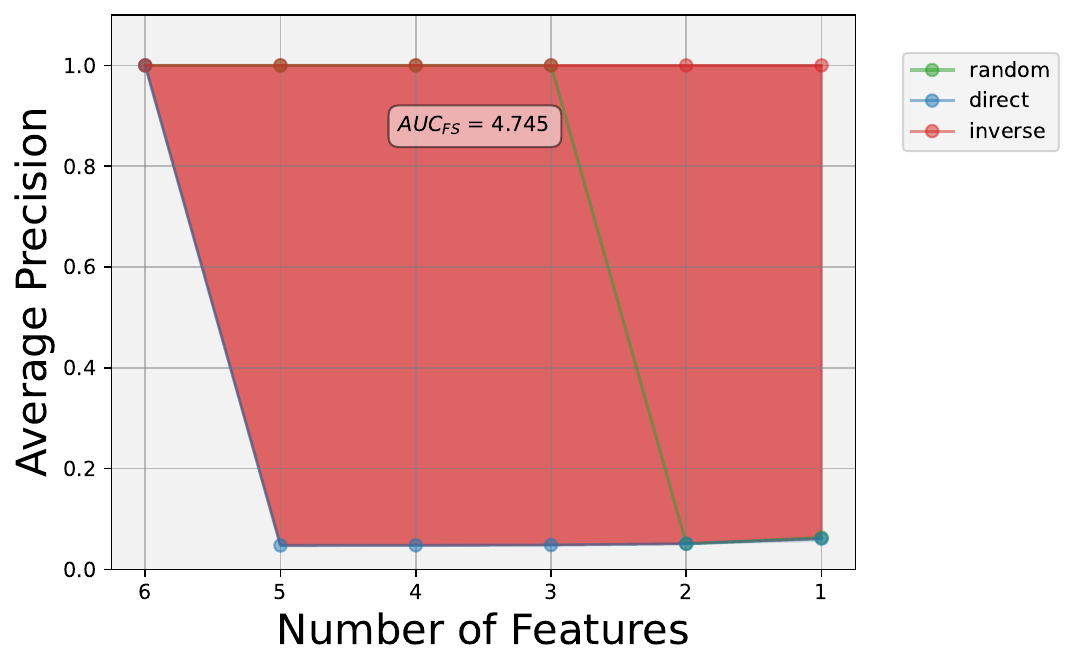}
      \caption{\approach applied to \EIFplus}
      \label{fig:Feat-Sel_Yaxis_valEIF+_EXIFFI+_2}
      \end{subfigure}
    \end{minipage}
\end{minipage}

% Second row with vertical caption on the left
\begin{minipage}{\textwidth}
    \rotatebox{90}{\parbox{15mm}{\centering \textbf{Post-Hoc}}} % Adjust as necessary
    \begin{minipage}{0.95\textwidth}
        \begin{subfigure}[t]{0.30\textwidth}
            \centering
              \includegraphics[trim={0 0 3.5cm 0}, clip,width=\linewidth]{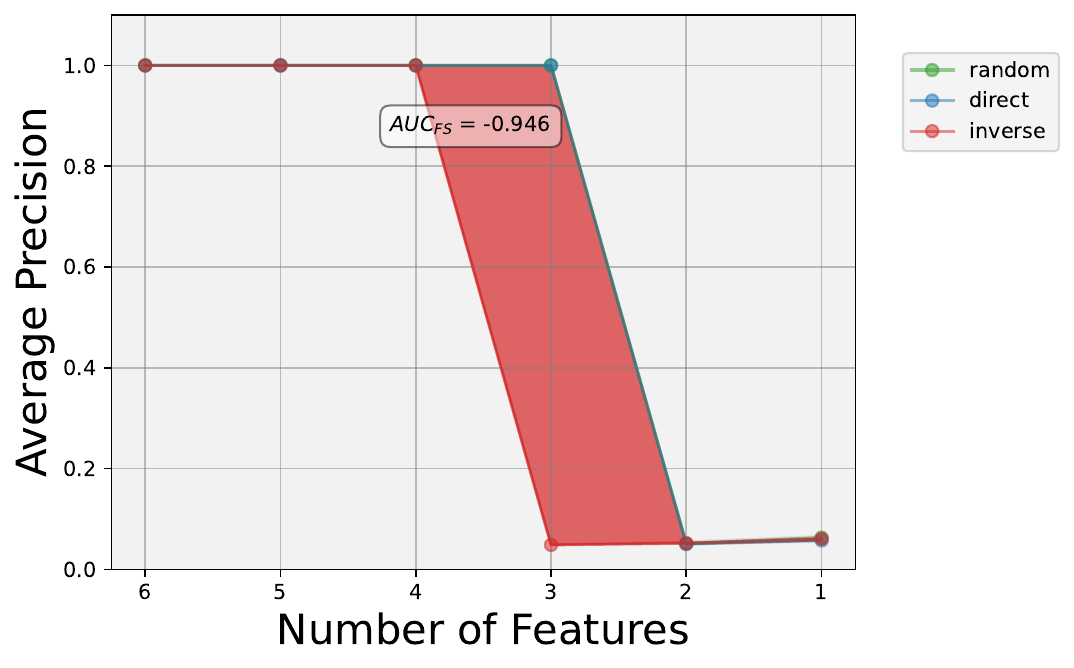}
              \caption{RandomForest fitted to IF}
              \label{fig:Feat-Sel_Yaxis_valEIF+_IF_RandomForest_2}
            \end{subfigure}\hfil % <-- added
            \begin{subfigure}[t]{0.30\textwidth}
            \centering
              \includegraphics[trim={0 0 3.5cm 0}, clip,width=\linewidth]{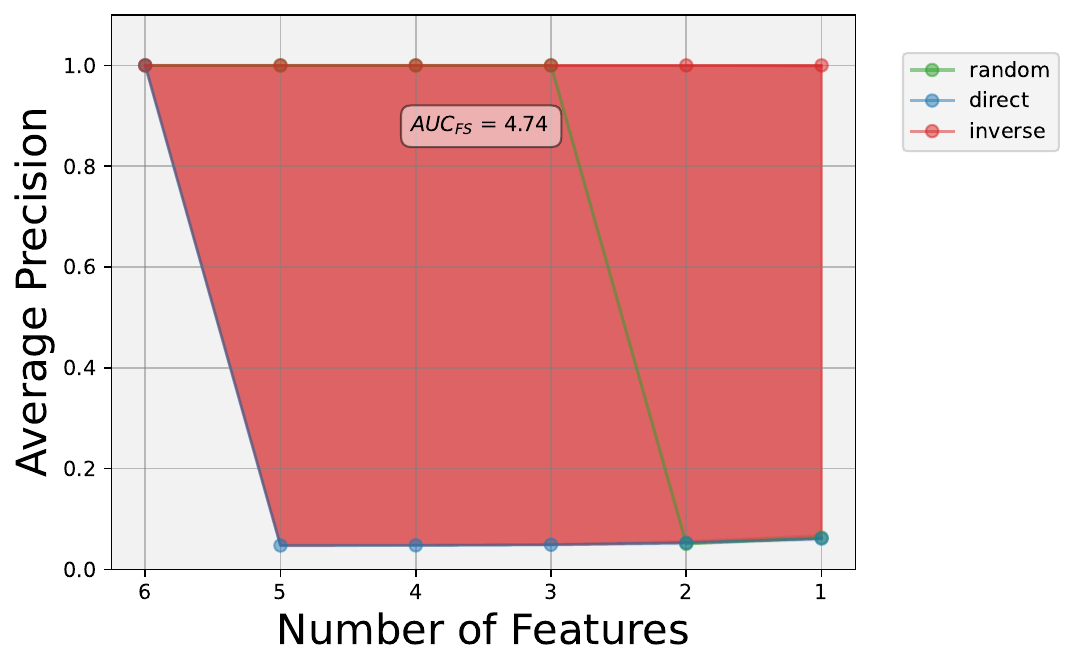}
              \caption{RandomForest fitted to EIF}
              \label{fig:Feat-Sel_Yaxis_valEIF+_EIF_RandomForest_2}
            \end{subfigure}\hfil % <-- added
            \begin{subfigure}[t]{0.30\textwidth}
            \centering
              \includegraphics[trim={0 0 3.5cm 0}, clip,width=\linewidth]{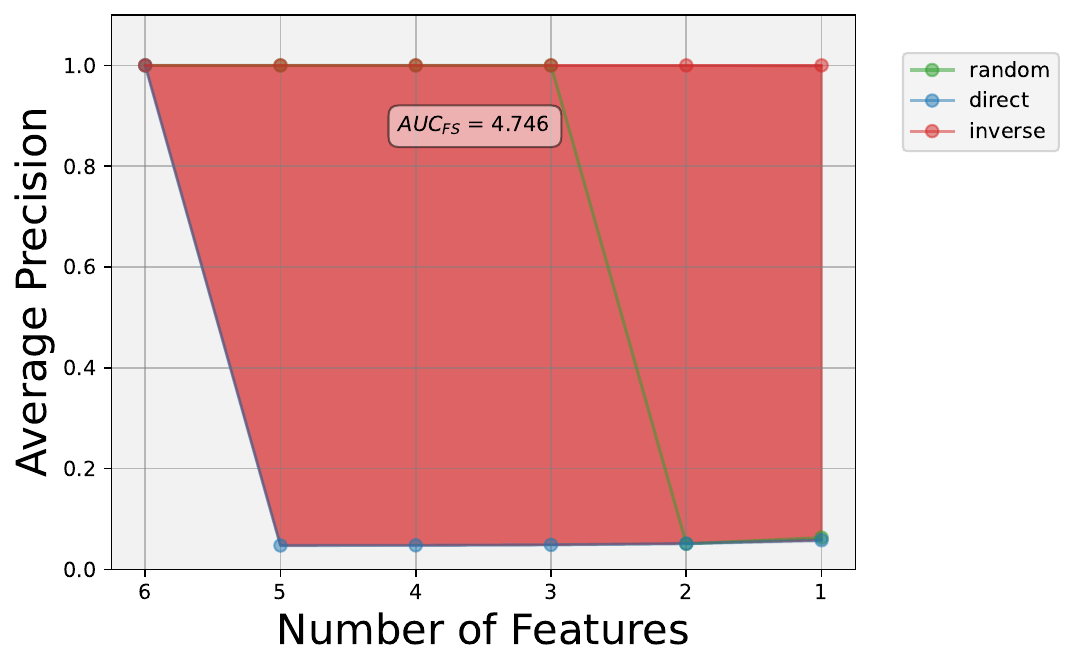}
              \caption{RandomForest fitted to \EIFplus}
              \label{fig:Feat-Sel_Yaxis_valEIF+_EIF+_RandomForest_2}
                    \end{subfigure}
            \end{minipage}
        \end{minipage}
      \caption{Feature Selection of the different Ad-Hoc and Post-Hoc methods applied to the 3 Isolation Forest models: IF, EIF and \EIFplus. The blue line is the values of average precision, calculated with the \EIFplus model in the Scenario II, dropping the most important feature at each step, the red line is the values of average precision dropping the least important feature at each step and the green line is the value of the feature selection dropping a random feature at each step.}\label{fig:fs-interpretation-Yaxis}
\end{figure}

\ale{The outcomes just commented after a detailed observation of the Feature Selection plots are reflected on the $AUC_{FS}$ values collected, for all the possible combinations of evaluation and interpretation methods, in Table \ref{tab:fs-tab-Yaxis}. The best values are associated to \approach and \approach+ models which are also the best performing ones in terms of computational efficiency. }

\subsection*{{\ttfamily Bisec}}

\subsubsection{Performance}

\ale{Figure \ref{fig:Bisec_contamination_full} reports the Average Precision of various AD models in relation to different percentages of outliers inserted in the training set and taking part to the fitting process. Similarly to what can be observed in the {\ttfamily Bisec3D} dataset, described in \ref{sec:Bisec3D-exp}, the entirety of the models shows comparable results except for DIF where the Average Precision suffers a significant drop as outliers are progressively included as training samples. The EIF and \EIFplus models emerge as the ones with the highest metric values and their performances are comparable as shown in Figure \ref{fig:Bisec_contaminationEIFvsEIF+}.}

\begin{figure}[!ht] 
    \centering % <-- added
    \begin{subfigure}[t]{0.49\textwidth}
      \includegraphics[width=\linewidth]{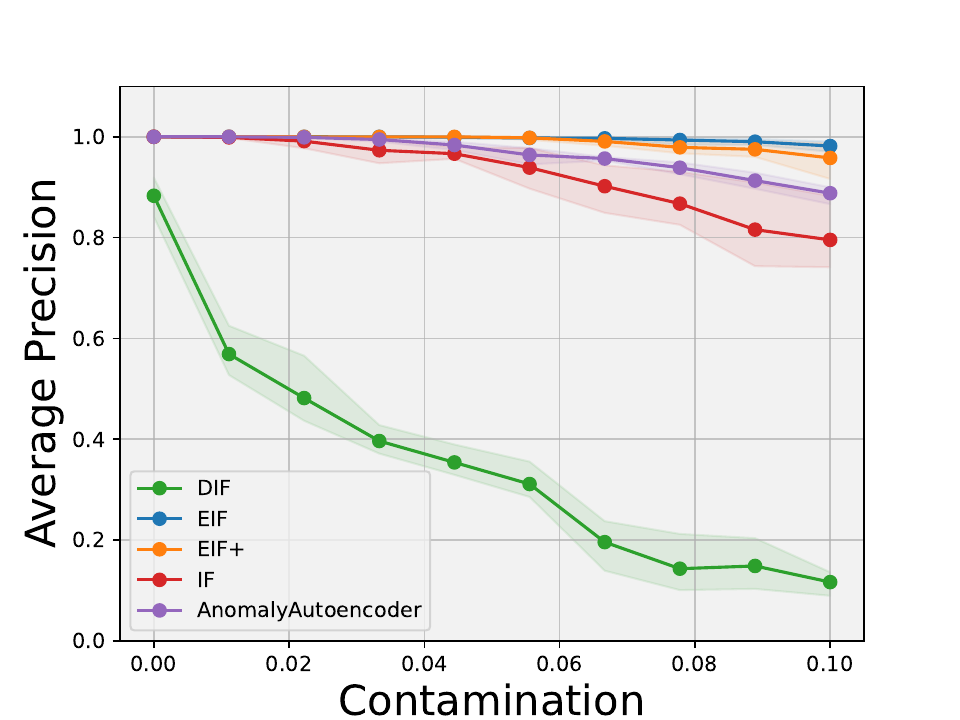}
      \caption{Models evaluation, varying the contamination levels}
      \label{fig:Bisec_contamination_full}
    \end{subfigure}\hfil % <-- added
    \begin{subfigure}[t]{0.44\textwidth}
      \includegraphics[width=\linewidth]{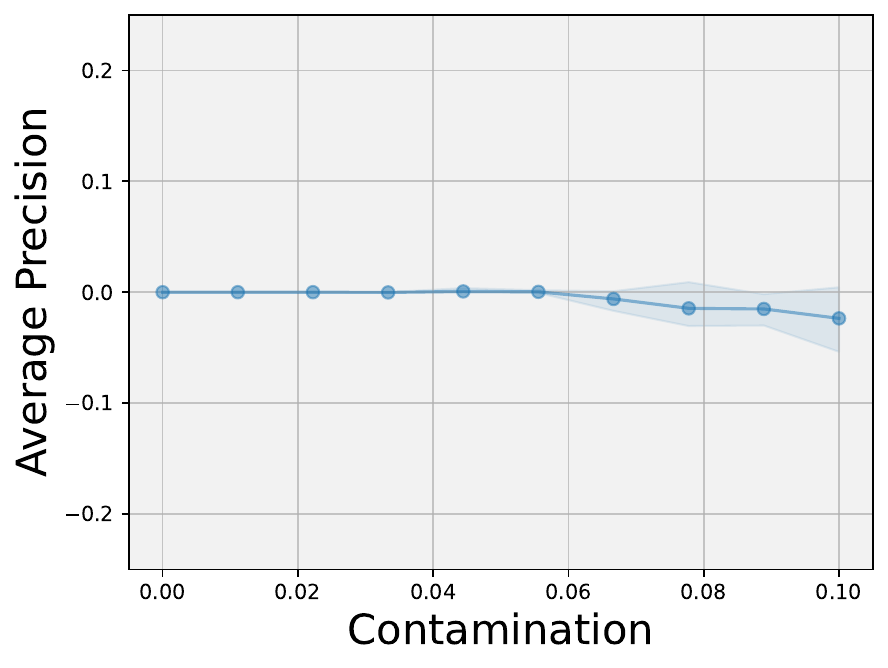}
      \caption{Difference between \EIFplus and EIF average precision}
      \label{fig:Bisec_contaminationEIFvsEIF+}
    \end{subfigure}\hfil % <-- added
\caption{Figure \ref{fig:Bisec_contamination_full} illustrates the average precision as the contamination level in the training set increases. Figure \ref{fig:Bisec_contaminationEIFvsEIF+} compares the performance graphs of EIF and \EIFplus, using the difference of their scores in various contamination levels.}
\label{fig:Bisec_contamination}
\end{figure}

\ale{Table \ref{tab:Bisec_perf}  offers a more detailed overview of the performances of the Anomaly Detection models considered focusing on the comparison between Scenario I (i.e. all the outliers inserted in the training set) and Scenario II (i.e. training set composed of only inliers). After a careful analysis of the values reported on the table it is possible to conclude about the superiority of the EIF and \EIFplus models, that achieve excellent results both in terms of precision in detecting anomalies and time efficiency. }

\begin{table}[htbp]
\begin{minipage}[t]{0.46\textwidth}
\strut\vspace*{-\baselineskip}\newline
\resizebox{\textwidth}{!}{
\begin{tabular}{|c||ccc|ccc||cc|}
\toprule
\hline
&\multicolumn{3}{c|}{Scenario I}&\multicolumn{3}{c||}{Scenario II}&\multicolumn{2}{c|}{Time}\\
\hline
AD Model& Avg & Prec & ROC & Avg & Prec & ROC & fit & pred \\
 & Prec &  & AUC & Prec &  & AUC &  &  \\
\hline
IF          & 0.75& 0.74& 0.85& 0.99& 0.95& 0.97& \textbf{0.05}& \textbf{0.006}\\
EIF         & 0.97& 0.91& 0.95& 0.99& 1.0& 1.0& \textbf{0.05}& 0.06\\
EIF+        & 0.94& 0.83& 0.9& \textbf{1.0}& \textbf{1.0}& \textbf{1.0}& \textbf{0.05}& 0.07\\
DIF         & 0.16& 0.2& 0.56& 0.85& 0.78& 0.87& 1.54& 1.21\\
AE & 0.89& 0.82& 0.9& 1.0& 1.0& 1.0& 3.77& 0.06\\
\hline
\end{tabular}}
\vspace{0.41cm}
\caption{Performances of 5 different Anomaly Detection models over {\ttfamily Bisec} are compared using classical Classification metrics. Moreover the last two columns contain the average time for a fit and predict operation. The highest metric values and the lowest execution times are highlighted in bold}\label{tab:Bisec_perf}
\end{minipage}
\hfill
\begin{minipage}[t]{0.46\textwidth}
\strut\vspace*{-\baselineskip}\newline
\resizebox{\textwidth}{!}{
\begin{tabular}{|c||c|c|c|c||c|}
\toprule
\hline
&\multicolumn{2}{c|}{Evaluation with EIF}&\multicolumn{2}{c||}{Evaluation with \EIFplus}&\\
\hline
& Scenario I & Scenario II & Scenario I & Scenario II & Time\\

 Algorithm & $AUC_{FS}$  & $AUC_{FS}$ & $AUC_{FS}$  & $AUC_{FS}$ &  \\
\hline
DIFFI                & 4.121& 2.925& \textbf{4.166}& 2.924& 0.34\\
IF\_\approach        & 4.137& \textbf{3.842}& 4.12& 3.828& \textbf{0.16}\\
EIF\_\approach       & \textbf{4.152}& 3.844& 4.042& 3.833& \textbf{0.16}\\
\EIFplus\_\approach  & 4.077& 3.827& 4.052& 3.833& \textbf{0.16}\\
IF\_RF               & 4.019& 3.828& 3.93& 3.83& 0.66\\
EIF\_RF              & 4.057& 3.834& 3.957& \textbf{3.841}& 0.66\\
EIF+\_RF             & 4.029& 3.832& 4.012& 3.832& 0.66\\
\hline
\end{tabular}}
\caption{Quantitative evaluation of the effectiveness of 6 different interpretation algorithms on {\ttfamily Bisec} through the $AUC_{FS}$ metric, introduced in \ref{sec:interpr_evaluat}. In the last column the average time taken by the different models to produce the importance scores is reported. The highest $AUC_{FS}$ and lowest Importance time values are highlighted in bold.}\label{tab:fs-tab-Bisec}
\end{minipage}
\end{table}

\subsubsection{Importance Plots}

\ale{The newly introduced \approach+ interpretation model is evaluated through the plots presented in Figure \ref{fig:interpretation-Bisec}. As expected, considering how this synthetic dataset was constructed, it is possible to select two relevant features (i.e. Feature 0 and 1) with similar importance scores that stand out with the respect to the ones of other variables contained in the dataset, as represented in Figures \ref{fig:Feat-imp-Bisec} and \ref{fig:Feat-imp-Bisec-split}. The Local Scoremaps, displayed in Figures \ref{fig:Local-Bisec} and \ref{fig:Local-Bisec-split}, provides a better visual explanation on how the anomalies and importance scores are distributed in the feature space.}

\begin{figure}[!ht] 
    \centering % <-- added
    \begin{subfigure}[t]{0.33\textwidth}
    \centering
      \includegraphics[width=\linewidth]{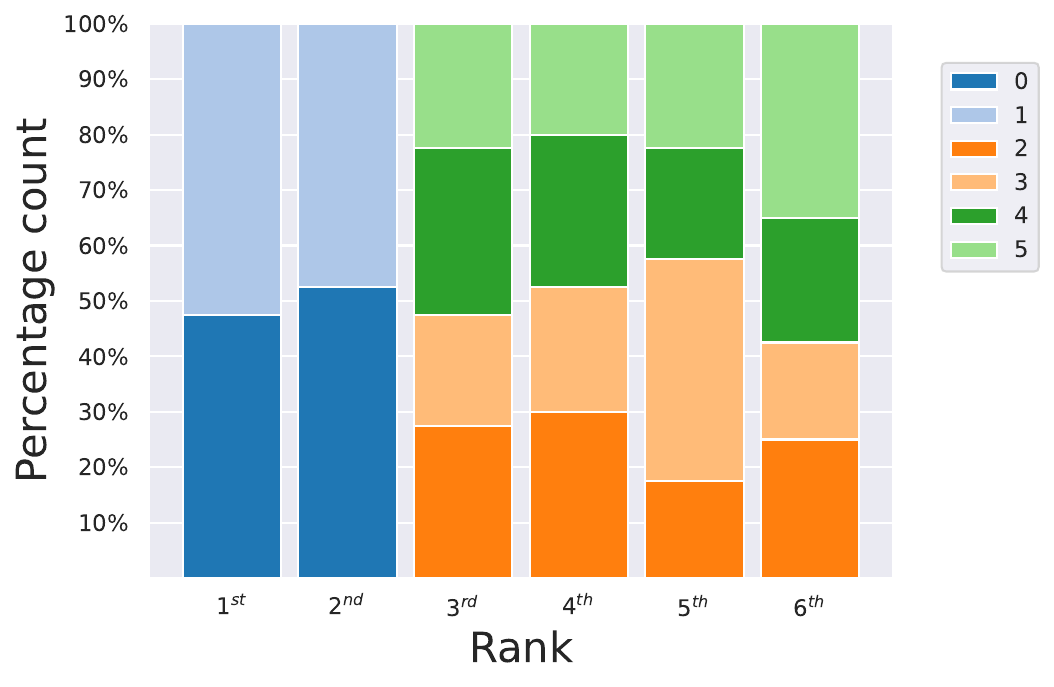}
      \caption{Bar Plot {\ttfamily Bisec} Scenario I}
      \label{fig:GFI-Bisec}
    \end{subfigure}\hfil % <-- added
    \begin{subfigure}[t]{0.27\textwidth}
    \centering
      \includegraphics[width=\linewidth]{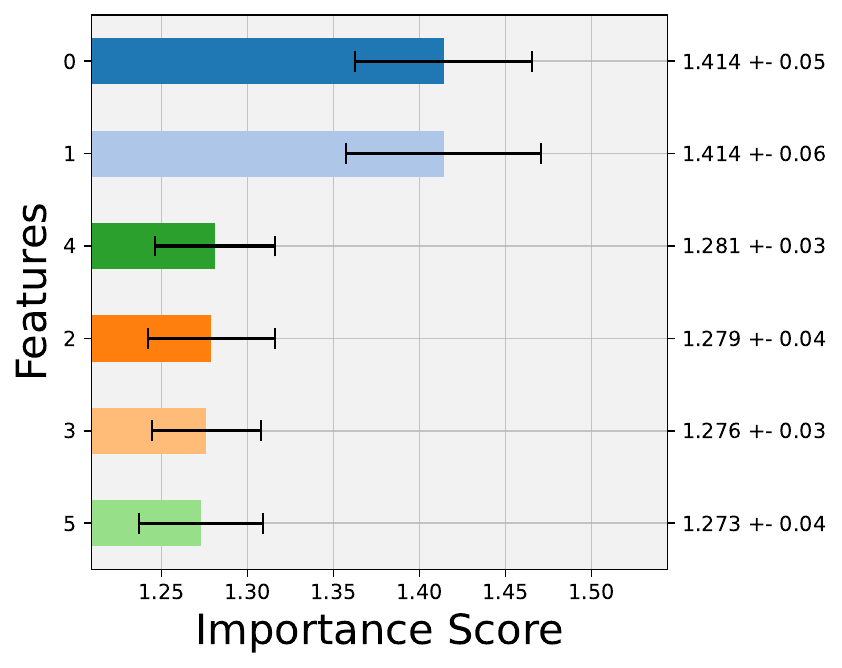}
      \caption{Score Plot {\ttfamily Bisec} Scenario I}
      \label{fig:Feat-imp-Bisec}
    \end{subfigure}\hfil % <-- added
    \begin{subfigure}[t]{0.28\textwidth}
    \centering
      \includegraphics[width=\linewidth]{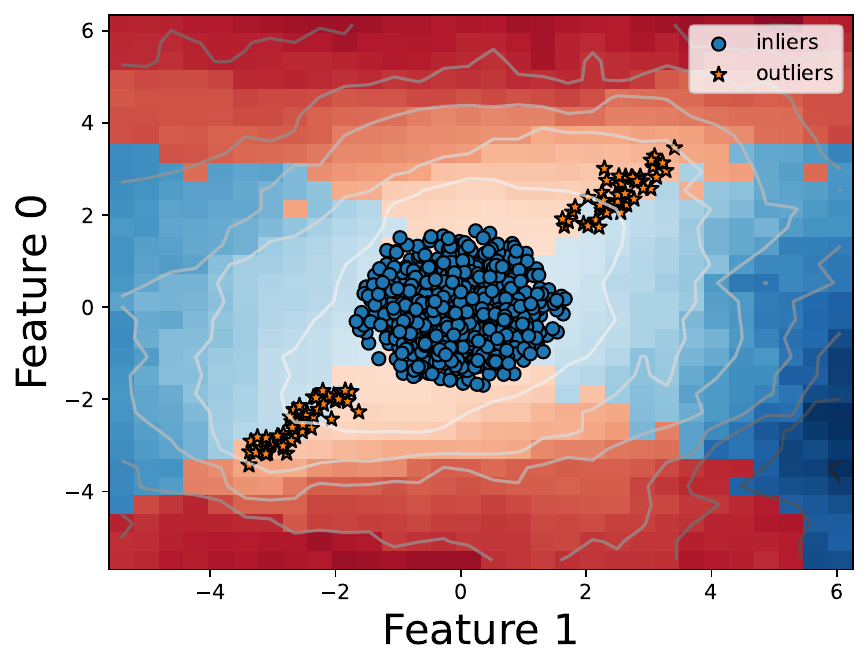}
      \caption{Scoremap {\ttfamily Bisec} Scenario I}
      \label{fig:Local-Bisec}
    \end{subfigure}\hfil % <-- added
    \begin{subfigure}[t]{0.33\textwidth}
    \centering
      \includegraphics[width=\linewidth]{Newfigures/Bisec/Importance_plots/25-03-2024_11-17-00_GFI_Bar_plot_bisect_EXIFFI+_1.pdf}
      \caption{Bar Plot {\ttfamily Bisec} Scenario II}
      \label{fig:GFI-Bisec-split}
    \end{subfigure}\hfil % <-- added
    \begin{subfigure}[t]{0.27\textwidth}
    \centering
      \includegraphics[width=\linewidth]{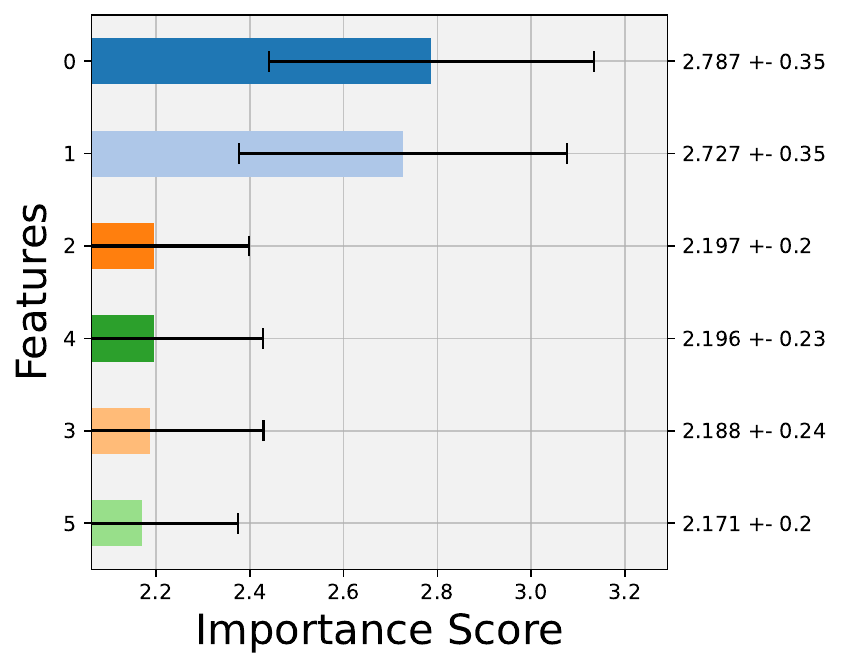}
      \caption{Score Plot {\ttfamily Bisec} Scenario II}
      \label{fig:Feat-imp-Bisec-split}
    \end{subfigure}\hfil % <-- added
    \begin{subfigure}[t]{0.28\textwidth}
    \centering
      \includegraphics[width=\linewidth]{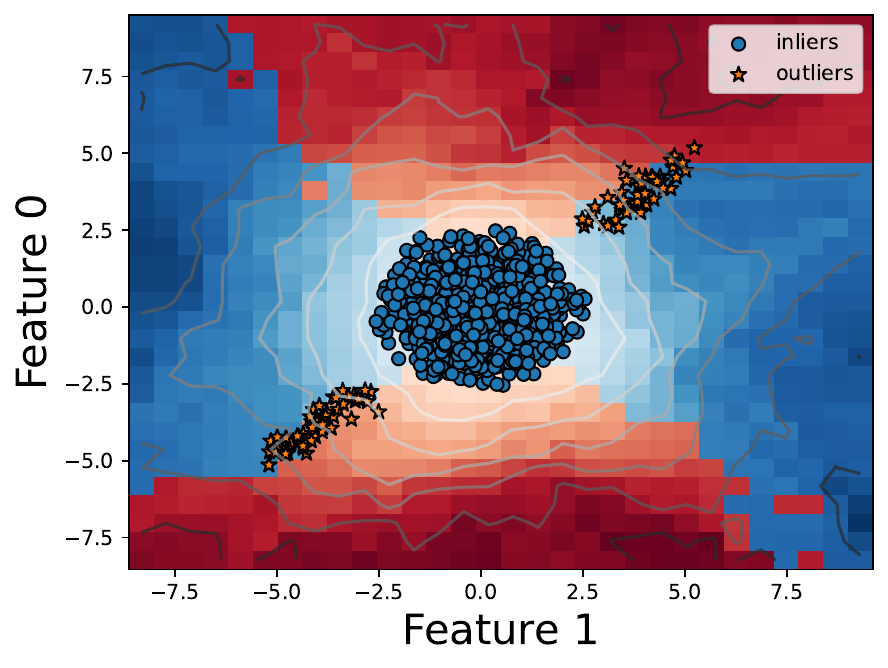}
      \caption{Scoremap {\ttfamily Bisec} Scenario II}
      \label{fig:Local-Bisec-split}
    \end{subfigure}\hfil % <-- added
\caption{Bar Plot, Score Plot and Scoremap for {\ttfamily Bisec} in the two different Scenarios, using the ExIFFI algorithm applied to the \EIFplus model.}\label{fig:interpretation-Bisec}
\end{figure}

\subsubsection{Feature Selection} \label{sec:Bisec-fs}

\ale{The plots obtained as a result of the application of the Unsupervised Feature Selection proxy task, represented in Figure \ref{fig:fs-interpretation-Bisec}, present a similar behavior. For what concerns the Feature Selection approach in which at every step the least important feature is excluded (i.e. red line) the Average Precision obtains constantly a perfect score of 1. On the the other hand, if attributes are removed starting from the most relevant one the precision drops significantly after both Feature 0 and Feature 1 are excluded, testifying the importance of these attributes, without which the model performances experience a dramatic degradation.}

\begin{figure}[!ht] 
\centering
\hspace{0.05\textwidth}\textbf{IF} \hspace{0.29\textwidth} \textbf{EIF} \hspace{0.29\textwidth} \textbf{EIF+}
% First row with vertical caption on the left
\begin{minipage}{\textwidth}
    \rotatebox{90}{\parbox{15mm}{\centering \textbf{Ad-Hoc}}} % Adjust the parbox width as necessary for your caption text
    \begin{minipage}{0.95\textwidth}
        \begin{subfigure}[t]{0.30\textwidth}
            \centering
            \includegraphics[trim={0 0 3.5cm 0}, clip, width=\linewidth]{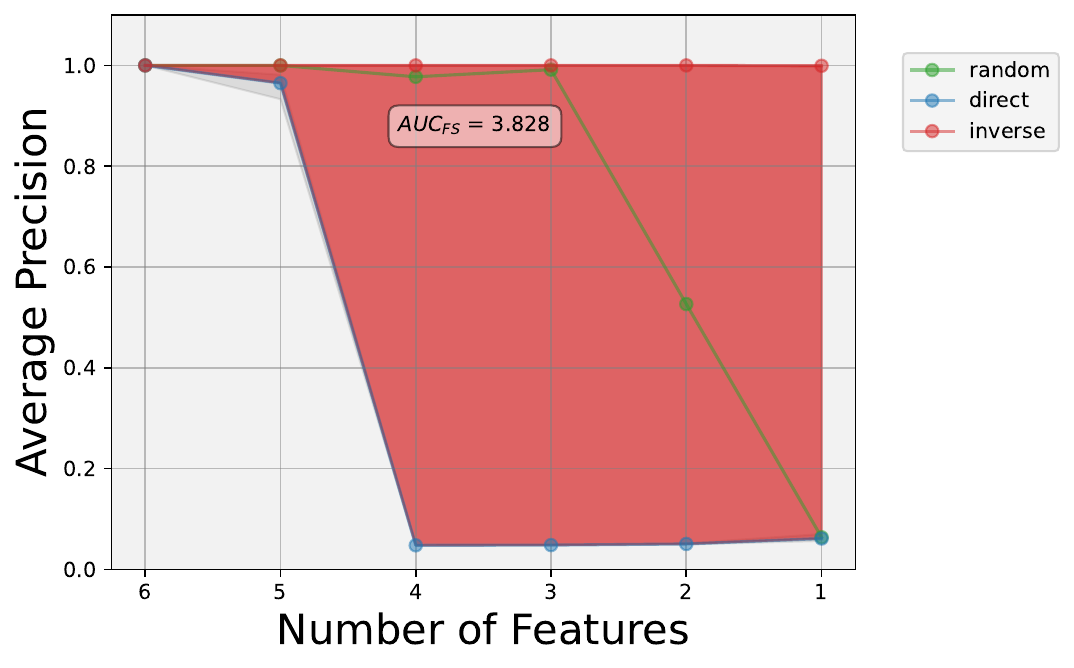}
            \caption{\approach applied to IF}
            \label{fig:Feat-Sel_Bisec_valEIF+_DIFFI_2}
        \end{subfigure}\hfill
        \begin{subfigure}[t]{0.30\textwidth}
            \centering
            \includegraphics[trim={0 0 3.5cm 0}, clip, width=\linewidth]{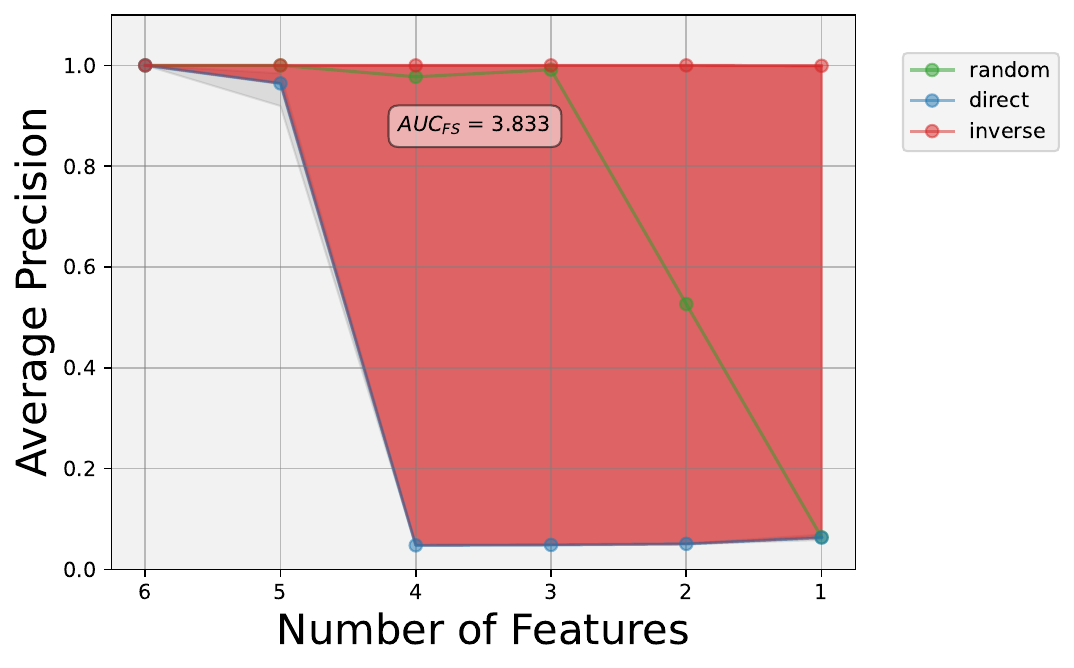}
            \caption{\approach applied to EIF}
            \label{fig:Feat-Sel_Bisec_valEIF+_EXIFFI_2}
        \end{subfigure}\hfill
        \begin{subfigure}[t]{0.30\textwidth}
            \centering
            \includegraphics[trim={0 0 3.5cm 0}, clip, width=\linewidth]{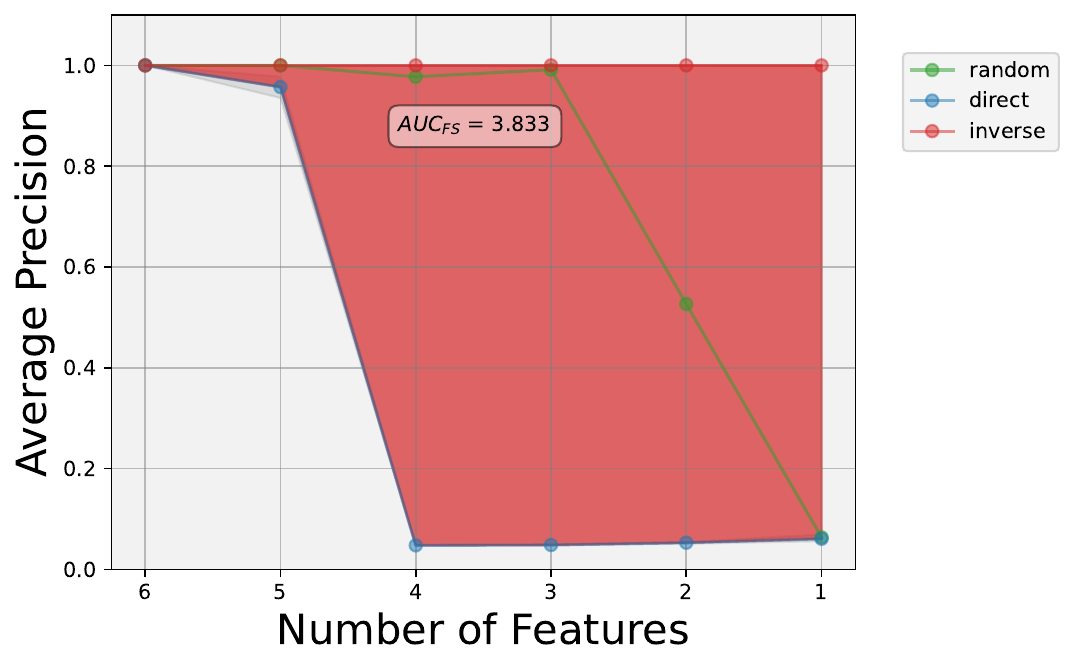}
            \caption{\approach applied to \EIFplus}
            \label{fig:Feat-Sel_Bisec_valEIF+_EXIFFI+_2}
        \end{subfigure}
    \end{minipage}
\end{minipage}

\vspace{5mm} % Space between rows

% Second row with vertical caption on the left
\begin{minipage}{\textwidth}
    \rotatebox{90}{\parbox{15mm}{\centering \textbf{Post-Hoc}}} % Adjust as necessary
    \begin{minipage}{0.95\textwidth}
        \begin{subfigure}[t]{0.30\textwidth}
            \centering
            \includegraphics[trim={0 0 3.5cm 0}, clip, width=\linewidth]{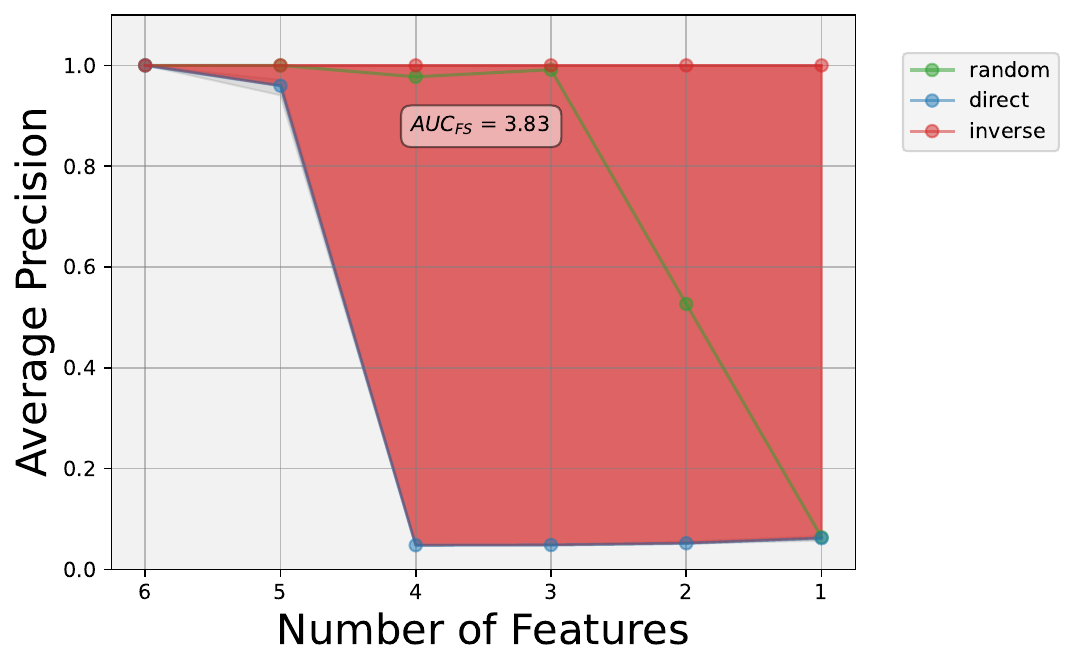}
            \caption{RandomForest fitted to IF}
            \label{fig:Feat-Sel_Bisec_valEIF+_IF_RandomForest_2}
        \end{subfigure}\hfill
        \begin{subfigure}[t]{0.30\textwidth}
            \centering
            \includegraphics[trim={0 0 3.5cm 0}, clip, width=\linewidth]{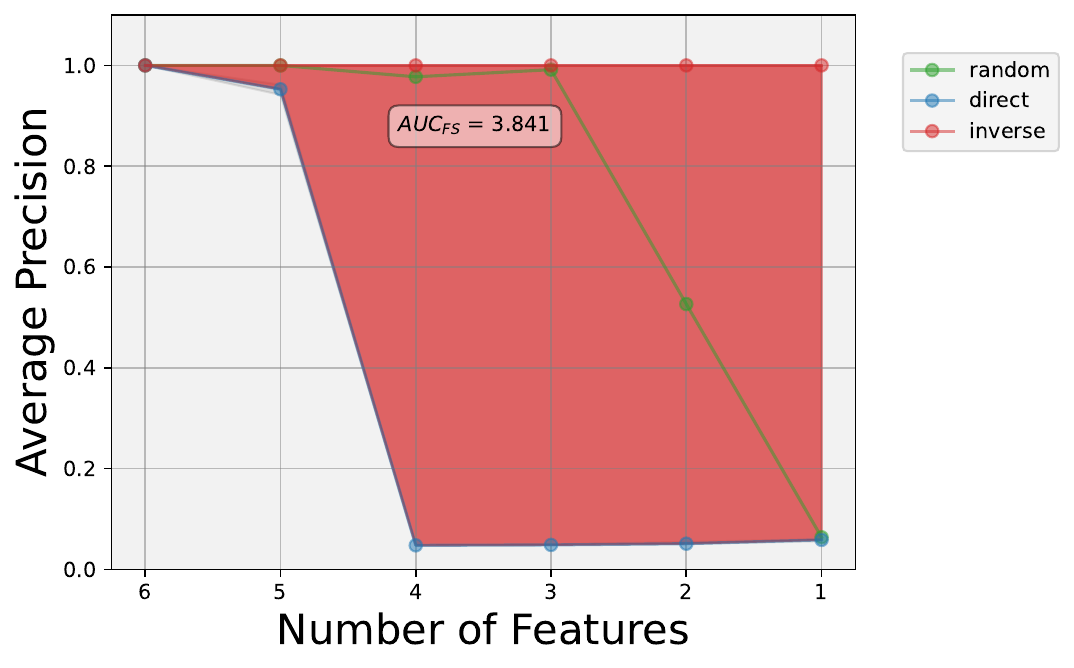}
            \caption{RandomForest fitted to EIF}
            \label{fig:Feat-Sel_Bisec_valEIF+_EIF_RandomForest_2}
        \end{subfigure}\hfill
        \begin{subfigure}[t]{0.30\textwidth}
            \centering
            \includegraphics[trim={0 0 3.5cm 0}, clip, width=\linewidth]{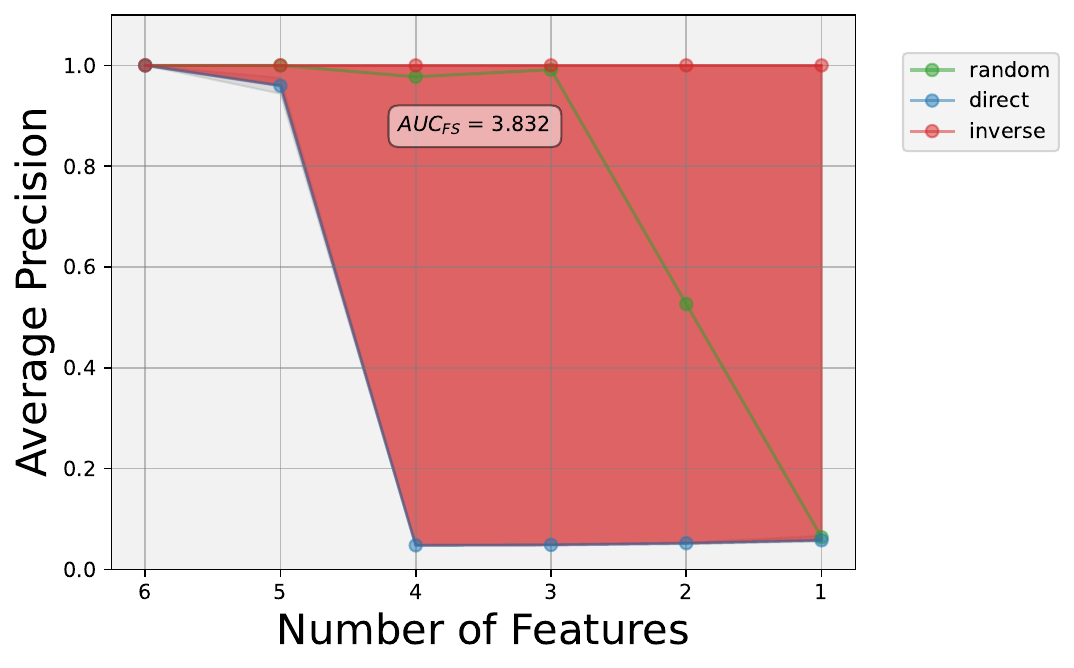}
            \caption{RandomForest fitted to \EIFplus}
            \label{fig:Feat-Sel_Bisec_valEIF+_EIF+_RandomForest_2}
        \end{subfigure}
    \end{minipage}
\end{minipage}

\caption{Feature Selection of the different Ad-Hoc and Post-Hoc methods applied to the 3 Isolation Forest models: IF, EIF and \EIFplus. The blue line is the values of average precision, calculated with the \EIFplus model in the Scenario II, dropping the most important feature at each step, the red line is the values of average precision dropping the least important feature at each step and the green line is the value of the feature selection dropping a random feature at each step.}\label{fig:fs-interpretation-Bisec}
\end{figure}

\ale{Various interpretation algorithms are quantitatively compared through the usage of the $AUC_{FS}$ metric, whose values are reported in Table \ref{tab:fs-tab-Bisec} . Because of the similarity across the plots observed in \ref{sec:Bisec-fs} the values of  $AUC_{FS}$ are comparable, thus all the models are valid choices. If a selection has to be made in order to use one of the cited models in a practical application the choice would fall on the proposed \approach and \approach+ that achieve a significant speed up in the computation of the importance scores with the respect to the other models.}

\subsection{Real World Experiments} \label{sec:appendix-real-world-experiments}
\subsection*{{\ttfamily Annthyroid}}

\subsubsection{Performance}
\ale{In Figure \ref{fig:Annthyroid_contamination}, we note that the DIF, EIF, and \EIFplus models exhibit similar performance levels, whereas the IF model overall surpasses them on this specific dataset, likely due to its structural characteristics. Interestingly, at a contamination value of $0$, the \EIFplus model slightly outperforms the others, underscoring its superior capability to generalize across unseen anomalies. This is particularly evident in Figure \ref{fig:Annthyroid_contaminationEIFvsEIF+}, where the \EIFplus model starts with negligible differences from EIF at a contamination level of $0.1$, but its advantage becomes more pronounced as the contamination level decreases. This pattern suggests the \EIFplus model's enhanced adaptability and effectiveness in handling datasets with lower contamination rates.}

\begin{figure}[!ht] 
    \centering % <-- added
    \begin{subfigure}[t]{0.49\textwidth}
      \includegraphics[width=\linewidth]{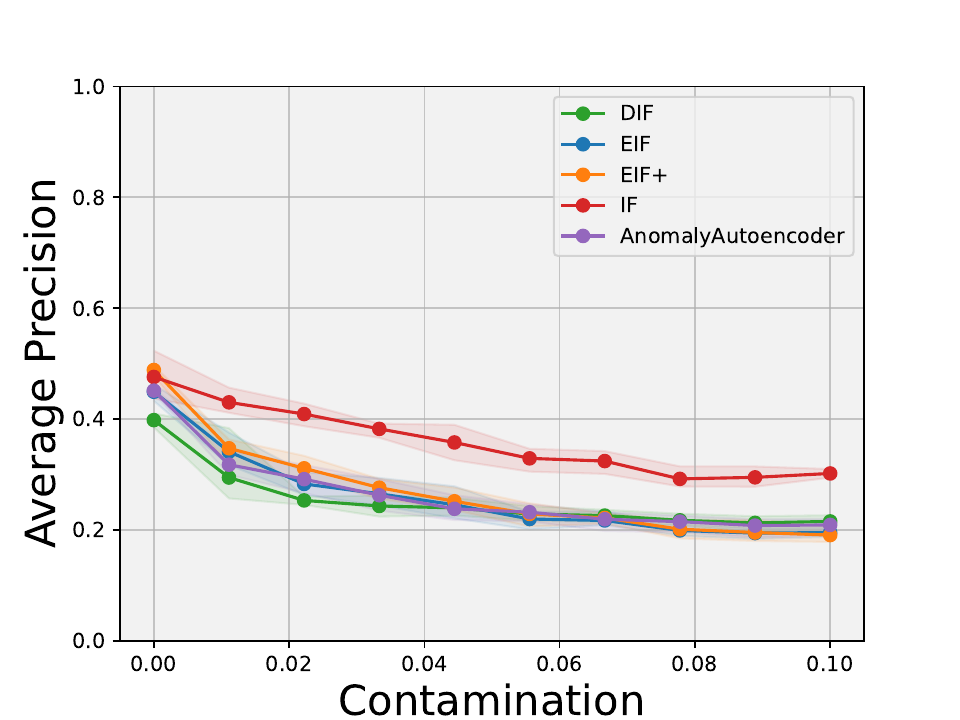}
      \caption{Models evaluation, varying the contamination levels}
      \label{fig:Annthyroid_contamination_full}
    \end{subfigure}\hfil % <-- added
    \begin{subfigure}[t]{0.44\textwidth}
      \includegraphics[width=\linewidth]{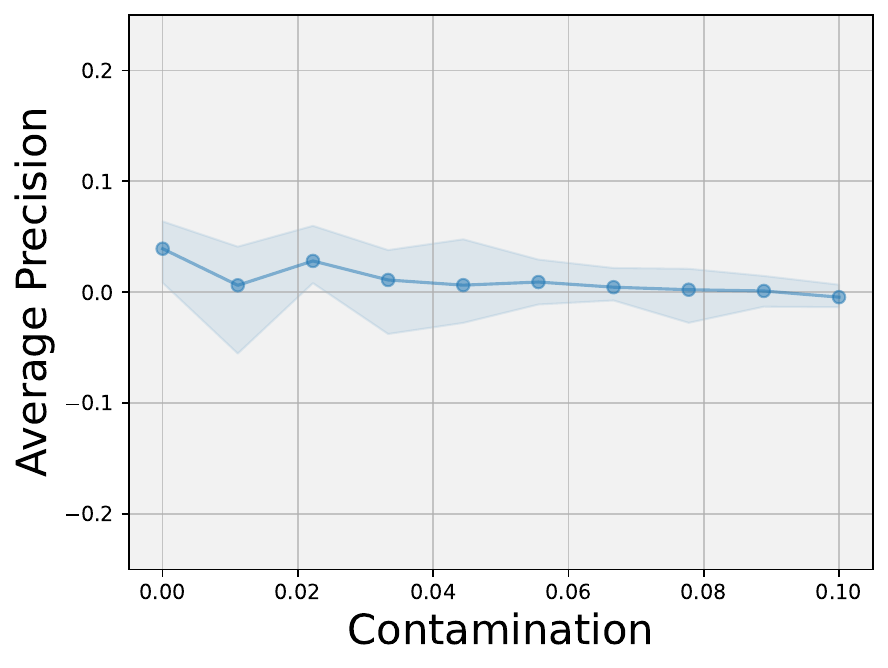}
      \caption{Difference between \EIFplus and EIF average precision}
      \label{fig:Annthyroid_contaminationEIFvsEIF+}
    \end{subfigure}\hfil % <-- added
\caption{Figure \ref{fig:Annthyroid_contamination_full} illustrates the average precision as the contamination level in the training set increases. Figure \ref{fig:Annthyroid_contaminationEIFvsEIF+} compares the performance graphs of EIF and \EIFplus, using the difference of their scores in various contamination levels.}
\label{fig:Annthyroid_contamination}
\end{figure}

\ale{The Table \ref{tab:Annthyroid_perf}  elaborates on the numerical results depicted in the plots from Figure \ref{fig:Annthyroid_contamination}, detailing the performance improvement from Scenario I to Scenario II. The most notable enhancement is observed with the \EIFplus model, which not only demonstrates significant performance gains but also retains the fastest computational efficiency in model fitting—being 100 times quicker than the DIF model. Additionally, it boasts the second-best timing in prediction speed. This showcases \EIFplus's dual advantage of superior anomaly detection capability across different scenarios and exceptional computational performance, highlighting its practicality for real-world applications.}

\begin{table}[htbp]
\centering
%\caption{{\ttfamily Annthyroid} Precision Report}
\caption{Performances of 5 different Anomaly Detection models over {\ttfamily Annthyroid} are compared using classical Classification metrics. Moreover, the last two columns contain the average time for a fit and predict operation. The highest metric values and the lowest execution times are highlighted in bold}\label{tab:Annthyroid_perf}
\begin{tabular}{|c||ccc|ccc||cc|}
\toprule
\hline
&\multicolumn{3}{c|}{Scenario I}&\multicolumn{3}{c||}{Scenario II}&\multicolumn{2}{c|}{Time}\\
\hline
AD Model & Avg & Prec & ROC & Avg & Prec & ROC & fit & pred \\
& Prec &  & AUC & Prec &  & AUC & fit & pred \\
\hline
IF          & \textbf{0.30} & \textbf{0.32} & \textbf{0.63} & 0.45 & 0.43 & 0.69 & 0.17 & \textbf{0.15} \\
EIF         & 0.19 & 0.24 & 0.59 & 0.45 & 0.41 & 0.68 & 0.09 & 0.43 \\
\EIFplus       & 0.20 & 0.28 & 0.61 & \textbf{0.46} & \textbf{0.46} & \textbf{0.70} & \textbf{0.08} & 0.35 \\
DIF         & 0.21 & 0.26 & 0.6 & 0.39 & 0.39 & 0.67 & 8.85 & 6.9 \\
AE & 0.21 & 0.25 & 0.59 & 0.44 & 0.42 & 0.69 & 16.7 & 0.29 \\
\hline
\end{tabular}
\end{table}

\subsubsection{Importance Plots}

\ale{In Figure \ref{fig:interpretation-annthyroid}, the interpretation plots for both scenarios reveal Feature 1 as the most significant, exhibiting greater robustness in Scenario II, where the model was trained solely on inliers. This robustness likely stems from enhanced precision scores. The scoremaps in Figures \ref{fig:Local-annthyroid} and \ref{fig:Local-annthyroid-split} highlight a unique distribution pattern across Features 1 and 5, suggesting a dependency between them. Notably, anomalies predominantly align along Feature 1, despite some outliers along Feature 5 that appear distanced from the normal distribution, potentially impacting negatively the right prediction of the outliers which has a significant effect on interpretation outcomes. In Scenario II, the local scoremap more clearly demonstrates how anomalies are concentrated in areas where Feature 1 holds greater significance, offering insights into the feature's critical role in anomaly distribution.}

\begin{figure}[!ht] 
    \centering % <-- added
    \begin{subfigure}[t]{0.33\textwidth}
    \centering
      \includegraphics[width=\linewidth]{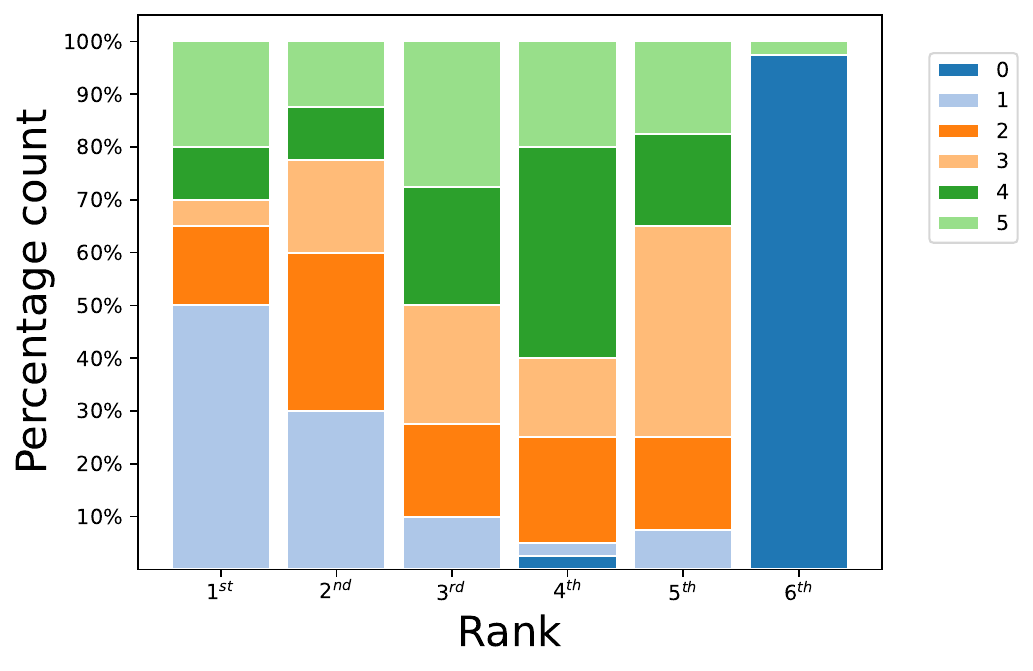}
      \caption{Score Plot {\ttfamily Annthyroid} Scenario I}
      \label{fig:Feat-imp-Annthyroid}
    \end{subfigure}\hfil % <-- added
    \begin{subfigure}[t]{0.27\textwidth}
    \centering
      \includegraphics[width=\linewidth]{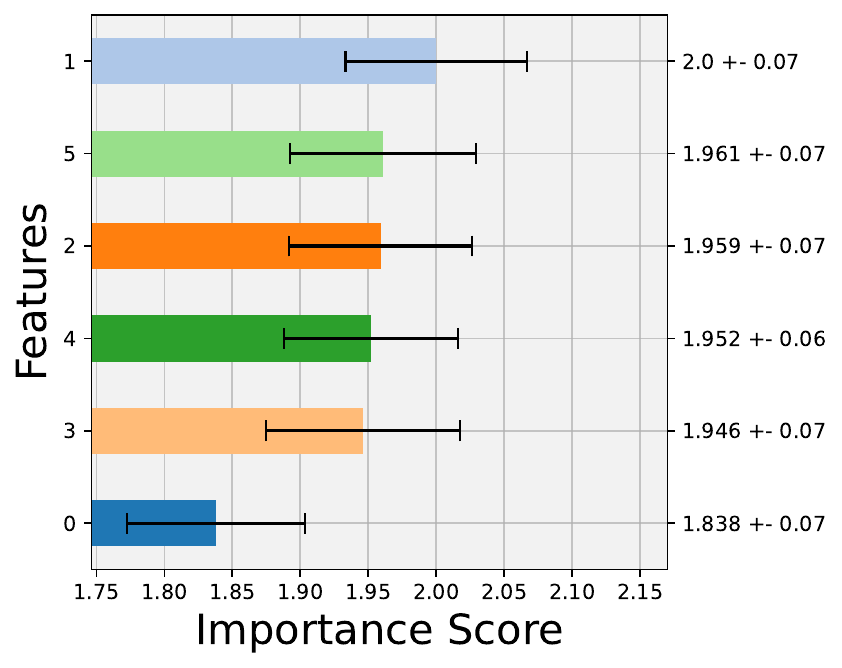}
      \caption{Bar Plot {\ttfamily Annthyroid} Scenario I}
      \label{fig:GFI-annthyroid}
    \end{subfigure}\hfil % <-- added
    \begin{subfigure}[t]{0.28\textwidth}
    \centering
      \includegraphics[width=\linewidth]{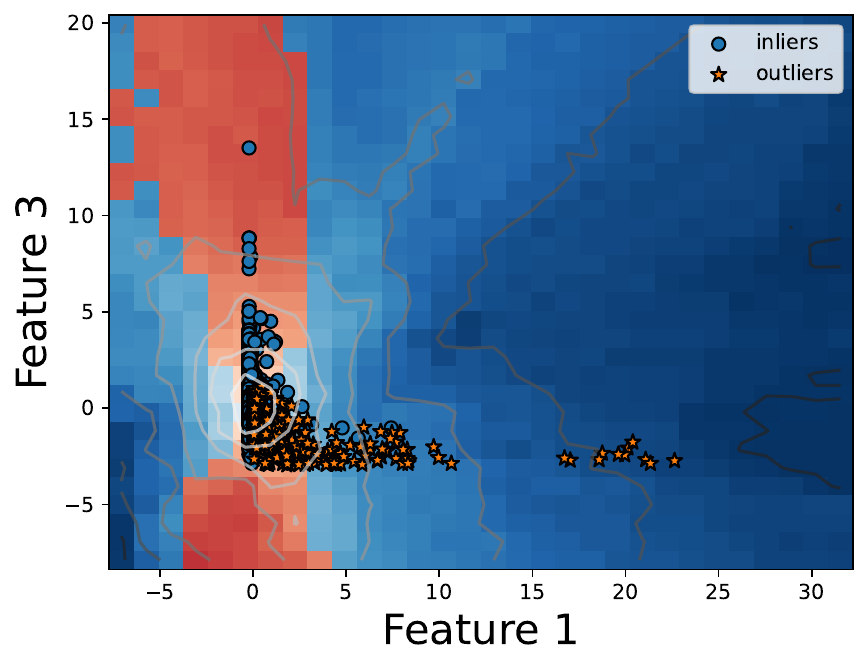}
      \caption{Scoremap {\ttfamily Annthyroid} Scenario I}
      \label{fig:Local-annthyroid}
    \end{subfigure}\hfil % <-- added
    \begin{subfigure}[t]{0.33\textwidth}
    \centering
      \includegraphics[width=\linewidth]{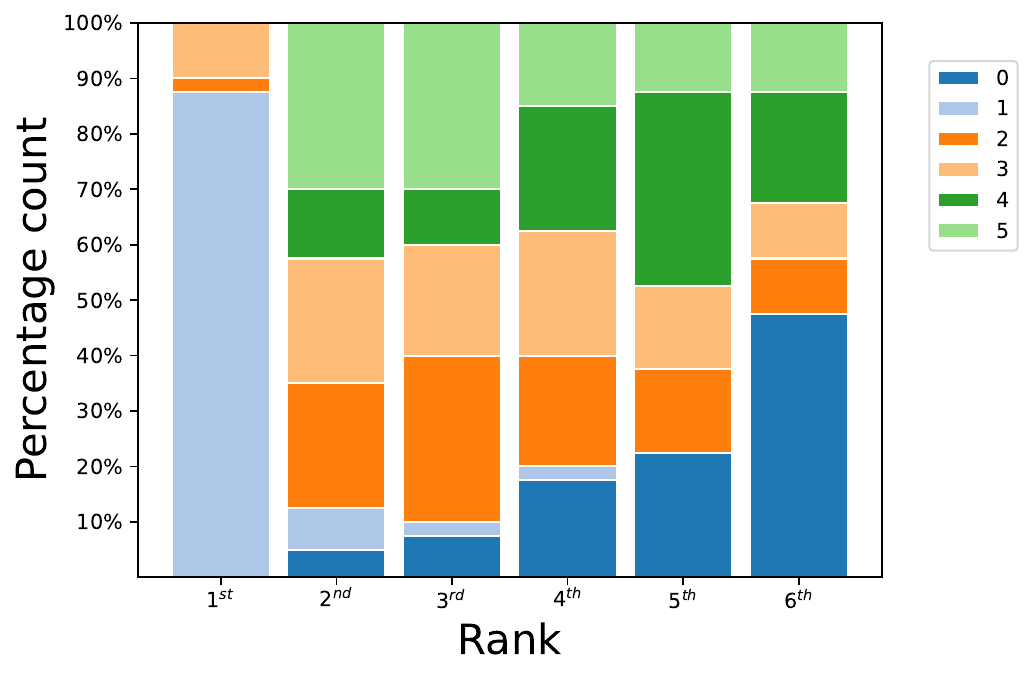}
      \caption{Score Plot {\ttfamily Annthyroid} Scenario II}
      \label{fig:Feat-imp-Annthyroid-split}
    \end{subfigure}\hfil % <-- added
    \begin{subfigure}[t]{0.27\textwidth}
    \centering
      \includegraphics[width=\linewidth]{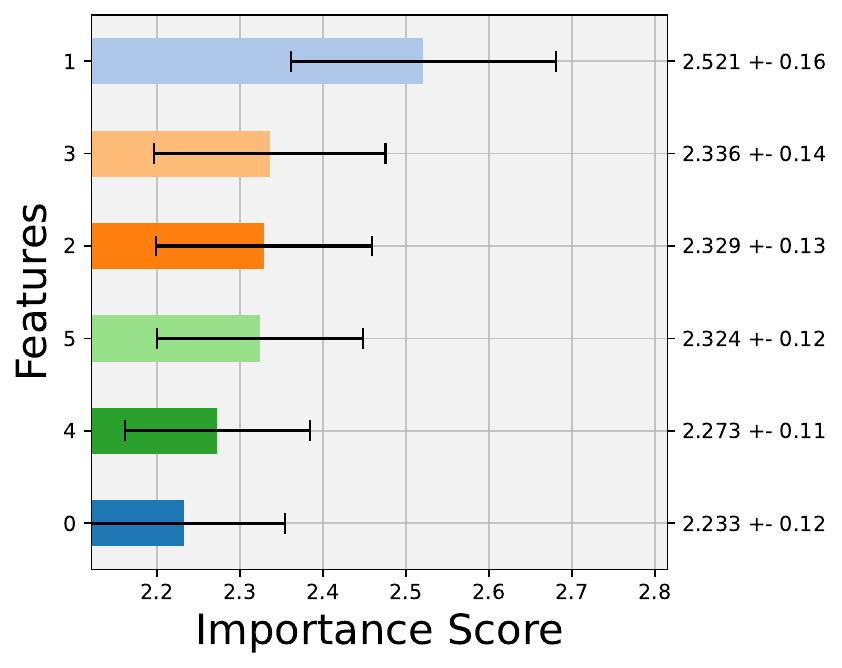}
      \caption{Bar Plot {\ttfamily Annthyroid} Scenario II}
      \label{fig:GFI-annthyroid-split}
    \end{subfigure}\hfil % <-- added
    \begin{subfigure}[t]{0.28\textwidth}
    \centering
      \includegraphics[width=\linewidth]{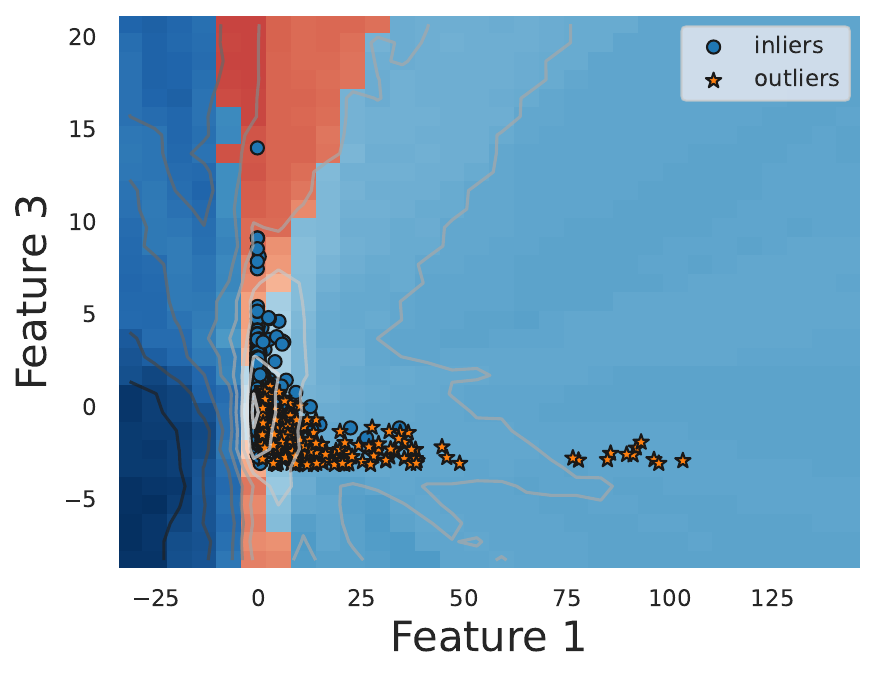}
      \caption{Scoremap {\ttfamily Annthyroid} Scenario II}
      \label{fig:Local-annthyroid-split}
    \end{subfigure}\hfil % <-- added
\caption{Bar Plot, Score Plot and Scoremap for {\ttfamily Annthyroid} in the two different Scenarios, using the \approach algorithm applied to the \EIFplus model.}\label{fig:interpretation-annthyroid}
\end{figure}

\subsubsection{Feature Selection}

\ale{Figure \ref{fig:interpretation-annthyroid} showcases the Feature Selection plots derived from the feature rankings provided by two distinct interpretation algorithms for each of the three Isolation based model, including one ad-hoc and one post-hoc interpretation via a surrogate Random Forest model. These plots depict the average precision achieved by the \EIFplus model on the dataset, progressively excluding the least important feature as identified by each interpretation algorithm (illustrated by the red line), and excluding the most important feature at every step (shown by the blue line). The similarity in the plots, particularly within the extent of the red areas, indicates that the Feature Selection outcomes are largely equivalent.} 

\begin{figure}[htbp] 
\centering
\hspace{0.05\textwidth}\textbf{IF} \hspace{0.29\textwidth} \textbf{EIF} \hspace{0.29\textwidth} \textbf{EIF+}
% First row with vertical caption on the left
\begin{minipage}{\textwidth}
    \rotatebox{90}{\parbox{15mm}{\centering \textbf{Ad-Hoc}}} % Adjust the parbox width as necessary for your caption text
    \begin{minipage}{0.95\textwidth}
        \begin{subfigure}[t]{0.30\textwidth}
            \centering
            \includegraphics[trim={0 0 3.5cm 0}, clip, width=\linewidth]{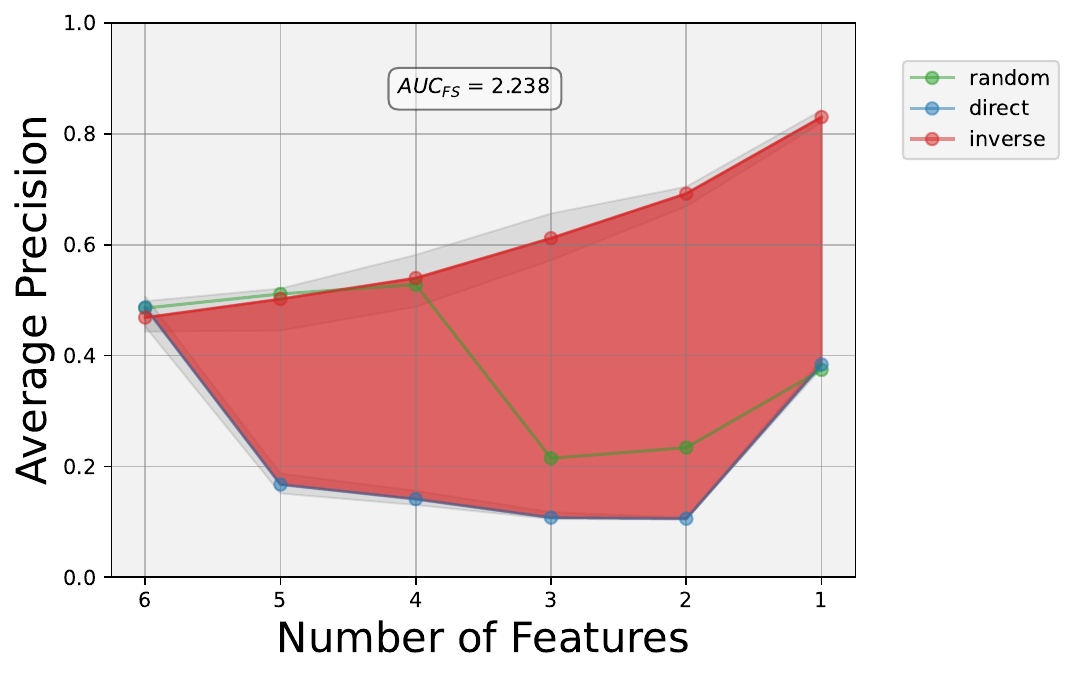}
            \caption{\approach applied to IF}
            \label{fig:Feat-Sel_Annthyroid_valEIF+_DIFFI_2}
        \end{subfigure}\hfill
        \begin{subfigure}[t]{0.30\textwidth}
            \centering
            \includegraphics[trim={0 0 3.5cm 0}, clip, width=\linewidth]{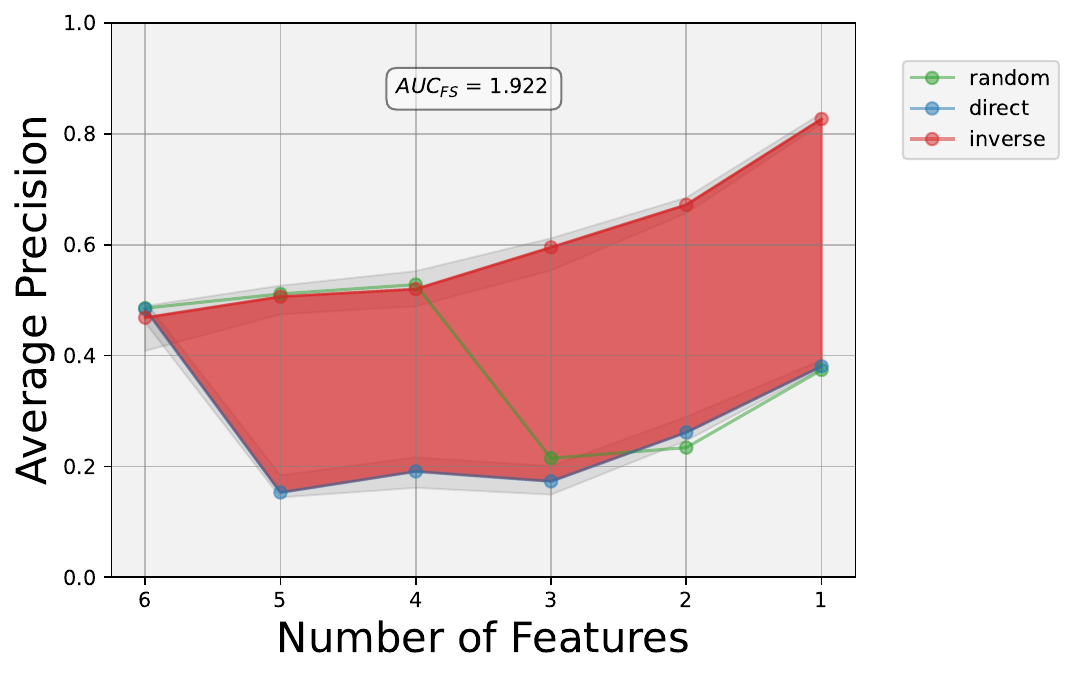}
            \caption{\approach applied to EIF}
            \label{fig:Feat-Sel_Annthyroid_valEIF+_EXIFFI_2}
        \end{subfigure}\hfill
        \begin{subfigure}[t]{0.30\textwidth}
            \centering
            \includegraphics[trim={0 0 3.5cm 0}, clip, width=\linewidth]{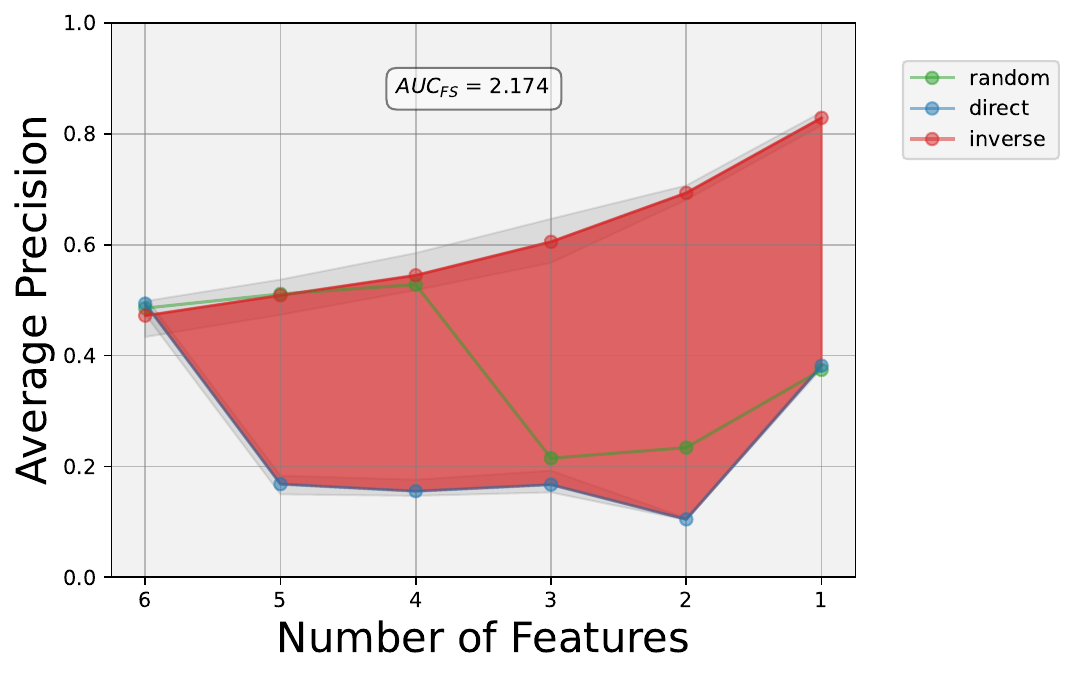}
            \caption{\approach applied to \EIFplus}
            \label{fig:Feat-Sel_Annthyroid_valEIF+_EXIFFI+_2}
        \end{subfigure}
    \end{minipage}
\end{minipage}

\vspace{5mm} % Space between rows

% Second row with vertical caption on the left
\begin{minipage}{\textwidth}
    \rotatebox{90}{\parbox{15mm}{\centering \textbf{Post-Hoc}}} % Adjust as necessary
    \begin{minipage}{0.95\textwidth}
        \begin{subfigure}[t]{0.30\textwidth}
            \centering
            \includegraphics[trim={0 0 3.5cm 0}, clip, width=\linewidth]{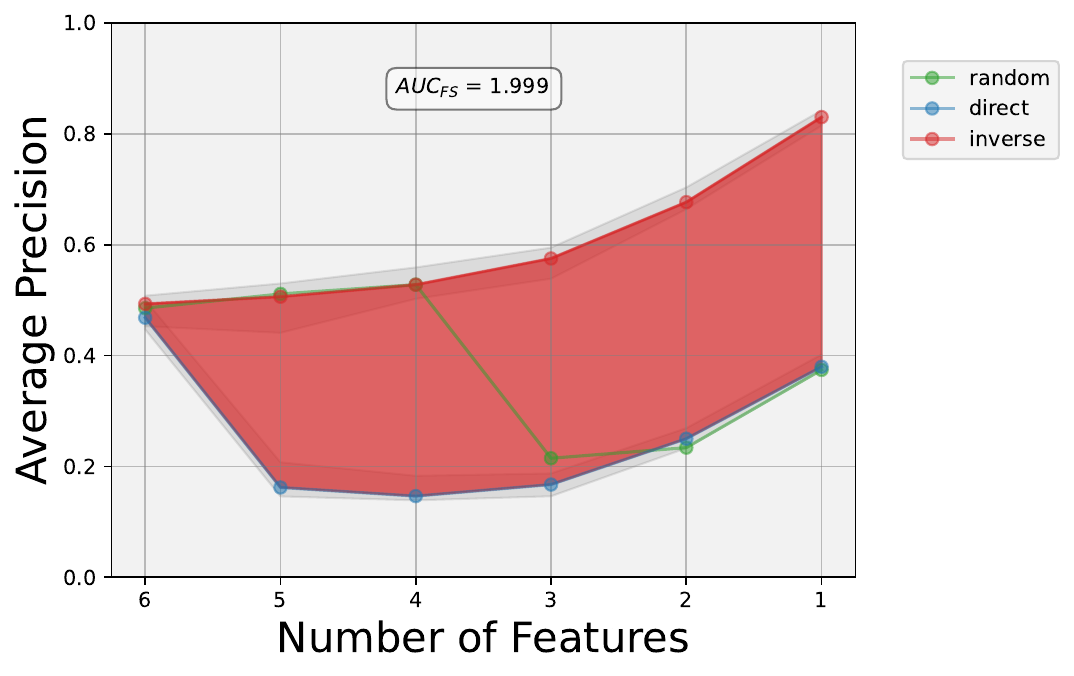}
            \caption{RandomForest fitted to IF}
            \label{fig:Feat-Sel_Annthyroid_valEIF+_IF_RandomForest_2}
        \end{subfigure}\hfill
        \begin{subfigure}[t]{0.30\textwidth}
            \centering
            \includegraphics[trim={0 0 3.5cm 0}, clip, width=\linewidth]{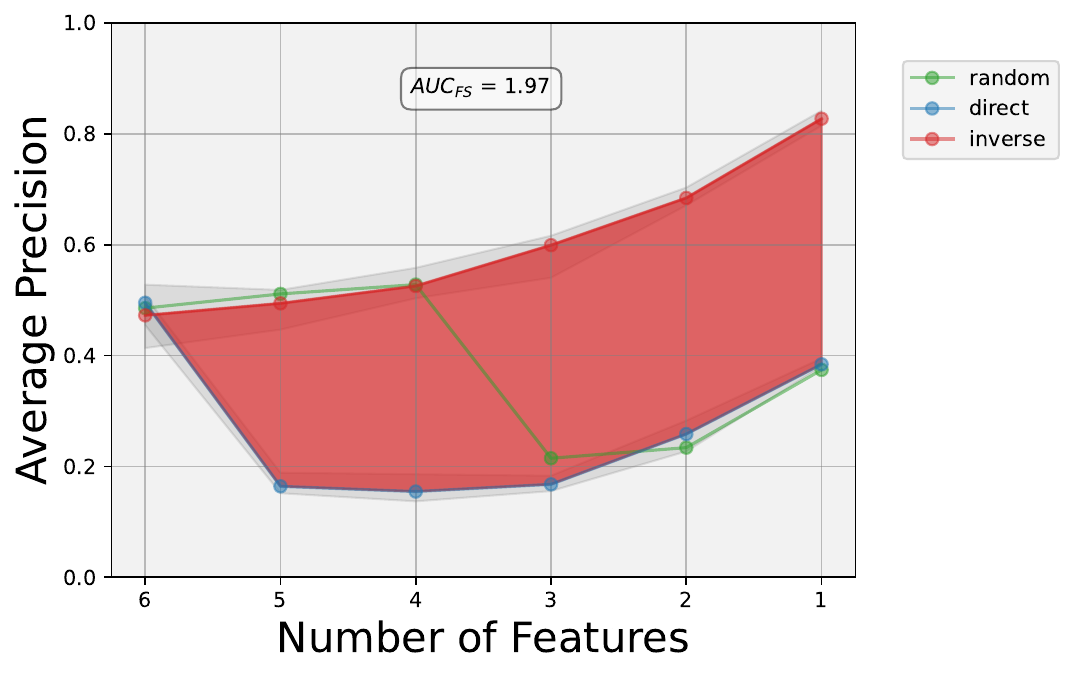}
            \caption{RandomForest fitted to EIF}
            \label{fig:Feat-Sel_Annthyroid_valEIF+_EIF_RandomForest_2}
        \end{subfigure}\hfill
        \begin{subfigure}[t]{0.30\textwidth}
            \centering
            \includegraphics[trim={0 0 3.5cm 0}, clip, width=\linewidth]{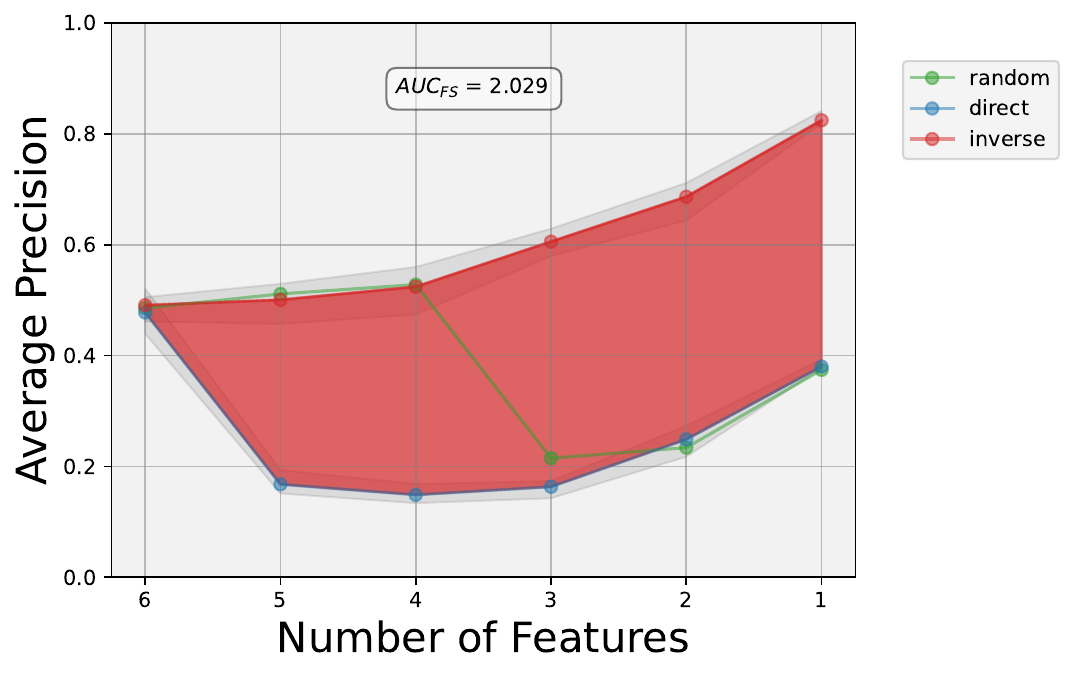}
            \caption{RandomForest fitted to \EIFplus}
            \label{fig:Feat-Sel_Annthyroid_valEIF+_EIF+_RandomForest_2}
        \end{subfigure}
    \end{minipage}
\end{minipage}

\caption{Feature Selection of the different Ad-Hoc and Post-Hoc methods applied to the 3 Isolation Forest models: IF, EIF and \EIFplus. The blue line is the values of average precision, calculated with the \EIFplus model in the Scenario II, dropping the most important feature at each step, the red line is the values of average precision dropping the least important feature at each step and the green line is the value of the feature selection dropping a random feature at each step.}\label{fig:feature_selections-annthyroid}
\end{figure}

\ale{Table \ref{tab:fs-tab-annthyroid}  highlights distinct performance variations between Scenario I and Scenario II, with Scenario I showing reduced effectiveness overall, particularly in post-hoc interpretation methods. This trend suggests that reliance on post-hoc interpretations might be less beneficial when the performance of anomaly detection (AD) models is low. In contrast, ad-hoc interpretation methods exhibit more consistency and slightly improved results in Scenario II, surpassing post-hoc techniques. Among these, the interpretation of the \approach applied to the IF model stands out for its superior efficiency. Moreover, the execution speed of ad-hoc interpretations notably exceeds that of post-hoc methods, emphasizing ad-hoc strategies' effectiveness and speed across different scenarios.}

\begin{table}[htbp]
\centering
\caption{Quantitative evaluation of the effectiveness of 6 different interpretation algorithms on {\ttfamily Annthyroid} through the $AUC_{FS}$ metric, introduced in \ref{sec:interpr_evaluat}. In the last column the average time taken by the different models to produce the importance scores is reported. The highest $AUC_{FS}$ and lowest Importance time values are highlighted in bold.}\label{tab:fs-tab-annthyroid}
\begin{tabular}{|c||c|c|c|c||c|}
\toprule
\hline
&\multicolumn{2}{c|}{Evaluation with EIF}&\multicolumn{2}{c||}{Evaluation with \EIFplus}&\\
\hline
& Scenario I & Scenario II & Scenario I & Scenario II & Time\\

 Algorithm & $AUC_{FS}$  & $AUC_{FS}$ & $AUC_{FS}$  & $AUC_{FS}$ &  \\
\hline
DIFFI         & 0.963      & 2.040& 0.910& 2.000& 0.57 \\
IF\_\approach         & \textbf{1.127}      & \textbf{2.259}& \textbf{1.103}& \textbf{2.238}& 0.93 \\
EIF\_\approach        & 0.985& 2.032& 0.937& 1.922& \textbf{0.55} \\
\EIFplus\_\approach       & 0.983 & 2.180& 0.975& 2.174& 0.59 \\
IF\_RF        & 0.453& 2.055& 0.429& 1.999& 2.82 \\
EIF\_RF       & -0.689& 2.034& -0.672& 1.97& 2.82 \\
EIF+\_RF      & -1.198& 2.094& -1.165& 2.029& 2.82 \\
\hline
\end{tabular}
\end{table}

\subsection*{{\ttfamily Breastw}} \label{sec:Breastw}

\subsubsection{Performance}

\ale{Figure \ref{fig:Breastw_contamination_full} portraits the trend of the Average Precision metric as the contamination of the training set enlarges from 0 to 10 \% on the different AD methods discussed in Section \ref{sec:performance_evaluation}. It can be noticed how all the models perform more or less perfectly (i.e. with a score of 1) independently on the amount of anomalous samples seen at training time except for the DIF model that shows low precision values, around 0.6.}

\begin{figure}[!ht] 
    \centering % <-- added
    \begin{subfigure}[t]{0.49\textwidth}
      \includegraphics[width=\linewidth]{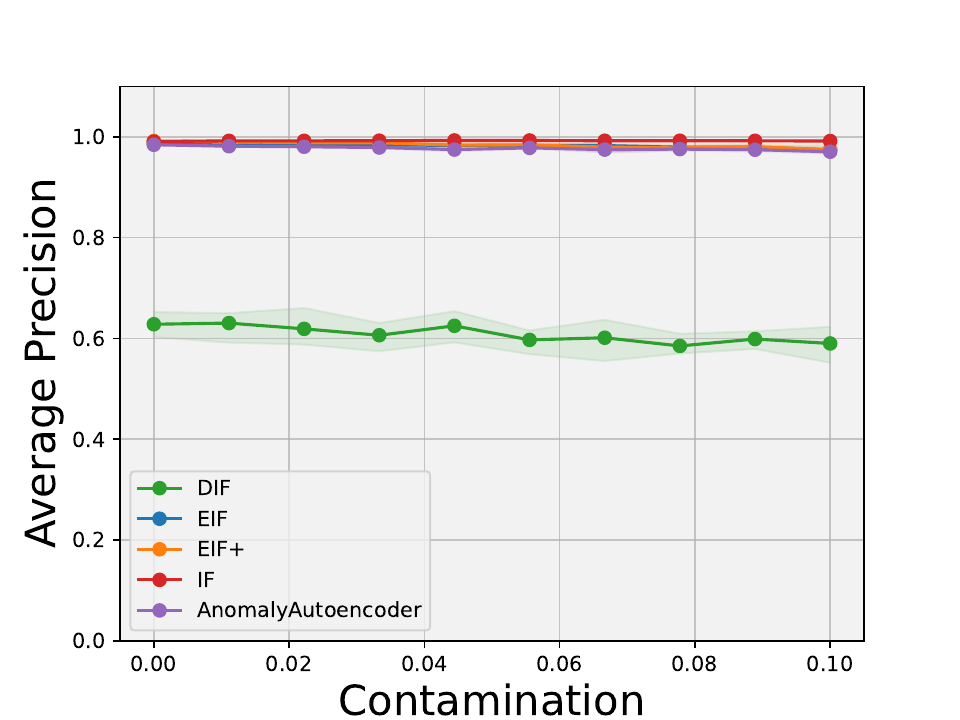}
      \caption{ }
      \label{fig:Breastw_contamination_full}
    \end{subfigure}\hfil % <-- added
    \begin{subfigure}[t]{0.44\textwidth}
      \includegraphics[width=\linewidth]{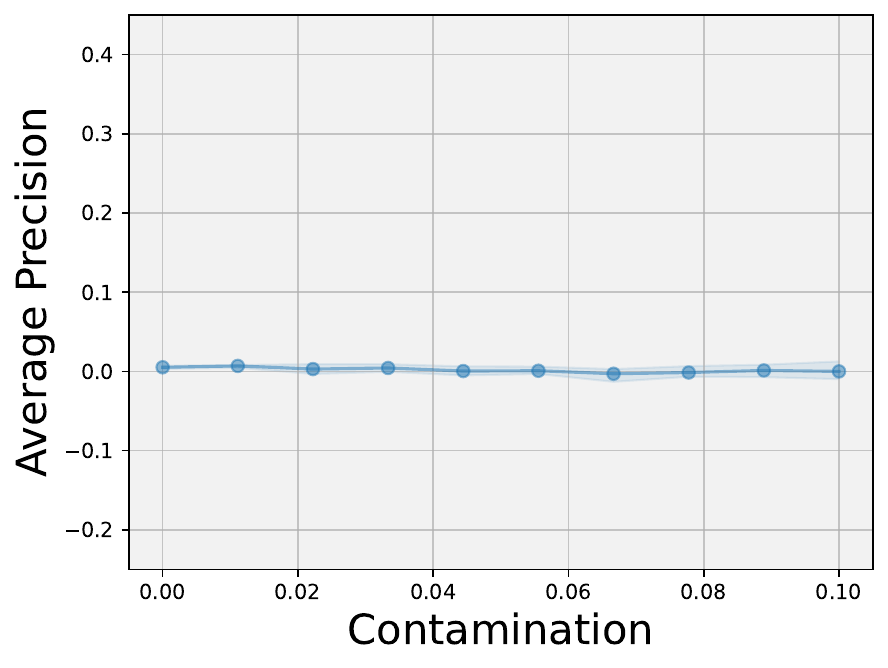}
      \caption{ }
      \label{fig:Breastw_contaminationEIFvsEIF+}
    \end{subfigure}\hfil % <-- added
\caption{Fig. \ref{fig:Breastw_contamination_full} Represent the average precision the more the level of contamination of the train set is increased. The Fig. \ref{fig:Breastw_contaminationEIFvsEIF+} Give show specifically the graphs of the EIF and EIF+}
\label{fig:Breastw_contamination}
\end{figure}

\ale{In Table \ref{tab:Breastw_perf}  it is possible to compare in detail different typical metrics used to assess the overall performances of AD models. In particular dividing the evaluation between Scenario I and Scenario II it is possible to observe how these two training strategies may or may not affect the model's performances. With regard to the {\ttfamily Breastw} dataset one can discern that there is a clear difference between the two scenarios only for the DIF model (that is in fact the only model not showing a perfectly constant trend in the Contamination Plot of Figure \ref{fig:Breastw_contamination_full}) while the other models manifest only minor changes passing from Scenario I to Scenario II. Finally in the context of time efficiency a significant gap can be observed between isolation-based approaches (i.e. IF, EIF and \EIFplus) and AD methods based on deep learning models (i.e. DIF and Autoencoder).}

\begin{table}[htbp]
\begin{minipage}[t]{0.46\textwidth}
\strut\vspace*{-\baselineskip}\newline
\resizebox{\textwidth}{!}{
%\caption{{\ttfamily Breastw} Precision Report}
\begin{tabular}{|c||ccc|ccc||cc|}
\toprule
\hline
&\multicolumn{3}{c|}{Scenario I}&\multicolumn{3}{c||}{Scenario II}&\multicolumn{2}{c|}{Time}\\
\hline
AD Model & Avg & Prec & ROC & Avg & Prec & ROC & fit & pred \\
& Prec &  & AUC & Prec &  & AUC &  &  \\
\hline
IF          & \textbf{0.96}& \textbf{0.90}& \textbf{0.90}& 0.99& 0.94& 0.94& \textbf{0.11}& 0.005\\
EIF         & 0.91& 0.86& 0.86& 0.98& 0.93& 0.93& 0.12& 0.0007\\
EIF+        & 0.88& 0.85& 0.84& \textbf{0.99}& \textbf{0.95}& \textbf{0.95}& 0.12& \textbf{0.0006}\\
DIF         & 0.44& 0.49& 0.46& 0.60& 0.66& 0.64& 0.74& 0.58\\
AE & 0.61& 0.44& 0.41& 0.98& 0.94& 0.93& 2.56& 0.05\\
\hline
\end{tabular}}
\vspace{0.41cm}
\caption{Performances of 5 different Anomaly Detection models over {\ttfamily Breastw} are compared using classical Classification metrics. Moreover, the last two columns contain the average time for a fit and predict operation. The highest metric values and the lowest execution times are highlighted in bold}\label{tab:Breastw_perf}
\end{minipage}
\hfill
\begin{minipage}[t]{0.46\textwidth}
\strut\vspace*{-\baselineskip}\newline
\resizebox{\textwidth}{!}{
\begin{tabular}{|c||c|c|c|c||c|}
\toprule
\hline
&\multicolumn{2}{c|}{Evaluation with EIF}&\multicolumn{2}{c||}{Evaluation with \EIFplus}&\\
\hline
& Scenario I & Scenario II & Scenario I & Scenario II & Time\\

 Algorithm & $AUC_{FS}$  & $AUC_{FS}$ & $AUC_{FS}$  & $AUC_{FS}$ &  \\
\hline
DIFFI         & 0.11& 0.064& 0.083& 0.067& 0.46\\
IF\_\approach        & \textbf{0.25}& 0.082& \textbf{0.284}& 0.087& 0.10\\
EIF\_\approach        & 0.044& 0.062& 0.026& 0.084& \textbf{0.04}\\
\EIFplus\_\approach       & 0.079& 0.027& 0.084& 0.063& 0.04\\
IF\_RF        & -0.148& 0.091& -0.142& 0.063& 0.19\\
EIF\_RF       & -0.181& \textbf{0.109}& -0.169& \textbf{0.090}& 0.19\\
EIF+\_RF      & -0.164& 0.104& -0.145& 0.079& 0.19\\
\hline
\end{tabular}}
\caption{Quantitative evaluation of the effectiveness of 6 different interpretation algorithms on {\ttfamily Breastw} through the $AUC_{FS}$ metric, introduced in \ref{sec:interpr_evaluat}. In the last column the average time taken by the different models to produce the importance scores is reported. The highest $AUC_{FS}$ and lowest Importance time values are highlighted in bold.}\label{tab:fs-tab-Breastw}
\end{minipage}
\end{table}

\subsubsection{Importance Plots}

\ale{The peculiar grid-like distribution of samples within the {\ttfamily Breastw} dataset, as exhibited in the Figure \ref{fig:Local-Breastw}, generates interpretation results in the Bar and Score plots not aligned with the typical outcomes described in the other real world datasets included in this study. Indeed discerning the distribution of relevance scores between different attributes is easier in Scenario I where Feature 8 clearly emerges as the crucial feature (Figure \ref{fig:Feat-imp-Breastw}  while in Scenario II the latter, still considered the most prominent as shown in Figure \ref{fig:Feat-imp-Breastw-split}, is associated with a lower margin on the other features. Figures \ref{fig:Local-Breastw} and \ref{fig:Local-Breastw-split}  illustrate the Local Scoremap that are not particularly effective in showing the distribution of anomalies as points easy to isolate from others because of the grid-like distribution of samples.}

\begin{figure}[!ht] 
    \centering % <-- added
    \begin{subfigure}[t]{0.33\textwidth}
    \centering
      \includegraphics[width=\linewidth]{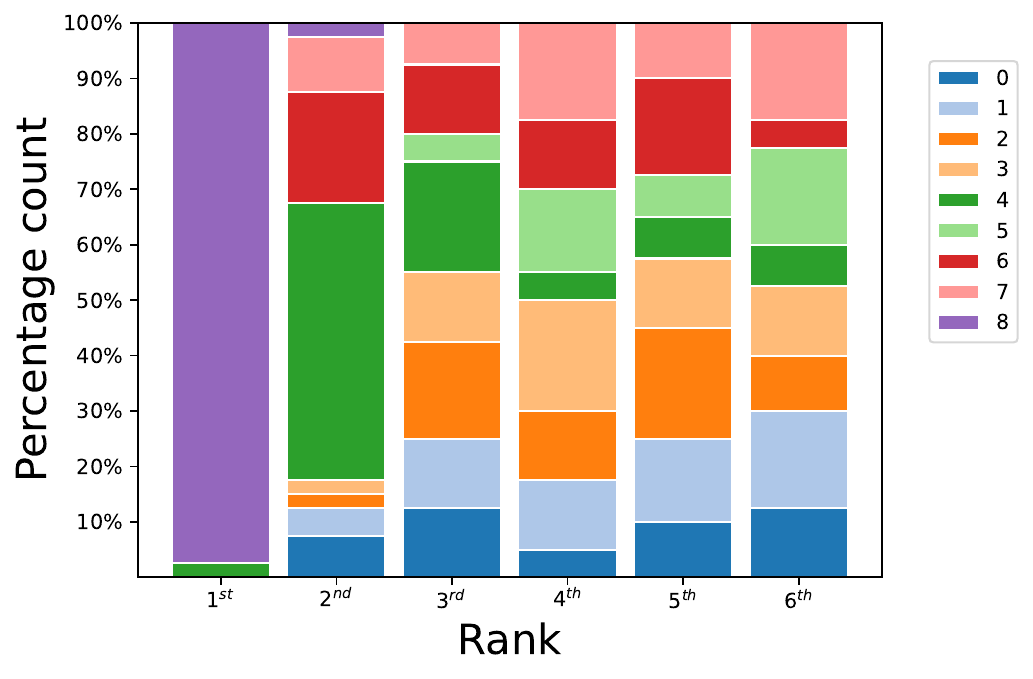}
      \caption{Score Plot {\ttfamily Breastw} Scenario I}
      \label{fig:Feat-imp-Breastw}
    \end{subfigure}\hfil % <-- added
    \begin{subfigure}[t]{0.27\textwidth}
    \centering
      \includegraphics[width=\linewidth]{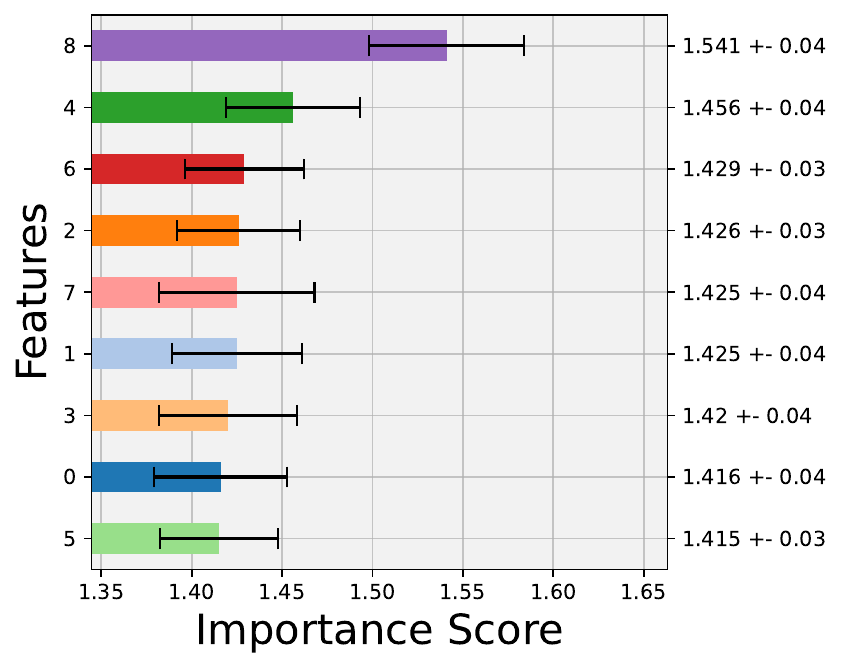}
      \caption{Bar Plot {\ttfamily Breastw} Scenario I}
      \label{fig:GFI-Breastw}
    \end{subfigure}\hfil % <-- added
    \begin{subfigure}[t]{0.28\textwidth}
    \centering
      \includegraphics[width=\linewidth]{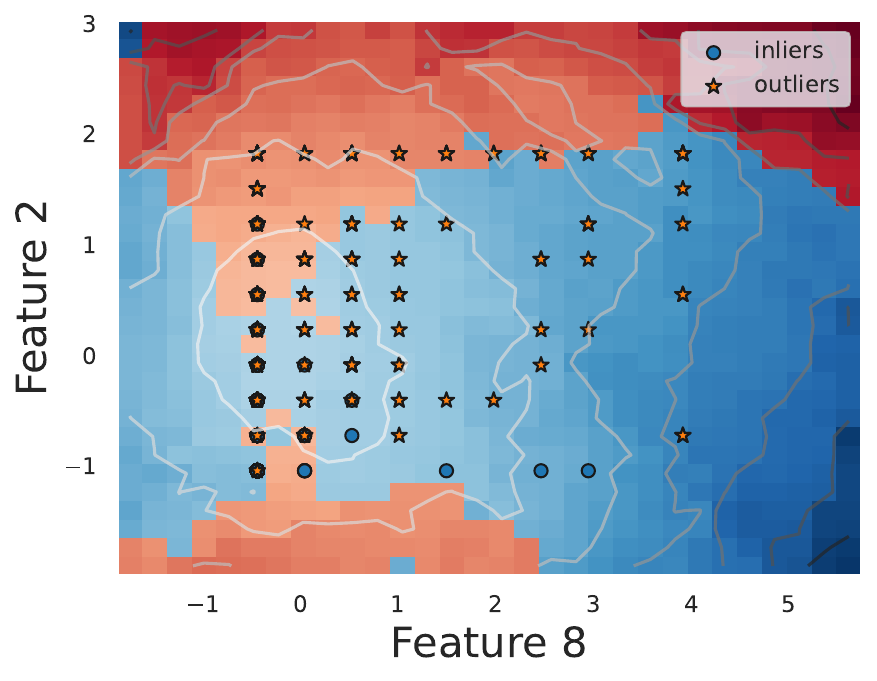}
      \caption{Scoremap {\ttfamily Breastw} Scenario I}
      \label{fig:Local-Breastw}
    \end{subfigure}\hfil % <-- added
    \begin{subfigure}[t]{0.33\textwidth}
    \centering
      \includegraphics[width=\linewidth]{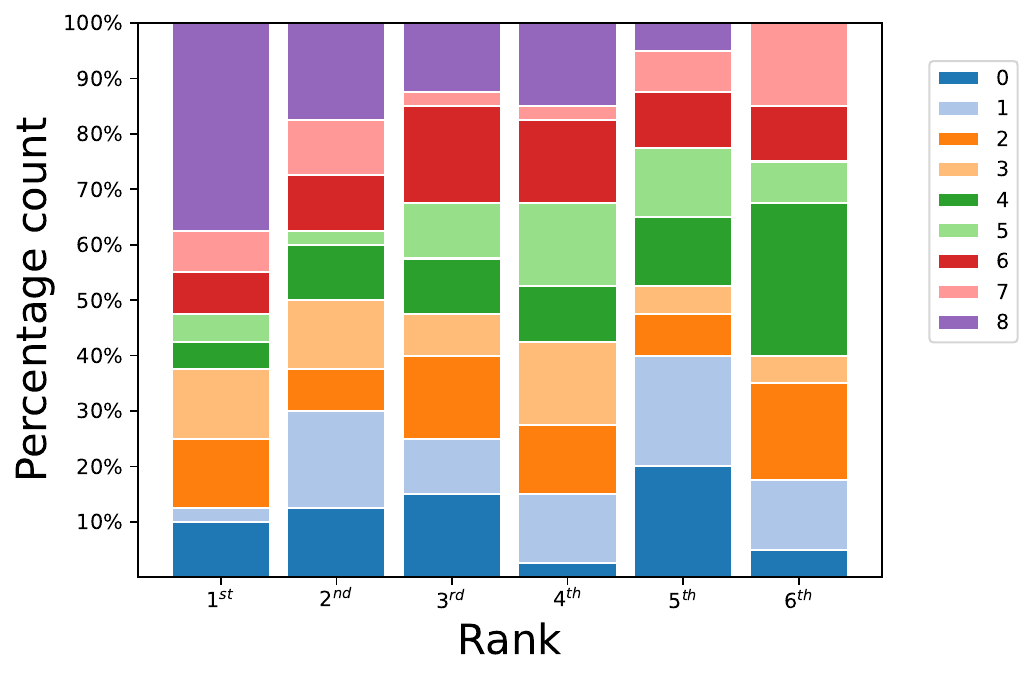}
      \caption{Score Plot {\ttfamily Breastw} Scenario II}
      \label{fig:Feat-imp-Breastw-split}
    \end{subfigure}\hfil % <-- added
    \begin{subfigure}[t]{0.27\textwidth}
    \centering
      \includegraphics[width=\linewidth]{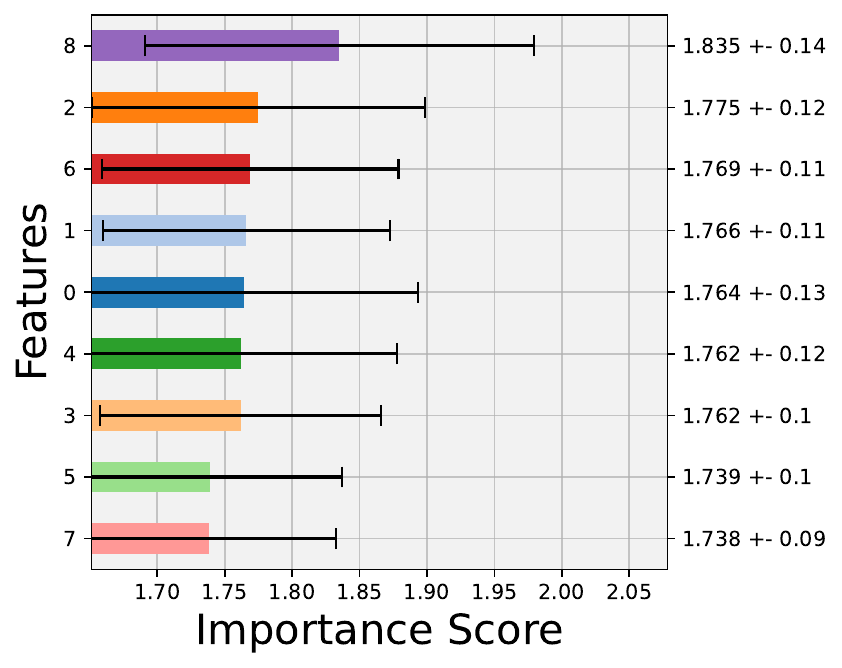}
      \caption{Bar Plot {\ttfamily Breastw} Scenario II}
      \label{fig:GFI-Breastw-split}
    \end{subfigure}\hfil % <-- added
    \begin{subfigure}[t]{0.28\textwidth}
    \centering
      \includegraphics[width=\linewidth]{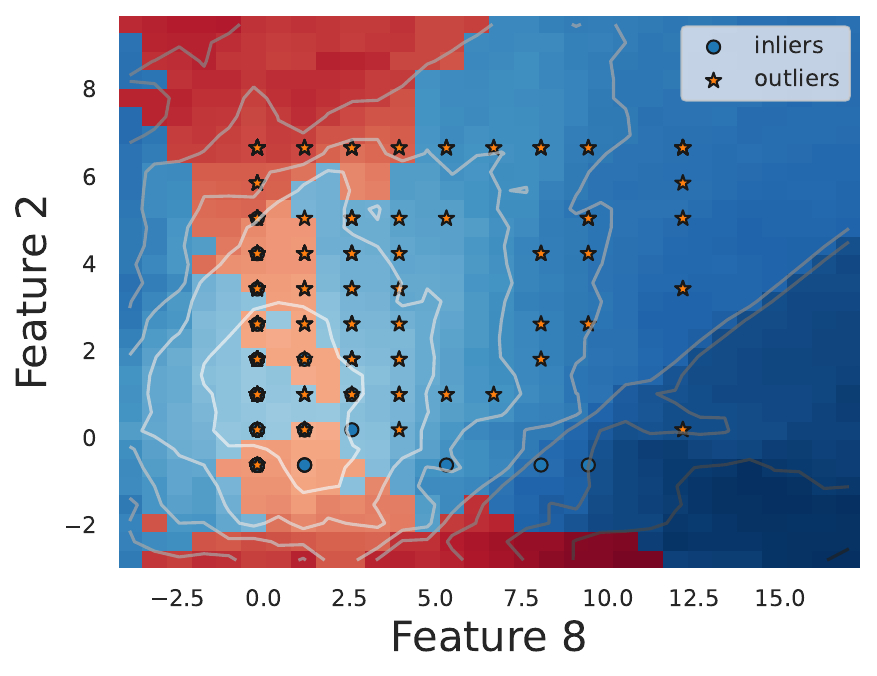}
      \caption{Scoremap {\ttfamily Breastw} Scenario II}
      \label{fig:Local-Breastw-split}
    \end{subfigure}\hfil % <-- added
\caption{Bar Plot, Score Plot and Scoremap for {\ttfamily Breastw}  in the two different Scenarios, using the \approach algorithm applied to the \EIFplus model.}\label{fig:interpretation-Breastw}
\end{figure}

\subsubsection{Feature Selection}

\ale{The series of plots contained in Figure \ref{fig:fs-interpretation-Breastw}  confirms the uncertainty in distributing the importance of different features in this particular set of data. In fact for all the interpretation algorithms evaluated there is not a significant difference in applying the Unsupervised Feature Selection proxy task in increasing (red line) or decreasing (blue line) order of feature relevance. Notably also the green line, representing a Feature Selection strategy in which a random feature is removed at each step, is almost overlapped to the other two meaning that there is not a single or a group of features with an importance significantly higher than the others. As a result, the quantitative measures of interpretability efficiency, represented by the $AUC_{FS}$ metric, are all approximately equal to zero. The trend of the Average Precision metric is roughly constant at perfect scores (i.e. close to 1) until the number of features composing the input space is reduced to 3 where the Average Precision starts to decrease its magnitude. The likely implication is that the model needs at least three features to maintain acceptable performances in detecting outliers. It is possible to conclude that the behavior depicted by plots below is very similar to the one observed for the {\ttfamily Bisect6D} synthetic dataset (Section \ref{sec:Bisect6D}), where the anomalies were distributed across all the features.}

\begin{figure}[!ht] 
\centering
\hspace{0.05\textwidth}\textbf{IF} \hspace{0.29\textwidth} \textbf{EIF} \hspace{0.29\textwidth} \textbf{EIF+}
% First row with vertical caption on the left
\begin{minipage}{\textwidth}
    \rotatebox{90}{\parbox{15mm}{\centering \textbf{Ad-Hoc}}} % Adjust the parbox width as necessary for your caption text
    \begin{minipage}{0.95\textwidth}
        \begin{subfigure}[t]{0.30\textwidth}
            \centering
            \includegraphics[trim={0 0 3.5cm 0}, clip, width=\linewidth]{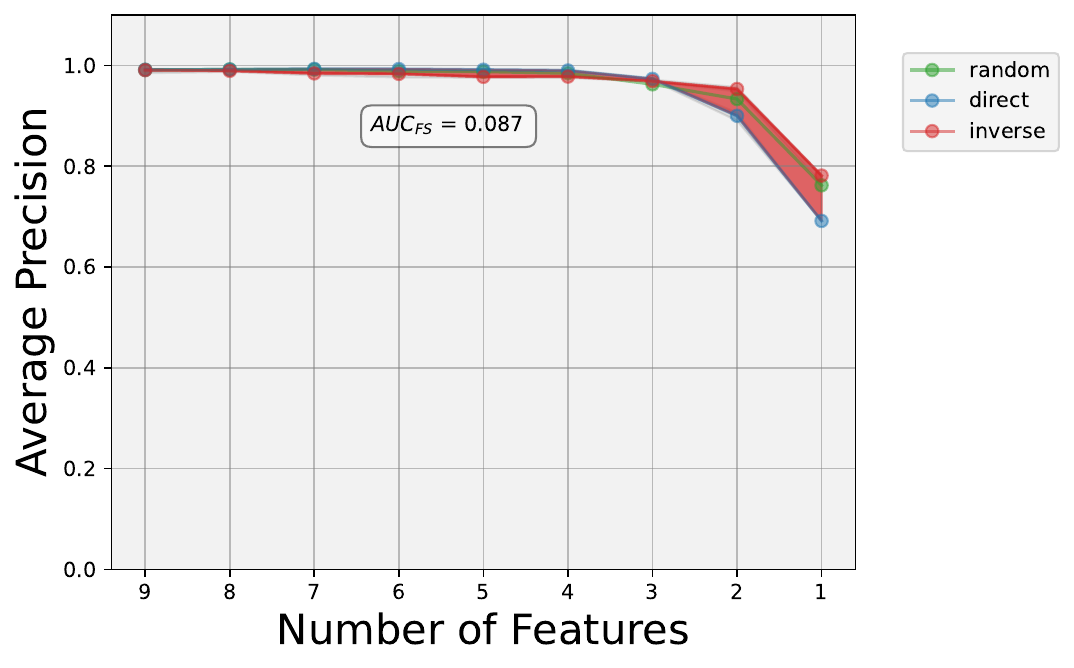}
            \caption{\approach applied to IF}
            \label{fig:Feat-Sel_Breastw_valEIF+_DIFFI_2}
        \end{subfigure}\hfill
        \begin{subfigure}[t]{0.30\textwidth}
            \centering
            \includegraphics[trim={0 0 3.5cm 0}, clip, width=\linewidth]{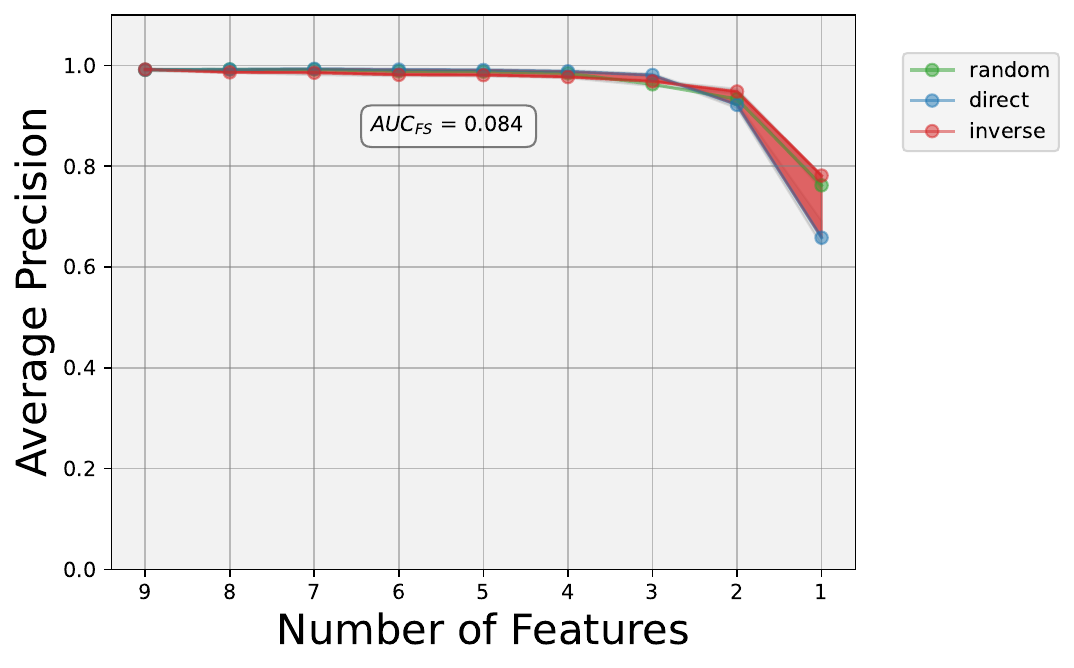}
            \caption{\approach applied to EIF}
            \label{fig:Feat-Sel_Breastw_valEIF+_EXIFFI_2}
        \end{subfigure}\hfill
        \begin{subfigure}[t]{0.30\textwidth}
            \centering
            \includegraphics[trim={0 0 3.5cm 0}, clip, width=\linewidth]{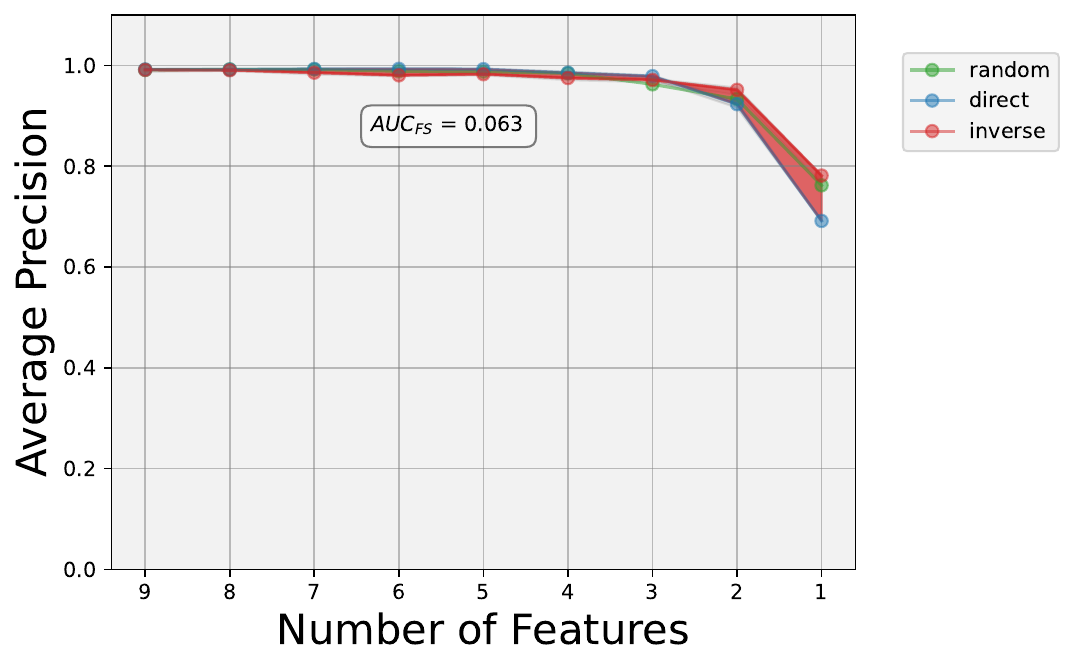}
            \caption{\approach applied to \EIFplus}
            \label{fig:Feat-Sel_Breastw_valEIF+_EXIFFI+_2}
        \end{subfigure}
    \end{minipage}
\end{minipage}

\vspace{5mm} % Space between rows

% Second row with vertical caption on the left
\begin{minipage}{\textwidth}
    \rotatebox{90}{\parbox{15mm}{\centering \textbf{Post-Hoc}}} % Adjust as necessary
    \begin{minipage}{0.95\textwidth}
        \begin{subfigure}[t]{0.30\textwidth}
            \centering
            \includegraphics[trim={0 0 3.5cm 0}, clip, width=\linewidth]{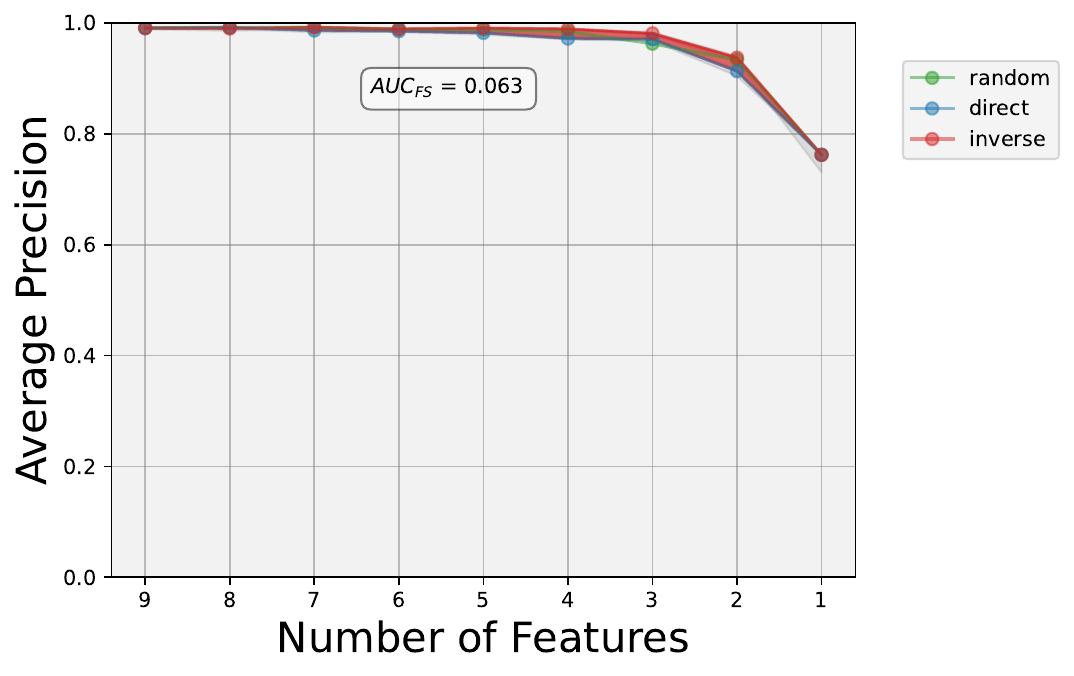}
            \caption{RandomForest fitted to IF}
            \label{fig:Feat-Sel_Breastw_valEIF+_IF_RandomForest_2}
        \end{subfigure}\hfill
        \begin{subfigure}[t]{0.30\textwidth}
            \centering
            \includegraphics[trim={0 0 3.5cm 0}, clip, width=\linewidth]{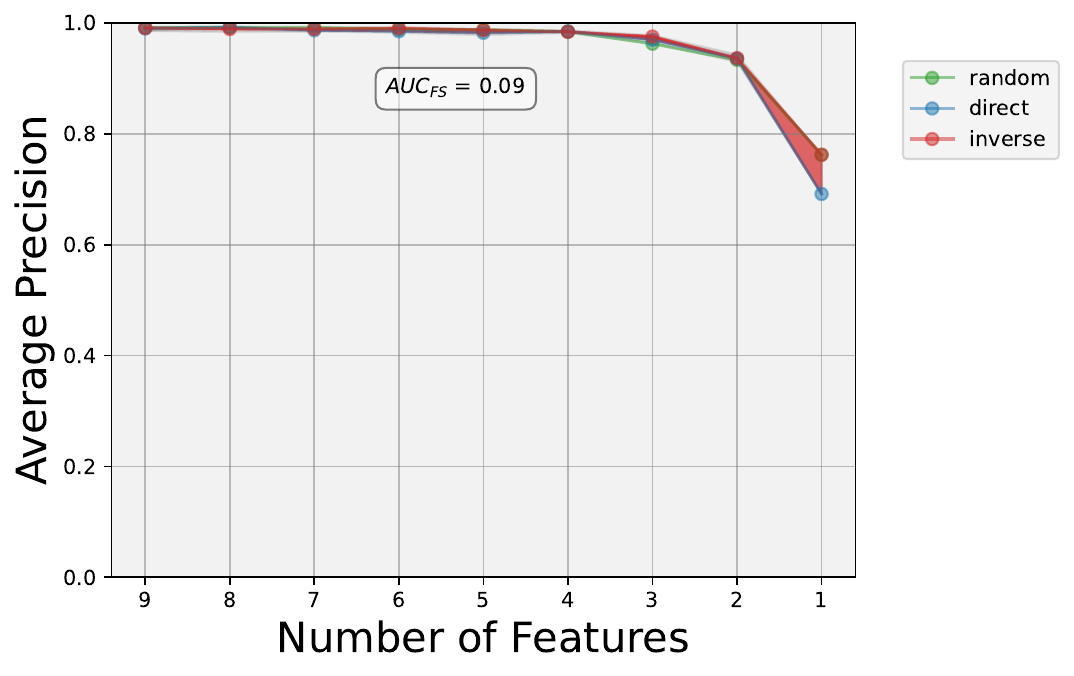}
            \caption{RandomForest fitted to EIF}
            \label{fig:Feat-Sel_Breastw_valEIF+_EIF_RandomForest_2}
        \end{subfigure}\hfill
        \begin{subfigure}[t]{0.30\textwidth}
            \centering
            \includegraphics[trim={0 0 3.5cm 0}, clip, width=\linewidth]{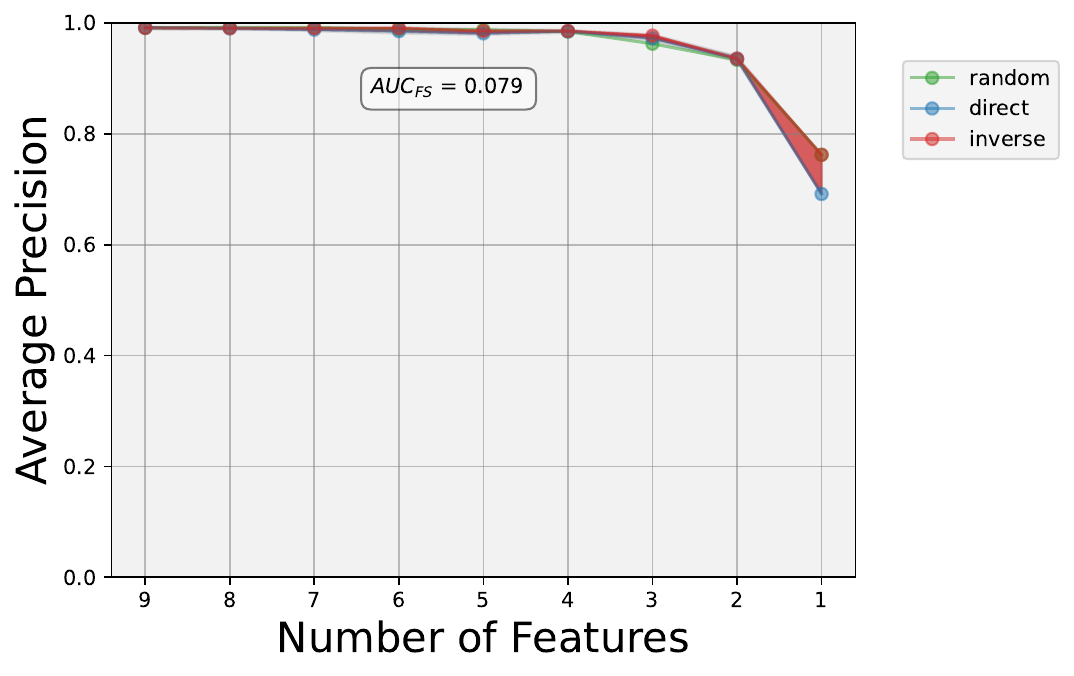}
            \caption{RandomForest fitted to \EIFplus}
            \label{fig:Feat-Sel_Breastw_valEIF+_EIF+_RandomForest_2}
        \end{subfigure}
    \end{minipage}
\end{minipage}

\caption{Feature Selection of the different Ad-Hoc and Post-Hoc methods applied to the 3 Isolation Forest models: IF, EIF and \EIFplus. The blue line is the values of average precision, calculated with the \EIFplus model in the Scenario II, dropping the most important feature at each step, the red line is the values of average precision dropping the least important feature at each step and the green line is the value of the feature selection dropping a random feature at each step.}\label{fig:fs-interpretation-Breastw}
\end{figure}

\ale{As already discussed in previous sections, in the {\ttfamily Breastw} dataset the relevance is evenly shared across most of the features and consequently there it not possible to identify an interpretation method that achieves a better explanation than the others. We can indeed consider the slight differences in the $AUC_{FS}$ values grouped in Table \ref{tab:fs-tab-Breastw} as a result of the stochasticity inherently present in the attribution of importance scores. Finally it is important to note how the interpretations obtained with the proposed approach \approach are an order of magnitude faster with the respect to post-hoc RandomForest based interpretations, making \approach certainly more appealing to be exploited in a practical application.}

\subsection*{{\ttfamily Cardio}}

\subsubsection{Performance}

\ale{The plot contained in Figure \ref{fig:Cardio_contamination_full} illustrates how the gradual addition of outliers in the training set affects the Average Precision values achieved by various AD models on the {\ttfamily Cardio} dataset. The trend is similar across all the datasets and the difference between the metrics values across the models are minor: passing from 0 to 10 \% of contamination the Average Precision is associated with a decrease of about 3 percentage points. A focus on the proposed method, \EIFplus, and its counterpart,  EIF, is proposed in Figure \ref{fig:Cardio_contaminationEIFvsEIF+} and it shows how\EIFplus starts from higher values for low contamination levels and it is overcomed by EIF as the number of anomalies included in the fitting stage raises. The following behavior aligns with the expectations associated to the inherent structure of these two algorithms, in fact \EIFplus is optimized in settings where there is a lack of anomalous points in the training set.}

\begin{figure}[!ht] 
    \centering % <-- added
    \begin{subfigure}[t]{0.49\textwidth}
      \includegraphics[width=\linewidth]{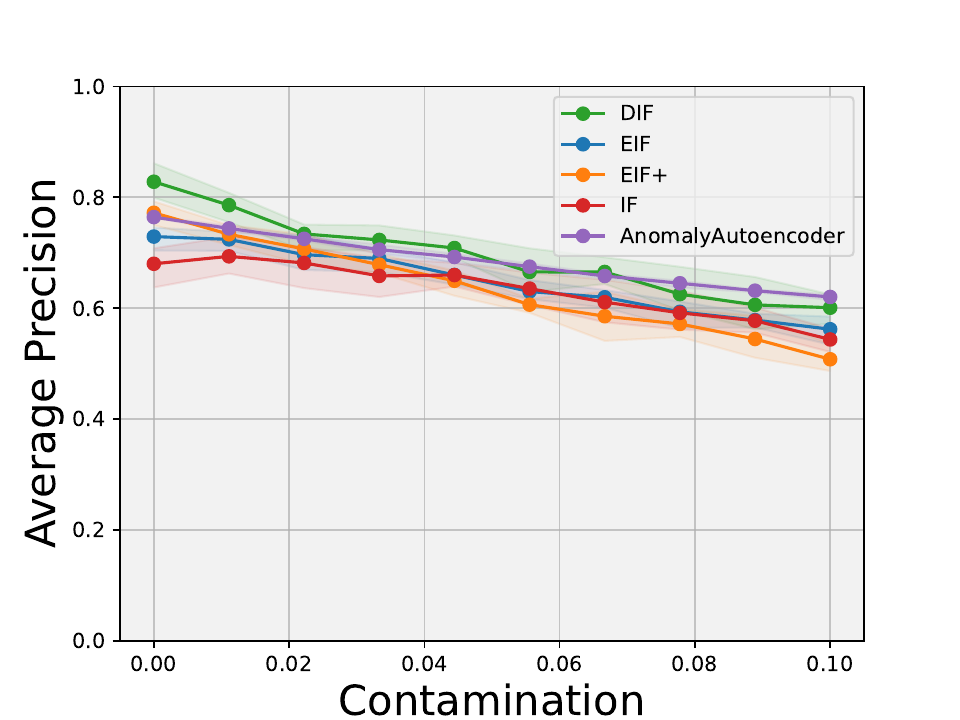}
      \caption{Models evaluation, varying the contamination levels}
      \label{fig:Cardio_contamination_full}
    \end{subfigure}\hfil % <-- added
    \begin{subfigure}[t]{0.44\textwidth}
      \includegraphics[width=\linewidth]{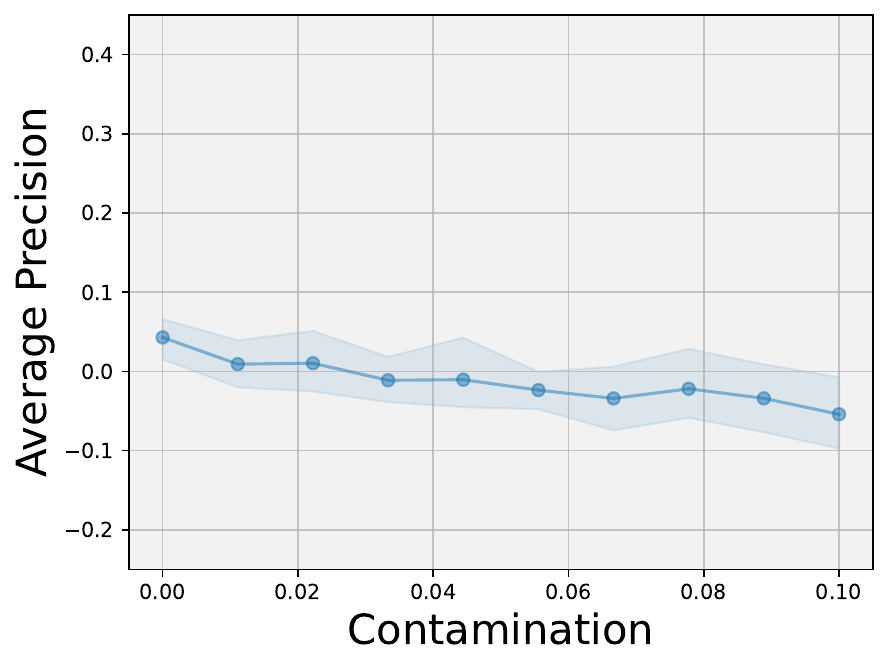}
      \caption{Difference between \EIFplus and EIF average precision}
      \label{fig:Cardio_contaminationEIFvsEIF+}
    \end{subfigure}\hfil % <-- added
\caption{Figure \ref{fig:Cardio_contamination_full} illustrates the average precision as the contamination level in the training set increases. Figure \ref{fig:Cardio_contaminationEIFvsEIF+} compares the performance graphs of EIF and \EIFplus, using the difference of their scores in various contamination levels.}
\label{fig:Cardio_contamination}
\end{figure}

\ale{In Table \ref{tab:Cardio_perf}  the AD models are evaluated through some well-known classification metrics in Scenario I and Scenario II. The decreasing trend described in Figure \ref{fig:Cardio_contamination_full} is reflected here not only on the Average Precision metrics but also on Precision and ROC AUC score. From an overall analysis of the metrics the DIF model appears as the one with the highest values of Average Precision but at the same time it is affected by notably elevated fit and prediction times. On the other hand, acceptable metric values and execution times are showed by EIF and \EIFplus making them more appropiate models for this task.}

\begin{table}[htbp]
\begin{minipage}[t]{0.46\textwidth}
\strut\vspace*{-\baselineskip}\newline
\resizebox{\textwidth}{!}{
\begin{tabular}{|c||ccc|ccc||cc|}
\toprule
\hline
&\multicolumn{3}{c|}{Scenario I}&\multicolumn{3}{c||}{Scenario II}&\multicolumn{2}{c|}{Time}\\
\hline
AD Model & Avg & Prec & ROC & Avg & Prec & ROC & fit & pred \\
& Prec &  & AUC & Prec &  & AUC &  &  \\
\hline
IF          & 0.53& 0.44& 0.69& 0.68& 0.60& 0.78& \textbf{0.12}& 0.014\\
EIF         & 0.55& 0.59& 0.77& 0.74& 0.72& 0.84& 0.16& \textbf{0.001}\\
EIF+        & 0.50& 0.52& 0.73& 0.76& \textbf{0.73}& \textbf{0.85}& 0.133& 0.05\\
DIF         & 0.58& 0.52& 0.73& \textbf{0.79}& 0.70& 0.83& 2.81& 2.28\\
AE & \textbf{0.62}& \textbf{0.62}& \textbf{0.79}& 0.83& 0.70& 0.76& 6.1& 0.104\\
\hline
\end{tabular}}
\vspace{0.41cm}
\caption{Performances of 5 different Anomaly Detection models over {\ttfamily Cardio} are compared using classical Classification metrics. Moreover, the last two columns contain the average time for a fit and predict operation. The highest metric values and the lowest execution times are highlighted in bold}\label{tab:Cardio_perf}
\end{minipage}
\hfill
\begin{minipage}[t]{0.46\textwidth}
\strut\vspace*{-\baselineskip}\newline
\resizebox{\textwidth}{!}{
\begin{tabular}{|c||c|c|c|c||c|}
\toprule
\hline
&\multicolumn{2}{c|}{Evaluation with EIF}&\multicolumn{2}{c||}{Evaluation with \EIFplus}&\\
\hline
& Scenario I & Scenario II & Scenario I & Scenario II & Time\\

 Algorithm & $AUC_{FS}$  & $AUC_{FS}$ & $AUC_{FS}$  & $AUC_{FS}$ &  \\
\hline
DIFFI                & 4.653& 4.768& 4.398& 4.333& 0.57 \\
IF\_\approach         & 1.933& 3.496& 2.4& 3.433& 0.36\\
EIF\_\approach        & \textbf{5.417}& 8.286& \textbf{5.122}& 8.381& \textbf{0.34}\\
\EIFplus\_\approach   & 4.421& \textbf{8.609}& 4.252& \textbf{8.730}& \textbf{0.30}\\
IF\_RF               & 1.483& 7.696& 1.282& 7.889& 1.80\\
EIF\_RF              & 1.358& 7.781& 1.353& 7.855& 1.80\\
EIF+\_RF             & 0.320& 8.241& 0.360& 8.302& 1.80\\
\hline
\end{tabular}}
\caption{Quantitative evaluation of the effectiveness of 6 different interpretation algorithms on {\ttfamily Cardio} through the $AUC_{FS}$ metric, introduced in \ref{sec:interpr_evaluat}. In the last column the average time taken by the different models to produce the importance scores is reported. The highest $AUC_{FS}$ and lowest Importance time values are highlighted in bold.}\label{tab:fs-tab-Cardio}
\end{minipage}
\end{table}

\subsubsection{Importance Plots}

\ale{Figure \ref{fig:interpretation-Cardio} exploits the Bar Plot, Score Plot and Local Scoremaps to compare the different explanations provided by \approach+ in Scenario I and Scenario II. In both training strategies Feature 6 and Feature 2 stand out as two of the most relevant features to distinguish between a normal and a pathological condition in a Cardiotogram, as explained in Appendix \ref{sec:appendix-real-world-data}. The Local Scoremaps (Figure \ref{fig:Local-Cardio} and \ref{fig:Local-Cardio-split}) provide a visual aid on how anomalies (represented by red stars) are indeed scattered along the directions identified by the previously cited attributes.}

\begin{figure}[!ht] 
    \centering % <-- added
    \begin{subfigure}[t]{0.38\textwidth}
    \centering
      \includegraphics[width=\linewidth]{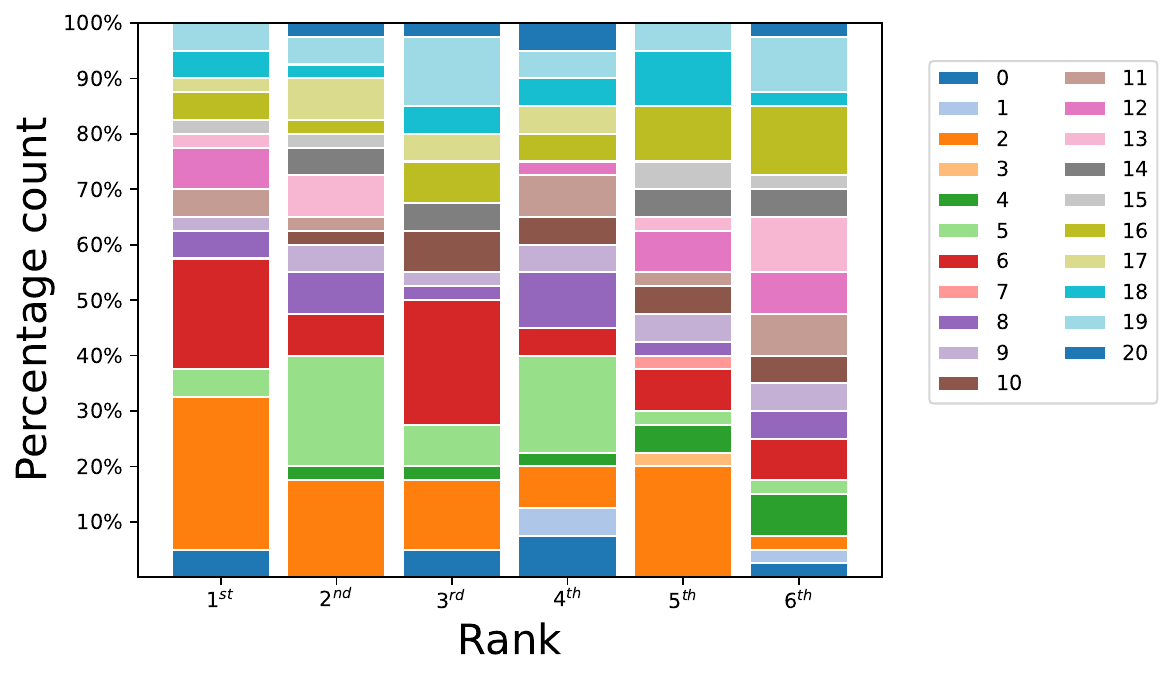}
      \caption{Bar Plot {\ttfamily Cardio} Scenario I}
      \label{fig:GFI-Cardio}
    \end{subfigure}\hfil % <-- added
    \begin{subfigure}[t]{0.27\textwidth}
    \centering
      \includegraphics[width=\linewidth]{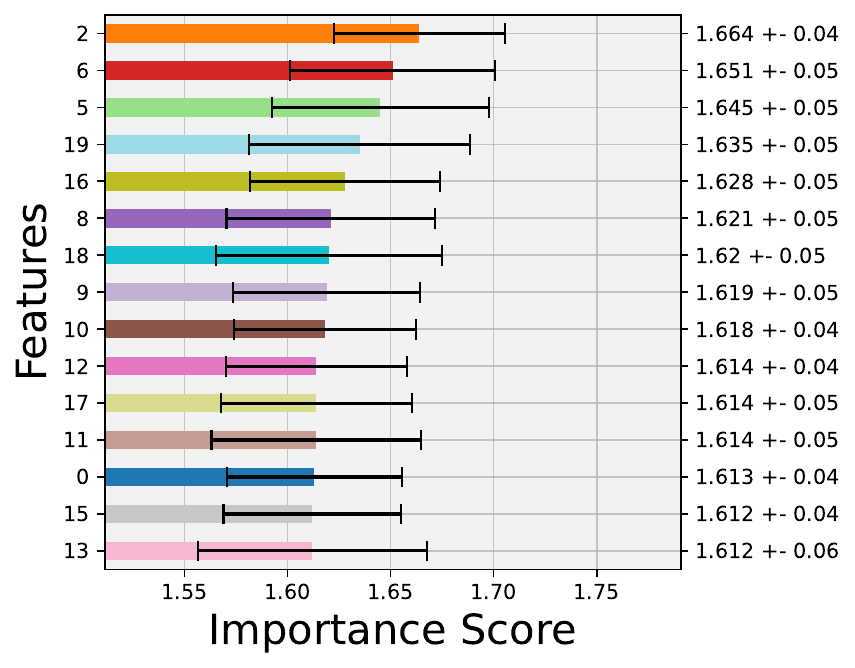}
      \caption{Score Plot {\ttfamily Cardio} Scenario I}
      \label{fig:Feat-imp-Cardio}
    \end{subfigure}\hfil % <-- added
    \begin{subfigure}[t]{0.28\textwidth}
    \centering
      \includegraphics[width=\linewidth]{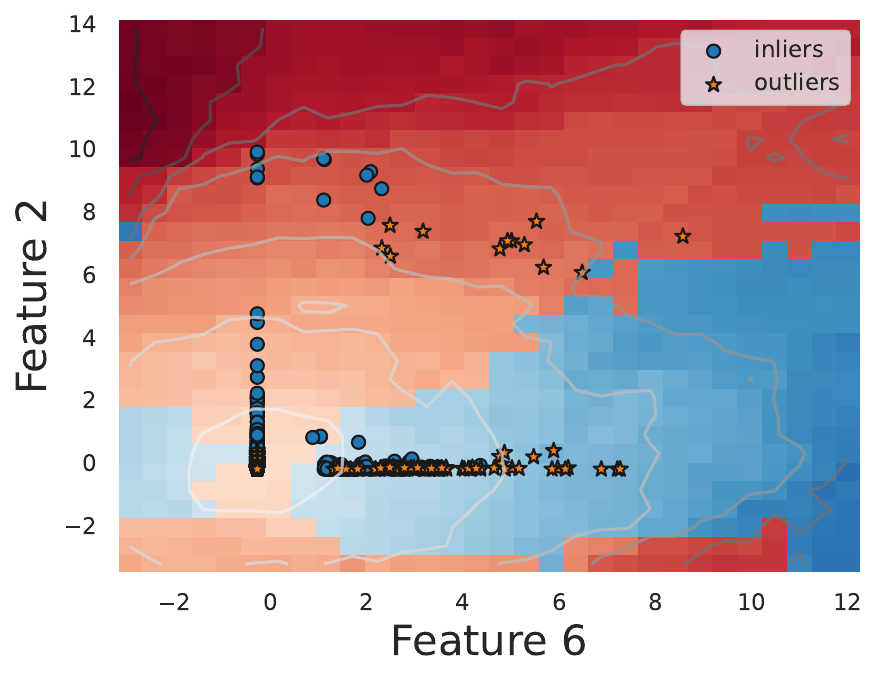}
      \caption{Scoremap {\ttfamily Cardio} Scenario I}
      \label{fig:Local-Cardio}
    \end{subfigure}\hfil % <-- added
    \begin{subfigure}[t]{0.38\textwidth}
    \centering
      \includegraphics[width=\linewidth]{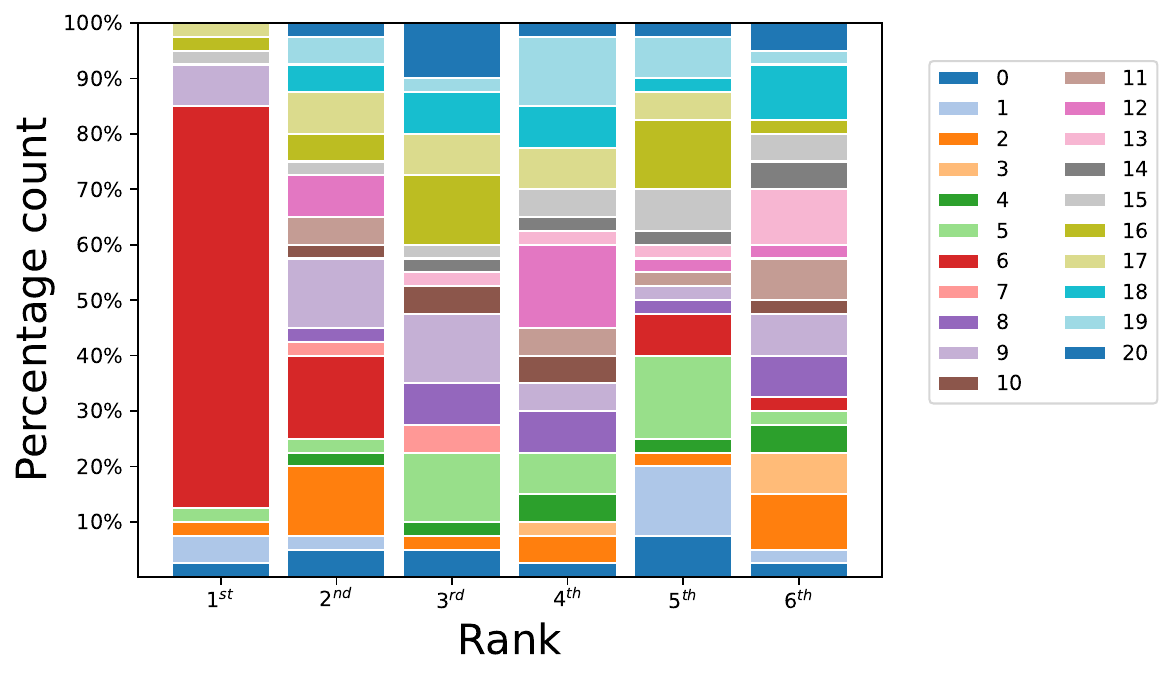}
      \caption{Bar Plot {\ttfamily Cardio} Scenario II}
      \label{fig:GFI-Cardio-split}
    \end{subfigure}\hfil % <-- added
    \begin{subfigure}[t]{0.27\textwidth}
    \centering
      \includegraphics[width=\linewidth]{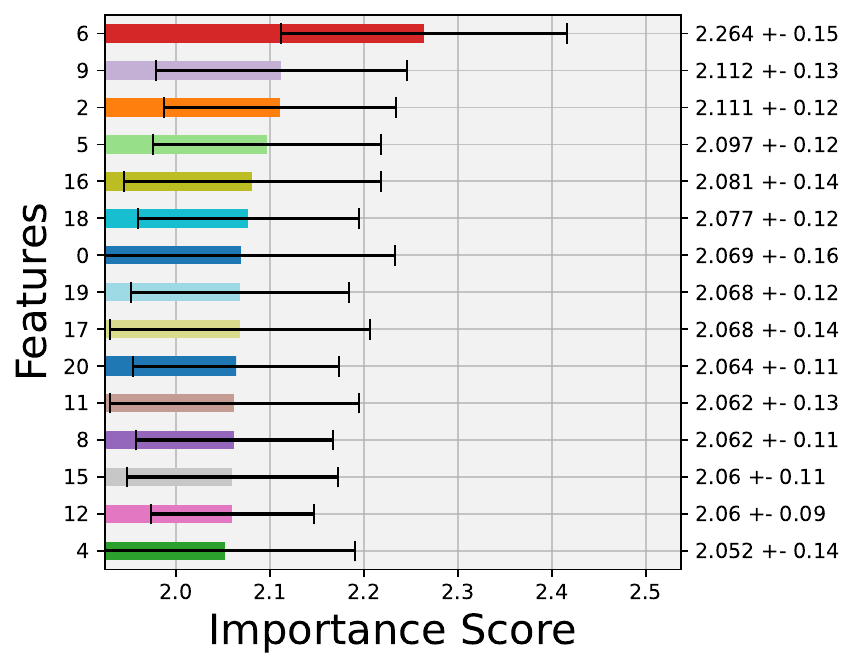}
      \caption{Score Plot {\ttfamily Cardio} Scenario II}
      \label{fig:Feat-imp-Cardio-split}
    \end{subfigure}\hfil % <-- added
    \begin{subfigure}[t]{0.28\textwidth}
    \centering
      \includegraphics[width=\linewidth]{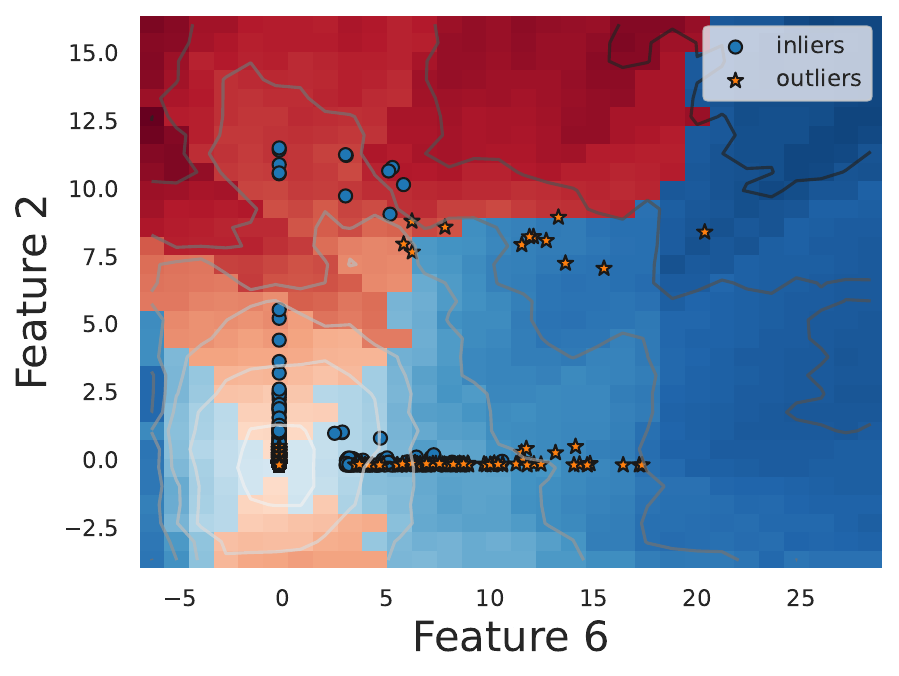}
      \caption{Scoremap {\ttfamily Cardio} Scenario II}
      \label{fig:Local-Cardio-split}
    \end{subfigure}\hfil % <-- added
\caption{Bar Plot, Score Plot and Scoremap for {\ttfamily Cardio} in the two different Scenarios, using the \approach algorithm applied to the \EIFplus model.}\label{fig:interpretation-Cardio}
\end{figure}

\subsubsection{Feature Selection}

\ale{The Feature Selection plots portrayed in Figure \ref{fig:fs-interpretation-Cardio} represents a clear marker in support of the superiority of the proposed interpretation algorithms \approach and \approach+. As a matter of fact the plots related to the methods just mentioned, contained in Figure \ref{fig:Feat-Sel_Cardio_valEIF+_EXIFFI_2} and \ref{fig:Feat-Sel_Cardio_valEIF+_EXIFFI+_2}, present a symmetric shape. This is the ideal shape we expected to achieve when this kind of plot for the performance evaluation and comparison of interpretation models was firstly designed. In fact, this shape proves that the model is able to correctly rank all the features according to its importance scores. This happens because as features are removed in increasing order of relevance (red line) the Average Precision displays a constantly increasing trend while a constantly decreasing one can be observed as the most important attributes are progressively excluded from the feature space.}
\begin{figure}[!ht] 
\centering
\hspace{0.05\textwidth}\textbf{IF} \hspace{0.29\textwidth} \textbf{EIF} \hspace{0.29\textwidth} \textbf{EIF+}
% First row with vertical caption on the left
\begin{minipage}{\textwidth}
    \rotatebox{90}{\parbox{15mm}{\centering \textbf{Ad-Hoc}}} % Adjust the parbox width as necessary for your caption text
    \begin{minipage}{0.95\textwidth}
        \begin{subfigure}[t]{0.30\textwidth}
            \centering
            \includegraphics[trim={0 0 3.5cm 0}, clip, width=\linewidth]{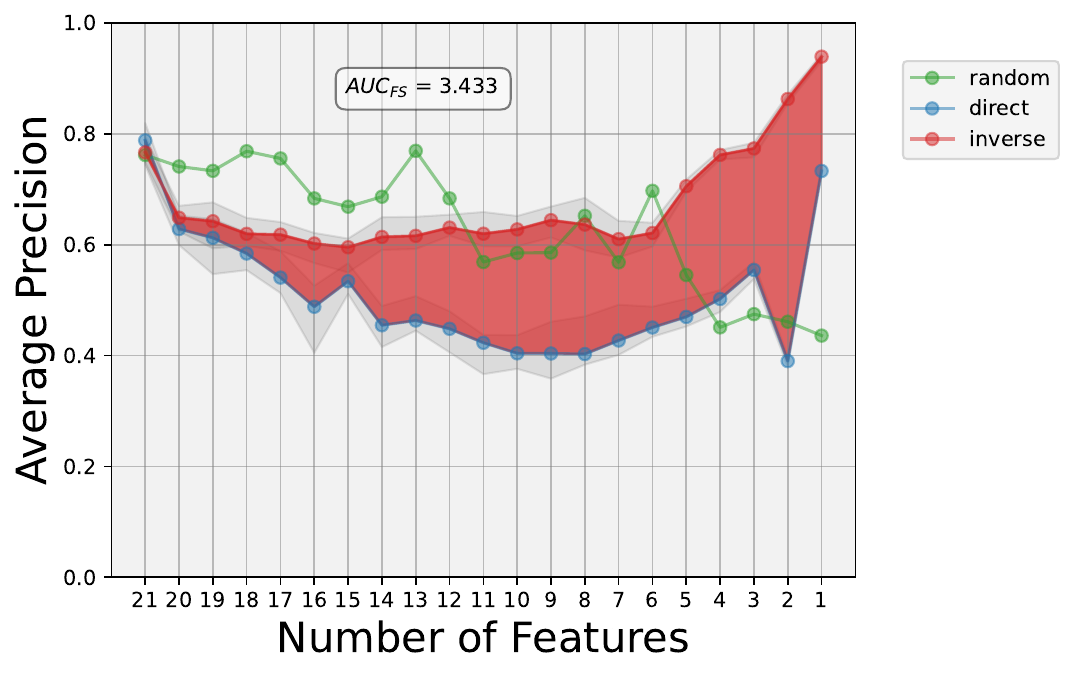}
            \caption{\approach applied to IF}
            \label{fig:Feat-Sel_Cardio_valEIF+_DIFFI_2}
        \end{subfigure}\hfill
        \begin{subfigure}[t]{0.30\textwidth}
            \centering
            \includegraphics[trim={0 0 3.5cm 0}, clip, width=\linewidth]{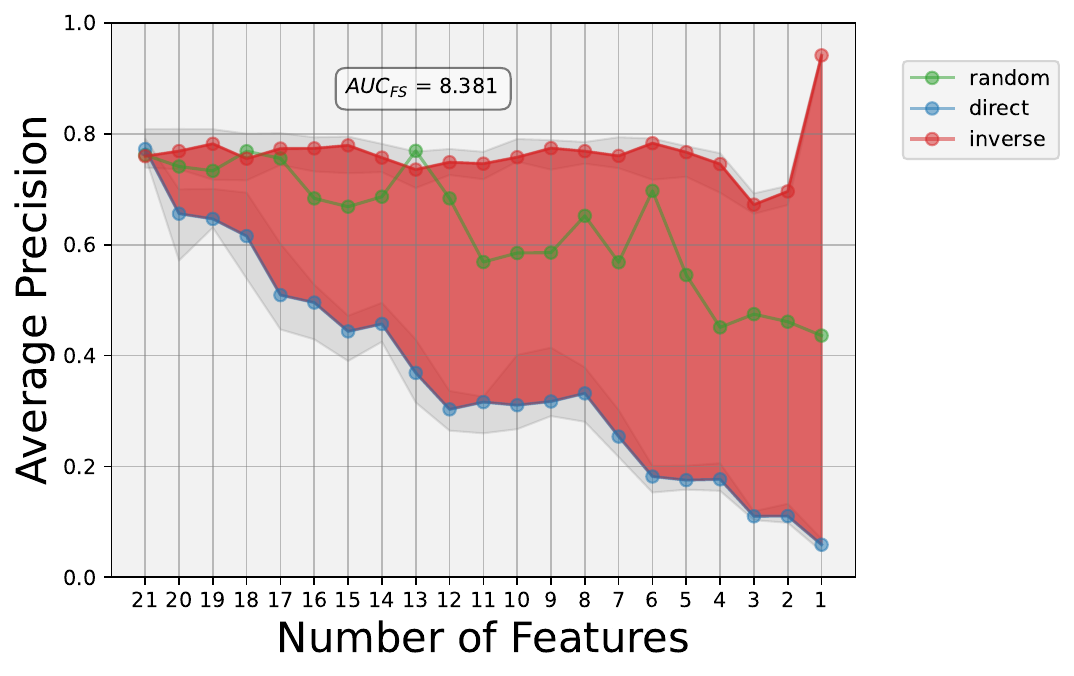}
            \caption{\approach applied to EIF}
            \label{fig:Feat-Sel_Cardio_valEIF+_EXIFFI_2}
        \end{subfigure}\hfill
        \begin{subfigure}[t]{0.30\textwidth}
            \centering
            \includegraphics[trim={0 0 3.5cm 0}, clip, width=\linewidth]{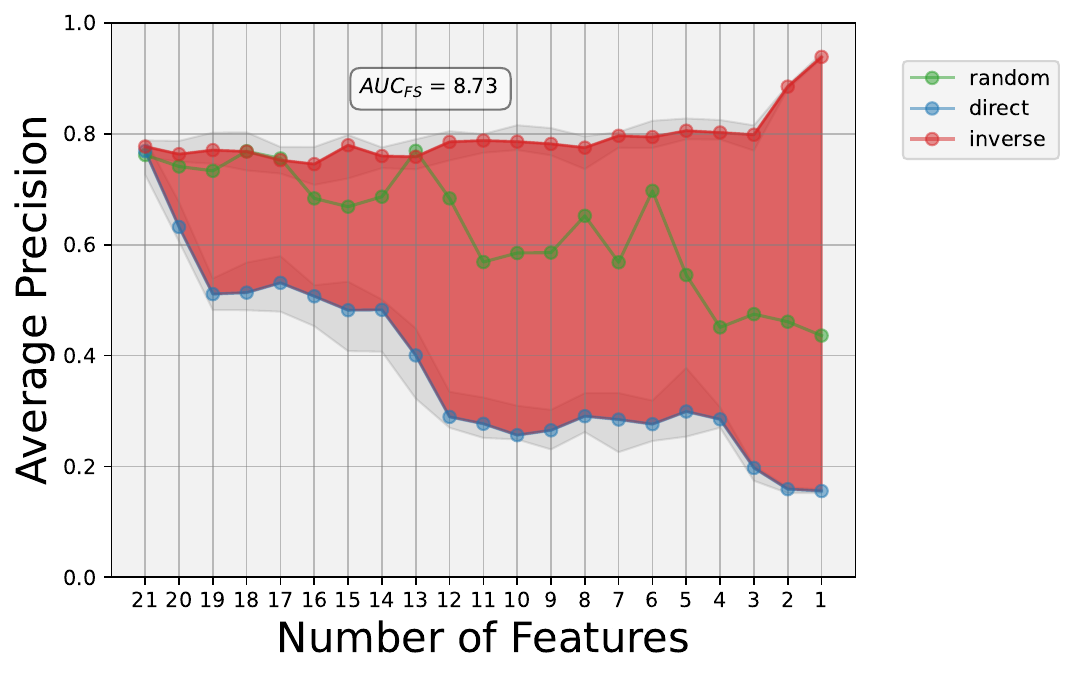}
            \caption{\approach applied to \EIFplus}
            \label{fig:Feat-Sel_Cardio_valEIF+_EXIFFI+_2}
        \end{subfigure}
    \end{minipage}
\end{minipage}

\vspace{5mm} % Space between rows

% Second row with vertical caption on the left
\begin{minipage}{\textwidth}
    \rotatebox{90}{\parbox{15mm}{\centering \textbf{Post-Hoc}}} % Adjust as necessary
    \begin{minipage}{0.95\textwidth}
        \begin{subfigure}[t]{0.30\textwidth}
            \centering
            \includegraphics[trim={0 0 3.5cm 0}, clip, width=\linewidth]{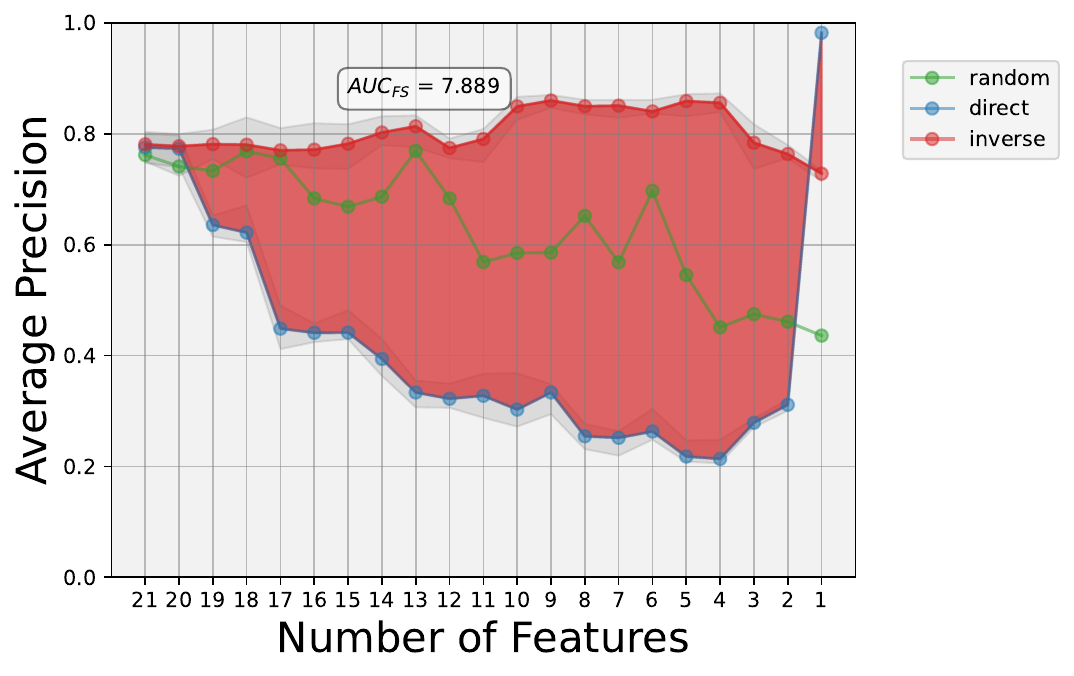}
            \caption{RandomForest fitted to IF}
            \label{fig:Feat-Sel_Cardio_valEIF+_IF_RandomForest_2}
        \end{subfigure}\hfill
        \begin{subfigure}[t]{0.30\textwidth}
            \centering
            \includegraphics[trim={0 0 3.5cm 0}, clip, width=\linewidth]{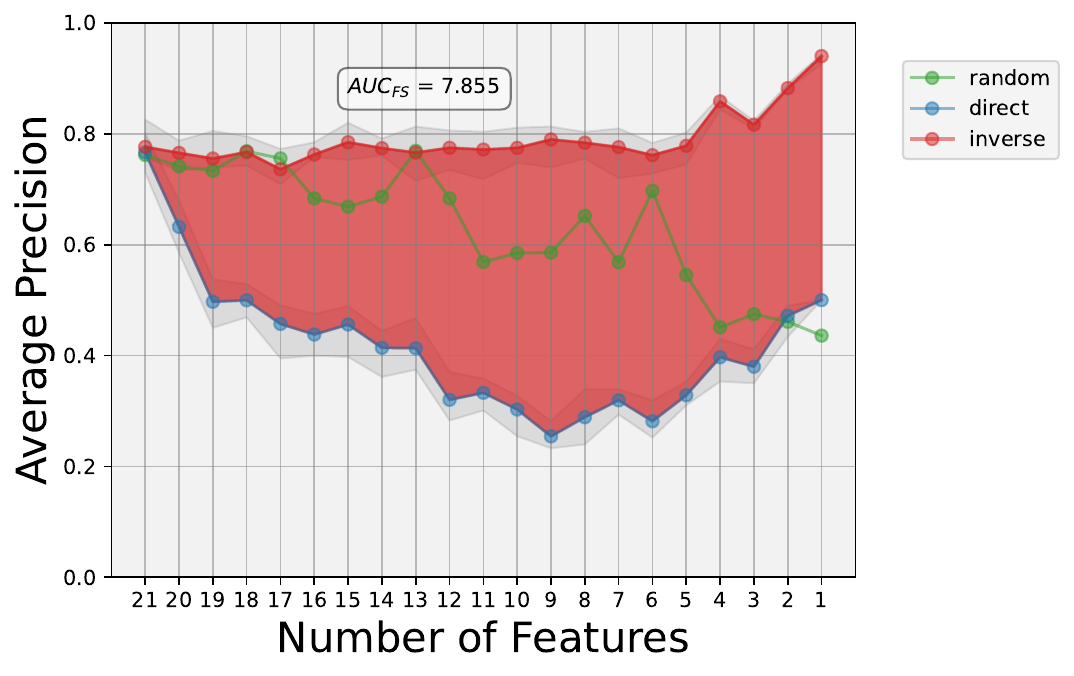}
            \caption{RandomForest fitted to EIF}
            \label{fig:Feat-Sel_Cardio_valEIF+_EIF_RandomForest_2}
        \end{subfigure}\hfill
        \begin{subfigure}[t]{0.30\textwidth}
            \centering
            \includegraphics[trim={0 0 3.5cm 0}, clip, width=\linewidth]{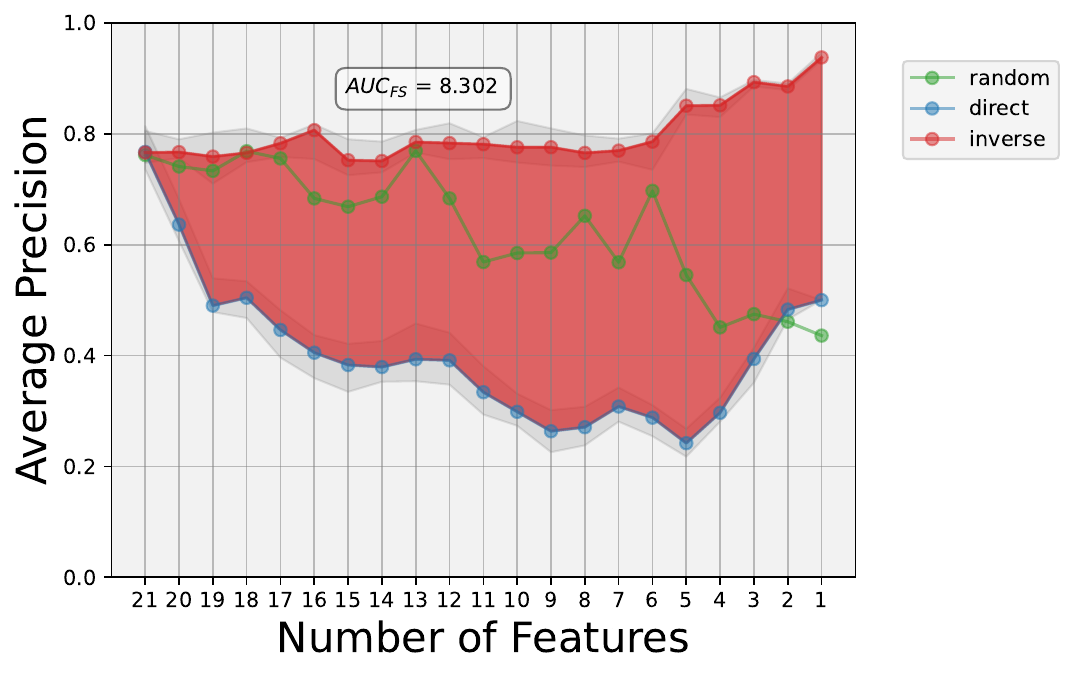}
            \caption{RandomForest fitted to \EIFplus}
            \label{fig:Feat-Sel_Cardio_valEIF+_EIF+_RandomForest_2}
        \end{subfigure}
    \end{minipage}
\end{minipage}

\caption{Feature Selection of the different Ad-Hoc and Post-Hoc methods applied to the 3 Isolation Forest models: IF, EIF and \EIFplus. The blue line is the values of average precision, calculated with the \EIFplus model in the Scenario II, dropping the most important feature at each step, the red line is the values of average precision dropping the least important feature at each step and the green line is the value of the feature selection dropping a random feature at each step.}\label{fig:fs-interpretation-Cardio}
\end{figure}

\ale{The direct consequence of the optimal behavior of \approach and \approach+ is certified in Table \ref{tab:fs-tab-Cardio} where these two models display the highest $AUC_{FS}$ values, weather they are evaluated with EIF or \EIFplus. The metric values obtained by \approach applied on IF and post-hoc interpretation based on Random Forest are instead inferior because, as it can be observed in Figures, the increasing trend of the red line is not perfectly mirrored by the blue one that displays a oscillating behavior. To conclude, another point in favour to the proposed approaches is the time taken to obtain the importance scores which is substantially reduced with the respect to the ones of the other models considered.}

\subsection*{{\ttfamily Diabetes}}

\subsubsection{Performance}

\ale{The peculiarity of the {\ttfamily Diabetes} dataset, as described in \ref{sec:appendix-real-world-data}, in the context of this study is its low dimensionality: its observations are, in fact, fully described using just four features. As a consequence the behavior of the AD models considered as abnormal samples are progressively included in the training set, displayed in Figure \ref{fig:Diabetes_contamination_full}, is diverse from the ones observed in other benchmark datasets. In particular the IF model possesses an unique increasing Average Precision trend that saturates at a contamination level around 5 \%. On the other hand the DIF model showcases an essentially constant trend at substantially low Average Precision values if compared to the other methods. An explanation of the underperformance of this model could be the presence of overfitting because of the usage of an highly complex approach from a simple task as the ones of separating anomalous points from normal ones on a four dimensional feature space. Finally, the proposed \EIFplus model stands out as the reference model in this study, immediately followed by EIF as highlighted in Figure \ref{fig:Diabetes_contaminationEIFvsEIF+}.} 

\begin{figure}[!ht] 
    \centering % <-- added
    \begin{subfigure}[t]{0.49\textwidth}
      \includegraphics[width=\linewidth]{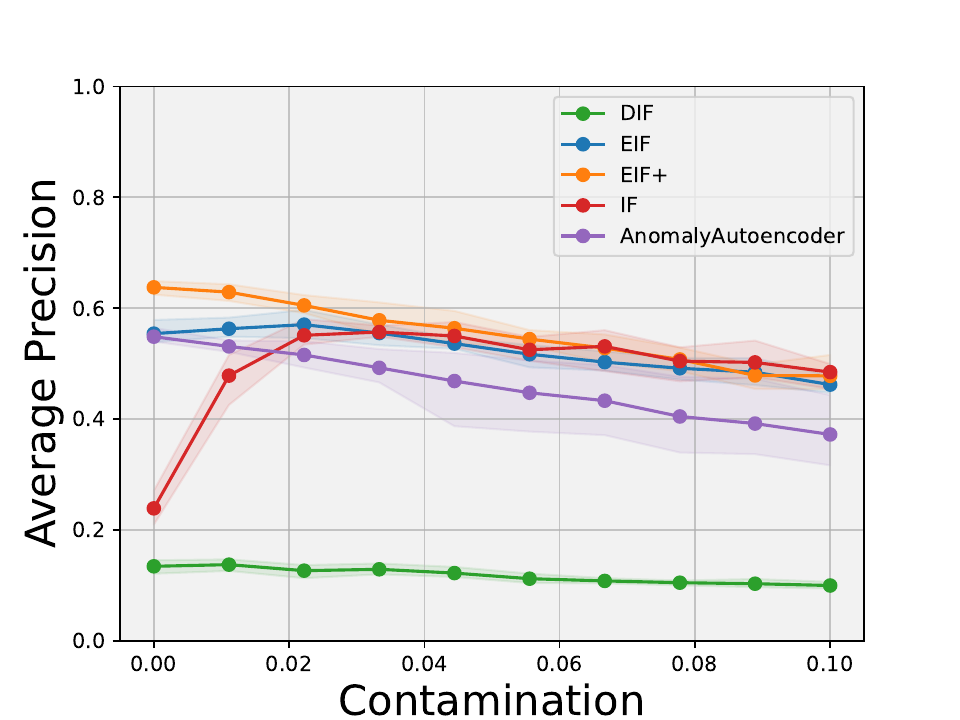}
      \caption{Models evaluation, varying the contamination levels}
      \label{fig:Diabetes_contamination_full}
    \end{subfigure}\hfil % <-- added
    \begin{subfigure}[t]{0.44\textwidth}
      \includegraphics[width=\linewidth]{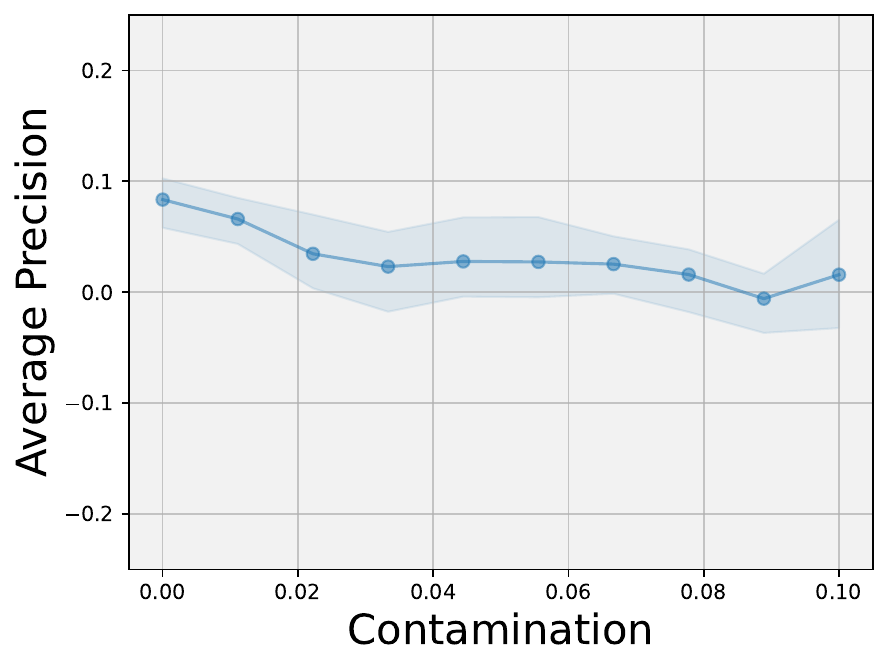}
      \caption{Difference between \EIFplus and EIF average precision}
      \label{fig:Diabetes_contaminationEIFvsEIF+}
    \end{subfigure}\hfil % <-- added
\caption{Figure \ref{fig:Diabetes_contamination_full} illustrates the average precision as the contamination level in the training set increases. Figure \ref{fig:Diabetes_contaminationEIFvsEIF+} compares the performance graphs of EIF and \EIFplus, using the difference of their scores in various contamination levels.}
\label{fig:Diabetes_contamination}
\end{figure}

\ale{Table \ref{tab:Diabetes_perf}  portraits the difference, in terms of the Average Precision, Precision and AUC ROC score metrics, in the two approaches used to train, and successively test, the presented Anomaly Detection approaches: Scenario I and Scenario II. As already made clear in Figure \ref{fig:Diabetes_contamination_full} there are some visible differences in the model performances as anomalies are included in the training process (i.e. in the passage from Scenario II to Scenario I). The most optimal model is the proposed \EIFplus due to its superior metric values and its unparalleled efficiency in both the fitting and prediction stages.}

\begin{table}[htbp]
\begin{minipage}[t]{0.46\textwidth}
\strut\vspace*{-\baselineskip}\newline
\resizebox{\textwidth}{!}{
\begin{tabular}{|c||ccc|ccc||cc|}
\toprule
\hline
&\multicolumn{3}{c|}{Scenario I}&\multicolumn{3}{c||}{Scenario II}&\multicolumn{2}{c|}{Time}\\
\hline
AD Model & Avg & Prec & ROC & Avg & Prec & ROC & fit & pred \\
& Prec &  & AUC & Prec &  & AUC &  &  \\
\hline
IF          & 0.46& 0.46& 0.70& 0.26& 0.31& 0.62& 0.13& 0.069\\
EIF         & \textbf{0.47}& 0.48& 0.71& 0.55& 0.61& 0.78& \textbf{0.10}& \textbf{0.008}\\
EIF+        & 0.44& \textbf{0.49}& \textbf{0.72}& \textbf{0.61}& \textbf{0.56}& \textbf{0.76}& \textbf{0.10}& \textbf{0.008}\\
DIF         & 0.10& 0.90& 0.49& 0.13& 0.17& 0.54& 10.2& 9.05\\
AE          & 0.45& 0.47& 0.70& 0.50& 0.52& 0.73& 17.82& 0.28\\
\hline
\end{tabular}}
\vspace{0.41cm}
\caption{Performances of 5 different Anomaly Detection models over {\ttfamily Diabetes} are compared using classical Classification metrics. Moreover, the last two columns contain the average time for a fit and predict operation. The highest metric values and the lowest execution times are highlighted in bold}\label{tab:Diabetes_perf}
\end{minipage}
\hfill
\begin{minipage}[t]{0.46\textwidth}
\strut\vspace*{-\baselineskip}\newline
\resizebox{\textwidth}{!}{
\begin{tabular}{|c||c|c|c|c||c|}
\toprule
\hline
&\multicolumn{2}{c|}{Evaluation with EIF}&\multicolumn{2}{c||}{Evaluation with \EIFplus}&\\
\hline
& Scenario I & Scenario II & Scenario I & Scenario II& Time\\

 Algorithm & $AUC_{FS}$  & $AUC_{FS}$ & $AUC_{FS}$  & $AUC_{FS}$ &  \\
\hline
DIFFI               & -0.363& -1.455& -0.345& -1.481& 0.63\\
IF\_\approach        & 0.847& -1.013& 0.812& -0.930& 0.73\\
EIF\_\approach       & 0.967& 0.354& \textbf{0.826}& 0.313& \textbf{0.50}\\
\EIFplus\_\approach  & \textbf{1.058}& \textbf{0.822}& 0.747& \textbf{1.171}& 0.52\\
IF\_RF              & -0.303& -0.059& -0.302& -0.123& 2.04\\
EIF\_RF             & 0.491& 0.315& 0.383& 0.355& 2.04\\
EIF+\_RF            & 0.463& 0.332& 0.407& 0.296& 2.04\\
\hline
\end{tabular}}
\caption{Quantitative evaluation of the effectiveness of 6 different interpretation algorithms on {\ttfamily Diabetes} through the $AUC_{FS}$ metric, introduced in \ref{sec:interpr_evaluat}. In the last column the average time taken by the different models to produce the importance scores is reported. The highest $AUC_{FS}$ and lowest Importance time values are highlighted in bold.}\label{tab:fs-tab-Diabetes}
\end{minipage}
\end{table}

\subsubsection{Importance Plots}

\ale{The outcomes of the explanations granted by \approach+ are illustrated in Figure \ref{fig:interpretation-Diabetes}. Analyzing the Score Plots, represented in Figures \ref{fig:Feat-imp-Diabetes} and \ref{fig:Feat-imp-Diabetes-split} and the Bar Plots, represented in Figures \ref{fig:GFI-Diabetes} and \ref{fig:GFI-Diabetes-split}, it is clear how the two most important features are  {\itshape HbA1c\_level} and  {\itshape blood\_glucose\_level}. As elucidated in \ref{sec:appendix-real-world-data} the Hemoglobin A1c Level and the amount of glucose in the bloodstream represent crucial indicators to discriminate between patients affected or not by diabetes.}

\begin{figure}[!ht] 
    \centering % <-- added
    \begin{subfigure}[t]{0.33\textwidth}
    \centering
      \includegraphics[width=\linewidth]{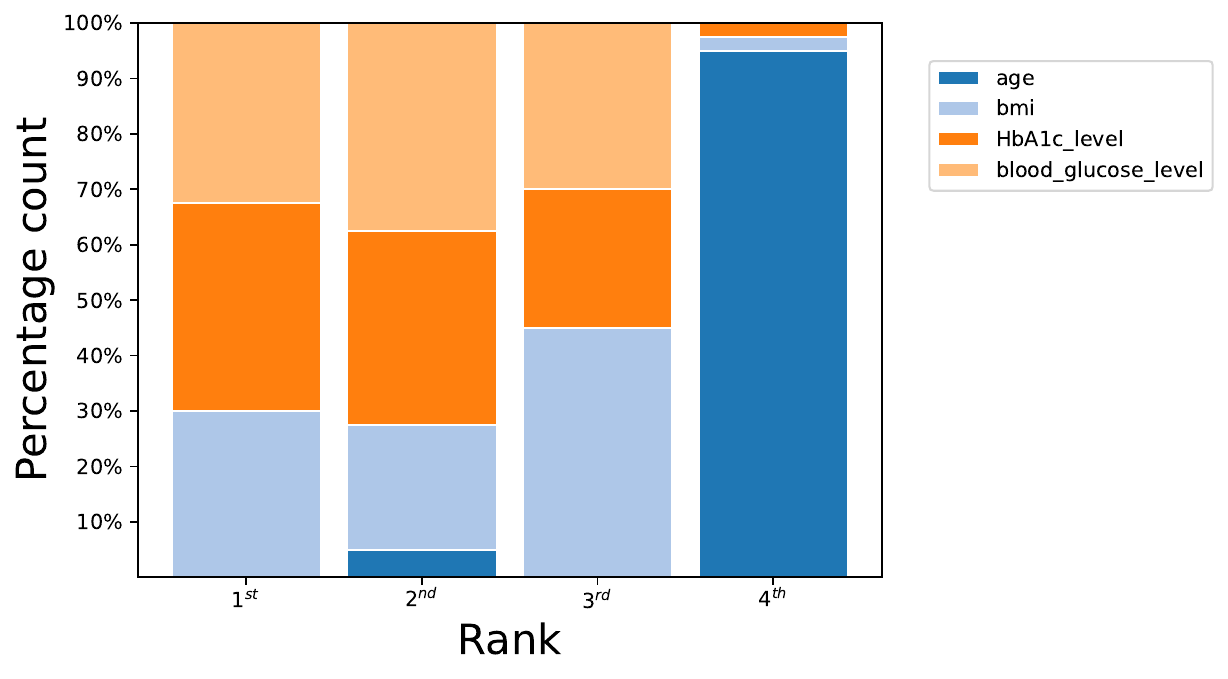}
      \caption{Bar Plot {\ttfamily Diabetes} Scenario I}
      \label{fig:GFI-Diabetes}
    \end{subfigure}\hfil % <-- added
    \begin{subfigure}[t]{0.29\textwidth}
    \centering
      \includegraphics[width=\linewidth]{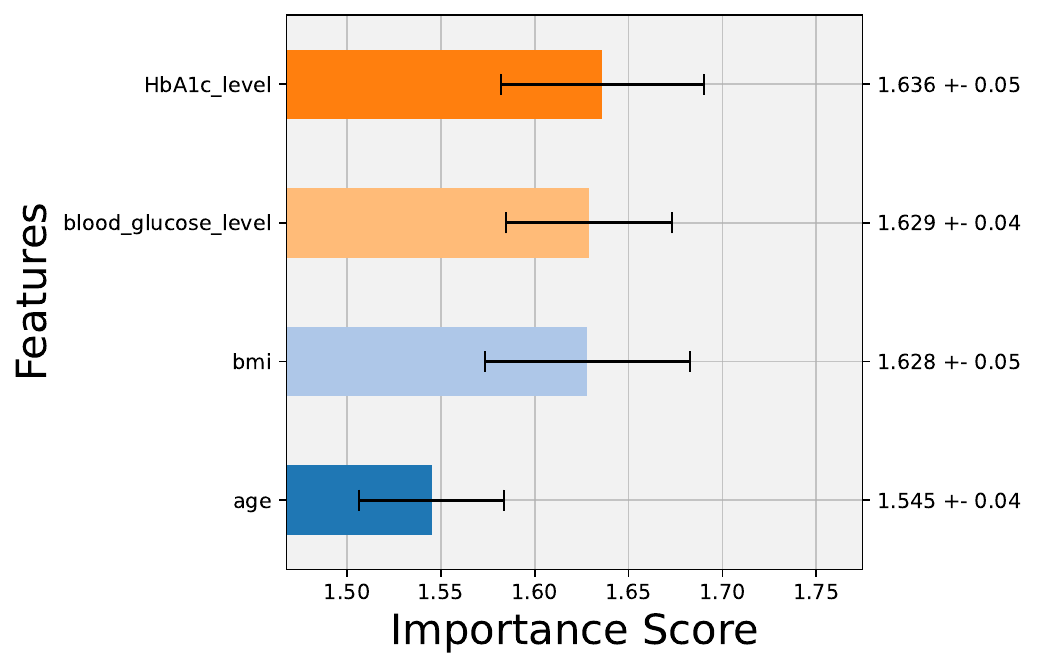}
      \caption{Score Plot {\ttfamily Diabetes} Scenario I}
      \label{fig:Feat-imp-Diabetes}
    \end{subfigure}\hfil % <-- added
    \begin{subfigure}[t]{0.26\textwidth}
    \centering
      \includegraphics[width=\linewidth]{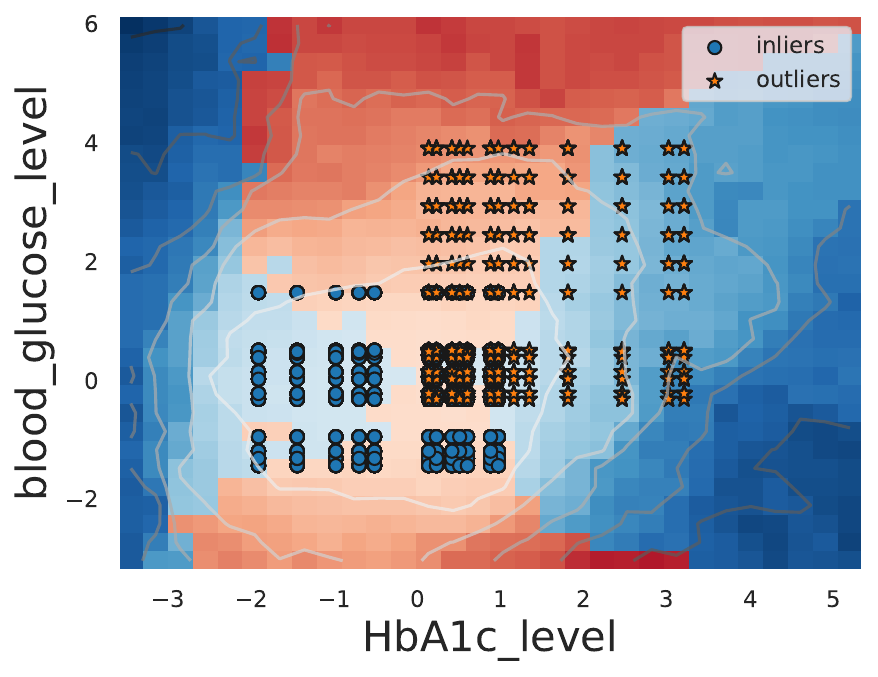}
      \caption{Scoremap {\ttfamily Diabetes} Scenario I}
      \label{fig:Local-Diabetes}
    \end{subfigure}\hfil % <-- added
    \begin{subfigure}[t]{0.33\textwidth}
    \centering
      \includegraphics[width=\linewidth]{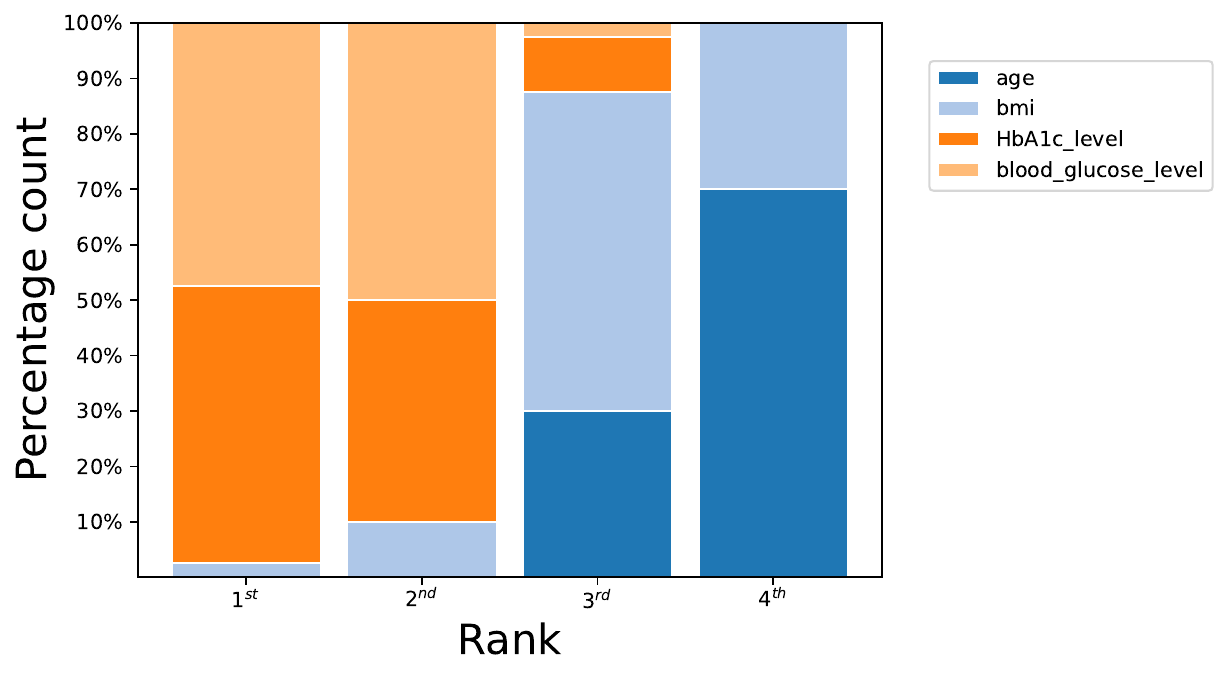}
      \caption{Bar Plot {\ttfamily Diabetes} Scenario II}
      \label{fig:GFI-Diabetes-split}
    \end{subfigure}\hfil % <-- added
    \begin{subfigure}[t]{0.29\textwidth}
    \centering
      \includegraphics[width=\linewidth]{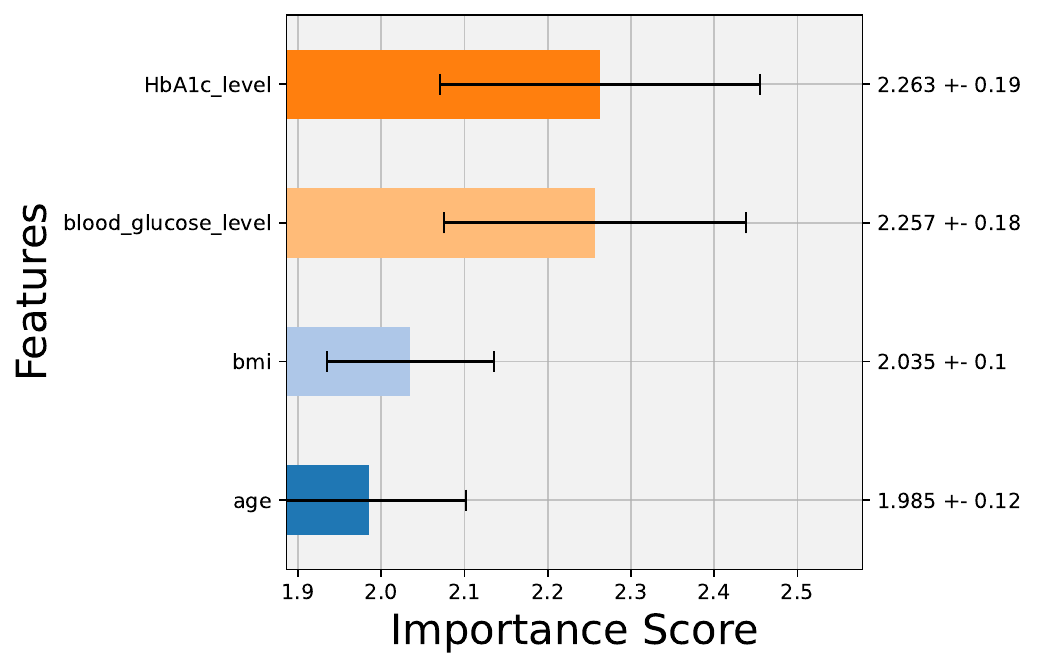}
      \caption{Score Plot {\ttfamily Diabetes} Scenario II}
      \label{fig:Feat-imp-Diabetes-split}
    \end{subfigure}\hfil % <-- added
    \begin{subfigure}[t]{0.26\textwidth}
    \centering
      \includegraphics[width=\linewidth]{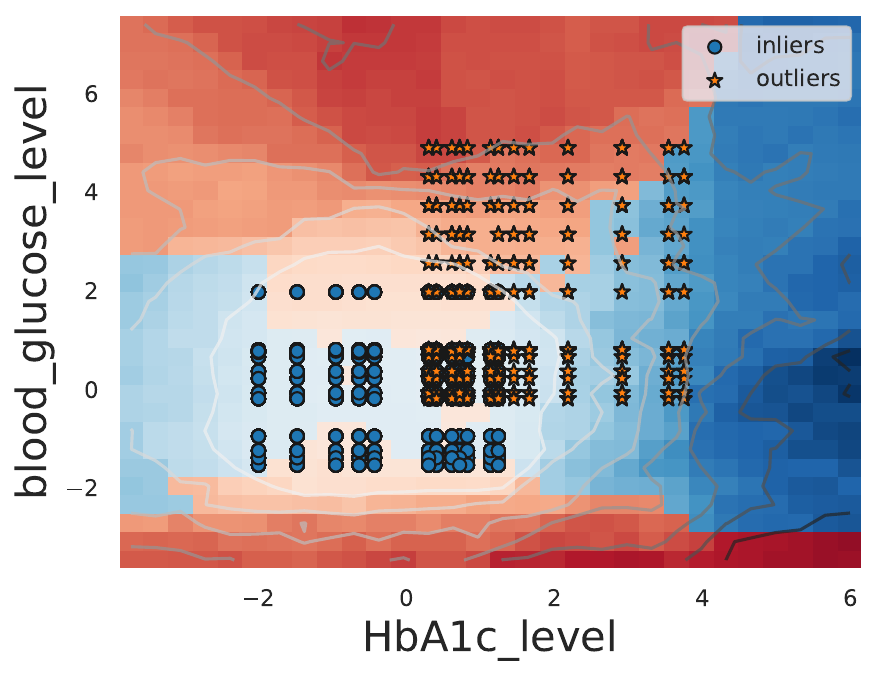}
      \caption{Scoremap {\ttfamily Diabetes} Scenario II}
      \label{fig:Local-Diabetes-split}
    \end{subfigure}\hfil % <-- addedDiabetes
\caption{Bar Plot, Score Plot and Scoremap for {\ttfamily Diabetes} in the two different Scenarios, using the \approach algorithm applied to the \EIFplus model.}\label{fig:interpretation-Diabetes}
\end{figure}

\subsubsection{Feature Selection}

\ale{The validity of the interpretation of the \EIFplus model provided by \approach is confirmed once again in the plots represented in Figure \ref{fig:interpretation-Diabetes} where Unsupervised Feature Selection is exploited as a proxy task for the comparison of ad-hoc and post-hoc interpretation algorithms. The plot related to the \approach+ model is the only one associated with a shape that certifies a correct feature ranking for the Anomaly Detection task. Indeed the plot placed in Figure \ref{fig:Feat-Sel_Diabetes_valEIF+_EXIFFI+_2} is the unique graph where the red line always contains superior Average Precision values in comparison to the blue line. Conversely in the plots referred to other interpretation methods the metrics values oscillate without providing any clear sign of weather the feature selection approach associated with the blue or red line is superior.} 

\begin{figure}[!ht] 
\centering
\hspace{0.05\textwidth}\textbf{IF} \hspace{0.29\textwidth} \textbf{EIF} \hspace{0.29\textwidth} \textbf{EIF+}
% First row with vertical caption on the left
\begin{minipage}{\textwidth}
    \rotatebox{90}{\parbox{15mm}{\centering \textbf{Ad-Hoc}}} % Adjust the parbox width as necessary for your caption text
    \begin{minipage}{0.95\textwidth}
        \begin{subfigure}[t]{0.30\textwidth}
            \centering
            \includegraphics[trim={0 0 3.5cm 0}, clip, width=\linewidth]{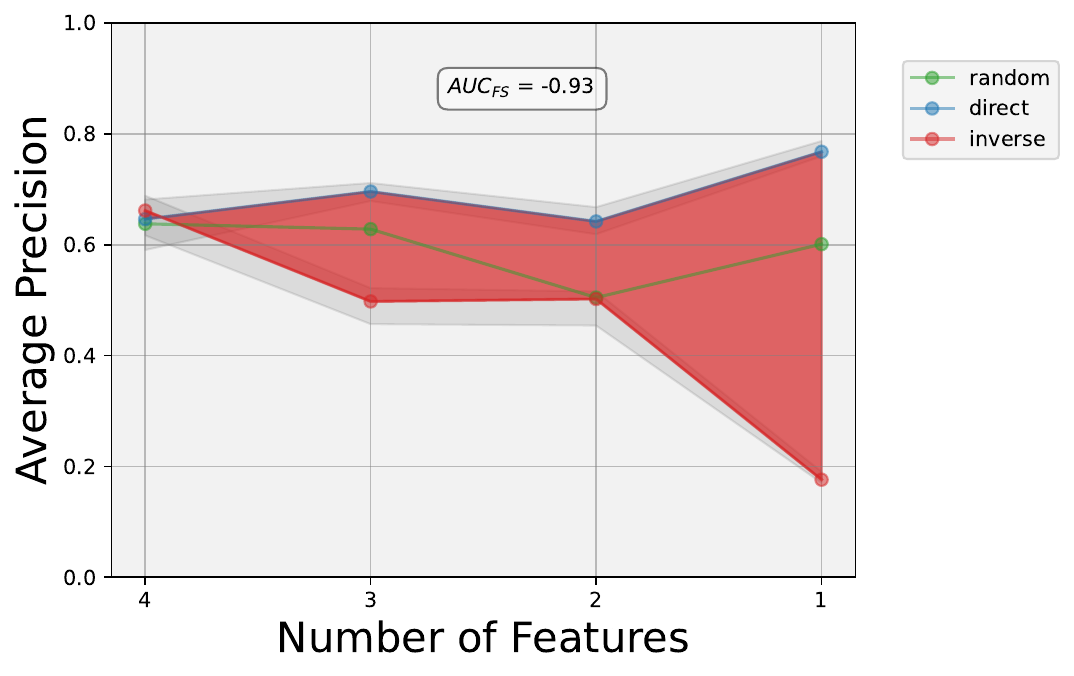}
            \caption{\approach applied to IF}
            \label{fig:Feat-Sel_Diabetes_valEIF+_DIFFI_2}
        \end{subfigure}\hfill
        \begin{subfigure}[t]{0.30\textwidth}
            \centering
            \includegraphics[trim={0 0 3.5cm 0}, clip, width=\linewidth]{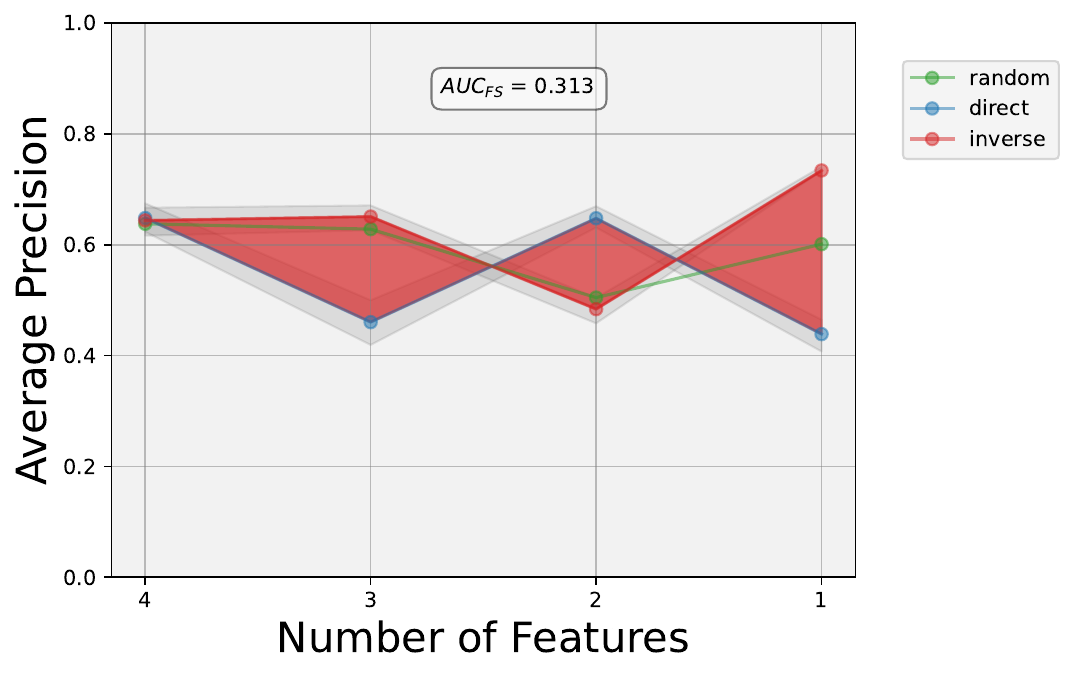}
            \caption{\approach applied to EIF}
            \label{fig:Feat-Sel_Diabetes_valEIF+_EXIFFI_2}
        \end{subfigure}\hfill
        \begin{subfigure}[t]{0.30\textwidth}
            \centering
            \includegraphics[trim={0 0 3.5cm 0}, clip, width=\linewidth]{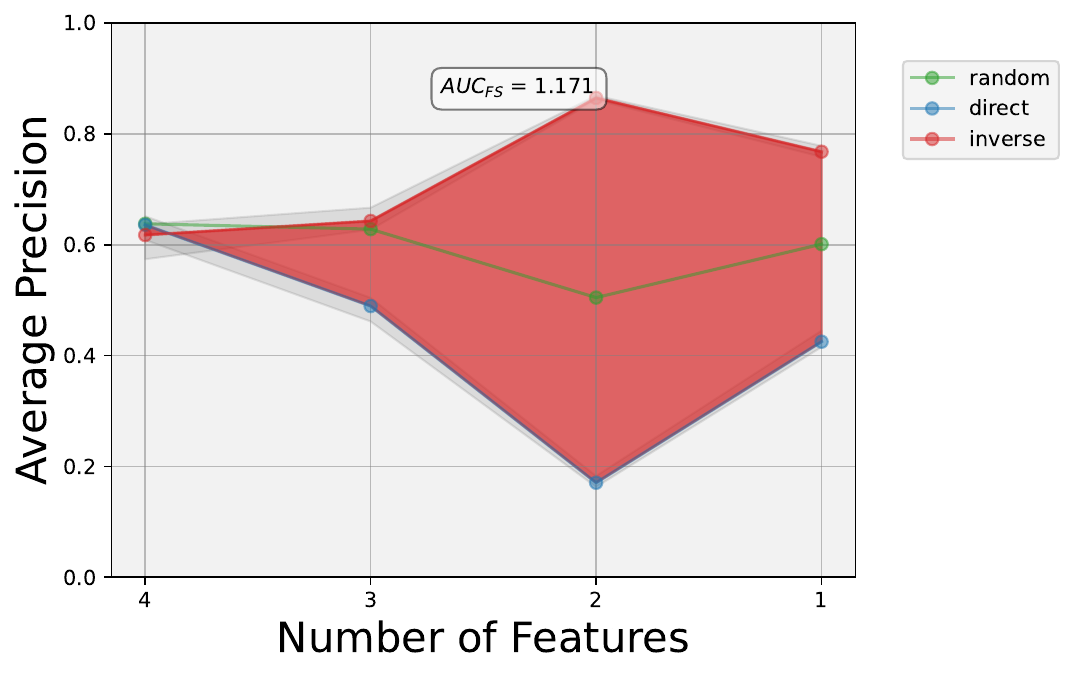}
            \caption{\approach applied to \EIFplus}
            \label{fig:Feat-Sel_Diabetes_valEIF+_EXIFFI+_2}
        \end{subfigure}
    \end{minipage}
\end{minipage}

\vspace{5mm} % Space between rows

% Second row with vertical caption on the left
\begin{minipage}{\textwidth}
    \rotatebox{90}{\parbox{15mm}{\centering \textbf{Post-Hoc}}} % Adjust as necessary
    \begin{minipage}{0.95\textwidth}
        \begin{subfigure}[t]{0.30\textwidth}
            \centering
            \includegraphics[trim={0 0 3.5cm 0}, clip, width=\linewidth]{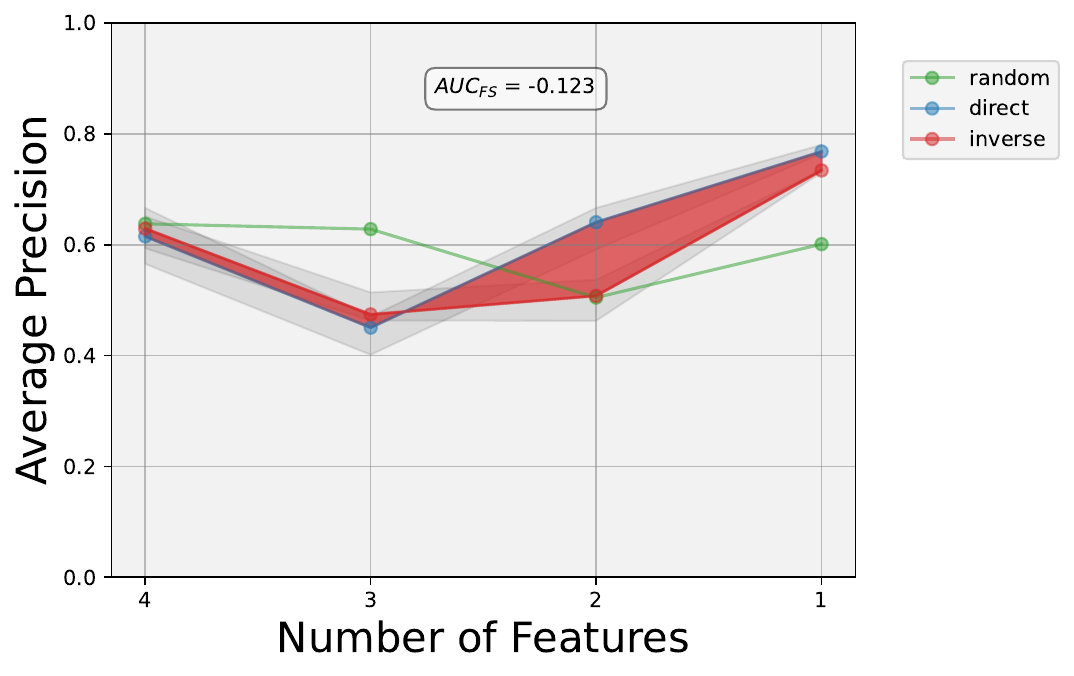}
            \caption{RandomForest fitted to IF}
            \label{fig:Feat-Sel_Diabetes_valEIF+_IF_RandomForest_2}
        \end{subfigure}\hfill
        \begin{subfigure}[t]{0.30\textwidth}
            \centering
            \includegraphics[trim={0 0 3.5cm 0}, clip, width=\linewidth]{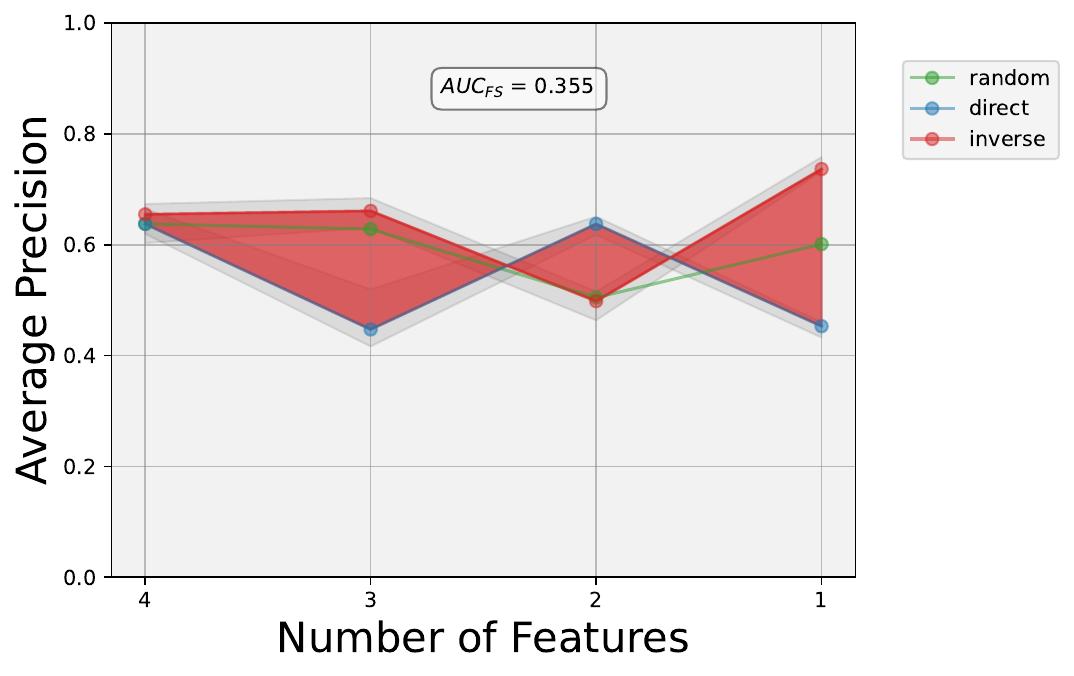}
            \caption{RandomForest fitted to EIF}
            \label{fig:Feat-Sel_Diabetes_valEIF+_EIF_RandomForest_2}
        \end{subfigure}\hfill
        \begin{subfigure}[t]{0.30\textwidth}
            \centering
            \includegraphics[trim={0 0 3.5cm 0}, clip, width=\linewidth]{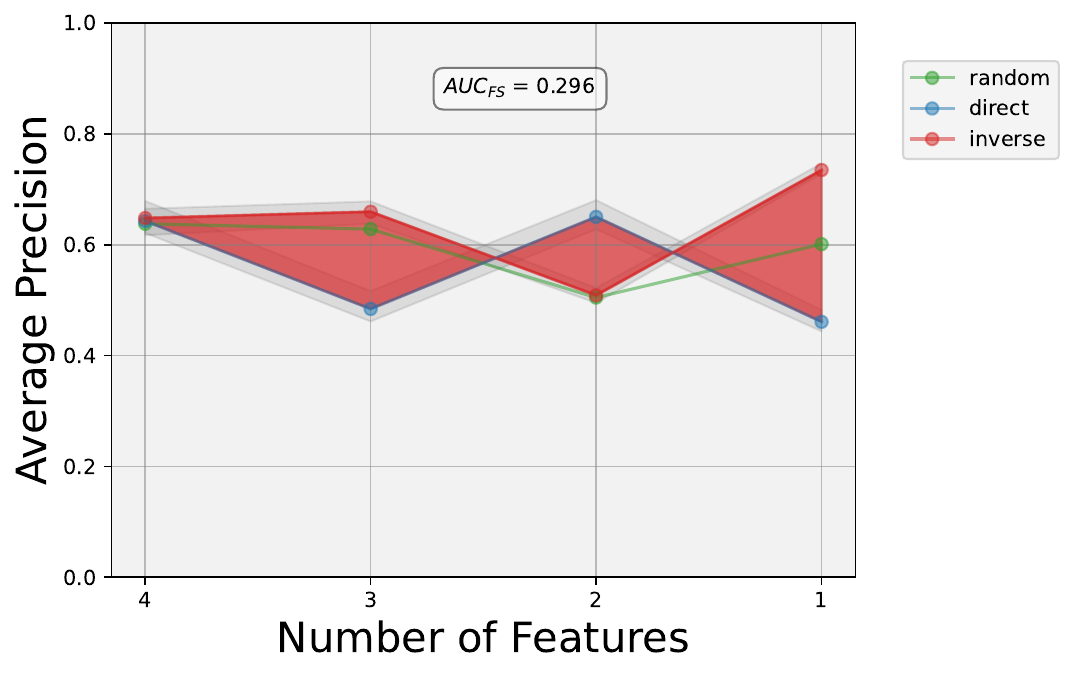}
            \caption{RandomForest fitted to \EIFplus}
            \label{fig:Feat-Sel_Diabetes_valEIF+_EIF+_RandomForest_2}
        \end{subfigure}
    \end{minipage}
\end{minipage}

\caption{Feature Selection of the different Ad-Hoc and Post-Hoc methods applied to the 3 Isolation Forest models: IF, EIF and \EIFplus. The blue line is the values of average precision, calculated with the \EIFplus model in the Scenario II, dropping the most important feature at each step, the red line is the values of average precision dropping the least important feature at each step and the green line is the value of the feature selection dropping a random feature at each step.}\label{fig:fs-interpretation-Diabetes}
\end{figure}

\ale{In Table \ref{tab:fs-tab-Diabetes} the $AUC_{FS}$ values, for a quantitative comparison of the effectiveness of the interpretability provided by the diverse methods analysed in this study are contained. As already observed from a careful analysis of the Feature Selection plots (Figure \ref{fig:fs-interpretation-Diabetes} the explanation better aligned with the ground truth is the one provided by the proposed \approach+ approach. On the other hand the outcomes provided by the other considered models prove to be less satisfactory, in particular the ones produced by \approach on the IF model which are paired with negative $AUC_{FS}$ values, a clear prove of an erroneous ranking of attributes' relevance.}

\subsection*{{\ttfamily Glass}}\label{sec:glass}

% Additional comment to satisfy comment 7 by reviewer 2 and Comment 11 of reviewer 1 
\davide{Next, the {\ttfamily Glass} dataset is considered. As explained in \ref{sec:appendix-real-world-data} this dataset in a Multi-Class Classification task to distinguish between different glass qualities. In particular this dataset was chosen for the evaluation of the reliability and alignment with human cognition of \approach since it is equipped with a sort of ground truth on what are the most important features to distinguish between anomalous and non anomalous samples, which is provided by studies conducted by domain experts.}

\subsubsection{Performance}
\ale{In Figure \ref{fig:Glass_contamination}, we notice that the performance of all models improves as the contamination level in the training dataset decreases, with the DIF model outperforming the rest, followed by the \EIFplus. Specifically, the plot in Figure \ref{fig:Glass_contaminationEIFvsEIF+} highlights the \EIFplus model's distinct advantage in achieving higher average precision at lower contamination levels, showcasing its enhanced capability to generalize effectively when trained without anomalies. This demonstrates the \EIFplus model's proficiency in adapting to datasets with low contamination, emphasizing its strength in scenarios with unseen anomalies compared to EIF.}

\begin{figure}[htbp] 
    \centering % <-- added
    \begin{subfigure}[t]{0.49\textwidth}
      \includegraphics[width=\linewidth]{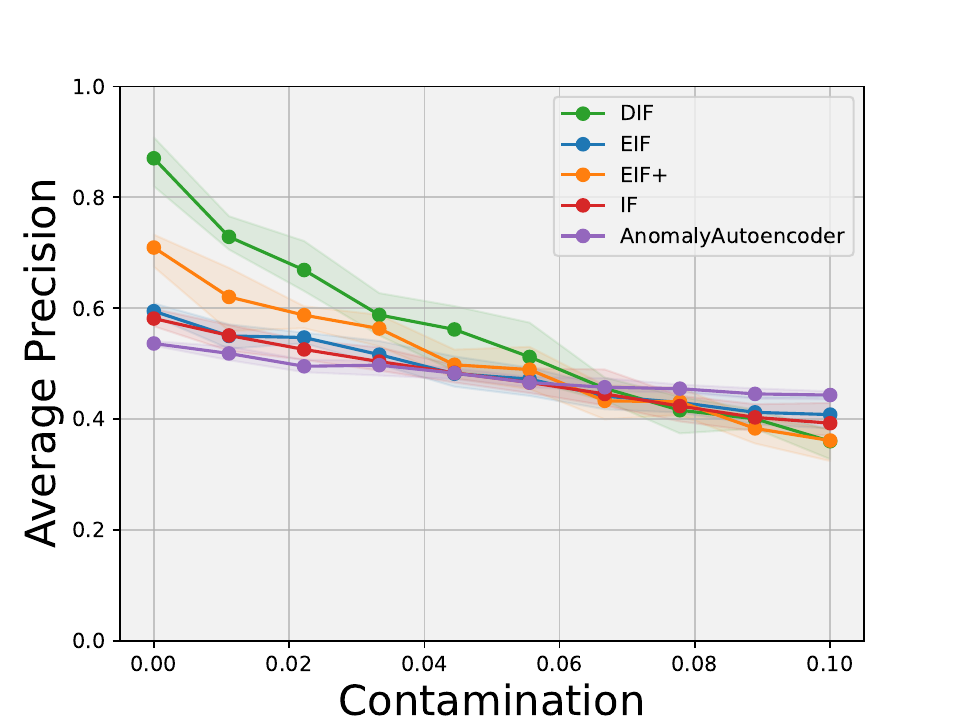}
      \caption{Models evaluation, varying the contamination levels}
      \label{fig:Glass_contamination_full}
    \end{subfigure}\hfil % <-- added
    \begin{subfigure}[t]{0.44\textwidth}
      \includegraphics[width=\linewidth]{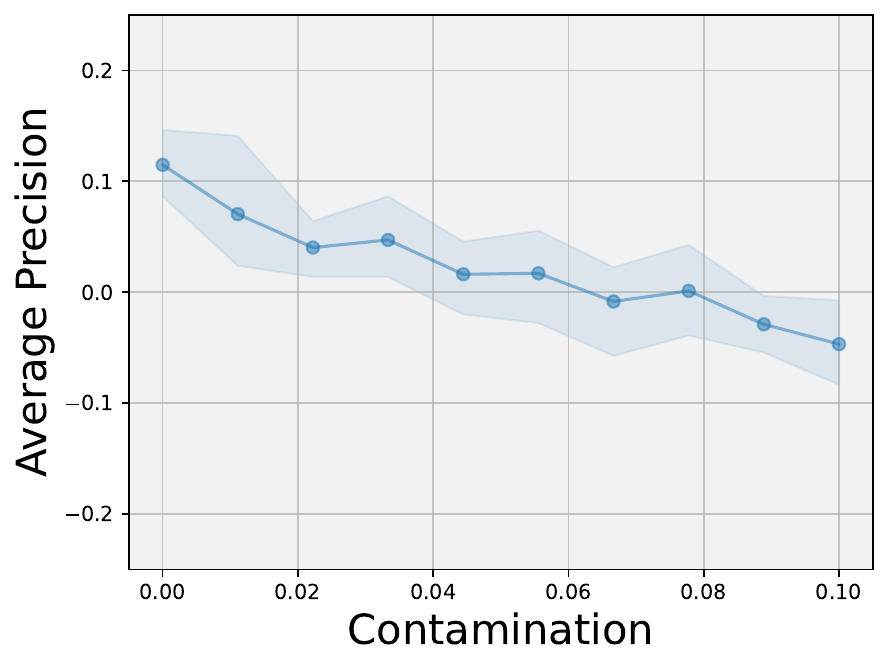}
      \caption{Difference between \EIFplus and EIF average precision}
      \label{fig:Glass_contaminationEIFvsEIF+}
    \end{subfigure}\hfil % <-- added
\caption{Figure \ref{fig:Glass_contamination_full} illustrates the average precision as the contamination level in the training set increases. Figure \ref{fig:Glass_contaminationEIFvsEIF+} compares the performance graphs of EIF and \EIFplus, using the difference of their scores in various contamination levels.}
\label{fig:Glass_contamination}
\end{figure}

\ale{Table \ref{tab:glasspr} illustrates that \EIFplus maintains comparable outcomes in Scenario I and, leveraging its enhanced generalization capabilities for unseen anomalies, ranks as the second highest-performing algorithm in Scenario II. Notably, it fits 10 times faster than the DIF and predicts the entire dataset's scores 30 times more swiftly, showcasing its efficiency and efficacy in both model fitting and anomaly detection across scenarios.}

\begin{table}[!ht]
\centering
%\caption{{\ttfamily Glass} Performance Report}
\caption{Performances of 5 different Anomaly Detection models over {\ttfamily Glass} are compared using classical Classification metrics. Moreover, the last two columns contain the average time for a fit and predict operation. The highest metric values and the lowest execution times are highlighted in bold}\label{tab:glasspr}
\begin{tabular}{|c||ccc|ccc||cc|}
\toprule
\hline
& \multicolumn{3}{c|}{Scenario I} & \multicolumn{3}{c||}{Scenario II} & \multicolumn{2}{c|}{Time} \\
\hline
AD Model & Avg & Prec & ROC & Avg & Prec & ROC & fit & pred \\
& Prec &  & AUC & Prec &  & AUC & fit & pred \\
\hline
IF          & 0.36 & 0.34 & 0.62 & 0.65 & 0.68 & 0.82 & \textbf{0.07}& \textbf{0.002}\\
EIF         & 0.35 & 0.27 & 0.58 & 0.57 & 0.68 & 0.82 & \textbf{0.07}& 0.01  \\
\EIFplus        & 0.31 & 0.24 & 0.56 & 0.69& 0.79& 0.88 & \textbf{0.07}& 0.01  \\
DIF         & 0.3 & 0.2& 0.54& \textbf{0.85}& \textbf{0.82}& \textbf{0.9}& 0.67 & 0.29  \\
AE & \textbf{0.41}& \textbf{0.44}& \textbf{0.68}& 0.53 & 0.62& 0.78& 2.25 & 0.04  \\
\hline
\end{tabular}
\end{table}

\subsubsection{Importance Plots} \label{sec:glass-imp-plots}
\ale{In the Figures \ref{fig:Feat-imp-Glass}, which illustrate the importance scores for Scenario I, there's noticeable uncertainty with no clear indication of a single feature standing out as the most important. This ambiguity is highlighted by the data point distribution in Figure \ref{fig:Local-glass}, where we see significant variance in both the dimensions. The model appears to blend a subset of anomalies with inliers, as indicated by a broader contour plot along the feature {\ttfamily Ba} (Barium) compared to its narrower counterpart in Scenario II (Figure \ref{fig:Local-glass-split}). This difference is likely because anomalies are more distinctly clustered in a specific area of the space, suggesting they are more a subset of the data distribution. This concept was further discussed in \ref{sec:appendix-real-world-data}.}

\ale{The dataset comprise objects made of glass, characterized by features like the refractive index (RI) and concentrations of elements. Carletti et al. \cite{carletti2019explainable} pointed out that the outliers are the data belonging to the subclass of headlamp glass. The key difference between headlamp and window glass is the Barium due to its contribution to optical enhancements. Specifically, Barium boosts the refractive index, thus augmenting light transmission and brightness \cite{D3RA08015C} vital for automotive headlamps. Its incorporation into headlamp glass optimizes light focus and directionality, underscoring its significance in improving headlamp functionality.}

\begin{figure}[htbp] 
    \centering % <-- added
    \begin{subfigure}[t]{0.33\textwidth}
    \centering
      \includegraphics[width=\linewidth]{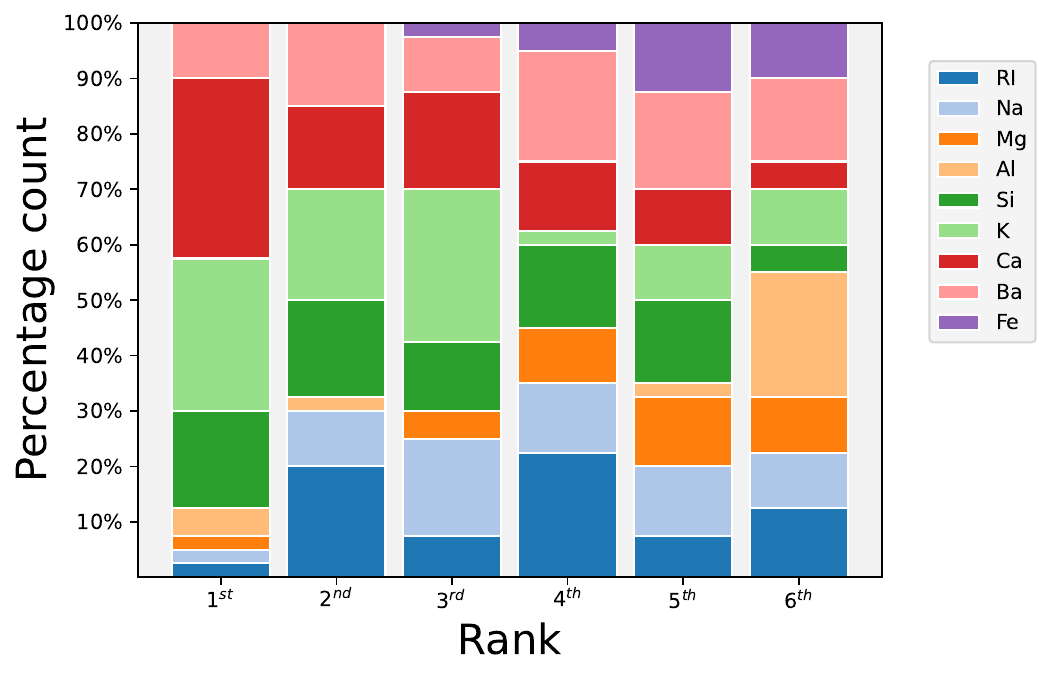}
      \caption{Score Plot {\ttfamily Glass} Scenario I}
      \label{fig:Feat-imp-Glass}
    \end{subfigure}\hfil % <-- added
    \begin{subfigure}[t]{0.27\textwidth}
    \centering
      \includegraphics[width=\linewidth]{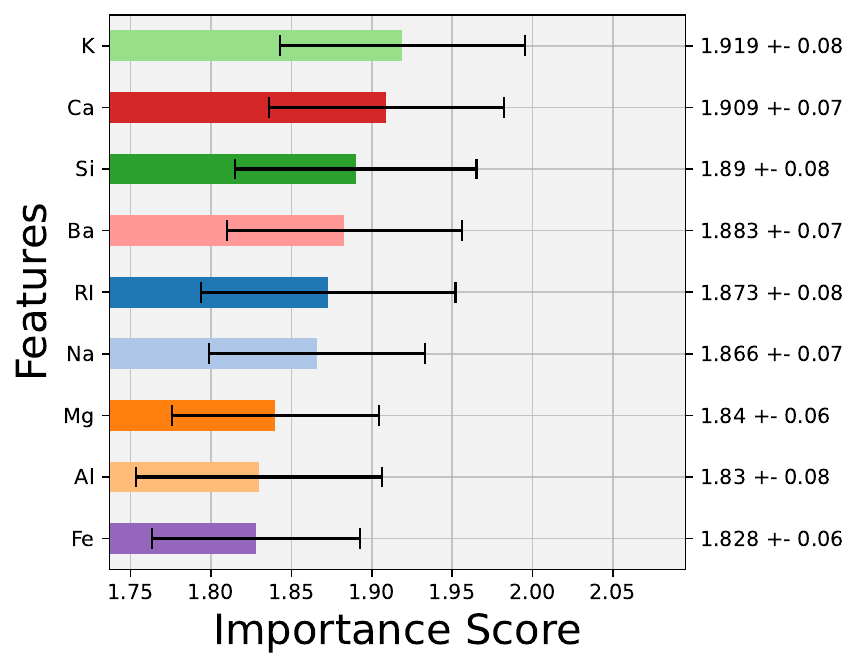}
      \caption{Bar Plot {\ttfamily Glass} Scenario I}
      \label{fig:GFI-glass}
    \end{subfigure}\hfil % <-- added
    \begin{subfigure}[t]{0.28\textwidth}
    \centering
      \includegraphics[width=\linewidth]{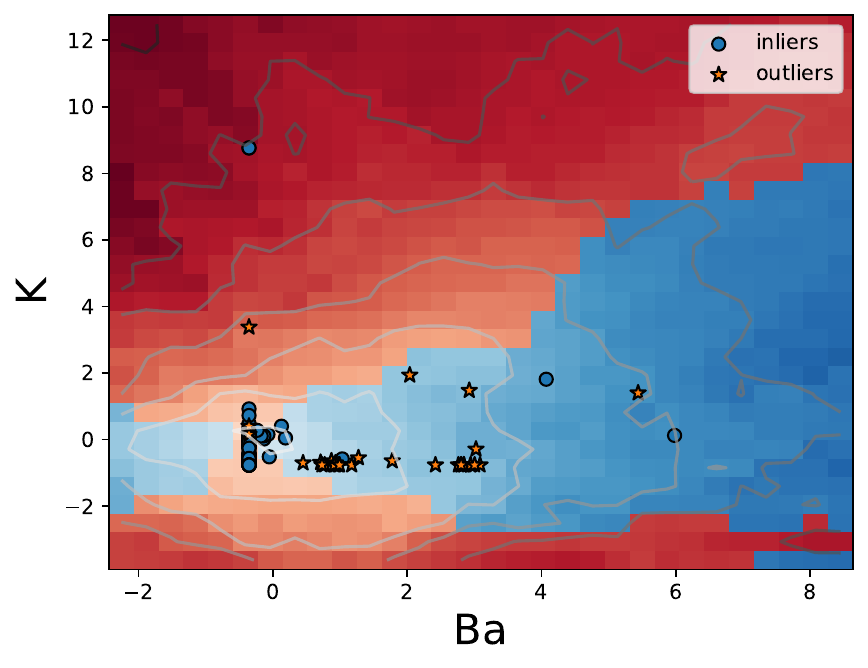}
      \caption{Scoremap {\ttfamily Glass} Scenario I}
      \label{fig:Local-glass}
    \end{subfigure}\hfil % <-- added
    \begin{subfigure}[t]{0.33\textwidth}
    \centering
      \includegraphics[width=\linewidth]{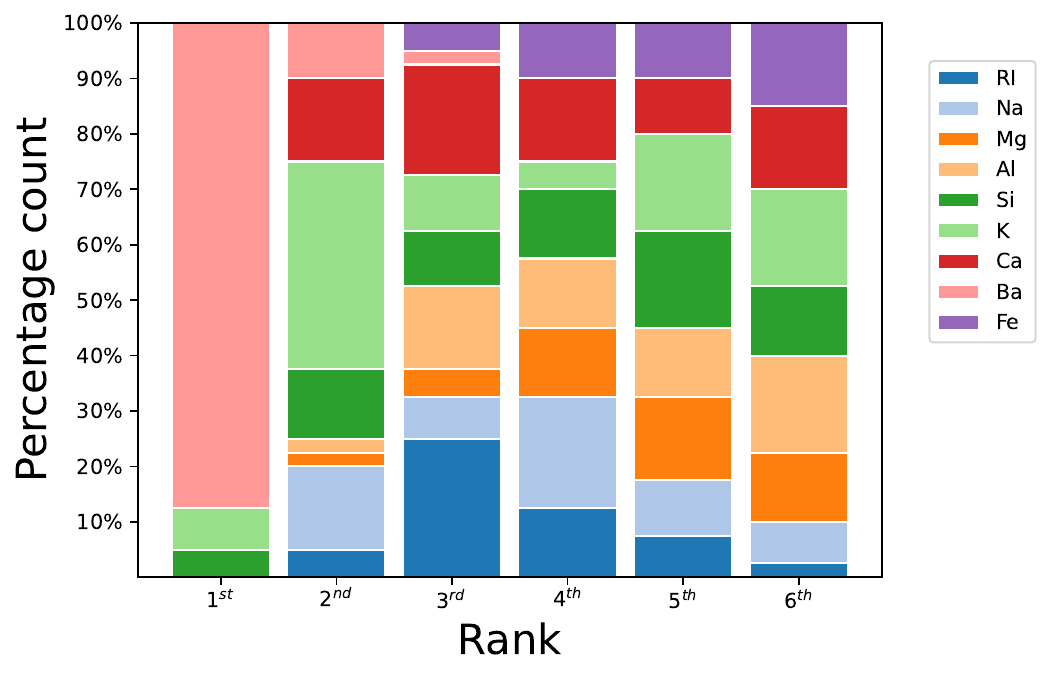}
      \caption{Score Plot {\ttfamily Glass} Scenario II}
      \label{fig:Feat-imp-Glass-split}
    \end{subfigure}\hfil % <-- added
    \begin{subfigure}[t]{0.27\textwidth}
    \centering
      \includegraphics[width=\linewidth]{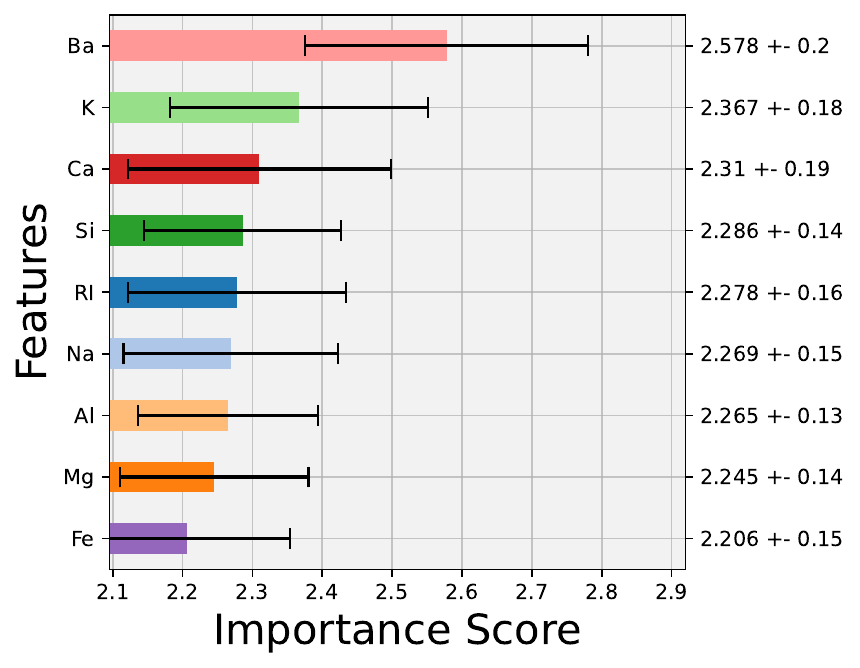}
      \caption{Bar Plot {\ttfamily Glass} Scenario II}
      \label{fig:GFI-glass-split}
    \end{subfigure}\hfil % <-- added
    \begin{subfigure}[t]{0.28\textwidth}
    \centering
      \includegraphics[width=\linewidth]{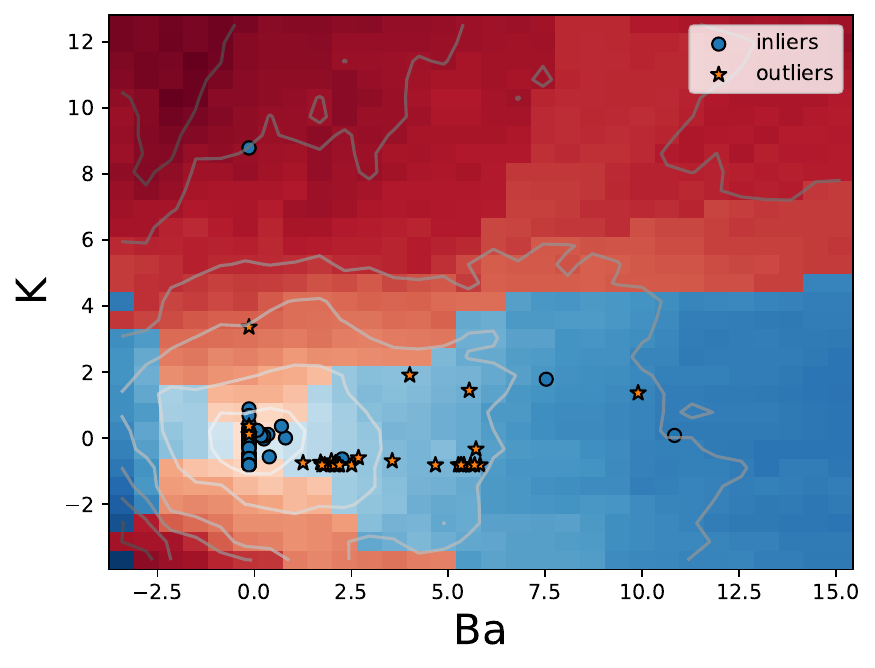}
      \caption{Scoremap {\ttfamily Glass} Scenario II}
      \label{fig:Local-glass-split}
    \end{subfigure}\hfil % <-- added
\caption{Bar Plot, Score Plot and Scoremap for {\ttfamily Glass}  in the two different Scenarios, using the \approach algorithm applied to the \EIFplus model.}\label{fig:interpretation-glass}
\end{figure}

\ale{In addition, The Potassium (K) it is especially used in glass types requiring increased strength or thermal resistance, such as certain window glasses. But we can observe in the local Scoremap that the deviation from the distribution along the variable K does not coincide with a particular distribution of anomalies.}

\ale{As depicted in Figures \ref{fig:Feat-imp-Glass-split} and \ref{fig:GFI-glass-split}  Scenario II's analysis highlights Barium (Ba) as a pivotal feature, followed by Potassium (K). This results provides an additional confirmation on the correctness of the proposed approach that aligns with the domain knowledge on what is the most relevant attribute for the distinction between window and headlamp glasses.}

\subsubsection{Feature Selection}
\ale{Figure \ref{fig:interpretation-glass} showcases the Feature Selection for the glass dataset, highlighting the superior performance of ad-hoc interpretation algorithms over the surrogate Random Forest's feature importance method. All models succeed in identifying key features because the performance improve the more the less important features are dropped, improving the average precision score as features are shrinked to the most important ones.}

\begin{figure}[htbp] 
\centering
\hspace{0.05\textwidth}\textbf{IF} \hspace{0.29\textwidth} \textbf{EIF} \hspace{0.29\textwidth} \textbf{EIF+}
% First row with vertical caption on the left
\begin{minipage}{\textwidth}
    \rotatebox{90}{\parbox{15mm}{\centering \textbf{Ad-Hoc}}} % Adjust the parbox width as necessary for your caption text
    \begin{minipage}{0.95\textwidth}
        \begin{subfigure}[t]{0.30\textwidth}
            \centering
            \includegraphics[trim={0 0 3.5cm 0}, clip, width=\linewidth]{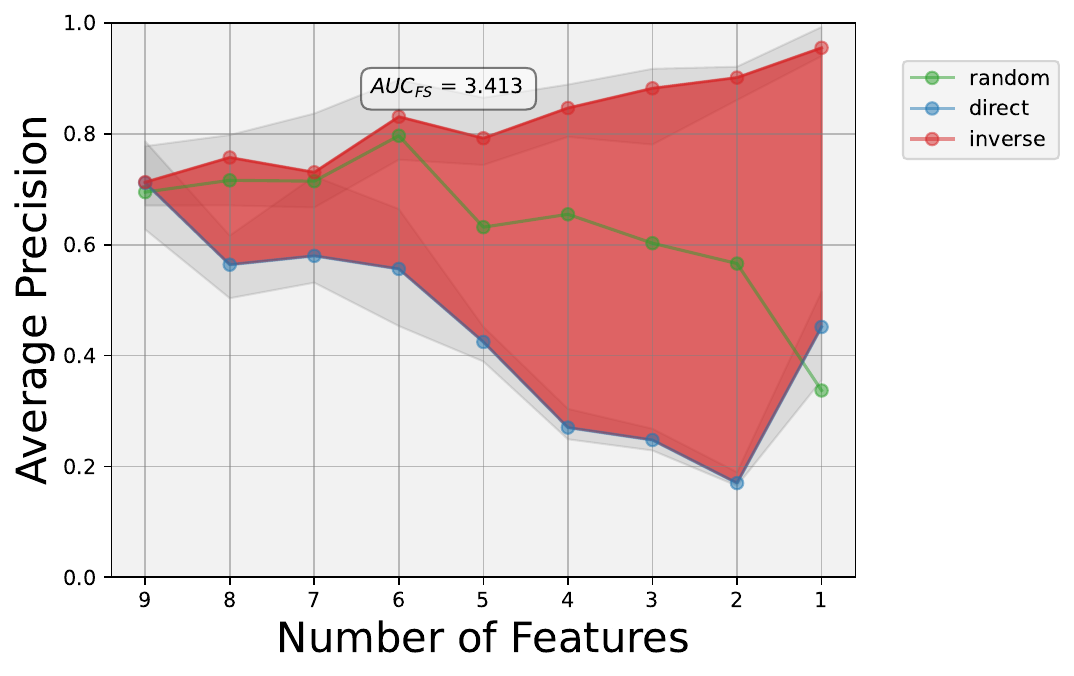}
            \caption{\approach applied to IF}
            \label{fig:Feat-Sel_Glass_valEIF+_DIFFI_2}
        \end{subfigure}\hfill
        \begin{subfigure}[t]{0.30\textwidth}
            \centering
            \includegraphics[trim={0 0 3.5cm 0}, clip, width=\linewidth]{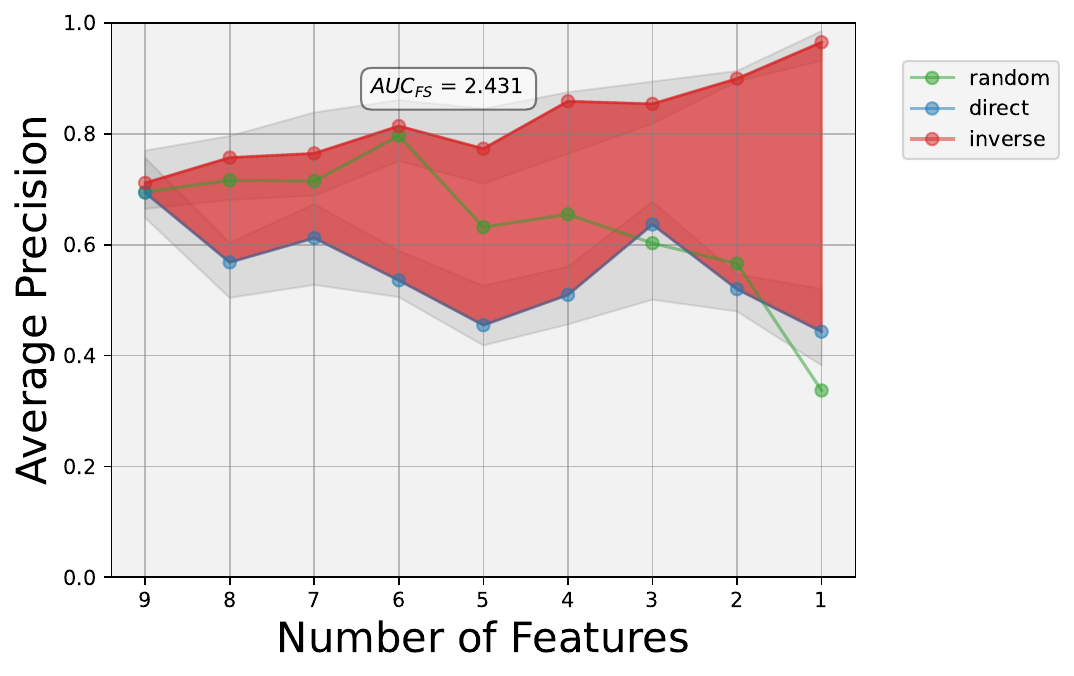}
            \caption{\approach applied to EIF}
            \label{fig:Feat-Sel_Glass_valEIF+_EXIFFI_2}
        \end{subfigure}\hfill
        \begin{subfigure}[t]{0.30\textwidth}
            \centering
            \includegraphics[trim={0 0 3.5cm 0}, clip, width=\linewidth]{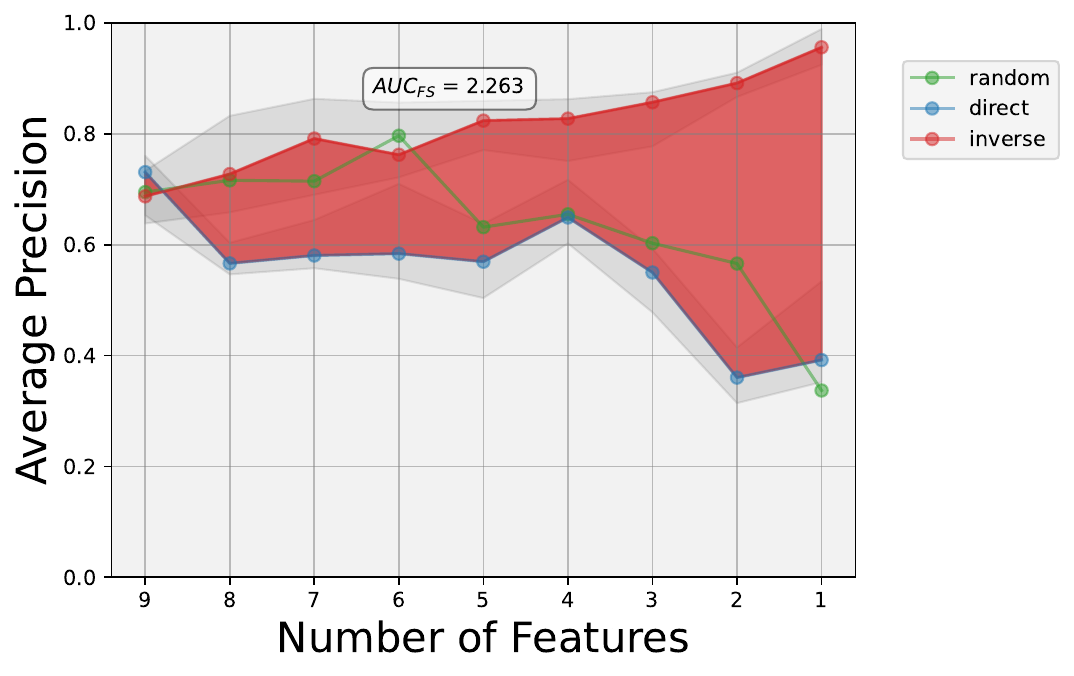}
            \caption{\approach applied to \EIFplus}
            \label{fig:Feat-Sel_Glass_valEIF+_EXIFFI+_2}
        \end{subfigure}
    \end{minipage}
\end{minipage}

\vspace{5mm} % Space between rows

% Second row with vertical caption on the left
\begin{minipage}{\textwidth}
    \rotatebox{90}{\parbox{15mm}{\centering \textbf{Post-Hoc}}} % Adjust as necessary
    \begin{minipage}{0.95\textwidth}
        \begin{subfigure}[t]{0.30\textwidth}
            \centering
            \includegraphics[trim={0 0 3.5cm 0}, clip, width=\linewidth]{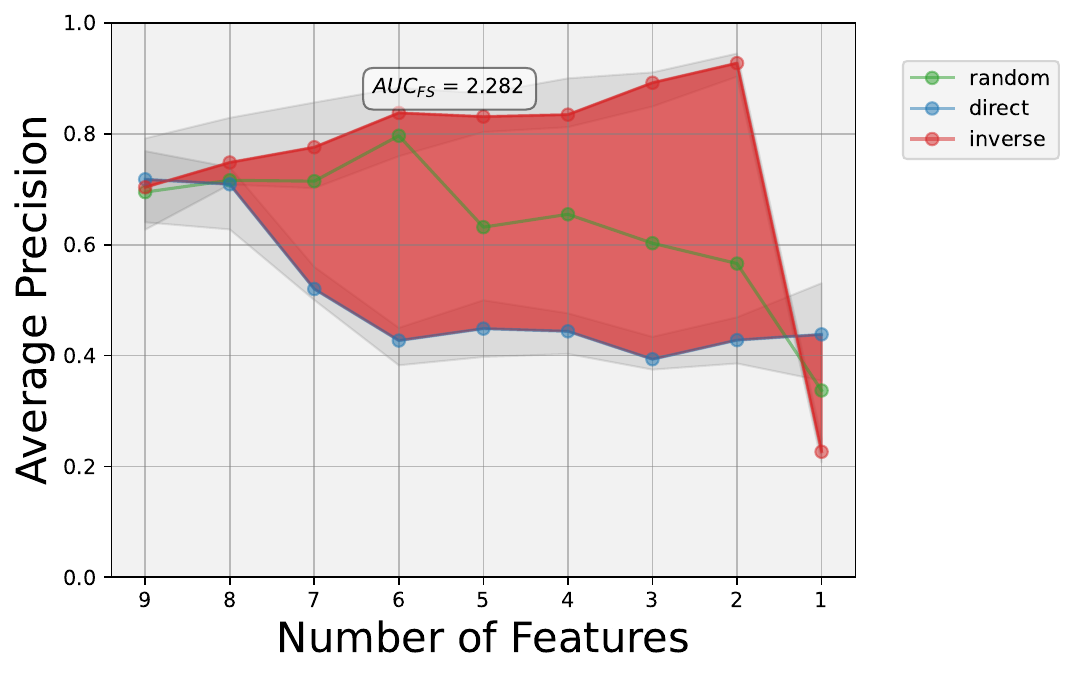}
            \caption{RandomForest applied to IF}
            \label{fig:Feat-Sel_Glass_valEIF+_IF_RandomForest_2}
        \end{subfigure}\hfill
        \begin{subfigure}[t]{0.30\textwidth}
            \centering
            \includegraphics[trim={0 0 3.5cm 0}, clip, width=\linewidth]{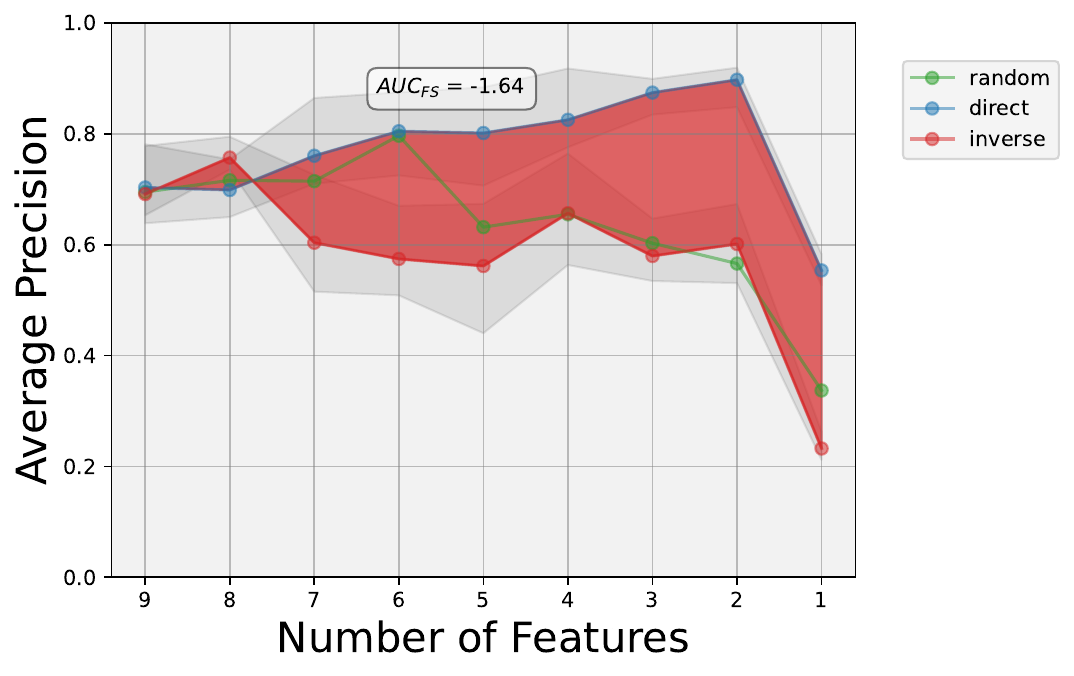}
            \caption{RandomForest applied to EIF}
            \label{fig:Feat-Sel_Glass_valEIF+_EIF_RandomForest_2}
        \end{subfigure}\hfill
        \begin{subfigure}[t]{0.30\textwidth}
            \centering
            \includegraphics[trim={0 0 3.5cm 0}, clip, width=\linewidth]{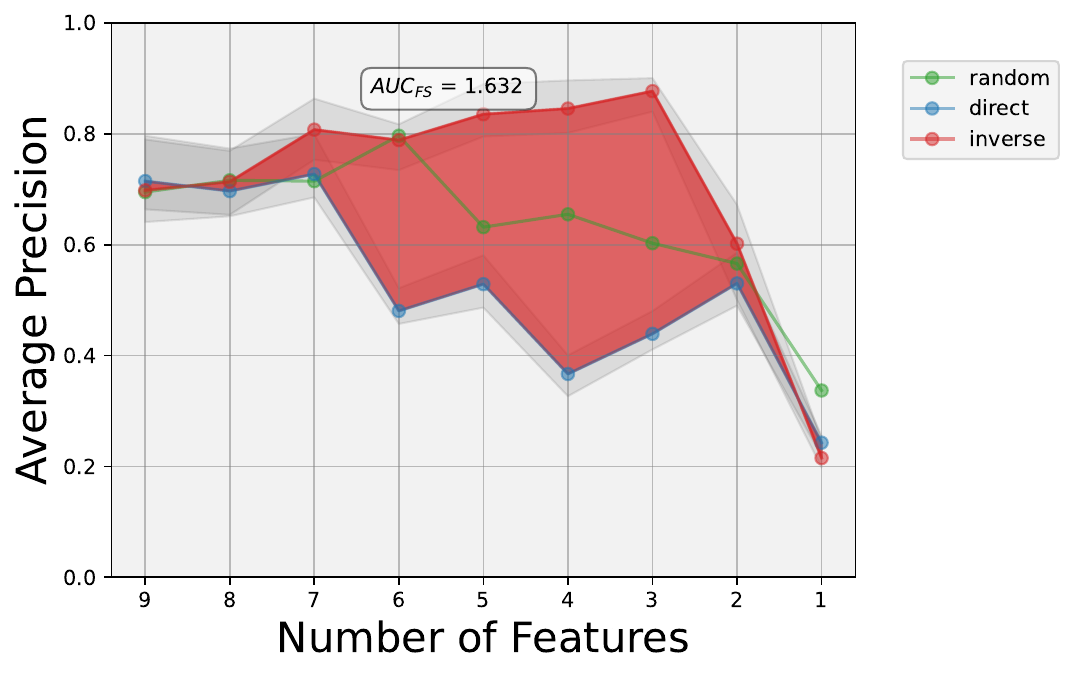}
            \caption{RandomForest applied to \EIFplus}
            \label{fig:Feat-Sel_Glass_valEIF+_EIF+_RandomForest_2}
        \end{subfigure}
    \end{minipage}
\end{minipage}
\caption{Feature Selection of the different Ad-Hoc and Post-Hoc methods applied to the 3 Isolation Forest models: IF, EIF and \EIFplus. The blue line is the values of average precision, calculated with the \EIFplus model in the Scenario II, dropping the most important feature at each step, the red line is the values of average precision dropping the least important feature at each step and the green line is the value of the feature selection dropping a random feature at each step.}\label{fig:feature_selections-Glass}
\end{figure}

\ale{In contrast, the Random Forest feature importance method not only falls short in selecting features that enhance the average precision score—resulting in a decreased score—but also demonstrates a scenario where the blue line surpasses the red line in the post-hoc interpretation of the EIF. This indicates that important features impacting the score were prematurely dropped due to being assigned low importance scores by the model. So the Random Forest not only have bad performances but in the specific case of the EIF it gave wrong scores.}

\ale{Table \ref{tab:fs-tab-glass} reveals the performance of various interpretation algorithms across two scenarios. In Scenario I, the DIFFI interpretation algorithm emerges as the top performer. Conversely, in Scenario II, \approach stand out when applied to the 3 models, in particular when applied to the IF model, demonstrating significantly improved results, whereas the Random Forest model consistently faces challenges in accurately interpreting feature importance. This contrast in performance between scenarios underscores the adaptability of ad-hoc algorithms in understanding feature relevance in complex datasets like {\ttfamily glass}, while highlighting the limitations of conventional methods like Random Forest in nuanced interpretation tasks. Moreover \approach shows an improved time efficiency in the computation of importance scores being almost 20 times faster than post-hoc interpretability methods like Random Forest.}

\begin{table}[htbp]
\centering
%\caption{Feature Selection Scores  {\ttfamily Glass}}
\caption{Quantitative evaluation of the effectiveness of 6 different interpretation algorithms on {\ttfamily Glass} through the $AUC_{FS}$ metric, introduced in \ref{sec:interpr_evaluat}. In the last column the average time taken by the different models to produce the importance scores is reported. The highest $AUC_{FS}$ and lowest Importance time values are highlighted in bold.}\label{tab:fs-tab-glass}
\begin{tabular}{|c||c|c|c|c||c|}
\toprule
\hline
&\multicolumn{2}{c|}{Evaluation with EIF}&\multicolumn{2}{c||}{Evaluation with \EIFplus}&\\
\hline
& Scenario I & Scenario II  & Scenario I & Scenario II & Time\\

 Algorithm & $AUC_{FS}$  & $AUC_{FS}$ & $AUC_{FS}$  & $AUC_{FS}$ &  \\
\hline
DIFFI         & \textbf{1.591}      & 2.117     & \textbf{1.555}    & 2.447     & 0.44 \\
IF\_\approach         & 0.302      & \textbf{3.45}     &  0.483   & \textbf{3.413}     & 0.08 \\
EIF\_\approach        & 0.465      & 2.554    & 0.564     & 2.431     & \textbf{0.01} \\
\EIFplus\_\approach       & 0.403      & 1.769     & 0.527     & 2.263     & \textbf{0.01} \\
IF\_RF        & -1.733      & 2.183       & -1.313     & 2.282     & 0.17 \\
EIF\_RF       & -1.718     & -1.634     & -1.511    & -1.64     & 0.17 \\
\EIFplus\_RF      & -1.464     & 1.944     & -1.308    & 1.632     & 0.17 \\
\hline
\end{tabular}
\end{table}

\subsection*{{\ttfamily Ionosphere}}

\ale{The {\ttfamily Ionosphere} dataset, as described in \ref{sec:appendix-real-world-data}, stands out as the dataset with the highest dimensionality (i.e. 33 features) inside the list of benchmark datasets used for the performance assessment in this study. This characteristic may have some consequences on the outcomes of the experiments described in the following sections.}

\subsubsection{Performance}

\ale{The results of the evaluation of each Anomaly Detection model across different values of the contamination hyperparameter are portrayed in Figure \ref{fig:Ionosphere_contamination_full}. The entirety of the models show how the gradual addition of anomalies in the dataset does not result in a significant effect on the Average Precision metric that, in fact, shows more or less constant values very close to a perfect score of 1. The proposed approach \EIFplus, together with the DIF model, are the ones showing the best metric values, followed by EIF, as highligthed in the comparison between \EIFplus and EIF displayed in Figure \ref{fig:Ionosphere_contaminationEIFvsEIF+}.}

\begin{figure}[!ht] 
    \centering % <-- added
    \begin{subfigure}[t]{0.49\textwidth}
      \includegraphics[width=\linewidth]{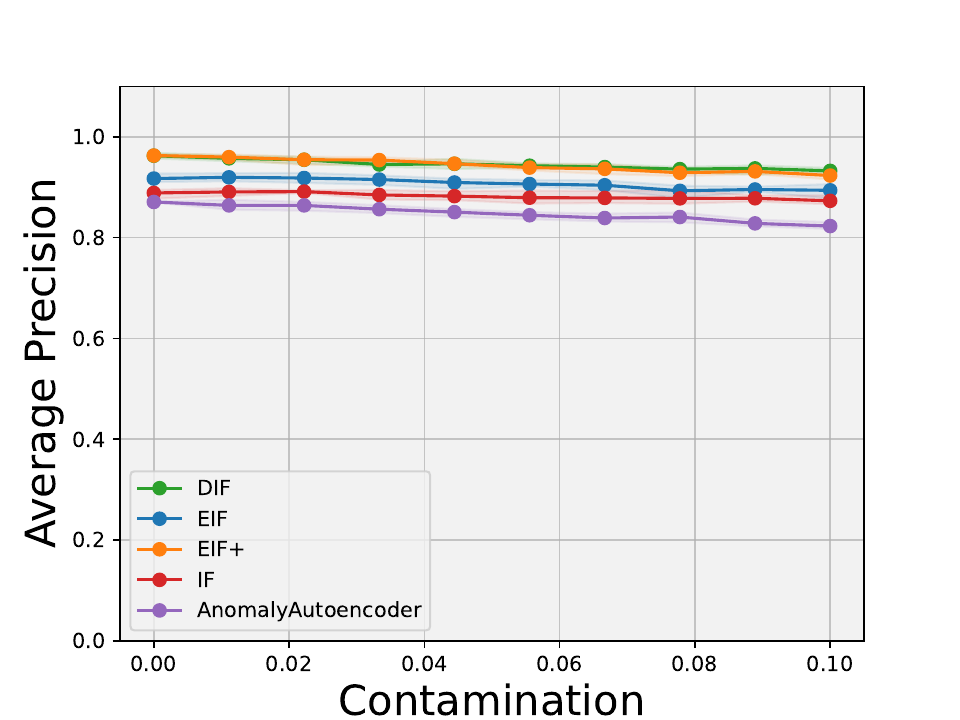}
      \caption{Models evaluation, varying the contamination levels}
      \label{fig:Ionosphere_contamination_full}
    \end{subfigure}\hfil % <-- added
    \begin{subfigure}[t]{0.44\textwidth}
      \includegraphics[width=\linewidth]{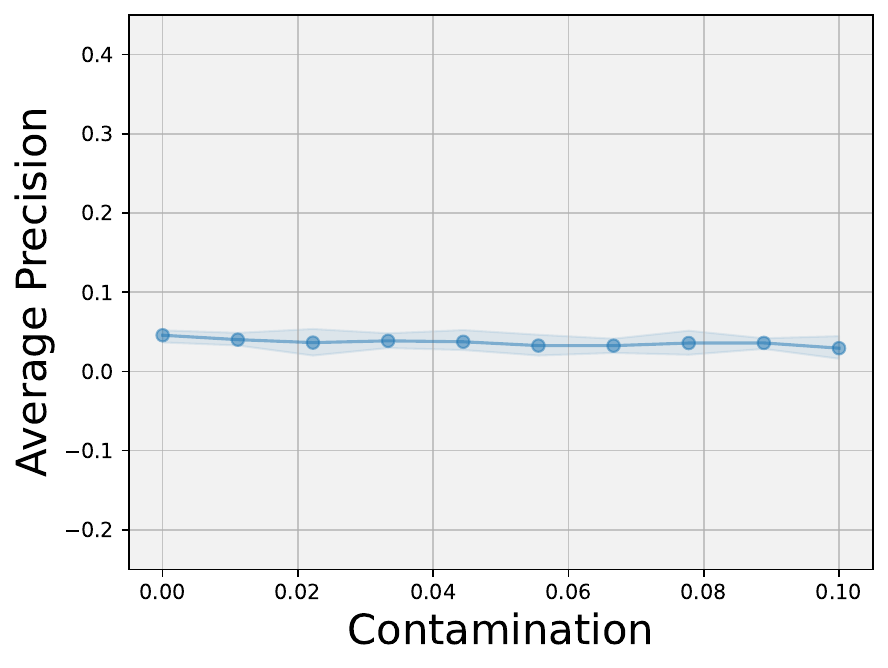}
      \caption{Difference between \EIFplus and EIF average precision}
      \label{fig:Ionosphere_contaminationEIFvsEIF+}
    \end{subfigure}\hfil % <-- added
\caption{Figure \ref{fig:Ionosphere_contamination_full} illustrates the average precision as the contamination level in the training set increases. Figure \ref{fig:Ionosphere_contaminationEIFvsEIF+} compares the performance graphs of EIF and \EIFplus, using the difference of their scores in various contamination levels.}
\label{fig:Ionosphere_contamination}
\end{figure}

\ale{As a result of a careful observations of Table \ref{tab:Ionosphere_perf}  it is possible to conclude that the optimal models for the Anomaly Detection task on the {\ttfamily Ionosphere} dataset are \EIFplus and DIF. The performances offered by these models are in fact  superior to the ones of all other methods but since \EIFplus demonstrates significantly improved efficiency during both the fitting and prediction phases it is the best choice in this scenario.}

\begin{table}[htbp]
\begin{minipage}[t]{0.46\textwidth}
\strut\vspace*{-\baselineskip}\newline
\resizebox{\textwidth}{!}{
\begin{tabular}{|c||ccc|ccc||cc|}
\toprule
\hline
&\multicolumn{3}{c|}{Scenario I}&\multicolumn{3}{c||}{Scenario II}&\multicolumn{2}{c|}{Time}\\
\hline
AD Model & Avg & Prec & ROC & Avg & Prec & ROC & fit & pred \\
& Prec &  & AUC & Prec &  & AUC &  &  \\
\hline
IF          & 0.79& 0.65& 0.73& 0.89& 0.79& 0.83& \textbf{0.05}& \textbf{0.0026}\\
EIF         & 0.82& 0.69& 0.76& 0.9& 0.82& 0.86& 0.14& 0.02\\
EIF+        & 0.84& 0.72& 0.78& 0.96& 0.87& 0.9& 0.11& 0.02\\
DIF         & \textbf{0.87}& \textbf{0.76}& \textbf{0.81}& \textbf{0.96}& \textbf{0.89}& \textbf{0.9}& 0.72& 0.44\\
AE & 0.76& 0.6& 0.68& 0.87& 0.75& 0.8& 2.26& 0.09\\
\hline
\end{tabular}}
\vspace{0.41cm}
\caption{Performances of 5 different Anomaly Detection models over {\ttfamily Ionosphere} are compared using classical Classification metrics. Moreover, the last two columns contain the average time for a fit and predict operation. The highest metric values and the lowest execution times are highlighted in bold}\label{tab:Ionosphere_perf}
\end{minipage}
\hfill
\begin{minipage}[t]{0.46\textwidth}
\strut\vspace*{-\baselineskip}\newline
\resizebox{\textwidth}{!}{
\begin{tabular}{|c||c|c|c|c||c|}
\toprule
\hline
&\multicolumn{2}{c|}{Evaluation with EIF}&\multicolumn{2}{c||}{Evaluation with \EIFplus}&\\
\hline
& Scenario I & Scenario II & Scenario I & Scenario II & Time\\

 Algorithm & $AUC_{FS}$  & $AUC_{FS}$ & $AUC_{FS}$  & $AUC_{FS}$ &  \\
\hline
DIFFI               & 2.367& -1.336& -1.135& 1.924& 0.31\\
IF\_\approach        & \textbf{3.294}& 0.891& \textbf{2.683}& 0.266& \textbf{0.16}\\
EIF\_\approach       & 1.828& \textbf{4.313}& 1.615& \textbf{2.841}& \textbf{0.16}\\
\EIFplus\_\approach  & 0.619& 2.268& 0.454& 1.410& 0.17\\
IF\_RF              & -1.914& -1.237& 1.762& -1.087& 0.60\\
EIF\_RF             & -1.975& 1.337& -1.857& 0.695& 0.60\\
EIF+\_RF            & -1.871& 3.586& -1.568& 2.171& 0.60\\
\hline
\end{tabular}}
\caption{Quantitative evaluation of the effectiveness of 6 different interpretation algorithms on {\ttfamily Ionosphere} through the $AUC_{FS}$ metric, introduced in \ref{sec:interpr_evaluat}. In the last column the average time taken by the different models to produce the importance scores is reported. The highest $AUC_{FS}$ and lowest Importance time values are highlighted in bold.}\label{tab:fs-tab-Ionosphere}
\end{minipage}
\end{table}

\subsubsection{Importance Plots}

\ale{In Figure \ref{fig:interpretation-Ionosphere} it is possible to see how challenging the task of interpreting the relevance of the features used by and AD model can be in the case of feature spaces of high dimensionality. As it can be in fact concluded observing both the Score Plots (Figures \ref{fig:Feat-imp-Ionosphere}, \ref{fig:Feat-imp-Ionosphere-split}) and the Bar Plots (Figures \ref{fig:GFI-Ionosphere}, \ref{fig:GFI-Ionosphere-split}) the importance is evenly shared across all features and it is daunting to find a single feature or a small subset of features whose relevance is significantly higher than the ones of the remaining attributes.} 

\begin{figure}[!ht] 
    \centering % <-- added
    \begin{subfigure}[t]{0.35\textwidth}
    \centering
      \includegraphics[width=\linewidth]{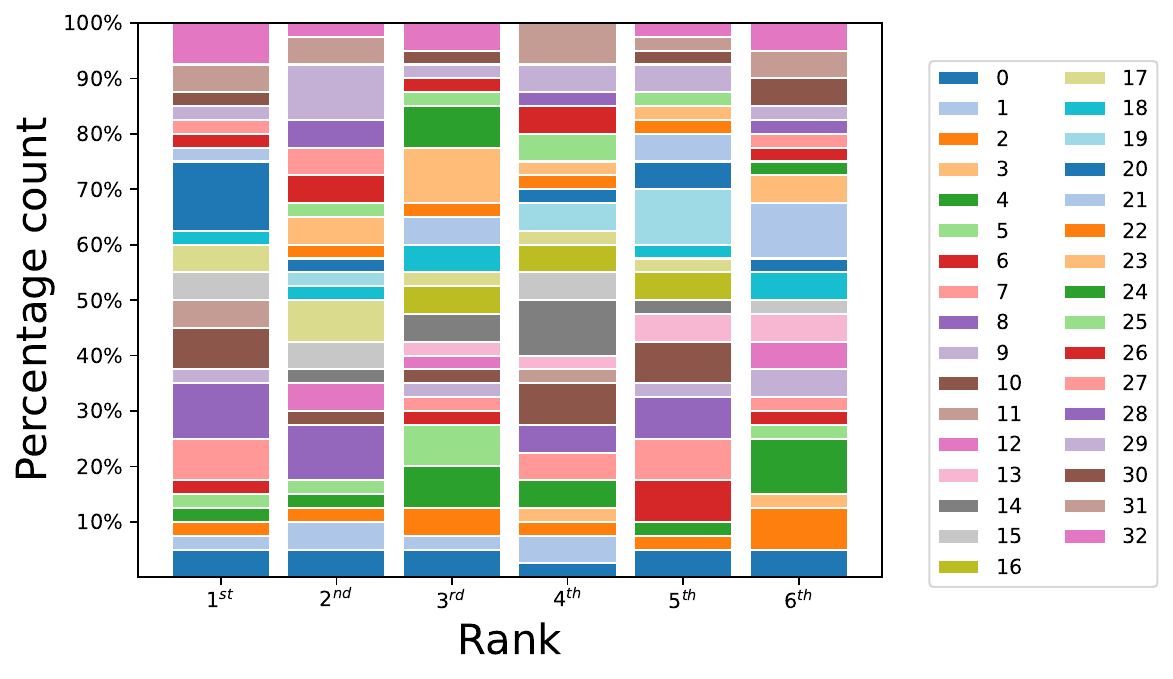}
      \caption{Bar Plot {\ttfamily Ionosphere} Scenario I}
      \label{fig:GFI-Ionosphere}
    \end{subfigure}\hfil % <-- added
    \begin{subfigure}[t]{0.25\textwidth}
    \centering
      \includegraphics[width=\linewidth]{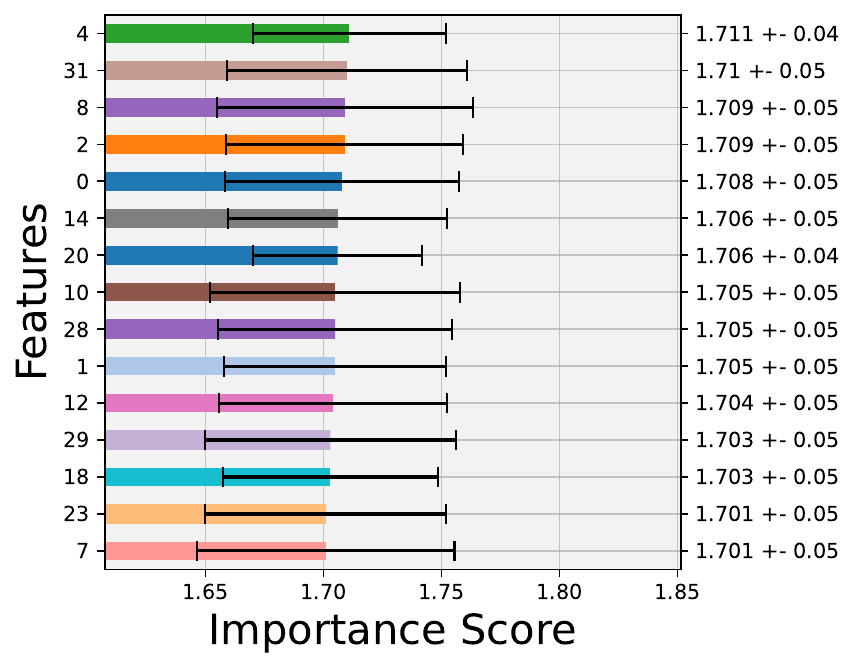}
      \caption{Score Plot {\ttfamily Ionosphere} Scenario I}
      \label{fig:Feat-imp-Ionosphere}
    \end{subfigure}\hfil % <-- added
    \begin{subfigure}[t]{0.28\textwidth}
    \centering
      \includegraphics[width=\linewidth]{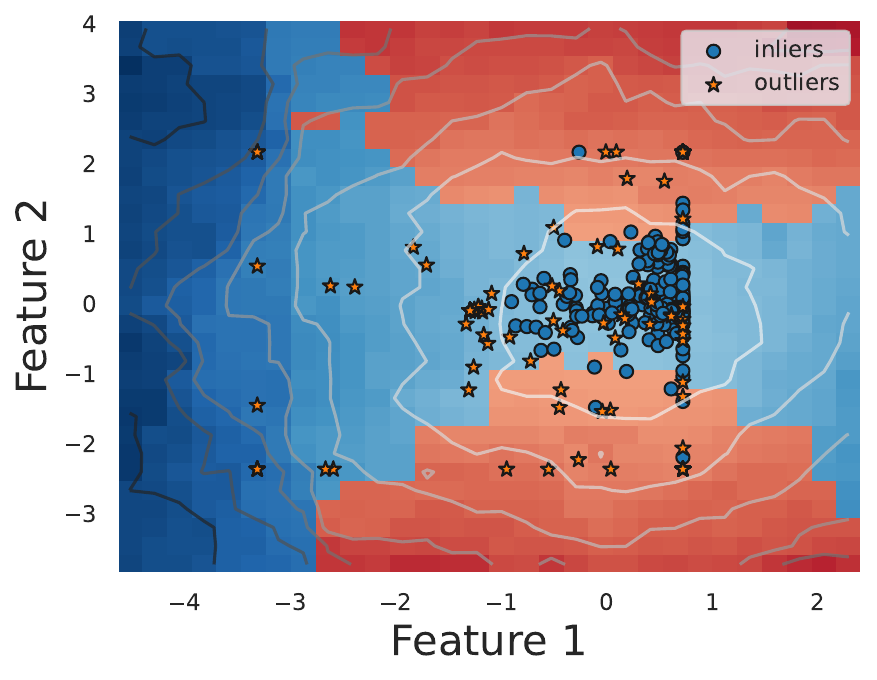}
      \caption{Scoremap {\ttfamily Ionosphere} Scenario I}
      \label{fig:Local-Ionosphere}
    \end{subfigure}\hfil % <-- added
    \begin{subfigure}[t]{0.35\textwidth}
    \centering
      \includegraphics[width=\linewidth]{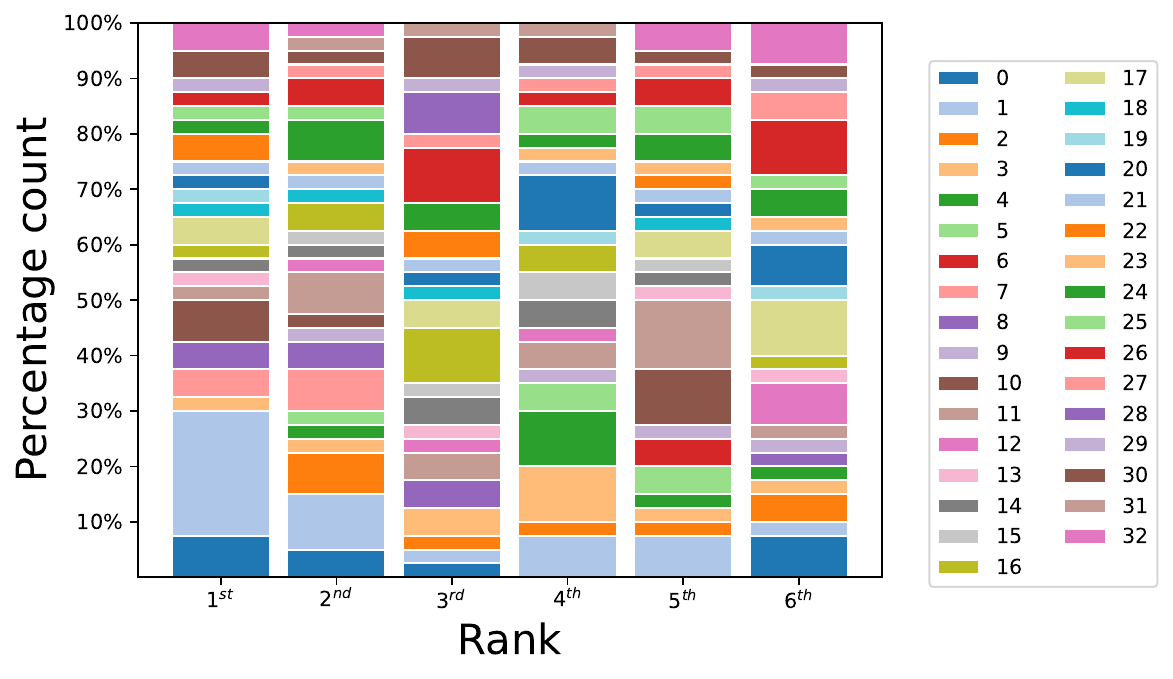}
      \caption{Bar Plot {\ttfamily Ionosphere} Scenario II}
      \label{fig:GFI-Ionosphere-split}
    \end{subfigure}\hfil % <-- added
    \begin{subfigure}[t]{0.25\textwidth}
    \centering
      \includegraphics[width=\linewidth]{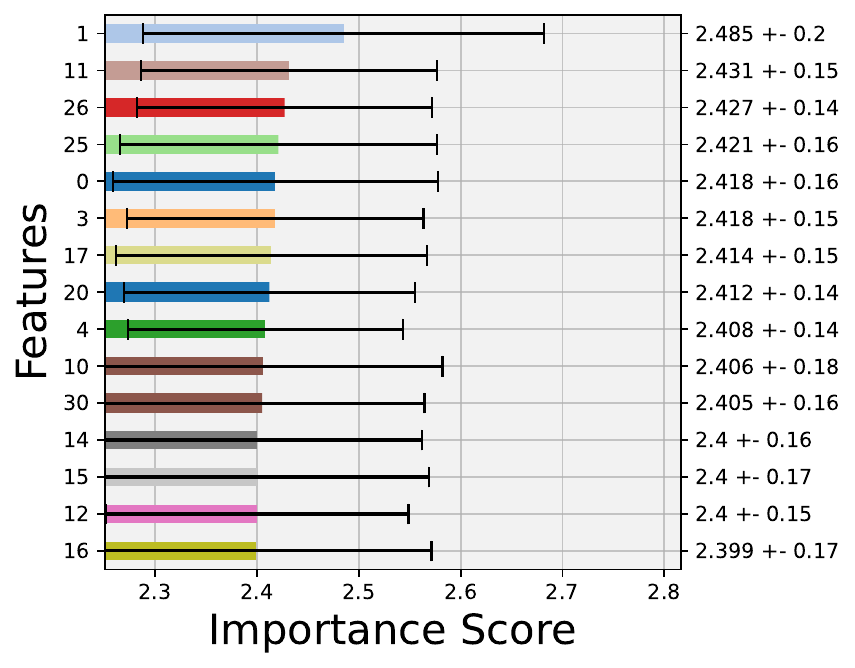}
      \caption{Score Plot {\ttfamily Ionosphere} Scenario II}
      \label{fig:Feat-imp-Ionosphere-split}
    \end{subfigure}\hfil % <-- added
    \begin{subfigure}[t]{0.28\textwidth}
    \centering
      \includegraphics[width=\linewidth]{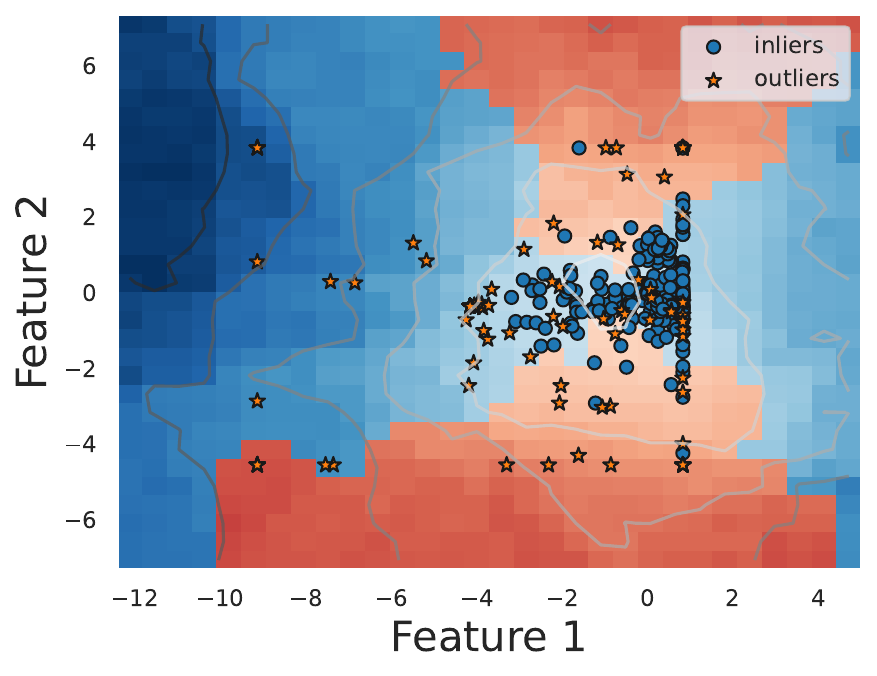}
      \caption{Scoremap {\ttfamily Ionosphere} Scenario II}
      \label{fig:Local-Ionosphere-split}
    \end{subfigure}\hfil % <-- added
\caption{Bar Plot, Score Plot and Scoremap for {\ttfamily Ionosphere} in the two different Scenarios, using the \approach algorithm applied to the \EIFplus model.}\label{fig:interpretation-Ionosphere}
\end{figure}

\subsubsection{Feature Selection}

\ale{The phenomenon observable in the Feature Selection plots of the {\ttfamily Ionosphere} (Figure \ref{fig:fs-interpretation-Diabetes}) dataset is similar to the one presented in section \ref{sec:Breastw}  for the {\ttfamily Breastw} dataset. Essentially since the importance is shared across a group of features the Average Precision follows a constant trend and starts to decrease as important features are progressively removed from the group of relevant attributes, as it can be noticed in Figure \ref{fig:Feat-Sel_Ionosphere_valEIF+_EXIFFI+_2}.}

\begin{figure}[!ht] 
\centering
\hspace{0.05\textwidth}\textbf{IF} \hspace{0.29\textwidth} \textbf{EIF} \hspace{0.29\textwidth} \textbf{EIF+}
% First row with vertical caption on the left
\begin{minipage}{\textwidth}
    \rotatebox{90}{\parbox{15mm}{\centering \textbf{Ad-Hoc}}} % Adjust the parbox width as necessary for your caption text
    \begin{minipage}{0.95\textwidth}
        \begin{subfigure}[t]{0.30\textwidth}
            \centering
            \includegraphics[trim={0 0 3.5cm 0}, clip, width=\linewidth]{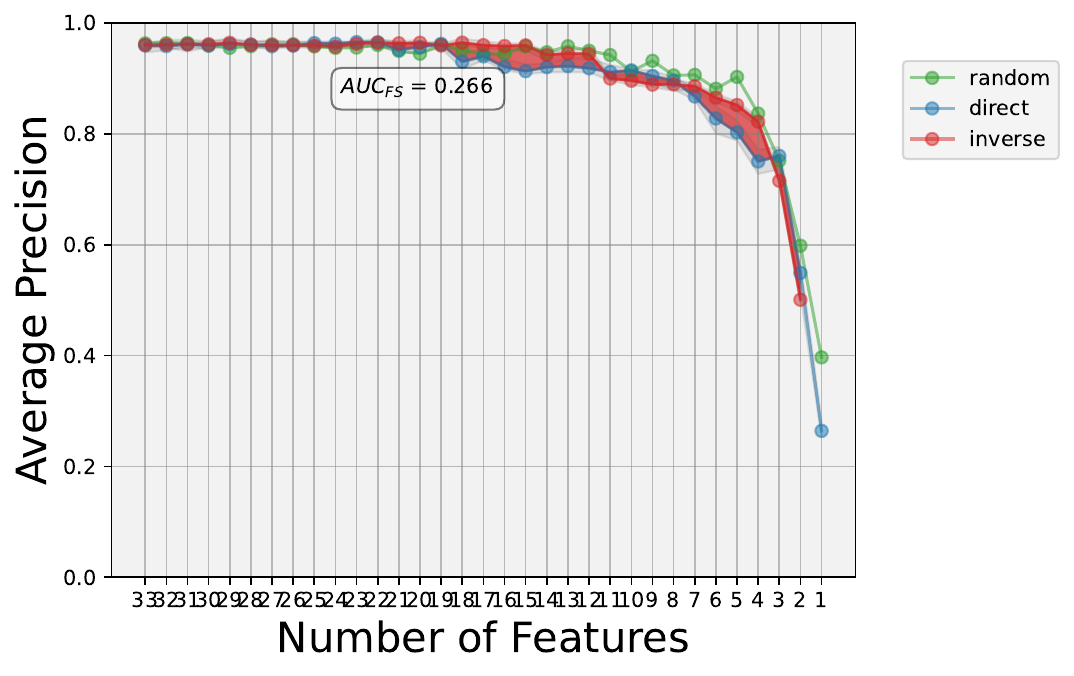}
            \caption{\approach applied to IF}
            \label{fig:Feat-Sel_Ionosphere_valEIF+_DIFFI_2}
        \end{subfigure}\hfill
        \begin{subfigure}[t]{0.30\textwidth}
            \centering
            \includegraphics[trim={0 0 3.5cm 0}, clip, width=\linewidth]{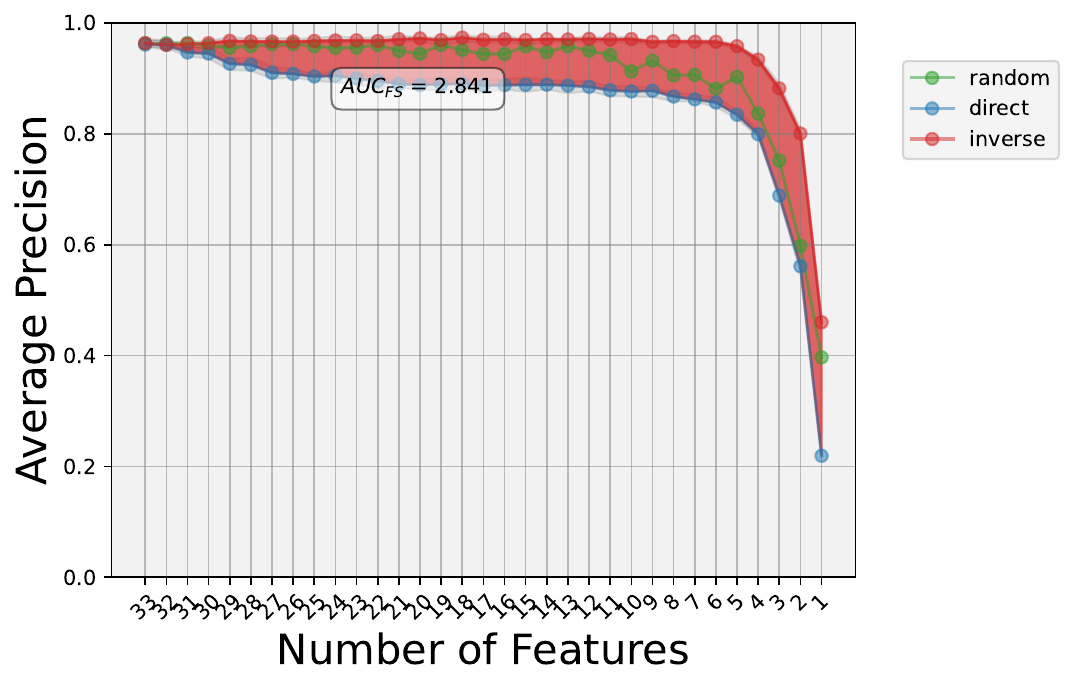}
            \caption{\approach applied to EIF}
            \label{fig:Feat-Sel_Ionosphere_valEIF+_EXIFFI_2}
        \end{subfigure}\hfill
        \begin{subfigure}[t]{0.30\textwidth}
            \centering
            \includegraphics[trim={0 0 3.5cm 0}, clip, width=\linewidth]{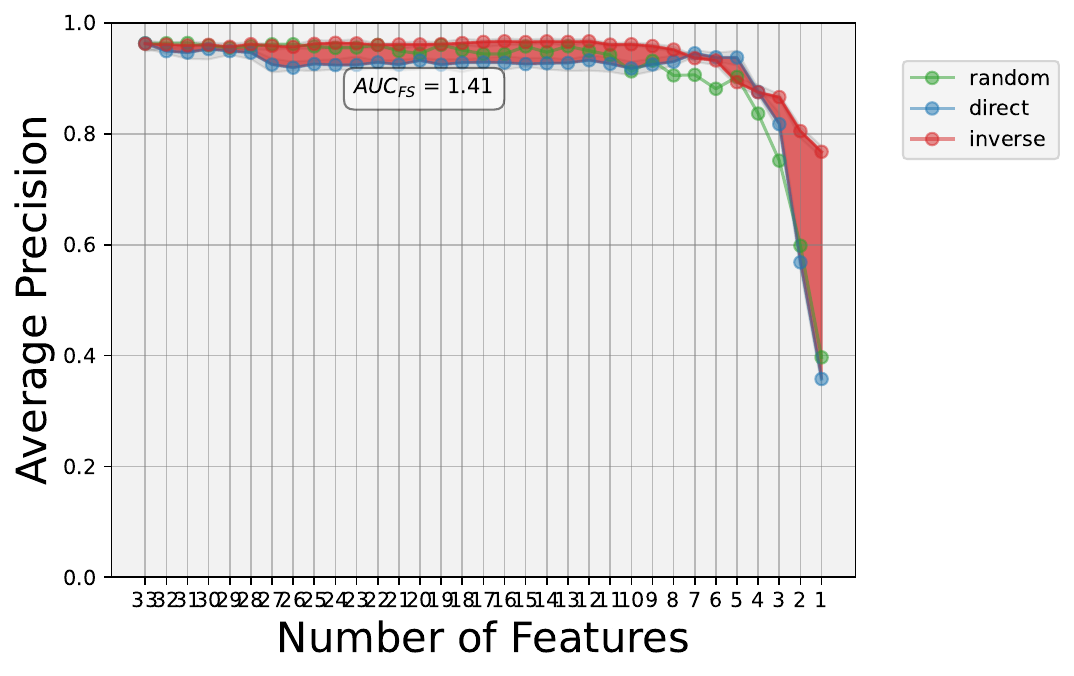}
            \caption{\approach applied to \EIFplus}
            \label{fig:Feat-Sel_Ionosphere_valEIF+_EXIFFI+_2}
        \end{subfigure}
    \end{minipage}
\end{minipage}

\vspace{5mm} % Space between rows

% Second row with vertical caption on the left
\begin{minipage}{\textwidth}
    \rotatebox{90}{\parbox{15mm}{\centering \textbf{Post-Hoc}}} % Adjust as necessary
    \begin{minipage}{0.95\textwidth}
        \begin{subfigure}[t]{0.30\textwidth}
            \centering
            \includegraphics[trim={0 0 3.5cm 0}, clip, width=\linewidth]{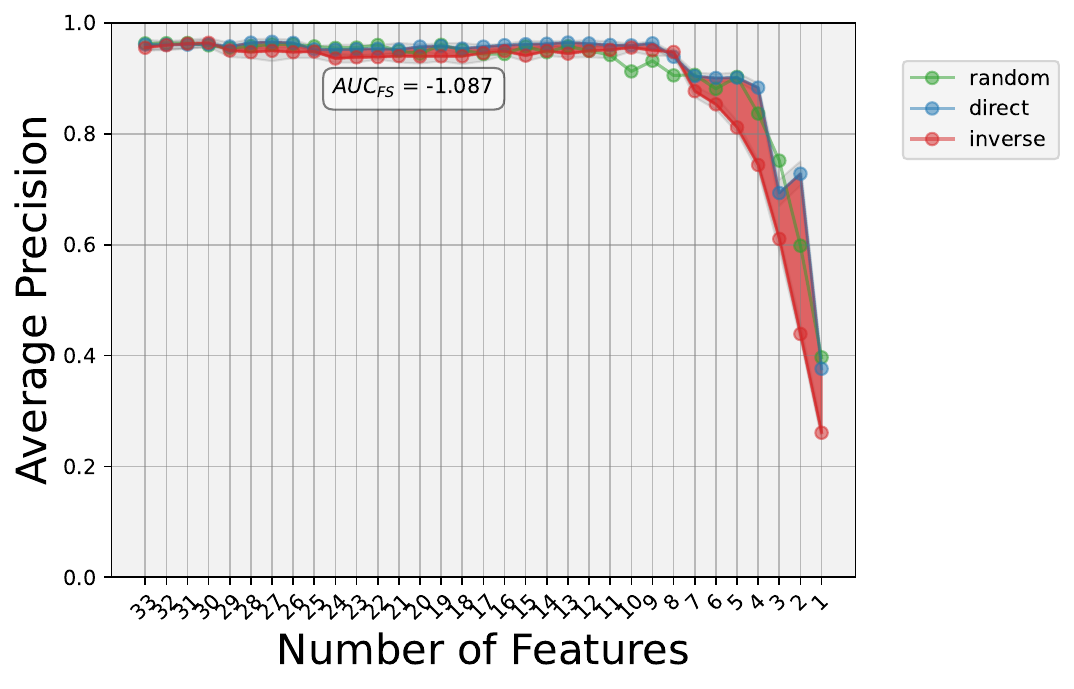}
            \caption{RandomForest fitted to IF}
            \label{fig:Feat-Sel_Ionosphere_valEIF+_IF_RandomForest_2}
        \end{subfigure}\hfill
        \begin{subfigure}[t]{0.30\textwidth}
            \centering
            \includegraphics[trim={0 0 3.5cm 0}, clip, width=\linewidth]{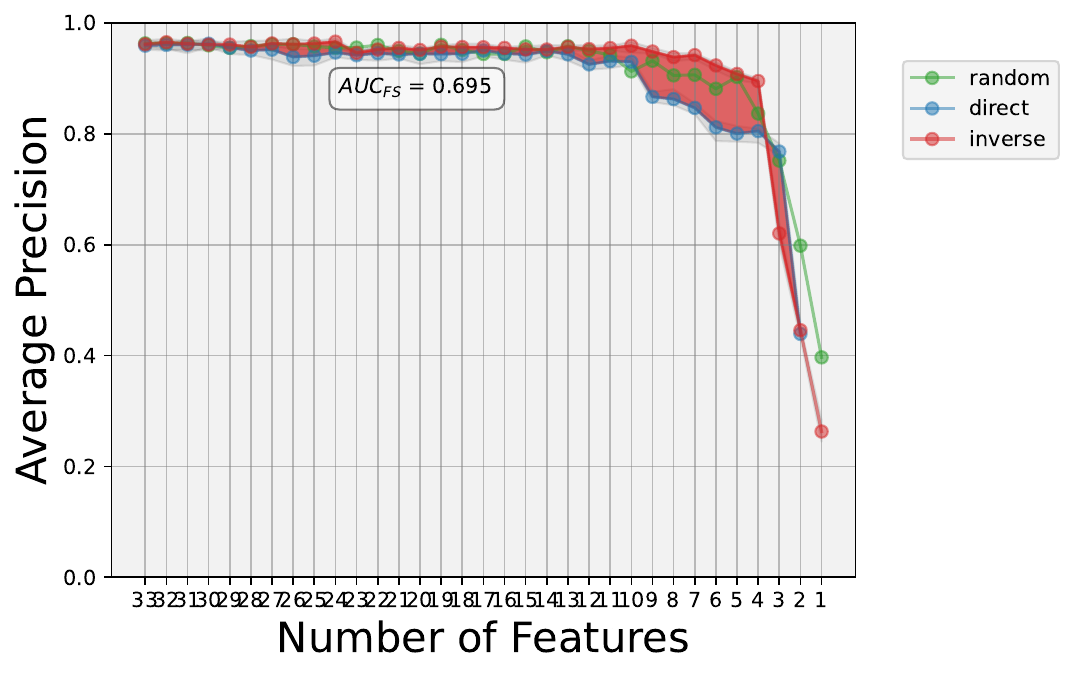}
            \caption{RandomForest fitted to EIF}
            \label{fig:Feat-Sel_Ionosphere_valEIF+_EIF_RandomForest_2}
        \end{subfigure}\hfill
        \begin{subfigure}[t]{0.30\textwidth}
            \centering
            \includegraphics[trim={0 0 3.5cm 0}, clip, width=\linewidth]{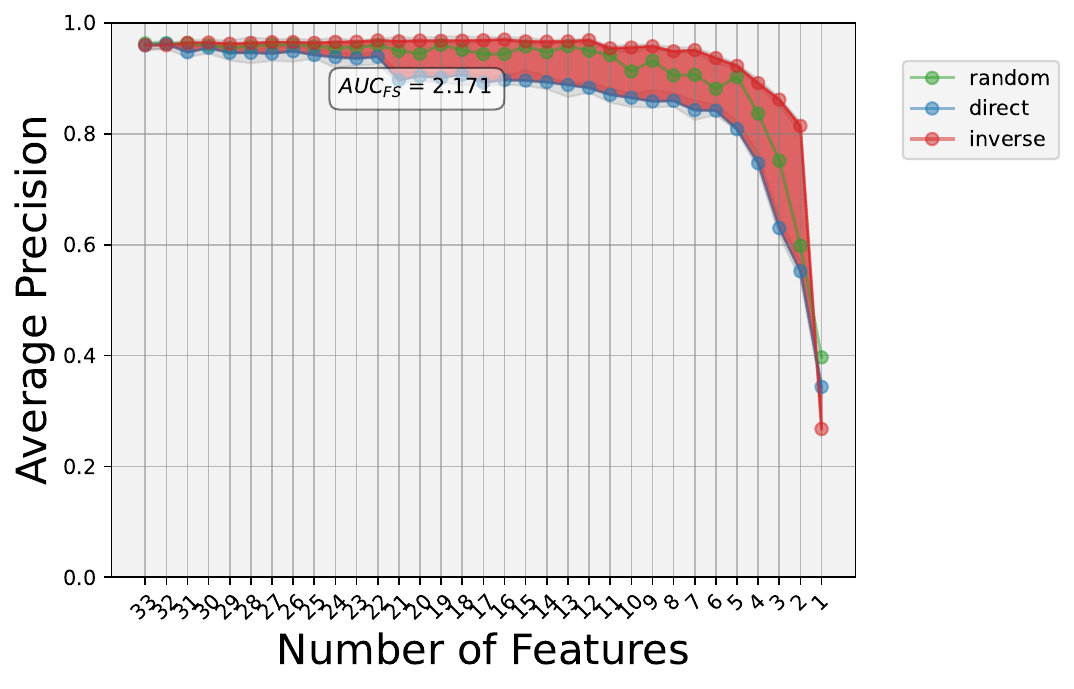}
            \caption{RandomForest fitted to \EIFplus}
            \label{fig:Feat-Sel_Ionosphere_valEIF+_EIF+_RandomForest_2}
        \end{subfigure}
    \end{minipage}
\end{minipage}

\caption{Feature Selection of the different Ad-Hoc and Post-Hoc methods applied to the 3 Isolation Forest models: IF, EIF and \EIFplus. The blue line is the values of average precision, calculated with the \EIFplus model in the Scenario II, dropping the most important feature at each step, the red line is the values of average precision dropping the least important feature at each step and the green line is the value of the feature selection dropping a random feature at each step.}\label{fig:fs-interpretation-Ionosphere}
\end{figure}

\ale{Table \ref{tab:fs-tab-Ionosphere} lists the values of the $AUC_{FS}$ metric in Scenario I and Scenario II. The only interpretation models able to provide a feature ranking correctly aligning with the dataset's characteristics are \approach, \approach+ and the post-hoc Random Forest model applied to the \EIFplus AD method. Among these two the most efficient one in terms of computational time is \approach+.}

\subsection*{{\ttfamily Moodify}}

% Additional comment to satisfy comment 7 by reviewer 2 and Comment 11 of reviewer 1 
\davide{The final datasets considered for the evaluation of the quality of the explanations is the {\ttfamily moodify} datasets, introduced in \ref{sec:appendix-real-world-data}. Converting this dataset in order to make it suitable for the Anomaly Detection task corresponds to distinguish \textit{calm} Spotify tracks from the rest. Thus, similarly to the {\ttfamily glass} dataset \ref{sec:glass}, it is possible to compare the conclusions reached by the model (i.e. \approach) with human intuition on what are the most relevent features to perform the previously cited distinction.} 

\subsubsection{Performance}
In the contamination plot \ref{fig:Moodify_contamination_full}, it's evident that all models perform better when there are no anomalies in the training data (contamination=0), with the DIF model showing the most significant improvement. Although the \EIFplus does not consistently yield high performance, it surpasses EIF in scenarios where it is trained exclusively on inliers, as anticipated. This trend is depicted in the plot comparing the performance differences between \EIFplus and EIF in Figure \ref{fig:Moodify_contaminationEIFvsEIF+}, illustrating \EIFplus's enhanced ability to adapt and identify anomalies when trained on a clean dataset.\ref{fig:Moodify_contaminationEIFvsEIF+}.

\begin{figure}[!ht] 
    \centering % <-- added
    \begin{subfigure}[t]{0.49\textwidth}
      \includegraphics[width=\linewidth]{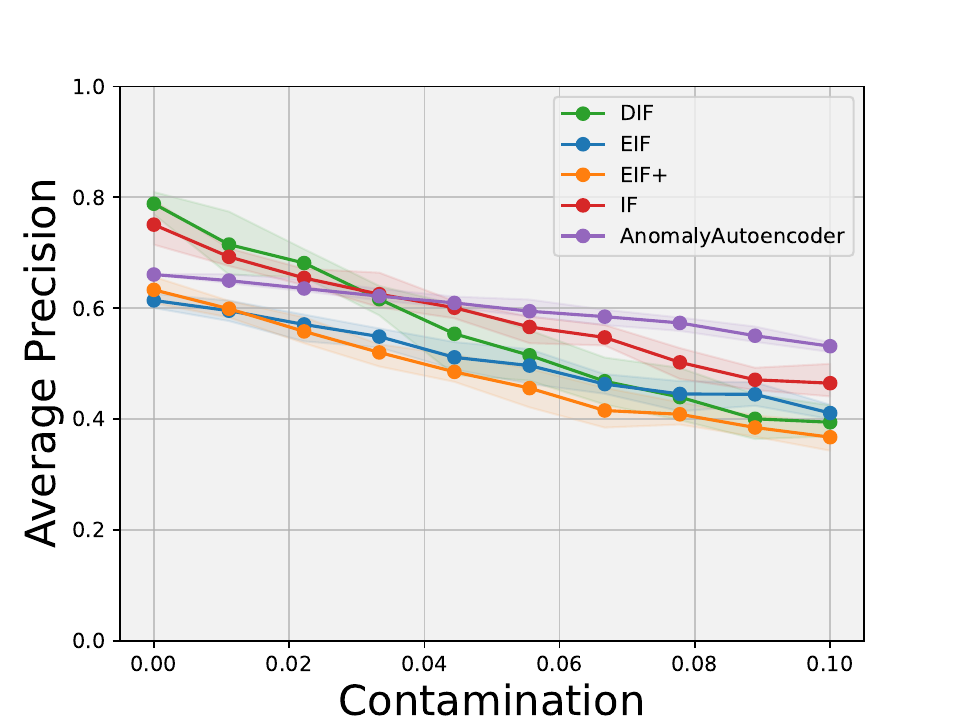}
      \caption{Models evaluation, varying the contamination levels}
      \label{fig:Moodify_contamination_full}
    \end{subfigure}\hfil % <-- added
    \begin{subfigure}[t]{0.44\textwidth}
      \includegraphics[width=\linewidth]{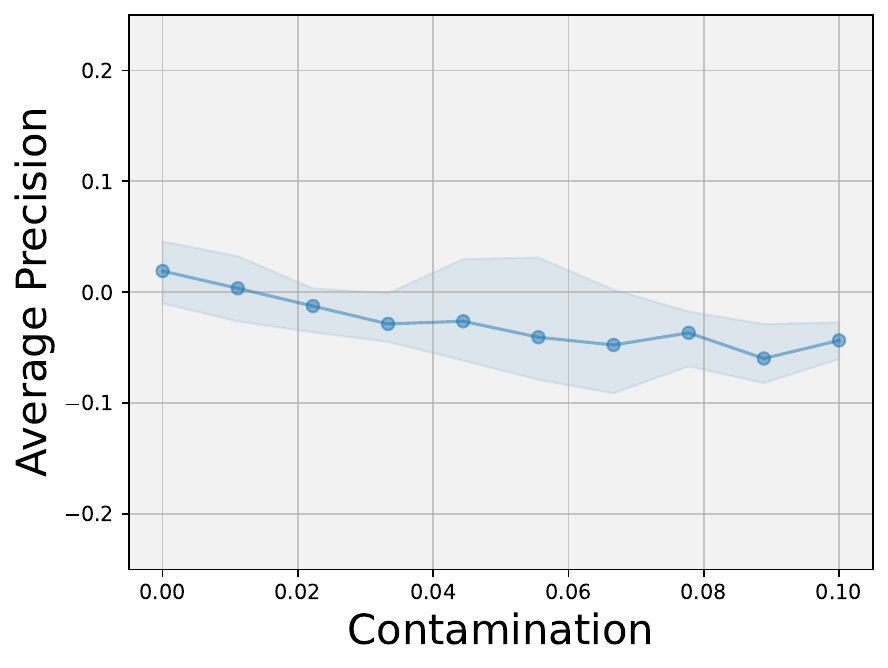}
      \caption{Difference between \EIFplus and EIF average precision}
      \label{fig:Moodify_contaminationEIFvsEIF+}
    \end{subfigure}\hfil % <-- added
\caption{Figure \ref{fig:Moodify_contamination_full} illustrates the average precision as the contamination level in the training set increases. Figure \ref{fig:Moodify_contaminationEIFvsEIF+} compares the performance graphs of EIF and \EIFplus, using the difference of their scores in various contamination levels.}
\label{fig:Moodify_contamination}
\end{figure}

Table \ref{tab:performance_moodify} provides detailed insights into the performance metrics of the models. 

Although both the DIF and the IF model achieves the highest value of Average Precision in Scenario II, as reported in the performance table,  the DIF proves to be significantly slower in the fitting and predicting operations compared to the IF method.

%This indicates that the DIF model fails to identify a significant number of actual anomalies within the dataset. 
\begin{table}[htbp]
\centering
%\caption{{\ttfamily Moodify} Precision Report}
\caption{Performances of 5 different Anomaly Detection models over {\ttfamily Moodify} are compared using classical Classification metrics. Moreover, the last two columns contain the average time for a fit and predict operation. The highest metric values and the lowest execution times are highlighted in bold}\label{tab:performance_moodify}
\begin{tabular}{|c||ccc|ccc||cc|}
\toprule
\hline
& \multicolumn{3}{c|}{Scenario I} & \multicolumn{3}{c||}{Scenario II} & \multicolumn{2}{c|}{Time} \\
\hline
AD Model& Avg & Prec & ROC & Avg & Prec & ROC & fit & pred \\
 & Prec &  & AUC & Prec &  & AUC &  &  \\
\hline
IF          & 0.35 & 0.30 & 0.59 & \textbf{0.72}& \textbf{0.73}& \textbf{0.84}& 0.11 & \textbf{0.05}\\
EIF         & 0.33 & 0.37 & 0.63 & 0.65 & 0.64 & 0.79 & \textbf{0.09}& 0.27  \\
\EIFplus        & 0.28 & 0.27 & 0.57 & 0.66 & 0.66 & 0.80 & \textbf{0.09}& 0.25 \\
DIF         & 0.26& 0.26& 0.56& \textbf{0.72}& \textbf{0.73}& \textbf{0.84}& 7.76 & 7.5  \\
AE & \textbf{0.45}& \textbf{0.53}& \textbf{0.72}& 0.65& 0.68& 0.81& 16.6 & 0.26 \\
\hline
\end{tabular}
\end{table}

Consequently, the consistent results demonstrated by the IF model make it a more reliable choice in this scenario, balancing the ability to detect anomalies with computational efficiency. %fewer misses 

The outcomes for Scenario I significantly diverge from those observed at a contamination level of 0.1, as depicted in plot \ref{fig:Moodify_contamination_full}. In Scenario I, the contamination level inherent to the dataset, 0.1527, is specifically considered. Notably, in this context, the Anomaly Autoencoder exhibits very low sensitivity to changes in the training dataset's contamination level compared to the other models.

\subsubsection{Importance Plots}

The importance plots in Scenario I, depicted in Figures \ref{fig:Feat-imp-Moodify}, highlight four features that significantly characterize the anomalies of the dataset, in particular the ``speechliness" and the ``duration", suggesting that the dataset includes unique song types. These variations may point to specific genres such as instrumental music or tracks of atypical lengths, like podcasts or classical music, that stand out from standard musical distributions.

In contrast, Scenario II sheds light on the characteristics that set the outlier class separates from the general dataset distribution. Specifically, the 'loudness' feature, which measures a track's overall volume in decibels (dB), as explained in the Appendix \ref{sec:appendix-real-world-data}, is identified as particularly significant in Figure \ref{fig:Feat-imp-Moodify-split}. This observation is consistent with the expectation that 'Calm' music tracks, the ones labelled as outliers, exhibit lower dB levels. The local scoremap presented in Figure \ref{fig:interpretation-Moodify} provides further insight, demonstrating how 'Calm' tracks distinctly deviate based on this feature, thus reinforcing the importance of 'loudness' in distinguishing these outliers within the dataset.

\begin{figure}[!ht] 
    \centering % <-- added
    \begin{subfigure}[t]{0.38\textwidth}
    \centering
      \includegraphics[width=\linewidth]{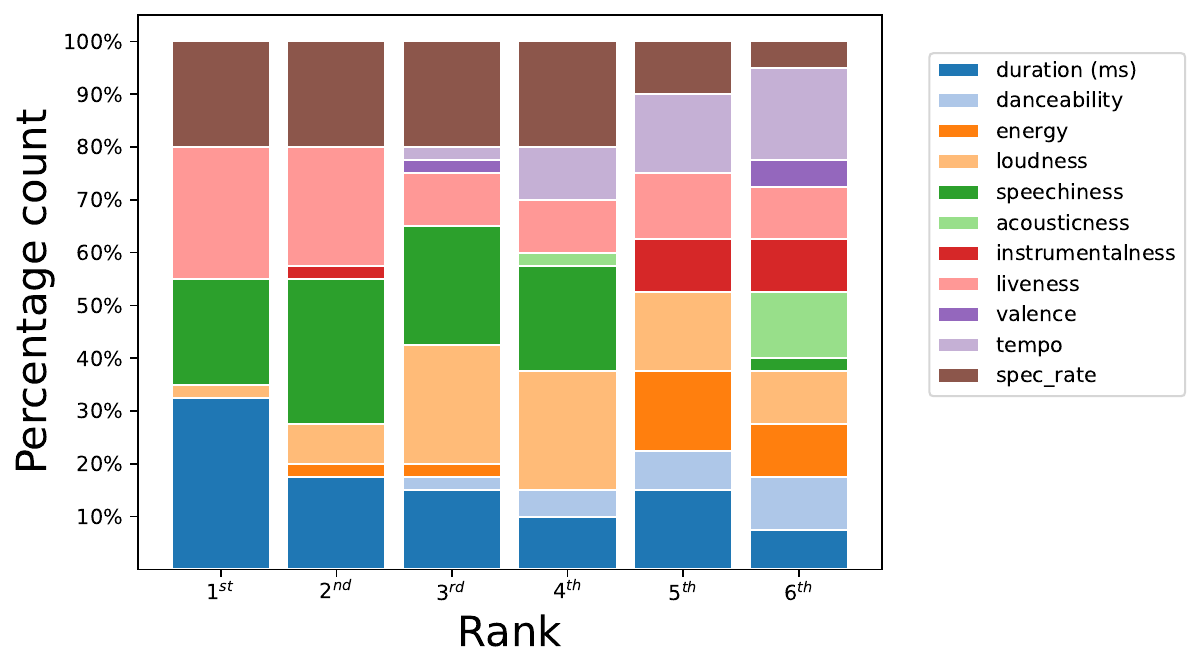}
      \caption{Score Plot {\ttfamily Moodify} Scenario I}
      \label{fig:Feat-imp-Moodify}
    \end{subfigure}\hfil % <-- added
    \begin{subfigure}[t]{0.32\textwidth}
    \centering
      \includegraphics[width=\linewidth]{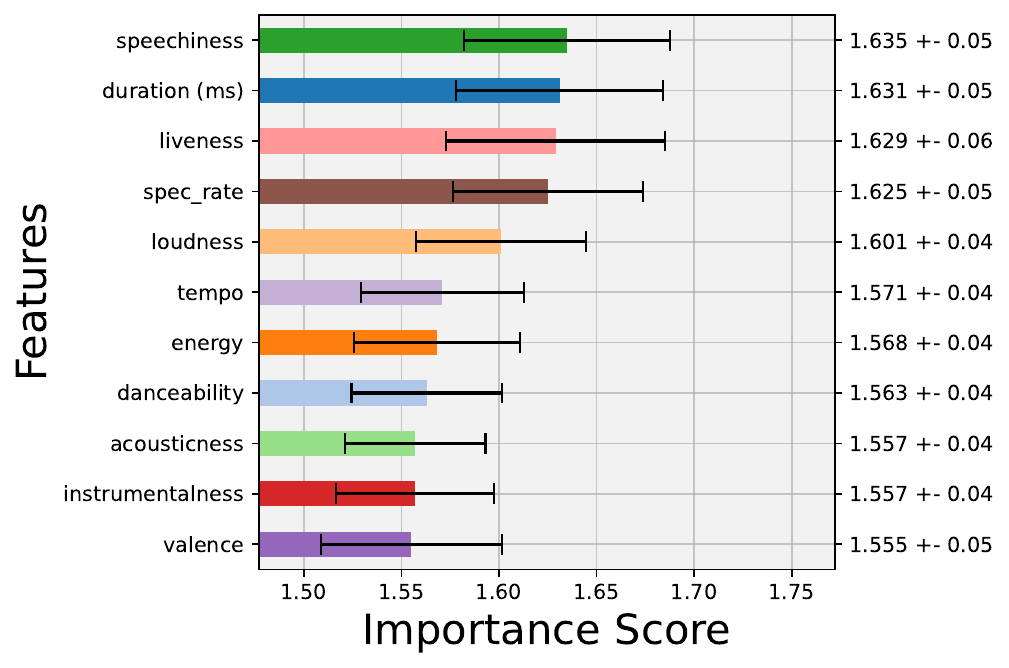}
      \caption{Bar Plot {\ttfamily Moodify} Scenario I}
      \label{fig:GFI-Moodify}
    \end{subfigure}\hfil % <-- added
    \begin{subfigure}[t]{0.28\textwidth}
    \centering
      \includegraphics[width=\linewidth]{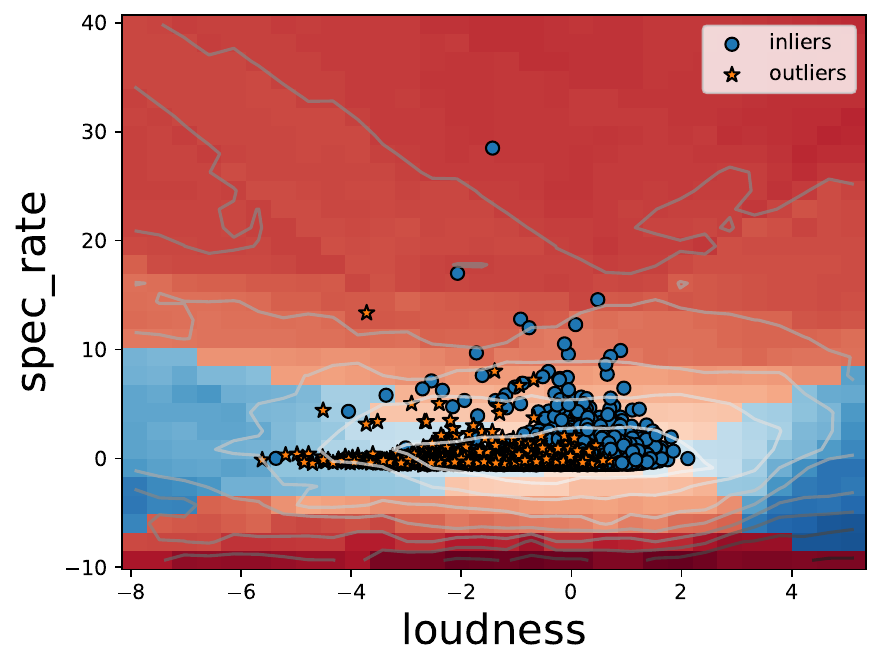}
      \caption{Scoremap {\ttfamily Moodify} Scenario I}
      \label{fig:Local-Moodify}
    \end{subfigure}\hfil % <-- added
    \begin{subfigure}[t]{0.35\textwidth}
    \centering
      \includegraphics[width=\linewidth]{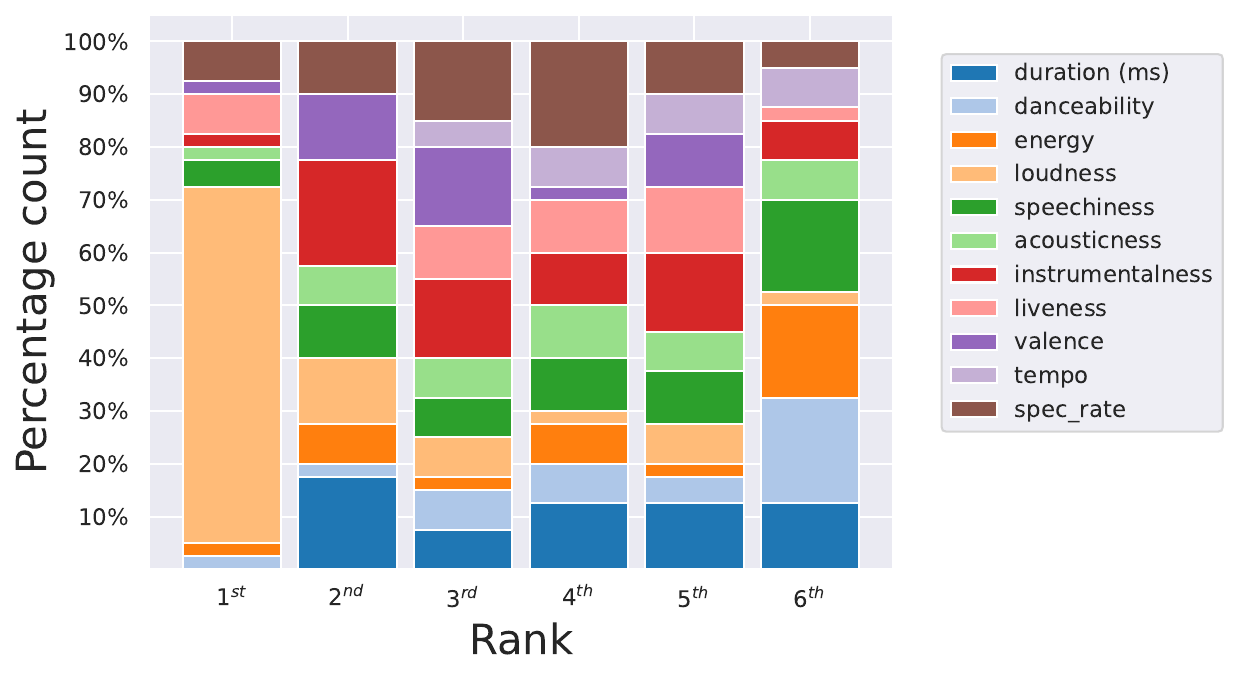}
      \caption{Score Plot {\ttfamily Moodify} Scenario II}
      \label{fig:Feat-imp-Moodify-split}
    \end{subfigure}\hfil % <-- added
    \begin{subfigure}[t]{0.30\textwidth}
    \centering
      \includegraphics[width=\linewidth]{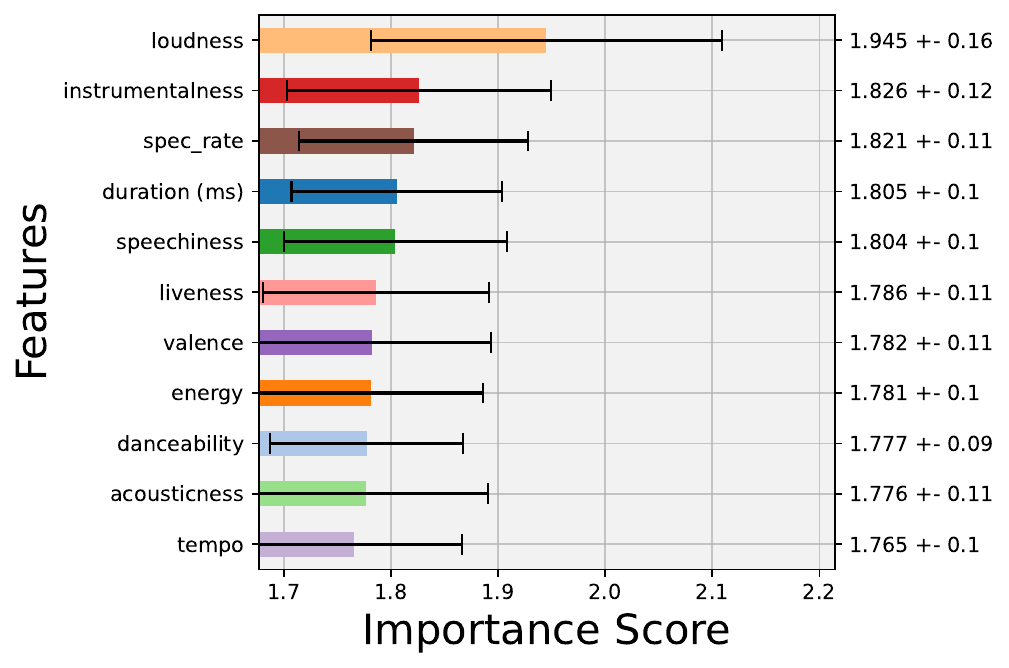}
      \caption{Bar Plot {\ttfamily Moodify} Scenario II}
      \label{fig:GFI-Moodify-split}
    \end{subfigure}\hfil % <-- added
    \begin{subfigure}[t]{0.28\textwidth}
    \centering
      \includegraphics[width=\linewidth]{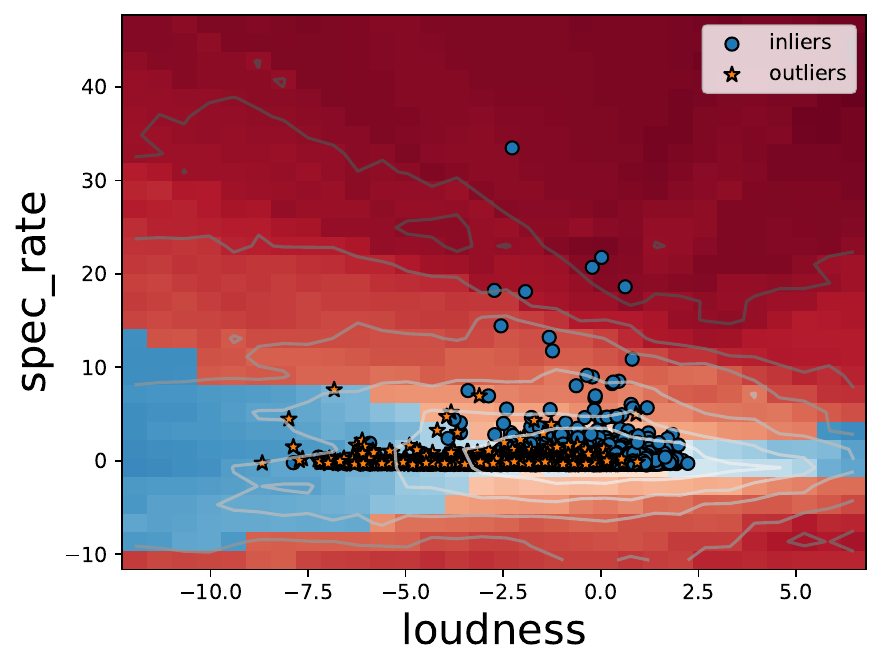}
      \caption{Scoremap {\ttfamily Moodify} Scenario II}
      \label{fig:Local-Moodify-split}
    \end{subfigure}\hfil % <-- added
\caption{Bar Plot, Score Plot and Scoremap for {\ttfamily Moodify}  in the two different Scenarios, using the \approach algorithm applied to the \EIFplus model.}\label{fig:interpretation-Moodify}
\end{figure}

\subsubsection{Feature Selection}

The Feature Selection plots grouped in \ref{fig:feature_selections-Moodify} outline a similar behavior, all showing positive values of the $AUC_{FS}$ metric. 

Both the EIF and \EIFplus models, when analyzed through ad-hoc and post-hoc interpretation methods, achieve high scores. They demonstrate a similar trend of improved average precision as the dataset is condensed to its most significant dimensions. This indicates that both interpretation algorithms, regardless of the interpretation method applied, are adept at distilling essential information, thereby enhancing their predictive accuracy when focusing on the most important features.

However, the application of \approach to the IF model (Figure \ref{fig:Feat-Sel_Moodify_valIF_EXIFFI_2}) stands out as the best interpretability approach for the {\ttfamily moodify} dataset. The main difference with the respect to the other methods can be observed in the Average Precision trend depicted in the blue curve, representing the approach of removing features in increasing order of relevance, that is associated with a clear decreasing behavior. On the other hand, in the other approaches the aforementioned curve presents an oscillating trend, consequence of a feature importance ranking not perfectly aligned with the ground truth. 

\begin{comment}
During the Feature Selection process, it becomes evident that the DIFFI algorithm struggles to accurately identify the most critical features, leading to bad performance when the feature selection evaluate the model using the most important features according to this interpretation method and , thus, yielding to a negative value of the $AUC_{FS}$ metric. Conversely, utilizing Random Forest as a surrogate model for interpreting the IF model's results yields better performance, showcasing its effectiveness in feature importance evaluation.
\end{comment}

\begin{figure}[!ht] 
\centering
\textbf{IF} \hspace{0.25\textwidth} \textbf{EIF} \hspace{0.25\textwidth} \textbf{\EIFplus}
% First row with vertical caption on the left
\begin{minipage}{\textwidth}
    \rotatebox{90}{\parbox{15mm}{\centering \textbf{Ad-Hoc}}} % Adjust the parbox width as necessary for your caption text
    \begin{minipage}{0.90\textwidth}
        \begin{subfigure}[t]{0.30\textwidth}
            \centering
            \includegraphics[trim={0 0 3.5cm 0}, clip, width=\linewidth]{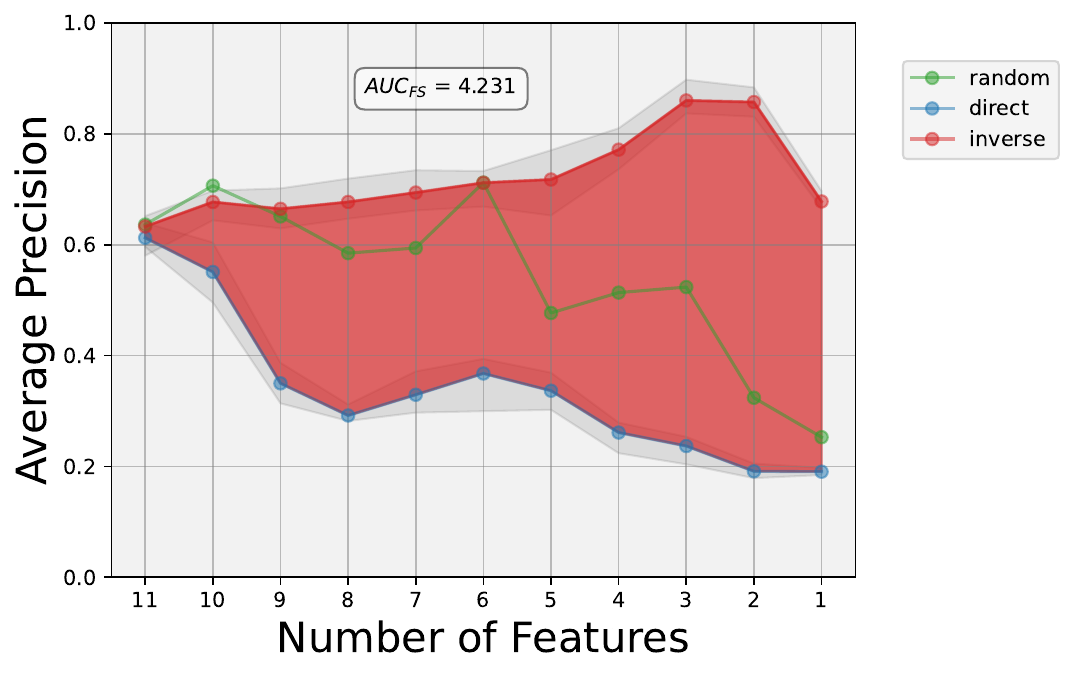}
            \caption{\approach applied to IF}
            \label{fig:Feat-Sel_Moodify_valIF_EXIFFI_2}
        \end{subfigure}\hfill
        \begin{subfigure}[t]{0.30\textwidth}
            \centering
            \includegraphics[trim={0 0 3.5cm 0}, clip, width=\linewidth]{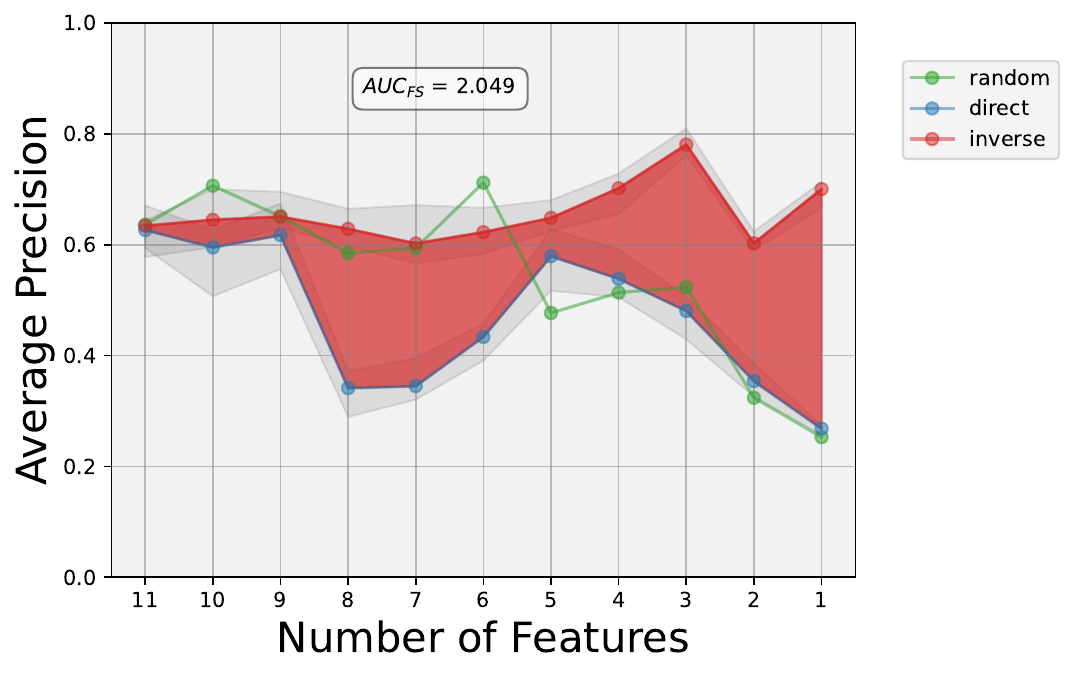}
            \caption{\approach applied to EIF}
            \label{fig:Feat-Sel_Moodify_valEIF+_EXIFFI_2}
        \end{subfigure}\hfill
        \begin{subfigure}[t]{0.30\textwidth}
            \centering
            \includegraphics[trim={0 0 3.5cm 0}, clip, width=\linewidth]{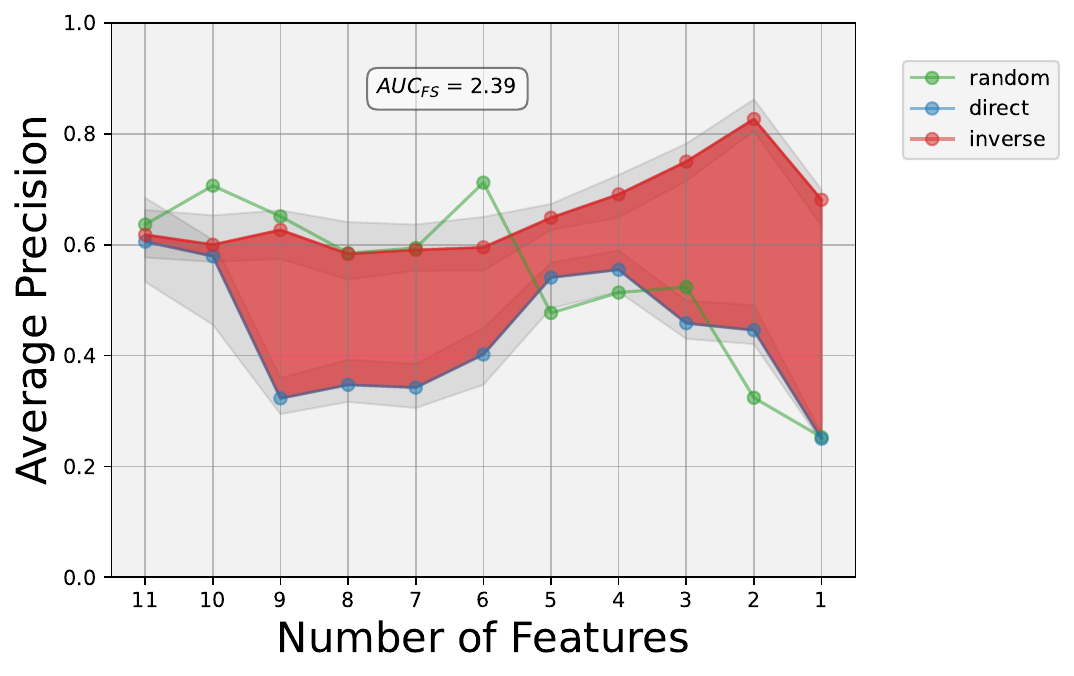}
            \caption{\approach applied to \EIFplus}
            \label{fig:Feat-Sel_Moodify_valEIF+_EXIFFI+_2}
        \end{subfigure}
    \end{minipage}
\end{minipage}

\vspace{5mm} % Space between rows

% Second row with vertical caption on the left
\begin{minipage}{\textwidth}
    \rotatebox{90}{\parbox{15mm}{\centering \textbf{Post-Hoc}}} % Adjust as necessary
    \begin{minipage}{0.90\textwidth}
        \begin{subfigure}[t]{0.30\textwidth}
            \centering
            \includegraphics[trim={0 0 3.5cm 0}, clip, width=\linewidth]{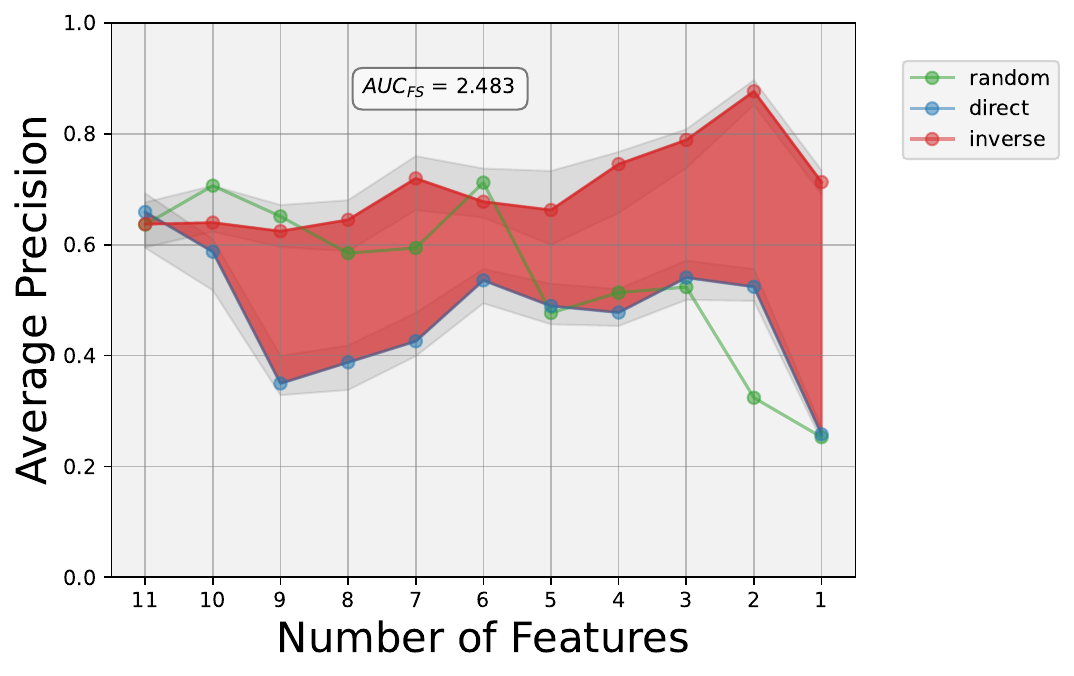}
            \caption{RandomForest applied to IF}
            \label{fig:Feat-Sel_Moodify_valEIF+_IF_RandomForest_2}
        \end{subfigure}\hfill
        \begin{subfigure}[t]{0.30\textwidth}
            \centering
            \includegraphics[trim={0 0 3.5cm 0}, clip, width=\linewidth]{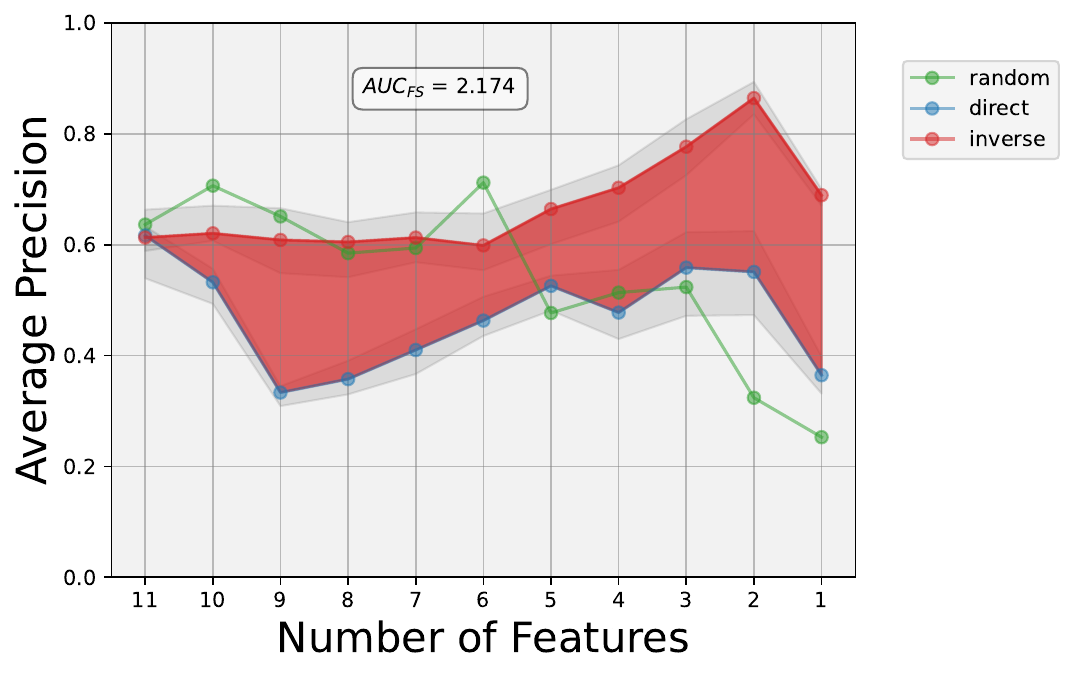}
            \caption{RandomForest applied to EIF}
            \label{fig:Feat-Sel_Moodify_valEIF+_EIF_RandomForest_2}
        \end{subfigure}\hfill
        \begin{subfigure}[t]{0.30\textwidth}
            \centering
            \includegraphics[trim={0 0 3.5cm 0}, clip, width=\linewidth]{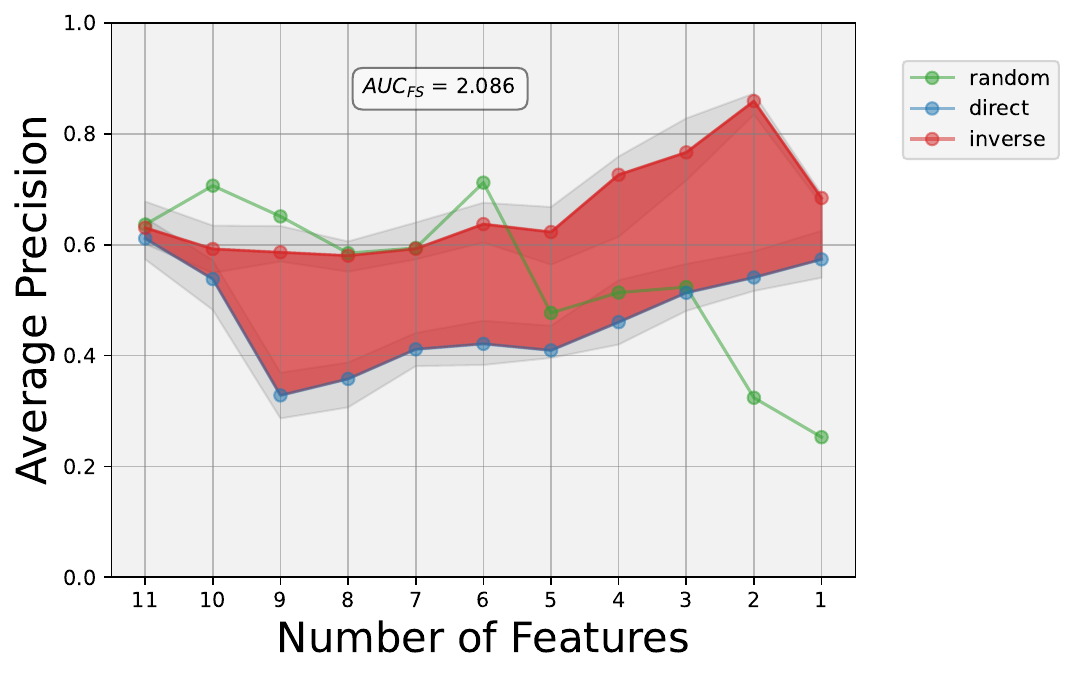}
            \caption{RandomForest applied to \EIFplus}
            \label{fig:Feat-Sel_Moodify_valEIF+_EIF+_RandomForest_2}
        \end{subfigure}
    \end{minipage}
\end{minipage}
\caption{Feature Selection of the different Ad-Hoc and Post-Hoc methods applied to the 3 Isolation Forest models: IF, EIF and \EIFplus. The blue line is the values of average precision, calculated with the \EIFplus model in the Scenario II, dropping the most important feature at each step, the red line is the values of average precision dropping the least important feature at each step and the green line is the value of the feature selection dropping a random feature at each step.}\label{fig:feature_selections-Moodify}
\end{figure}

\begin{table}[htbp]
\centering
%\caption{Feature Selection Scores {\ttfamily moodify}}
\caption{Quantitative evaluation of the effectiveness of 6 different interpretation algorithms on {\ttfamily Moodify} through the $AUC_{FS}$ metric, introduced in \ref{sec:interpr_evaluat}. In the last column the average time taken by the different models to produce the importance scores is reported. The highest $AUC_{FS}$ and lowest Importance time values are highlighted in bold.}\label{tab:fs-tab-moodify}
\begin{tabular}{|c||c|c|c|c||c|}
\toprule
\hline
&\multicolumn{2}{c|}{Evaluation with EIF}&\multicolumn{2}{c||}{Evaluation with \EIFplus}&\\
\hline
& Scenario I & Scenario II & Scenario I & Scenario II & Time\\

 Algorithm & $AUC_{FS}$  & $AUC_{FS}$ & $AUC_{FS}$  & $AUC_{FS}$ &  \\
\hline
DIFFI         & -1.484     & -3.66    & -1.118     & -3.368   & \textbf{0.57} \\
IF\_\approach         & -1.681    & \textbf{4.398}    & -1.162     & \textbf{4.231}   & 1.05 \\
EIF\_\approach        & -1.787     & 1.844& -1.37     & 2.049& \textbf{0.94} \\
\EIFplus\_\approach       & -1.51     & 2.331& -0.991     & 2.39& 0.99 \\
IF\_RF        & \textbf{-0.785}     & 2.077     & \textbf{-0.723}     & 2.483     & 8.05 \\
EIF\_RF       & -0.848    & 1.631    & -0.717     & 2.174    & 8.05  \\
\EIFplus\_RF      & -1.882     & 1.476     & -1.433     & 2.086     & 8.05  \\
\hline
\end{tabular}
\end{table}

Table \ref{tab:fs-tab-moodify} showcases the $AUC_{FS}$ scores derived from various interpretation methods. In Scenario I, interpretations appear to fail, likely because the model fails to accurately pinpoint the given anomalies, but rather represent other kinds of deviation from the normal distribution of the dataset. Conversely, when models are trained exclusively with inliers, there's a notable improvement in results. Particularly, the \approach and post-hoc algorithms excel, demonstrating robust performance. This behavior holds for all the considered interpretation apporaches except for DIFFI, where the struggle to accurately identify the most critical features becomes evident for the presence of negative values of the $AUC_{FS}$ metric in both scenarios. 

Finally, a critical observation is the computational efficiency of the \approach, which is 10 times faster than that of post-hoc models. This highlights the \approach's advantage in scenarios with limited computational resources, emphasizing its efficacy and speed in model interpretation tasks.

\subsection*{{\ttfamily Pendigits}}

\subsubsection{Performance}

\ale{Figure \ref{fig:Pendigits_contamination_full} represents the trend of the Average Precision metrics as anomalies are gradually inserted into the train process of the five Anomaly Detection models used for experimental evaluation. The models presenting the higher precision values in presence of only inliers in the training set (i.e. Scenario II) are DIF, IF and the proposed \EIFplus, whose performances drop as the number of outliers increases and saturate to reach similar values as the other models. For what concerns the comparison between EIF and its improved version, introduced in this study, \EIFplus , depicted in Figure \ref{fig:Pendigits_contaminationEIFvsEIF+}, it is possible to notice how \EIFplus shows better performances than EIF when the number of outliers considers for training is limited and the two models tend to become closer in terms of performances as the contamination factor increases. This behavior is a direct consequence of how the \EIFplus approach is build to optimize the generalizability capabilities of the EIF model.} 

\begin{figure}[!ht] 
    \centering % <-- added
    \begin{subfigure}[t]{0.49\textwidth}
      \includegraphics[width=\linewidth]{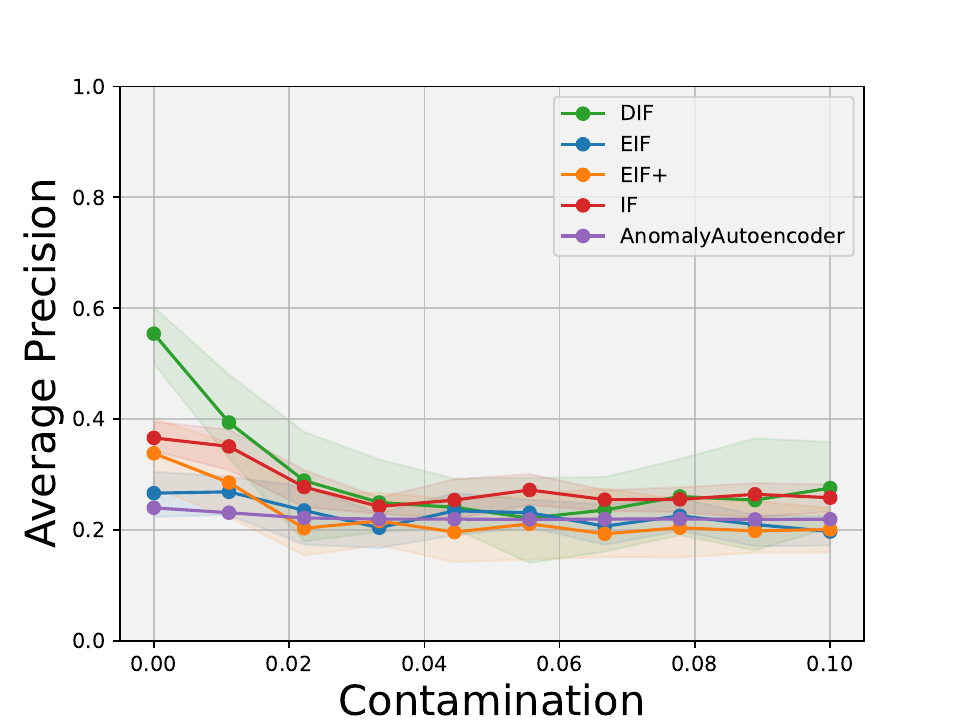}
      \caption{Models evaluation, varying the contamination levels}
      \label{fig:Pendigits_contamination_full}
    \end{subfigure}\hfil % <-- added
    \begin{subfigure}[t]{0.44\textwidth}
      \includegraphics[width=\linewidth]{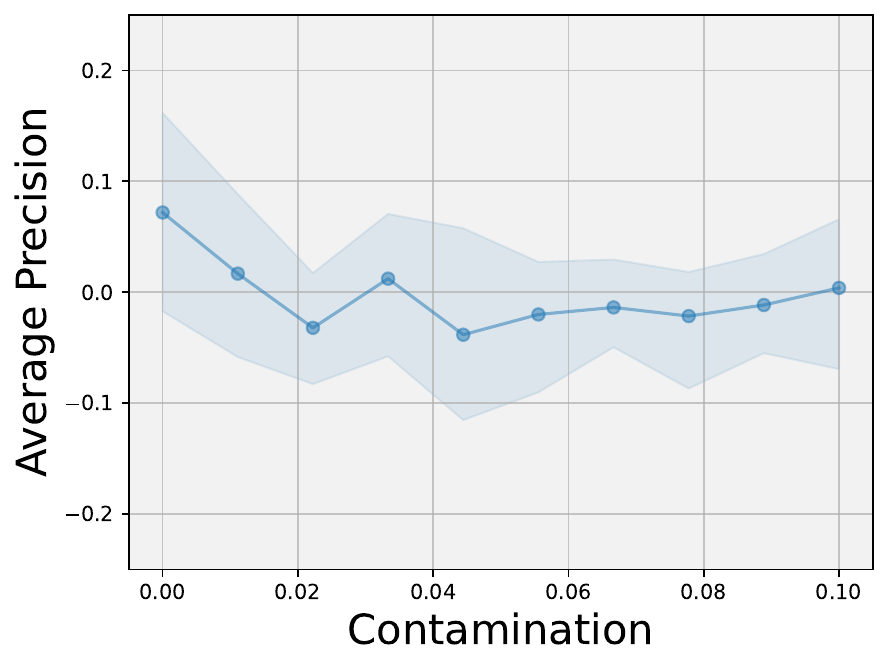}
      \caption{Difference between \EIFplus and EIF average precision}
      \label{fig:Pendigits_contaminationEIFvsEIF+}
    \end{subfigure}\hfil % <-- added
\caption{Figure \ref{fig:Pendigits_contamination_full} illustrates the average precision as the contamination level in the training set increases. Figure \ref{fig:Pendigits_contaminationEIFvsEIF+} compares the performance graphs of EIF and \EIFplus, using the difference of their scores in various contamination levels.}
\label{fig:Pendigits_contamination}
\end{figure}

Table \ref{tab:Pendigits_perf}  reports a detailed evaluation of the performances of the AD models compared in the Contamination plot, focusing on the comparison between the Scenario I and Scenario II training approaches. The three models highligthed in Figure \ref{fig:Pendigits_contamination_full} (i.e. IF, DIF and \EIFplus) are the unique ones where a significant difference can be noticed switching from Scenario I to Scenario II. The best model in terms of Average Precision is DIF but, at the same time, it is associated with dramatically high computational time, in terms of fit and predict, with the respect to the isolation-based AD models making its usage not ideal, mainly in real world applications. As a consequence \EIFplus can be considered as the optimal choice for the {\ttfamily Pendigits} dataset.

\begin{table}[htbp]
\begin{minipage}[t]{0.46\textwidth}
\strut\vspace*{-\baselineskip}\newline
\resizebox{\textwidth}{!}{
\begin{tabular}{|c||ccc|ccc||cc|}
\toprule
\hline
&\multicolumn{3}{c|}{Scenario I}&\multicolumn{3}{c||}{Scenario II}&\multicolumn{2}{c|}{Time}\\
\hline
AD Model & Avg & Prec & ROC & Avg & Prec & ROC & fit & pred \\
& Prec &  & AUC & Prec &  & AUC &  &  \\
\hline
IF          & 0.28& 0.31& 0.64& 0.37& 0.42& 0.7& \textbf{0.07}& \textbf{0.03}\\
EIF         & 0.23& 0.24 & 0.61& 0.27& 0.36& 0.67& 0.07& 0.44\\
EIF+        & 0.21& 0.41& \textbf{0.69}& 0.36& 0.45& 0.72& 0.07& 0.45\\
DIF         & \textbf{0.34}& \textbf{0.39}& 0.68& \textbf{0.46}& \textbf{0.53}& \textbf{0.76}& 10.2& 8.36\\
AE & 0.22& 0.33& 0.65& 0.24& 0.33& 0.66& 19.0& 0.32  \\
\hline
\end{tabular}}
\vspace{0.41cm}
\caption{Performances of 5 different Anomaly Detection models over {\ttfamily Pendigits} are compared using classical Classification metrics. Moreover, the last two columns contain the average time for a fit and predict operation. The highest metric values and the lowest execution times are highlighted in bold}\label{tab:Pendigits_perf}
\end{minipage}
\hfill
\begin{minipage}[t]{0.46\textwidth}
\strut\vspace*{-\baselineskip}\newline
\resizebox{\textwidth}{!}{
\begin{tabular}{|c||c|c|c|c||c|}
\toprule
\hline
&\multicolumn{2}{c|}{Evaluation with EIF}&\multicolumn{2}{c||}{Evaluation with \EIFplus}&\\
\hline
& Scenario I & Scenario II & Scenario I & Scenario II & Time\\

 Algorithm & $AUC_{FS}$  & $AUC_{FS}$ & $AUC_{FS}$  & $AUC_{FS}$ &  \\
\hline
DIFFI               & 0.118& -0.384& 0.233& -0.766& 0.37\\
IF\_\approach        & \textbf{2.198}& \textbf{2.688}& \textbf{2.172}& \textbf{3.187}& 1.13\\
EIF\_\approach       & 1.588& 1.887& 1.767& 2.232& 1.25\\
EIF+\_\approach      & 1.868& 1.227& 1.921& 1.326& 1.22\\
IF\_RF              & 1.484& 1.281& 1.377& 1.380& 8.90\\
EIF\_RF             & -0.728& -0.842& -0.368& -1.287& 8.90\\
EIF+\_RF            & -1.402& -0.249& -0.971& -0.748& 8.90\\
\hline
\end{tabular}}
\caption{Quantitative evaluation of the effectiveness of 6 different interpretation algorithms on {\ttfamily Pendigits} through the $AUC_{FS}$ metric, introduced in \ref{sec:interpr_evaluat}. In the last column the average time taken by the different models to produce the importance scores is reported. The highest $AUC_{FS}$ and lowest Importance time values are highlighted in bold.}\label{tab:fs-tab-Pendigits}
\end{minipage}
\end{table}

\subsubsection{Importance Plots} \label{sec:Pendigits-imp-plots}

\ale{Similarly to what can be observed in the {\ttfamily Ionosphere} dataset, Figure \ref{fig:interpretation-Pendigits} portraits how it is challenging to identify a single dominant feature in terms of importance. As a consequence it can be concluded the probably there is a small group of features along which anomalies are distributed. Observing the Score Plots (Figures \ref{fig:Feat-imp-Pendigits}, \ref{fig:Feat-imp-Pendigits-split}) and the Bar Plots (Figures \ref{fig:GFI-Pendigits}, \ref{fig:GFI-Pendigits-split}) it can be noticed how Features 1, 3 and 5 appear in the top 3 ranking in both Scenario I and Scenario II and thus may be the variables composing the aforementioned group of important features.} 

\begin{figure}[!ht] 
    \centering % <-- added
    \begin{subfigure}[t]{0.33\textwidth}
    \centering
      \includegraphics[width=\linewidth]{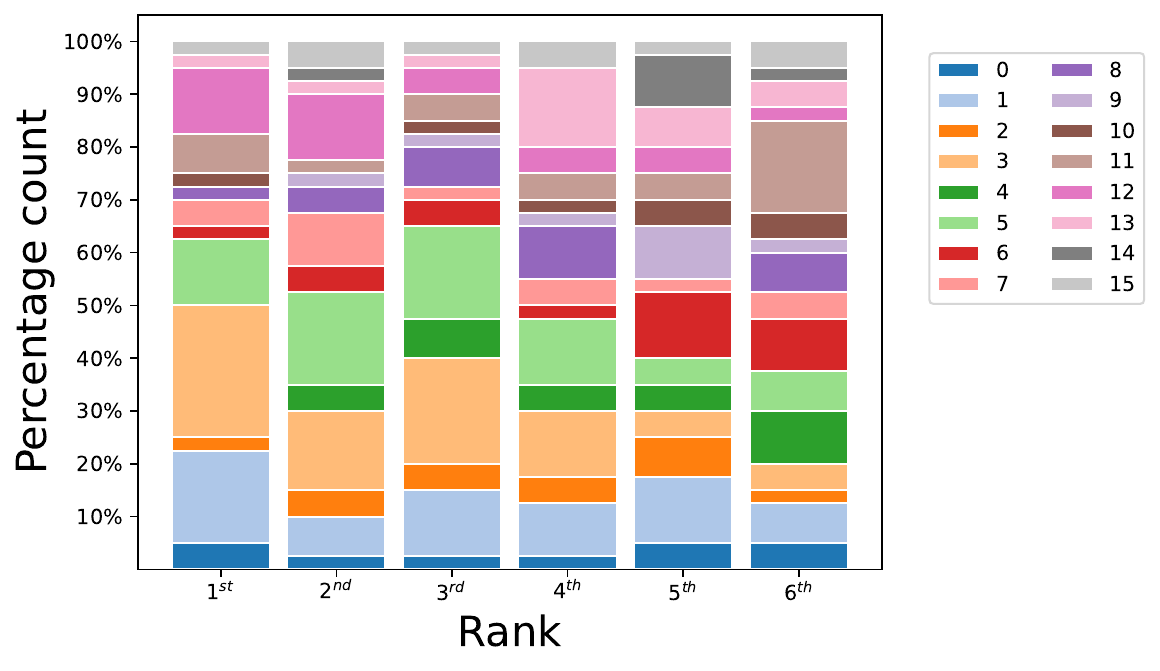}
      \caption{Bar Plot {\ttfamily Pendigits} Scenario I}
      \label{fig:GFI-Pendigits}
    \end{subfigure}\hfil % <-- added
    \begin{subfigure}[t]{0.27\textwidth}
    \centering
      \includegraphics[width=\linewidth]{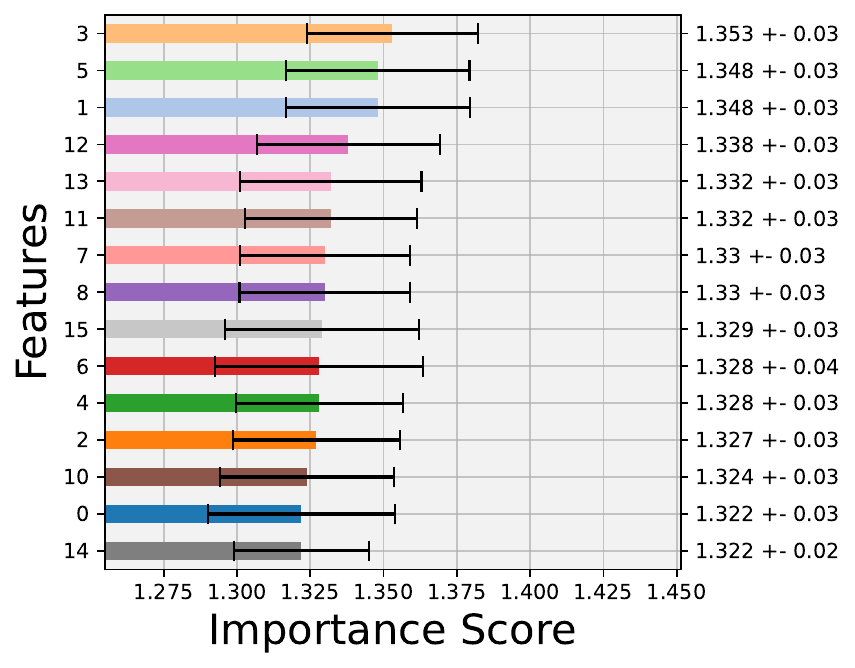}
      \caption{Score Plot {\ttfamily Pendigits} Scenario I}
      \label{fig:Feat-imp-Pendigits}
    \end{subfigure}\hfil % <-- added
    \begin{subfigure}[t]{0.28\textwidth}
    \centering
      \includegraphics[width=\linewidth]{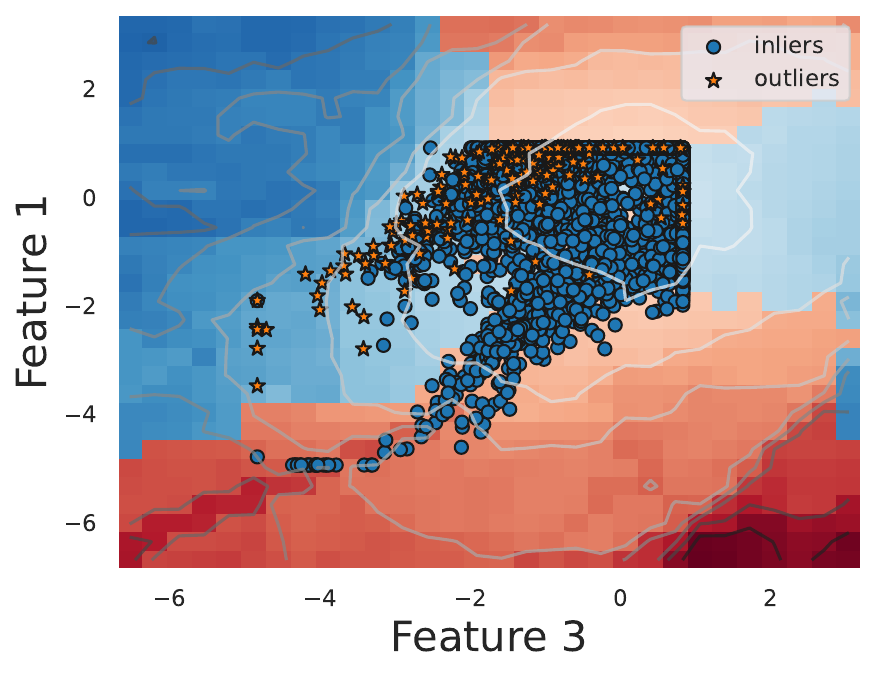}
      \caption{Scoremap {\ttfamily Pendigits} Scenario I}
      \label{fig:Local-Pendigits}
    \end{subfigure}\hfil % <-- added
    \begin{subfigure}[t]{0.33\textwidth}
    \centering
      \includegraphics[width=\linewidth]{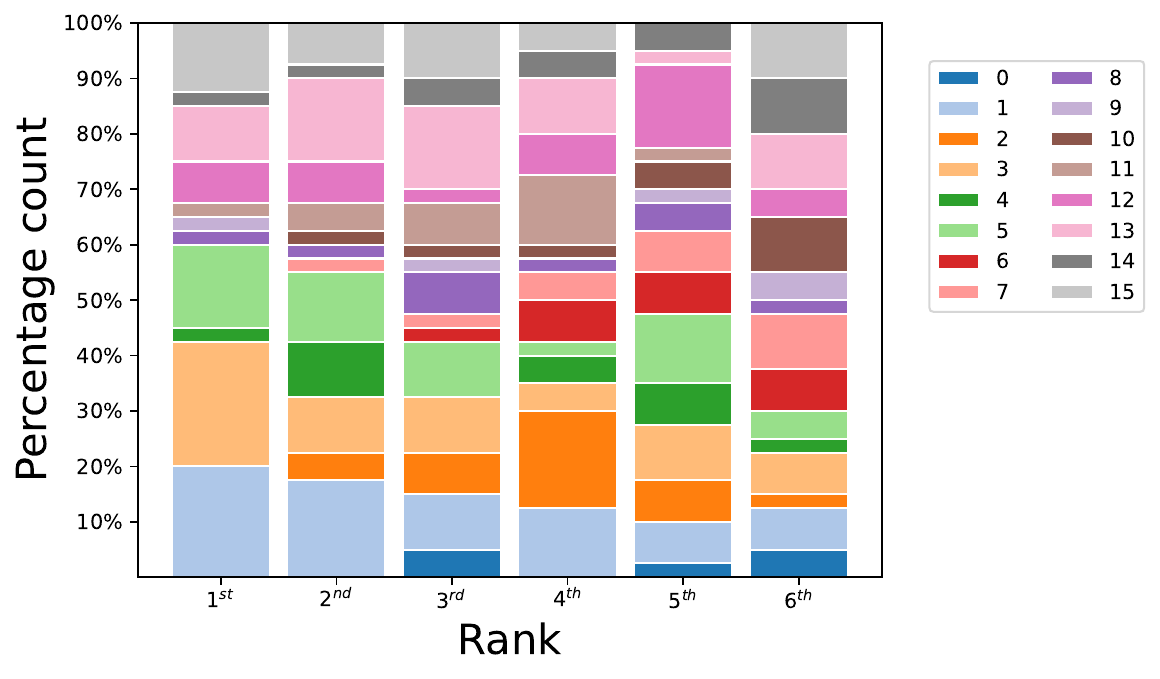}
      \caption{Bar Plot {\ttfamily Pendigits} Scenario II}
      \label{fig:GFI-Pendigits-split}
    \end{subfigure}\hfil % <-- added
    \begin{subfigure}[t]{0.27\textwidth}
    \centering
      \includegraphics[width=\linewidth]{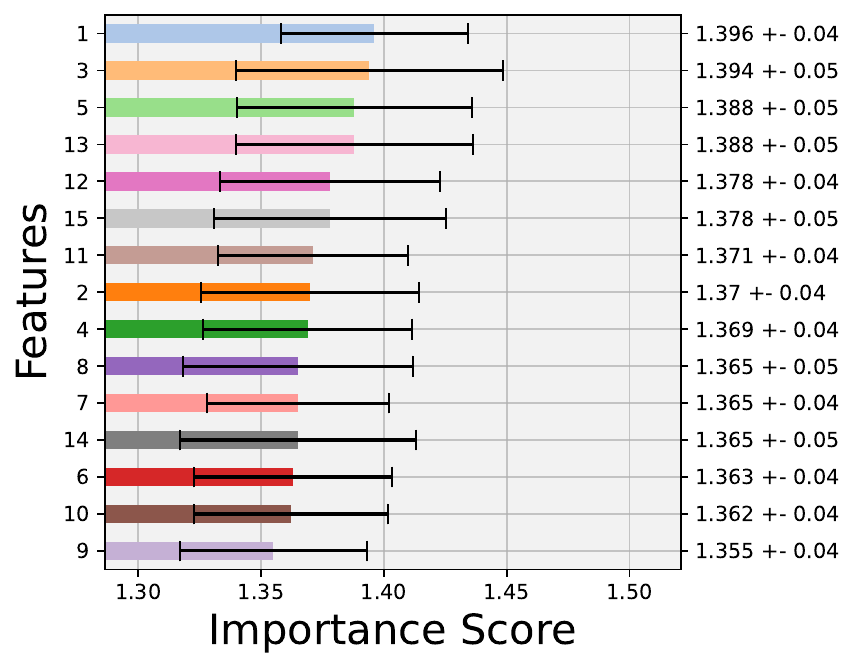}
      \caption{Score Plot {\ttfamily Pendigits} Scenario II}
      \label{fig:Feat-imp-Pendigits-split}
    \end{subfigure}\hfil % <-- added
    \begin{subfigure}[t]{0.28\textwidth}
    \centering
      \includegraphics[width=\linewidth]{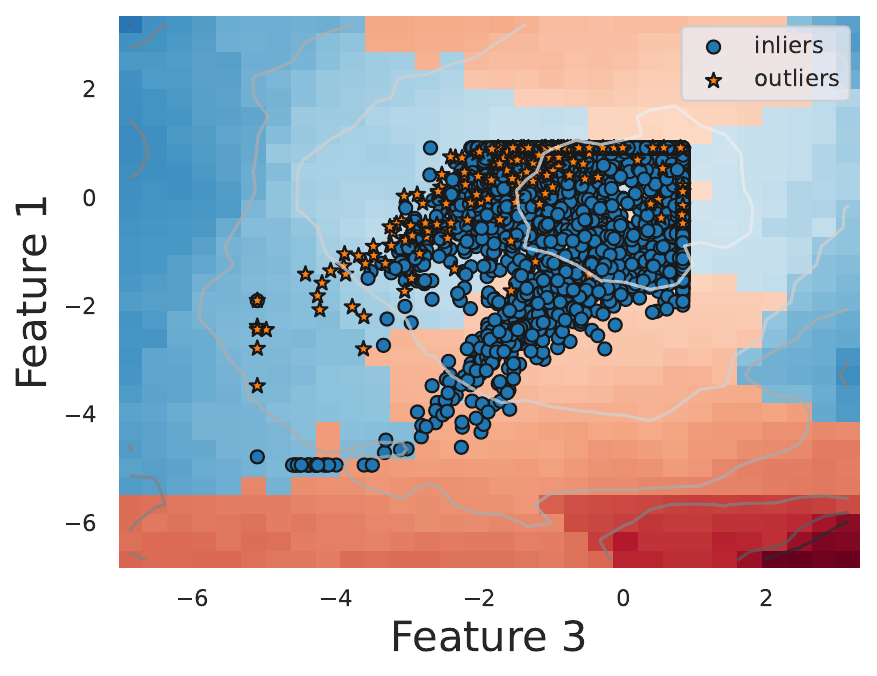}
      \caption{Scoremap {\ttfamily Pendigits} Scenario II}
      \label{fig:Local-Pendigits-split}
    \end{subfigure}\hfil % <-- added
\caption{Bar Plot, Score Plot and Scoremap for {\ttfamily Pendigits} in the two different Scenarios, using the \approach algorithm applied to the \EIFplus model.}\label{fig:interpretation-Pendigits}
\end{figure}

\subsubsection{Feature Selection}

\ale{A confirmation of the conclusions reached from the analysis conducted in \ref{sec:Pendigits-imp-plots} can be achieved looking at the Feature Selection plots organized in Figure \ref{fig:fs-interpretation-Pendigits}. In particular in Figure \ref{fig:Feat-Sel_Pendigits_valEIF+_EXIFFI+_2}  it is possible to highlight how the Average Precision gradually decreases reducing the number of input features from 3 to 1, meaning that dropping one of features 1,3 or 5 the model loses crucial information for the detection of anomalous points and thus its detecting performance experience a considerable drop. Notably the only model whose explanations are associated to a Feature Selection plot where the red curve is always placed above the blue one is the IF model as depicted in Figures \ref{fig:Feat-Sel_Pendigits_valEIF+_DIFFI_2} and \ref{fig:Feat-Sel_Pendigits_valEIF+_IF_RandomForest_2}.}

\begin{figure}[!ht] 
\centering
\hspace{0.05\textwidth}\textbf{IF} \hspace{0.29\textwidth} \textbf{EIF} \hspace{0.29\textwidth} \textbf{EIF+}
% First row with vertical caption on the left
\begin{minipage}{\textwidth}
    \rotatebox{90}{\parbox{15mm}{\centering \textbf{Ad-Hoc}}} % Adjust the parbox width as necessary for your caption text
    \begin{minipage}{0.95\textwidth}
        \begin{subfigure}[t]{0.30\textwidth}
            \centering
            \includegraphics[trim={0 0 3.5cm 0}, clip, width=\linewidth]{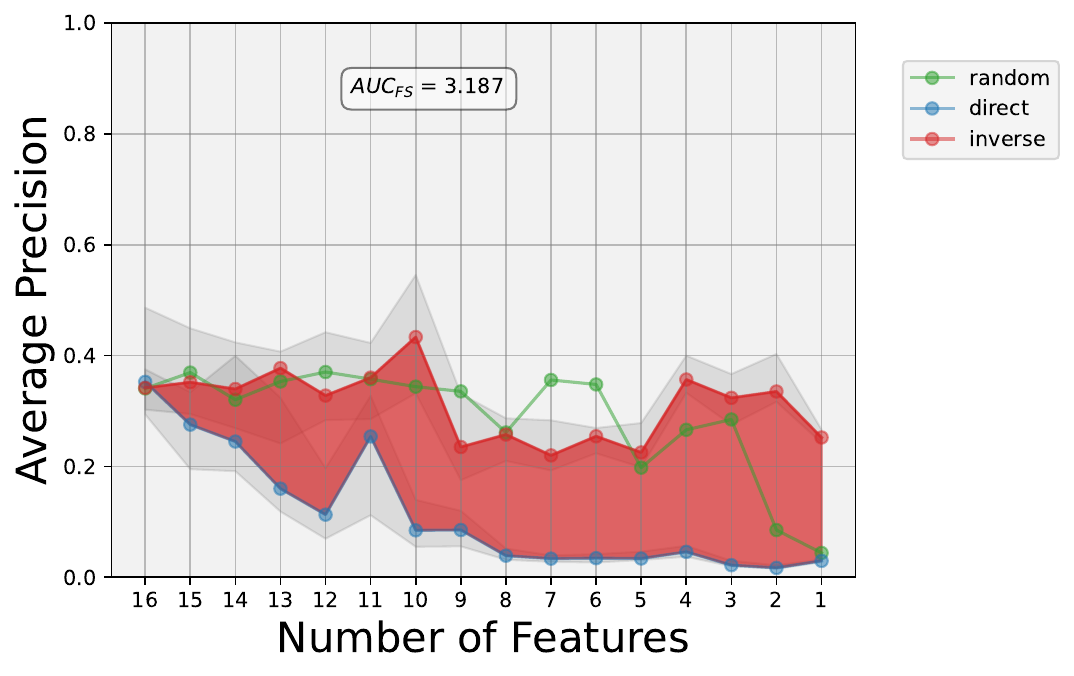}
            \caption{\approach applied to IF}
            \label{fig:Feat-Sel_Pendigits_valEIF+_DIFFI_2}
        \end{subfigure}\hfill
        \begin{subfigure}[t]{0.30\textwidth}
            \centering
            \includegraphics[trim={0 0 3.5cm 0}, clip, width=\linewidth]{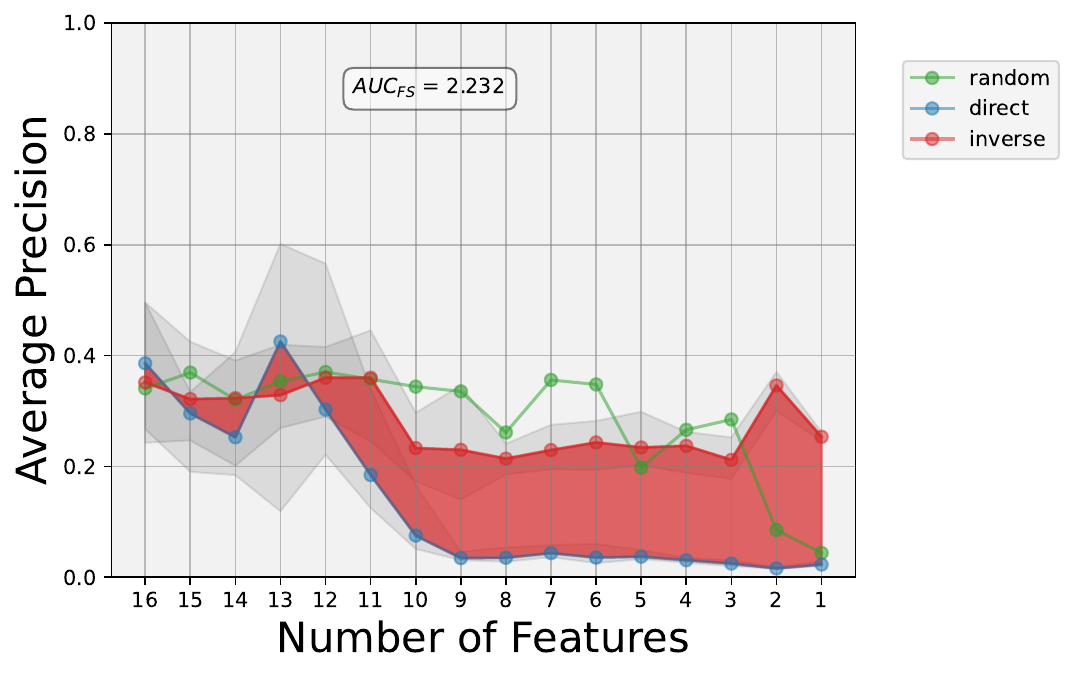}
            \caption{\approach applied to EIF}
            \label{fig:Feat-Sel_Pendigits_valEIF+_EXIFFI_2}
        \end{subfigure}\hfill
        \begin{subfigure}[t]{0.30\textwidth}
            \centering
            \includegraphics[trim={0 0 3.5cm 0}, clip, width=\linewidth]{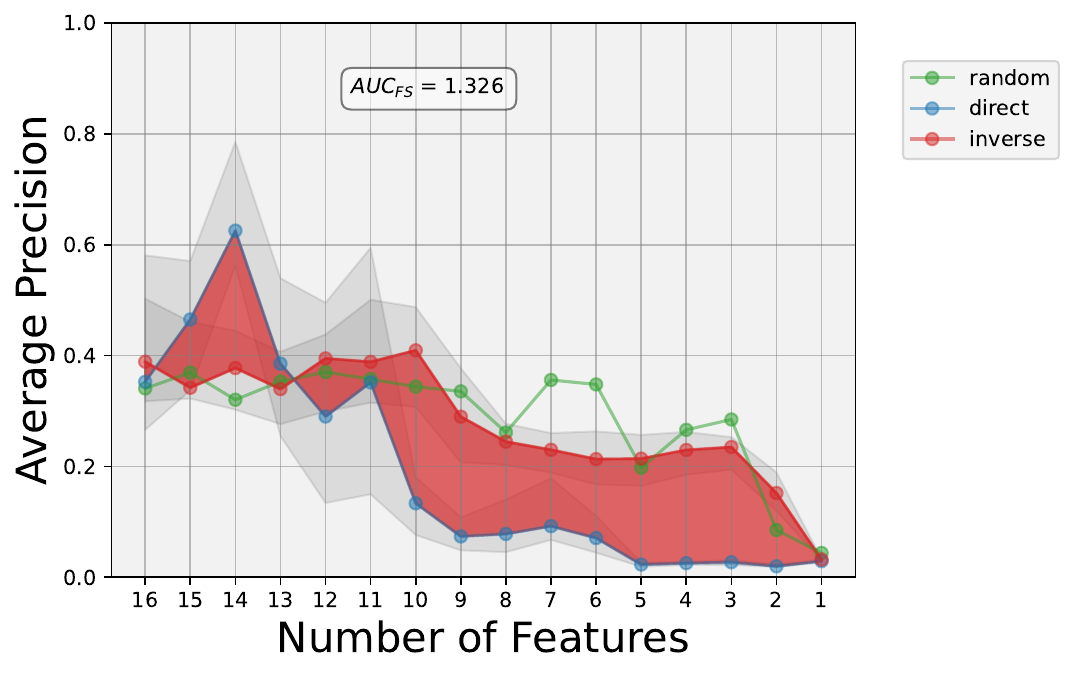}
            \caption{\approach applied to \EIFplus}
            \label{fig:Feat-Sel_Pendigits_valEIF+_EXIFFI+_2}
        \end{subfigure}
    \end{minipage}
\end{minipage}

\vspace{5mm} % Space between rows

% Second row with vertical caption on the left
\begin{minipage}{\textwidth}
    \rotatebox{90}{\parbox{15mm}{\centering \textbf{Post-Hoc}}} % Adjust as necessary
    \begin{minipage}{0.95\textwidth}
        \begin{subfigure}[t]{0.30\textwidth}
            \centering
            \includegraphics[trim={0 0 3.5cm 0}, clip, width=\linewidth]{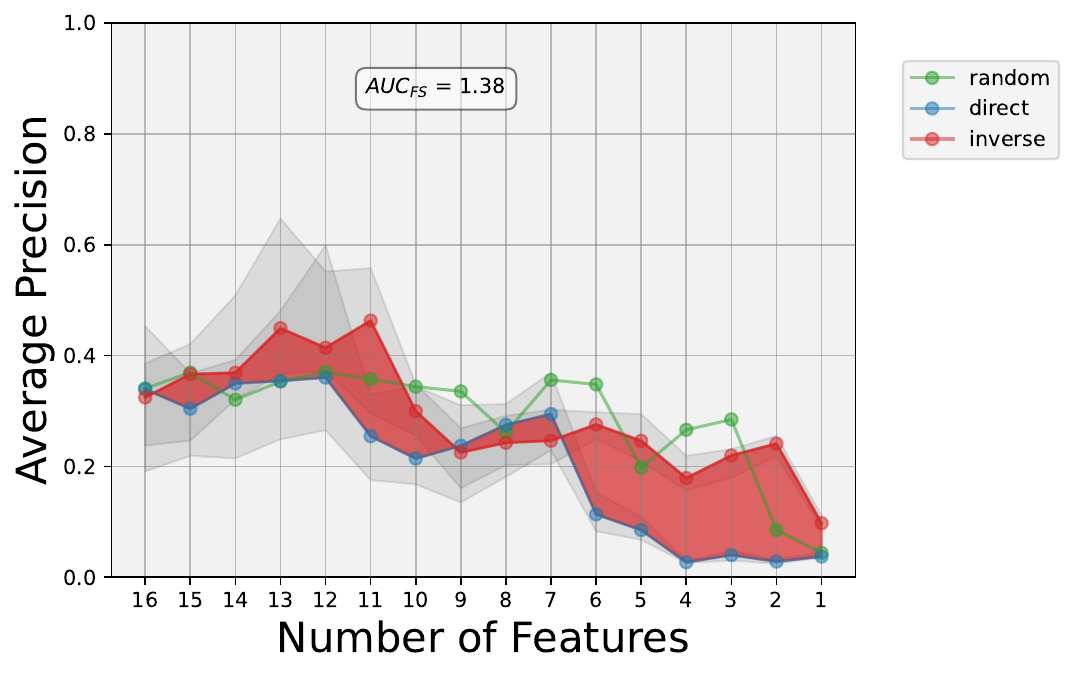}
            \caption{RandomForest fitted to IF}
            \label{fig:Feat-Sel_Pendigits_valEIF+_IF_RandomForest_2}
        \end{subfigure}\hfill
        \begin{subfigure}[t]{0.30\textwidth}
            \centering
            \includegraphics[trim={0 0 3.5cm 0}, clip, width=\linewidth]{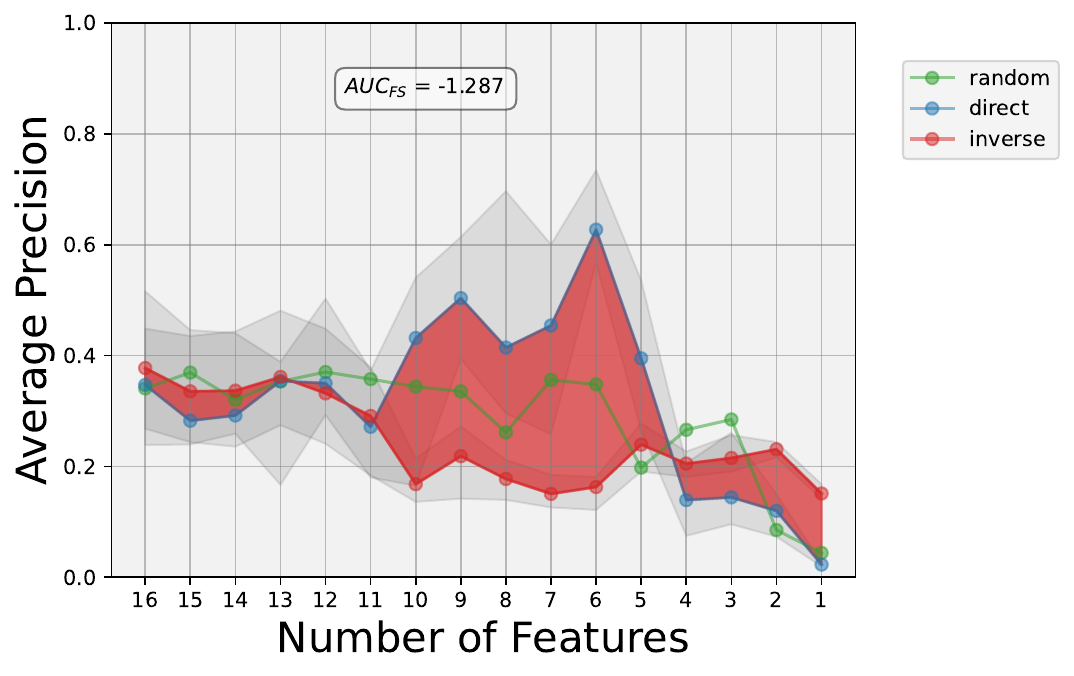}
            \caption{RandomForest fitted to EIF}
            \label{fig:Feat-Sel_Pendigits_valEIF+_EIF_RandomForest_2}
        \end{subfigure}\hfill
        \begin{subfigure}[t]{0.30\textwidth}
            \centering
            \includegraphics[trim={0 0 3.5cm 0}, clip, width=\linewidth]{Newfigures/Pendigits/Feature_Selection/22-03-2024_16-23-48_pendigits_EIF+_EXIFFI+_feature_selection_2.pdf}
            \caption{RandomForest fitted to \EIFplus}
            \label{fig:Feat-Sel_Pendigits_valEIF+_EIF+_RandomForest_2}
        \end{subfigure}
    \end{minipage}
\end{minipage}

\caption{Feature Selection of the different Ad-Hoc and Post-Hoc methods applied to the 3 Isolation Forest models: IF, EIF and \EIFplus. The blue line is the values of average precision, calculated with the \EIFplus model in the Scenario II, dropping the most important feature at each step, the red line is the values of average precision dropping the least important feature at each step and the green line is the value of the feature selection dropping a random feature at each step.}\label{fig:fs-interpretation-Pendigits}
\end{figure}

\ale{To conclude the experimental evaluation of the {\ttfamily Pendigits} dataset it is possible to analyse Table \ref{tab:fs-tab-Pendigits}, where a quantitative analysis of the effectiveness of the different interpretation methods proposed is presented. The model that correctly captures the ranking of features according to their relevance is IF\_\approach, followed by \approach+ as it is testified by the high values of the $AUC_{FS}$ metric. On the other hand explanations based on DIFFI and post-hoc methods using Random Forest as a surrogate model prove to wrongly interpret the importance of features and are consequently associated to negative values of $AUC_{FS}$. Finally it is also worth noticing how the interpretation methods deriving from Isolation-based AD methods (i.e. IF\_\approach, \approach and \approach+) showcase much more efficient time performances in the computation of the importance scores with the respect to the post-hoc methods.}

\subsection*{{\ttfamily Pima}}

\subsubsection{Performance} \label{sec:Pima-Contamination-sec}

\ale{The Contamination plot for the {\ttfamily Pima} dataset is reported in Figure \ref{fig:Pima_contamination_full}. It depicts how the Average Precision metric of the AD models considered is not affected by the amount of outliers included in the training set. The Isolation-based models (i.e. IF, EIF and \EIFplus) emerge as the ones with the better performances, though the margin on the deep learning based methods (i.e. DIF and Autoencoder) is minimal.}

\begin{figure}[!ht] 
    \centering % <-- added
    \begin{subfigure}[t]{0.49\textwidth}
      \includegraphics[width=\linewidth]{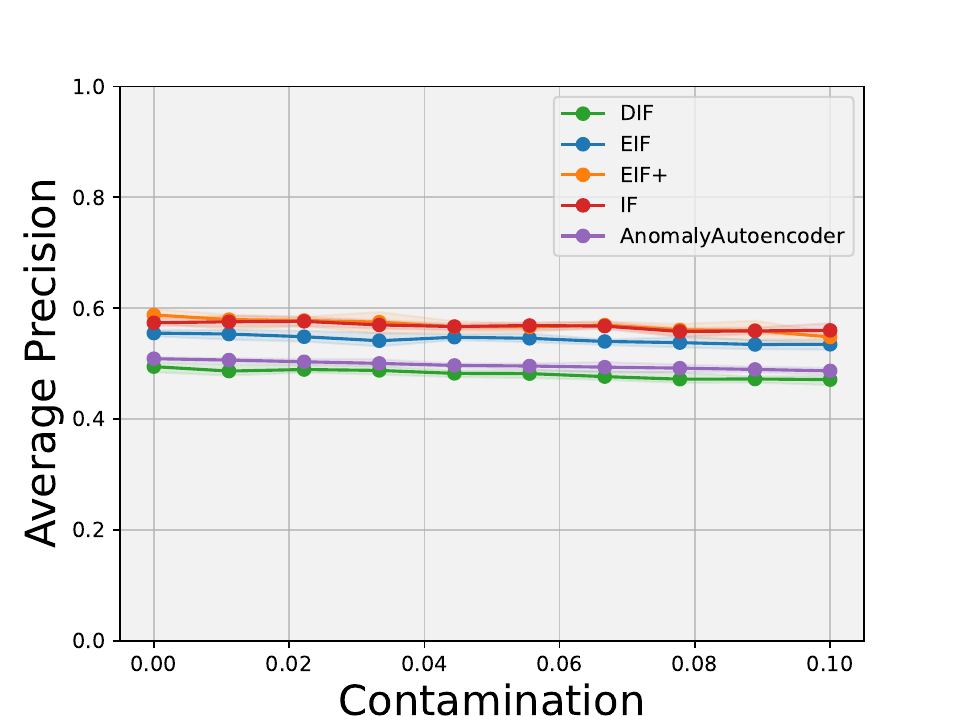}
      \caption{Models evaluation, varying the contamination levels}
      \label{fig:Pima_contamination_full}
    \end{subfigure}\hfil % <-- added
    \begin{subfigure}[t]{0.44\textwidth}
      \includegraphics[width=\linewidth]{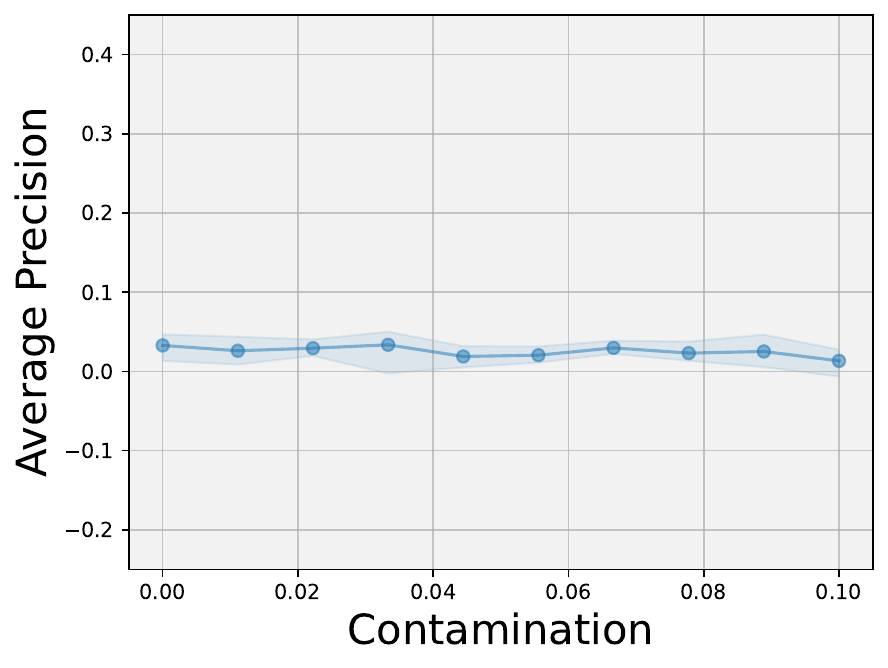}
      \caption{Difference between \EIFplus and EIF average precision}
      \label{fig:Pima_contaminationEIFvsEIF+}
    \end{subfigure}\hfil % <-- added
\caption{Figure \ref{fig:Pima_contamination_full} illustrates the average precision as the contamination level in the training set increases. Figure \ref{fig:Pima_contaminationEIFvsEIF+} compares the performance graphs of EIF and \EIFplus, using the difference of their scores in various contamination levels.}
\label{fig:Pima_contamination}
\end{figure}

\ale{Table \ref{tab:Pima_perf} includes additional metrics other than Average Precision and focuses on the cases in which the training set's contamination is null (i.e. Scenario II) and equal to the total number of outliers in the dataset (i.e. Scenario I). As already described in \ref{sec:Pima-Contamination-sec} the difference between the two previously depicted scenarios is minimal and the proposed \EIFplus once again proves to be the optimal model also on the {\ttfamily Pima} dataset.}

\begin{table}[htbp]
\begin{minipage}[t]{0.46\textwidth}
\strut\vspace*{-\baselineskip}\newline
\resizebox{\textwidth}{!}{
\begin{tabular}{|c||ccc|ccc||cc|}
\toprule
\hline
&\multicolumn{3}{c|}{Scenario I}&\multicolumn{3}{c||}{Scenario II}&\multicolumn{2}{c|}{Time}\\
\hline
AD Model & Avg & Prec & ROC & Avg & Prec & ROC & fit & pred \\
& Prec &  & AUC & Prec &  & AUC &  &  \\
\hline
IF          & \textbf{0.51}& \textbf{0.52}& \textbf{0.63}& 0.58& 0.55& 0.66& 0.11& \textbf{0.008}\\
EIF         & 0.49& 0.49& 0.61& 0.54& 0.57& 0.67& \textbf{0.07}& 0.03\\
EIF+        & 0.49& 0.5& 0.61 & \textbf{0.58}& \textbf{0.57}& \textbf{0.67}& 0.08& 0.03\\
DIF         & 0.41& 0.41& 0.54& 0.49& 0.46& 0.59& 1.17& 1.00\\
AE & 0.43& 0.44& 0.57& 0.5& 0.54& 0.64& 3.11& 0.06\\
\hline
\end{tabular}}
\vspace{0.41cm}
\caption{Performances of 5 different Anomaly Detection models over {\ttfamily Pima} are compared using classical Classification metrics. Moreover, the last two columns contain the average time for a fit and predict operation. The highest metric values and the lowest execution times are highlighted in bold}\label{tab:Pima_perf}
\end{minipage}
\hfill
\begin{minipage}[t]{0.46\textwidth}
\strut\vspace*{-\baselineskip}\newline
\resizebox{\textwidth}{!}{
\begin{tabular}{|c||c|c|c|c||c|}
\toprule
\hline
&\multicolumn{2}{c|}{Evaluation with EIF}&\multicolumn{2}{c||}{Evaluation with \EIFplus}&\\
\hline
& Scenario I & Scenario II & Scenario I & Scenario II & Time\\

 Algorithm & $AUC_{FS}$  & $AUC_{FS}$ & $AUC_{FS}$  & $AUC_{FS}$ &  \\
\hline
DIFFI                    & -0.489& 0.256& -0.497& 0.303& 0.57 \\
IF\_\approach             & -0.310& \textbf{0.373}& \textbf{-0.237}& \textbf{0.367}& 0.14\\
EIF\_\approach            & -0.316& -0.214& -0.324& -0.201& \textbf{0.07}\\
\EIFplus\_\approach       & -0.309& -0.037& -0.272& -0.020& 0.06\\
IF\_RF                   & -0.369& 0.191& -0.301& 0.218& 0.43\\
EIF\_RF                  & -0.443& 0.127& -0.416& 0.178& 0.43\\
EIF+\_RF                 & \textbf{-0.288}& 0.063& -0.286& 0.149& 0.43\\
\hline
\end{tabular}
}
\caption{Quantitative evaluation of the effectiveness of 6 different interpretation algorithms on {\ttfamily Pima} through the $AUC_{FS}$ metric, introduced in \ref{sec:interpr_evaluat}. In the last column the average time taken by the different models to produce the importance scores is reported. The highest $AUC_{FS}$ and lowest Importance time values are highlighted in bold.}\label{tab:fs-tab-Pima}
\end{minipage}
\end{table}

\subsubsection{Importance Plots}

\ale{In Figure \ref{fig:interpretation-Pima} the outcomes produced by the \approach+ model in interpreting the \EIFplus model are reported. Prior to commenting the feature ranking produced by the Score and Bar Plots it is crucial to notice how the outliers are overlapped with the normal points in the {\ttfamily Pima} dataset as it can be realized looking at the Local scoremaps contained in Figures \ref{fig:Local-Pima} and \ref{fig:Local-Pima-split}. This observation is explanatory for the peculiar phenomenon encountered in the Contamination plot, in fact since outliers are mostly overlapped to normal points including them or not into the training set will not affect the Average Precision metric.}

\ale{The superimposition of anomalies and normal observations is verified because, as described in \ref{sec:real-dataset-experiments}, the real world benchmark datasets normally used in the literature to assess the performances of Anomaly Detection models are nothing more than an adaptation of Binary or Multi Class Classification datasets to the task of identifying outliers. As a consequence the data points that are labeled as anomalous (i.e. the data samples beholding to the least represented class) in some cases may not truly deviate from the inliers distributions as they should as anomalous points. As a consequence AD models based on the concept of isolating anomalies from inliers (such as \EIFplus) may not be effective to solve the Anomaly Detection task on this dataset and the interpretations furnished by \approach+ may be misleading and not aligned with the ground truth. 
In any case, according to the Score Plots produced (and represented in Figure \ref{fig:Feat-imp-Pima} and \ref{fig:Feat-imp-Pima-split}) the most important features, both in Scenario I and Scenatio II, are \textit{BloodPressure, BMI} and \textit{Insulin}.}

\begin{figure}[!ht] 
    \centering % <-- added
    \begin{subfigure}[t]{0.33\textwidth}
    \centering
      \includegraphics[width=\linewidth]{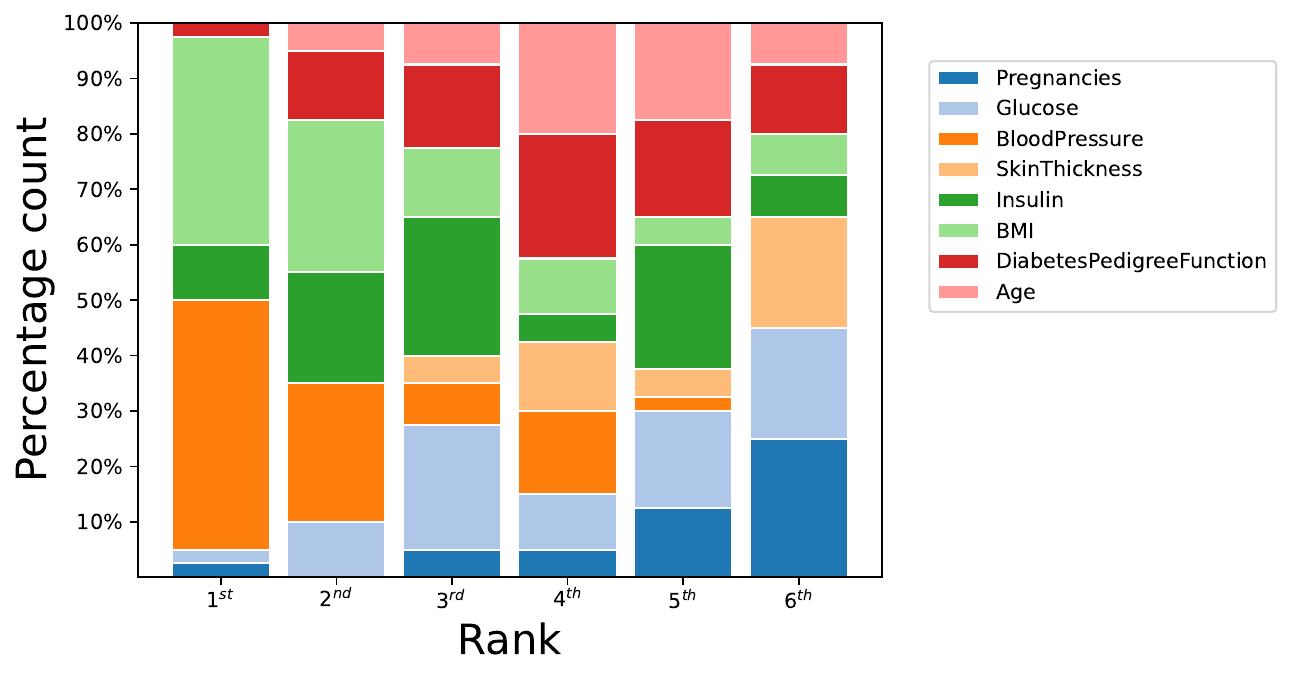}
      \caption{Bar Plot {\ttfamily Pima} Scenario I}
      \label{fig:GFI-Pima}
    \end{subfigure}\hfil % <-- added
    \begin{subfigure}[t]{0.27\textwidth}
    \centering
      \includegraphics[width=\linewidth]{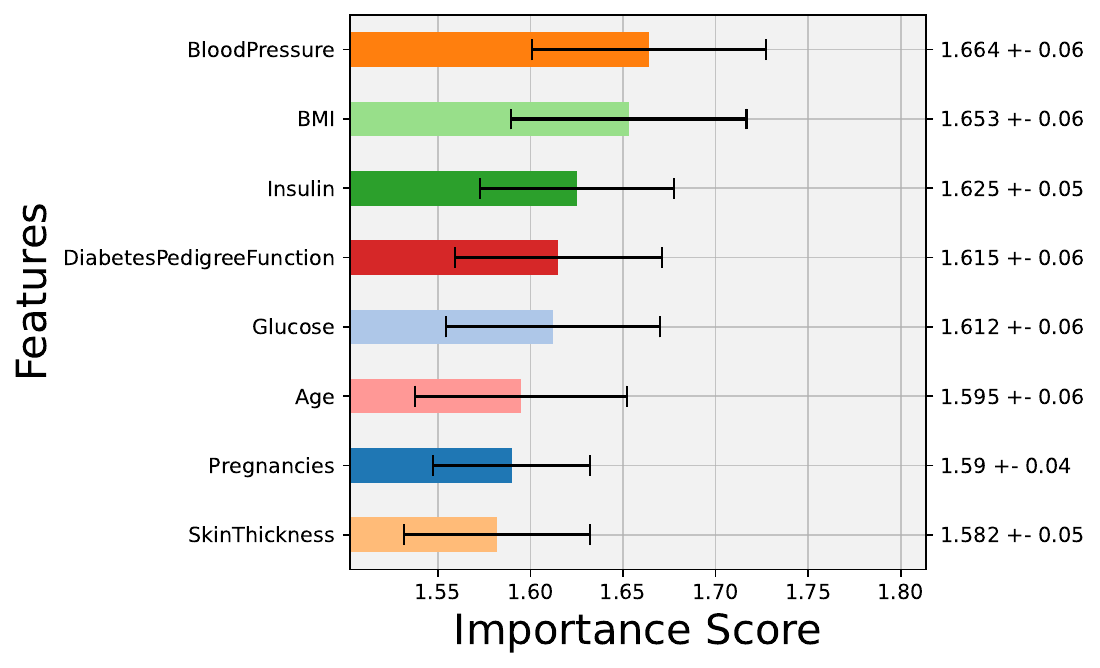}
      \caption{Score Plot {\ttfamily Pima} Scenario I}
      \label{fig:Feat-imp-Pima}
    \end{subfigure}\hfil % <-- added
    \begin{subfigure}[t]{0.28\textwidth}
    \centering
      \includegraphics[width=\linewidth]{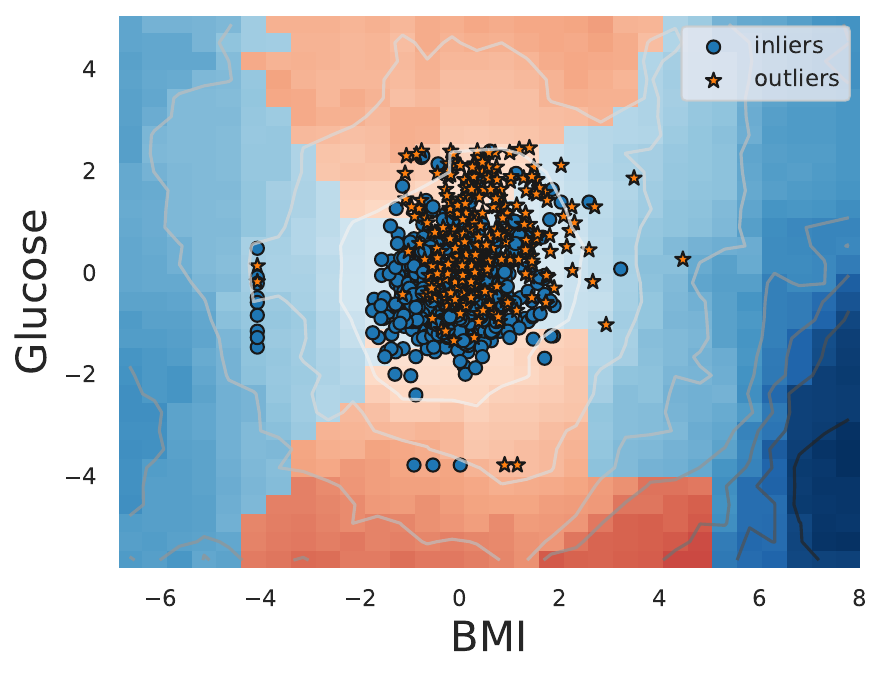}
      \caption{Scoremap {\ttfamily Pima} Scenario I}
      \label{fig:Local-Pima}
    \end{subfigure}\hfil % <-- added
    \begin{subfigure}[t]{0.33\textwidth}
    \centering
      \includegraphics[width=\linewidth]{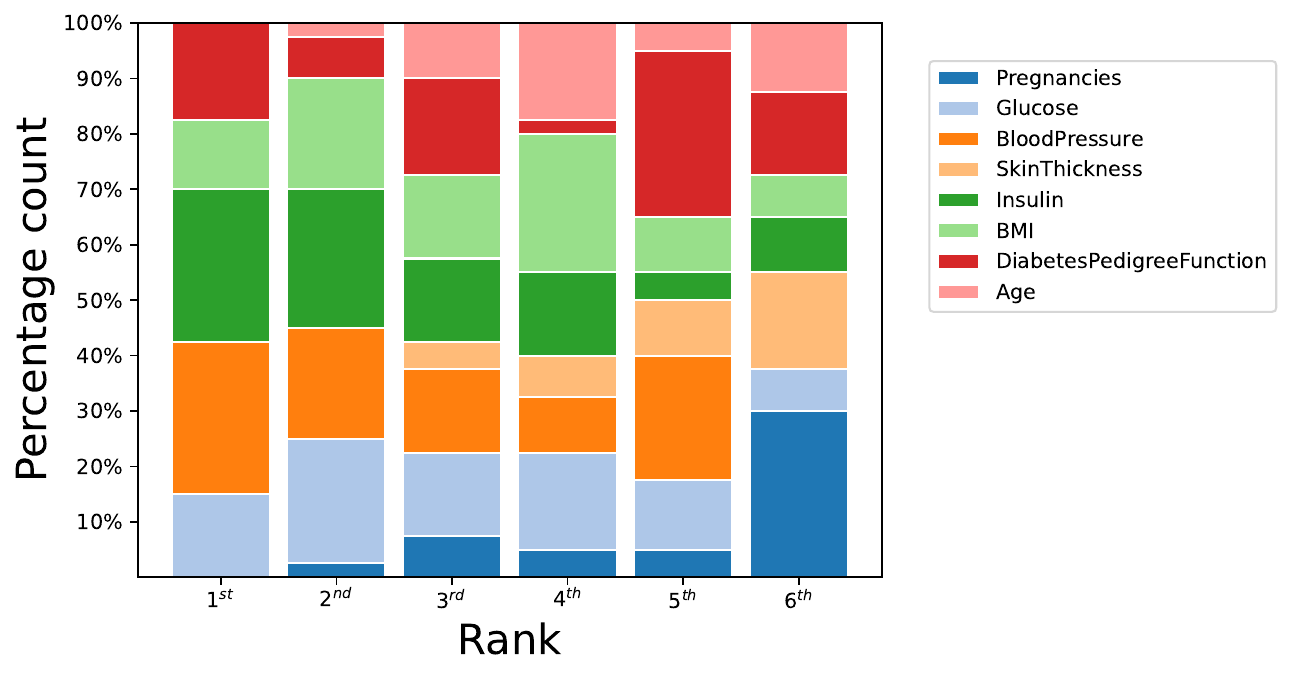}
      \caption{Bar Plot {\ttfamily Pima} Scenario II}
      \label{fig:GFI-Pima-split}
    \end{subfigure}\hfil % <-- added
    \begin{subfigure}[t]{0.27\textwidth}
    \centering
      \includegraphics[width=\linewidth]{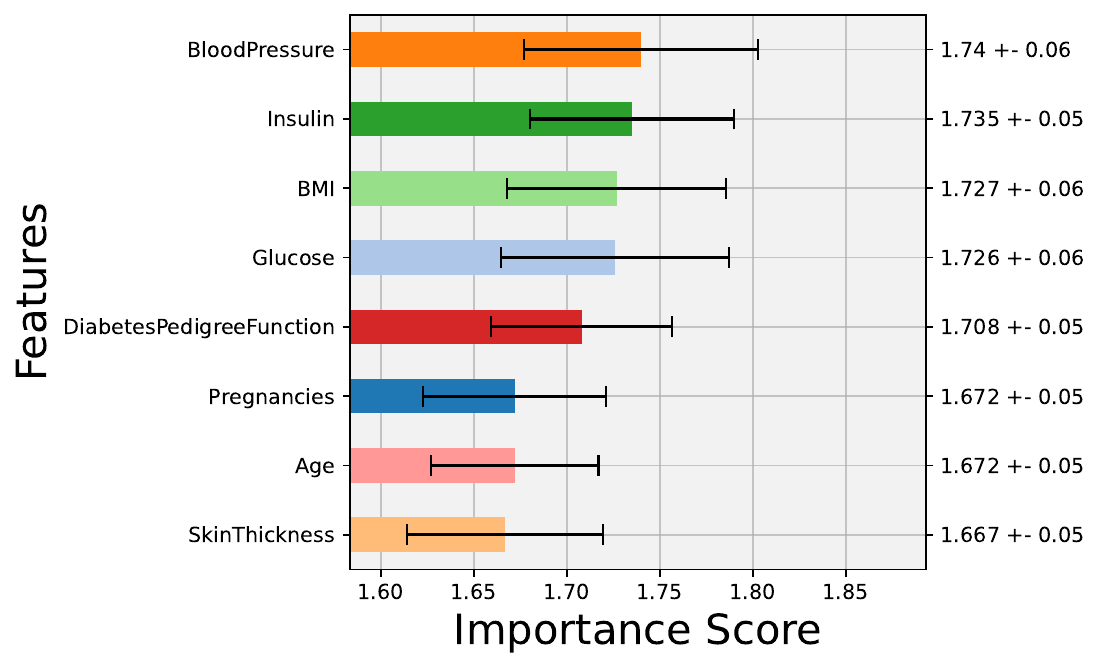}
      \caption{Score Plot {\ttfamily Pima} Scenario II}
      \label{fig:Feat-imp-Pima-split}
    \end{subfigure}\hfil % <-- added
    \begin{subfigure}[t]{0.28\textwidth}
    \centering
      \includegraphics[width=\linewidth]{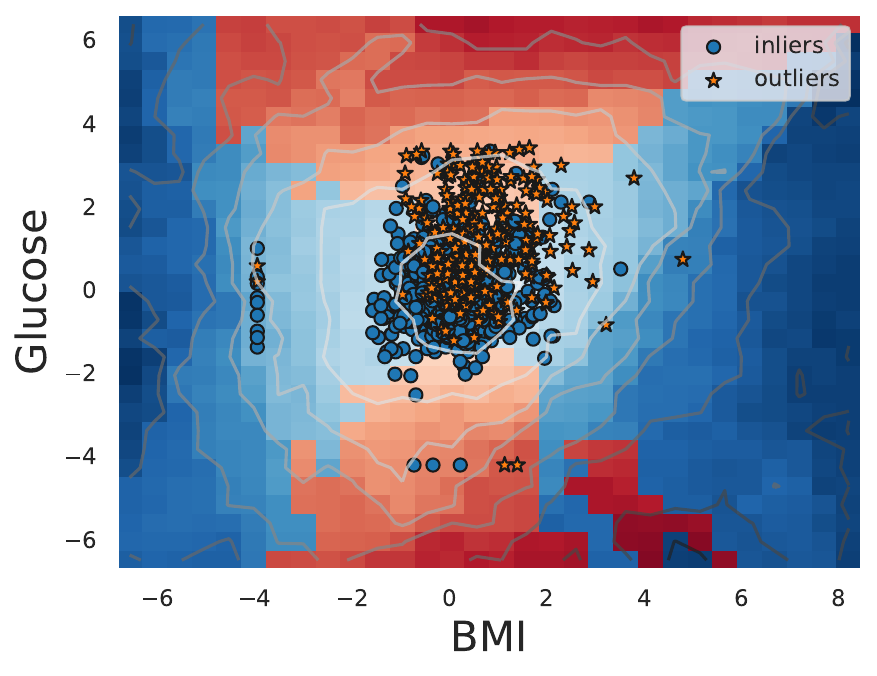}
      \caption{Scoremap {\ttfamily Pima} Scenario II}
      \label{fig:Local-Pima-split}
    \end{subfigure}\hfil % <-- added
\caption{Bar Plot, Score Plot and Scoremap for {\ttfamily Pima} in the two different Scenarios, using the \approach algorithm applied to the \EIFplus model.}\label{fig:interpretation-Pima}
\end{figure}

\subsubsection{Feature Selection}

\ale{As a consequence of the peculiar distribution of anomalies in the {\ttfamily Pima} dataset, the results produced by the application of the Unsupervised Feature Selection proxy task (Figure \ref{fig:interpretation-Pima} do not show interesting shapes since in most of the cases the Average Precision stays more or less constant, both in the red and blue line, across all the different subset of features considered. A possible exception to this behavior is represented by the IF\_\approach interpretation approach, presented in Figure \ref{fig:Feat-Sel_Pima_valEIF+_DIFFI_2}, which shows a slight advantage in omitting features in increasing order of importance (i.e. red line) with the respect to the decreasing order (i.e. blue line), however it is not as significant as in other datasets.}
 
\begin{figure}[!ht] 
\centering
\hspace{0.05\textwidth}\textbf{IF} \hspace{0.29\textwidth} \textbf{EIF} \hspace{0.29\textwidth} \textbf{EIF+}
% First row with vertical caption on the left
\begin{minipage}{\textwidth}
    \rotatebox{90}{\parbox{15mm}{\centering \textbf{Ad-Hoc}}} % Adjust the parbox width as necessary for your caption text
    \begin{minipage}{0.95\textwidth}
        \begin{subfigure}[t]{0.30\textwidth}
            \centering
            \includegraphics[trim={0 0 3.5cm 0}, clip, width=\linewidth]{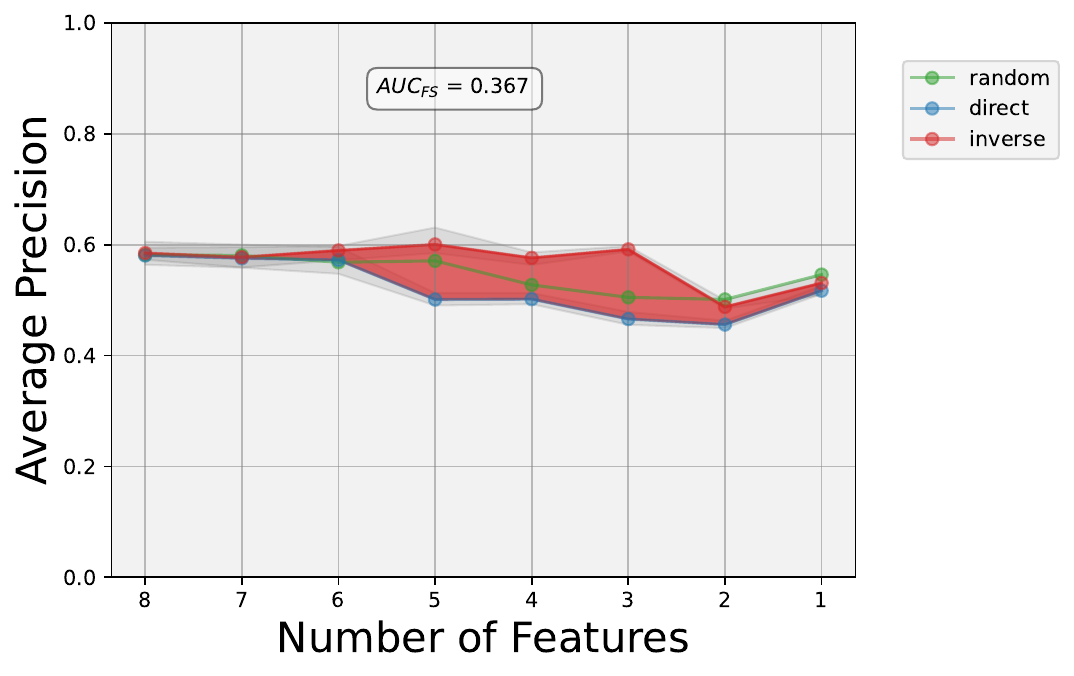}
            \caption{\approach applied to IF}
            \label{fig:Feat-Sel_Pima_valEIF+_DIFFI_2}
        \end{subfigure}\hfill
        \begin{subfigure}[t]{0.30\textwidth}
            \centering
            \includegraphics[trim={0 0 3.5cm 0}, clip, width=\linewidth]{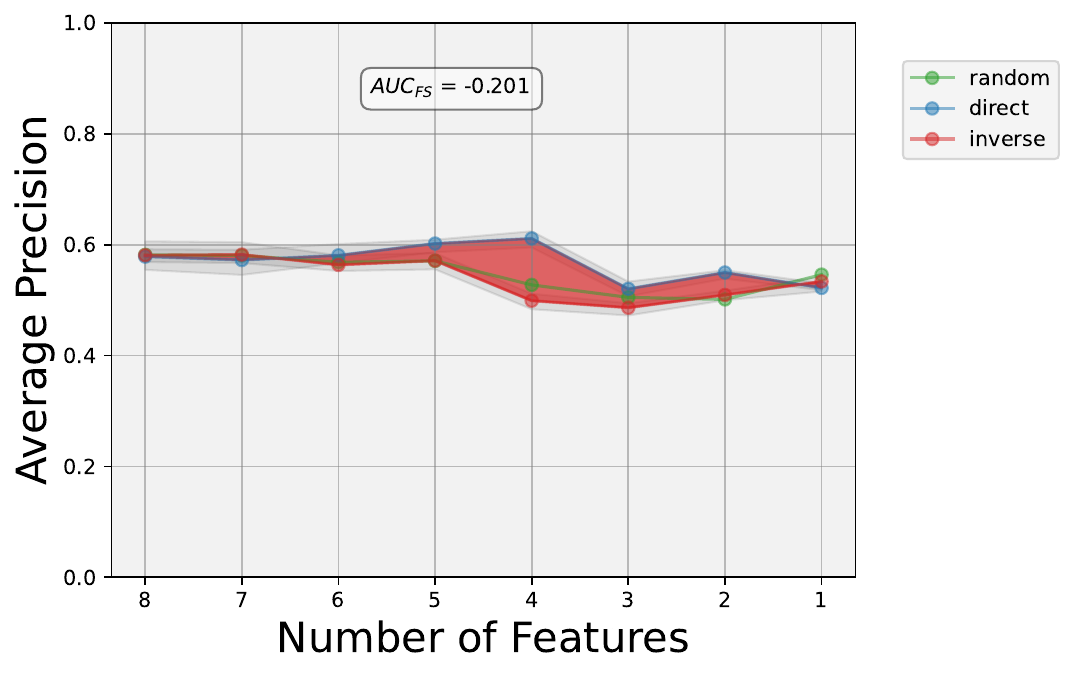}
            \caption{\approach applied to EIF}
            \label{fig:Feat-Sel_Pima_valEIF+_EXIFFI_2}
        \end{subfigure}\hfill
        \begin{subfigure}[t]{0.30\textwidth}
            \centering
            \includegraphics[trim={0 0 3.5cm 0}, clip, width=\linewidth]{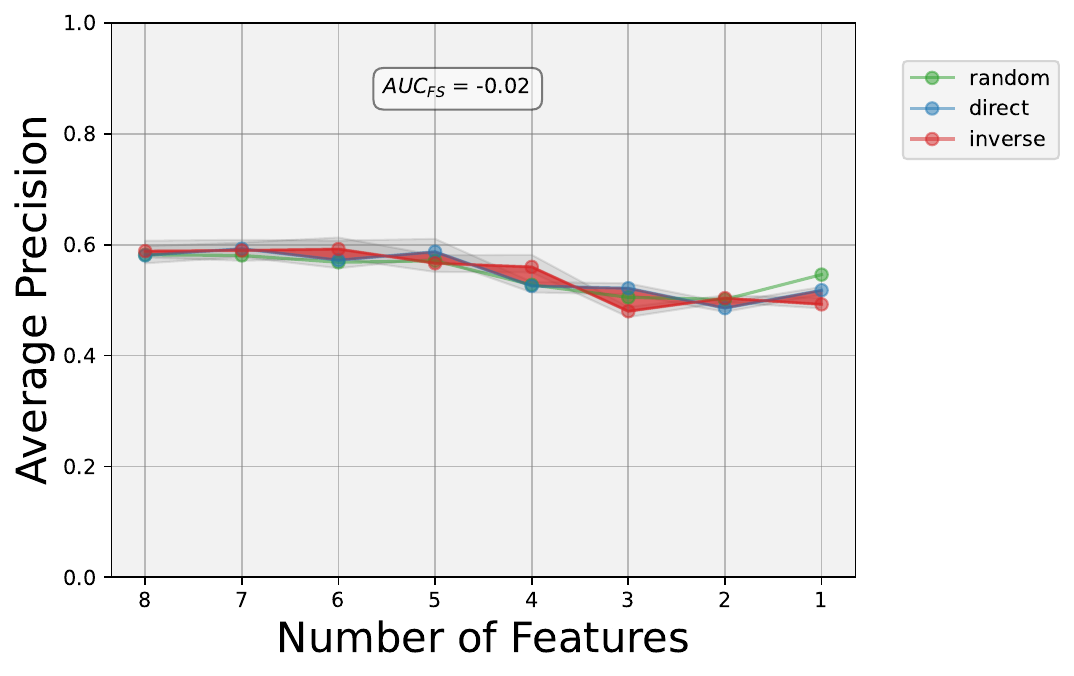}
            \caption{\approach applied to \EIFplus}
            \label{fig:Feat-Sel_Pima_valEIF+_EXIFFI+_2}
        \end{subfigure}
    \end{minipage}
\end{minipage}

\vspace{5mm} % Space between rows

% Second row with vertical caption on the left
\begin{minipage}{\textwidth}
    \rotatebox{90}{\parbox{15mm}{\centering \textbf{Post-Hoc}}} % Adjust as necessary
    \begin{minipage}{0.95\textwidth}
        \begin{subfigure}[t]{0.30\textwidth}
            \centering
            \includegraphics[trim={0 0 3.5cm 0}, clip, width=\linewidth]{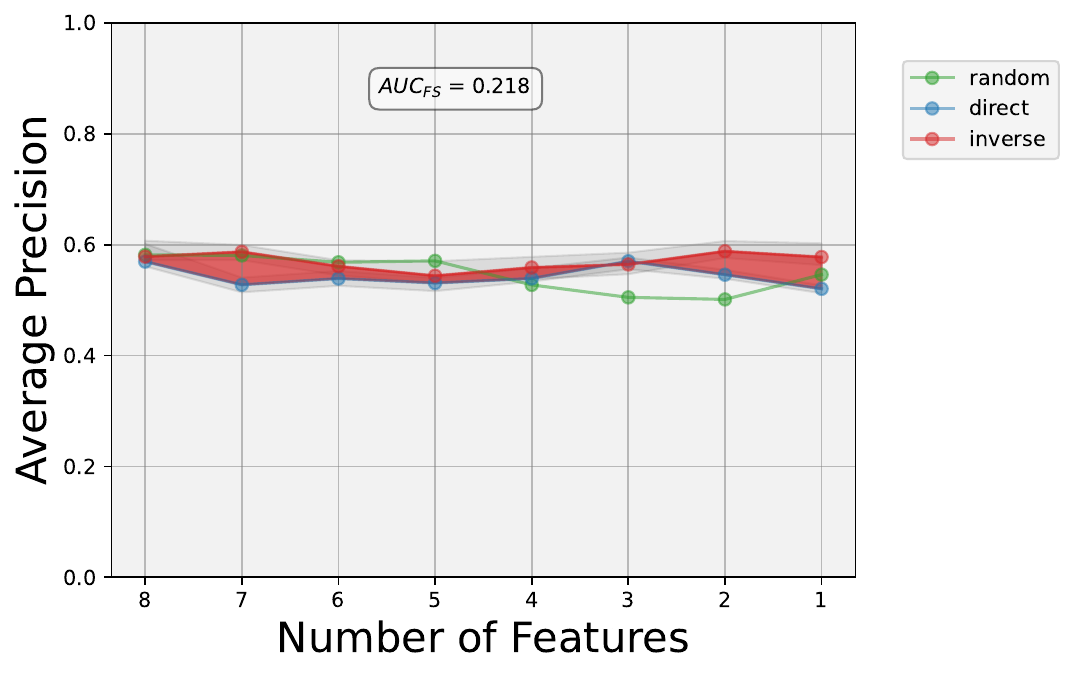}
            \caption{RandomForest fitted to IF}
            \label{fig:Feat-Sel_Pima_valEIF+_IF_RandomForest_2}
        \end{subfigure}\hfill
        \begin{subfigure}[t]{0.30\textwidth}
            \centering
            \includegraphics[trim={0 0 3.5cm 0}, clip, width=\linewidth]{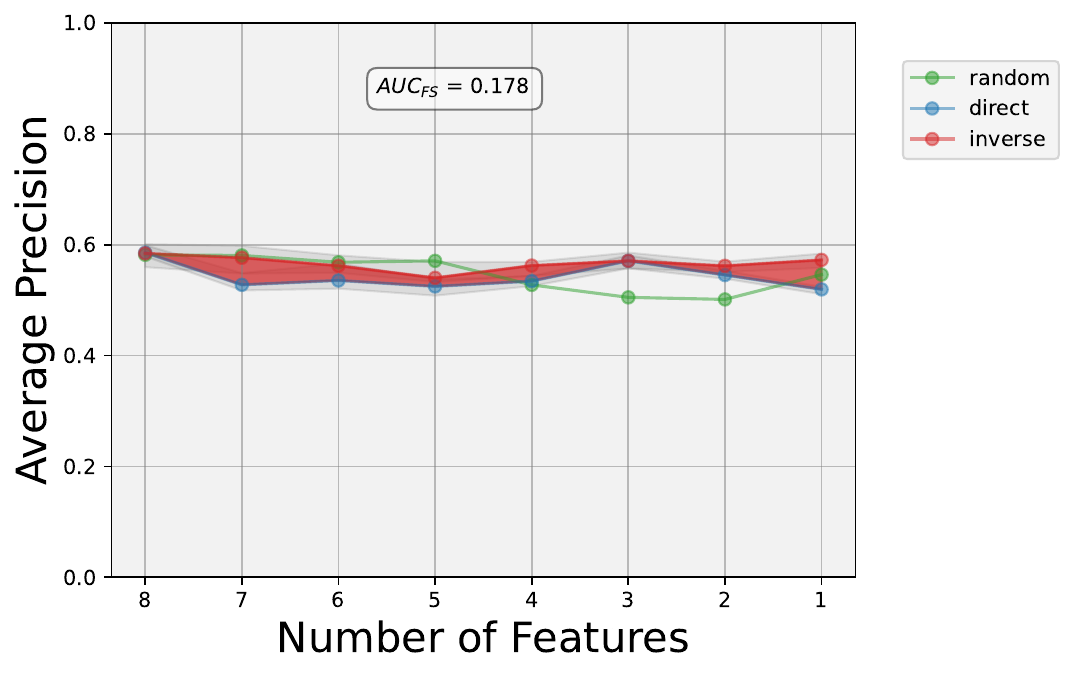}
            \caption{RandomForest fitted to EIF}
            \label{fig:Feat-Sel_Pima_valEIF+_EIF_RandomForest_2}
        \end{subfigure}\hfill
        \begin{subfigure}[t]{0.30\textwidth}
            \centering
            \includegraphics[trim={0 0 3.5cm 0}, clip, width=\linewidth]{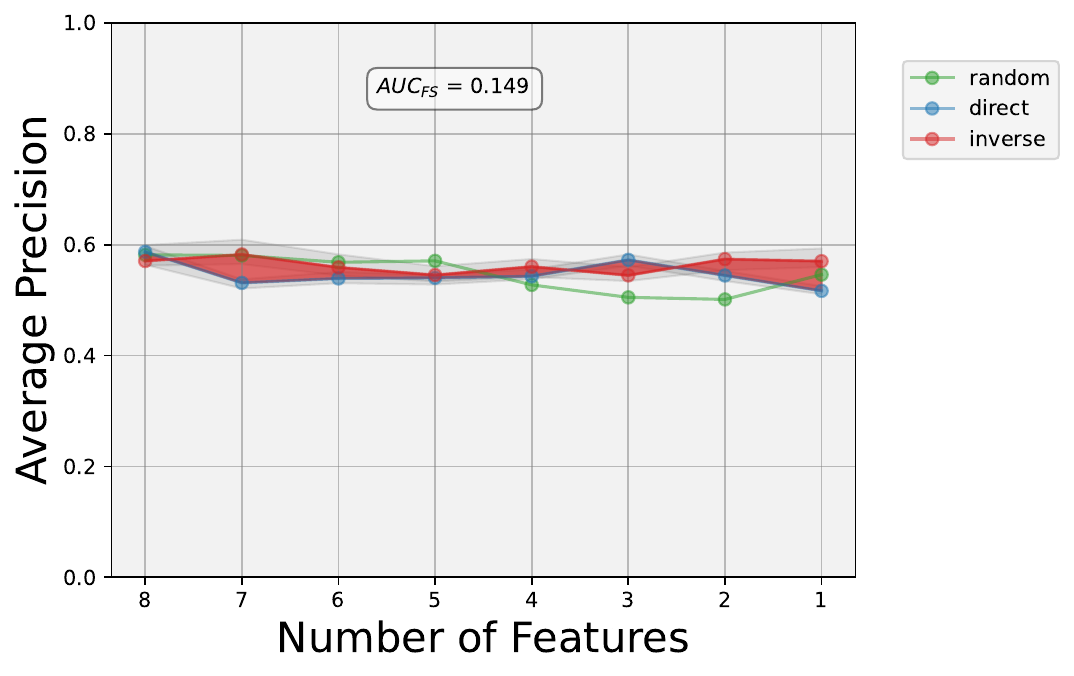}
            \caption{RandomForest fitted to \EIFplus}
            \label{fig:Feat-Sel_Pima_valEIF+_EIF+_RandomForest_2}
        \end{subfigure}
    \end{minipage}
\end{minipage}

\caption{Feature Selection of the different Ad-Hoc and Post-Hoc methods applied to the 3 Isolation Forest models: IF, EIF and \EIFplus. The blue line is the values of average precision, calculated with the \EIFplus model in the Scenario II, dropping the most important feature at each step, the red line is the values of average precision dropping the least important feature at each step and the green line is the value of the feature selection dropping a random feature at each step.}\label{fig:fs-interpretaion-Pima}
\end{figure}

\ale{The values of the $AUC_{FS}$ metric are grouped together in Table \ref{tab:fs-tab-Pima}. As previously explained the best interpretation method in quantitative terms is IF\_\approach although not presenting significant values of the metric. For what concerns the remaining approaches considered their scores are mostly close to zero or negative, as a consequence of the flat shapes observed in the Feature Selection plots.}

\subsection*{{\ttfamily Shuttle}}

\subsubsection{Performance}

\ale{Figure \ref{fig:Shuttle_contamination_full} displays changes in the Average Precision metric as the contamination level of the training set used for the fitting process of the AD models considered in this study increased from 0 to 10 \%. The \EIFplus and DIF model present a decreasing trend proving once again how these methods, \EIFplus in particular, are more suitable for datasets in which the contamination is limited. As it can be observed in Figure \ref{fig:Shuttle_contaminationEIFvsEIF+} the EIF model achieves sligthly better performances than \EIFplus in this particular dataset.} 

\begin{figure}[!ht] 
    \centering % <-- added
    \begin{subfigure}[t]{0.49\textwidth}
      \includegraphics[width=\linewidth]{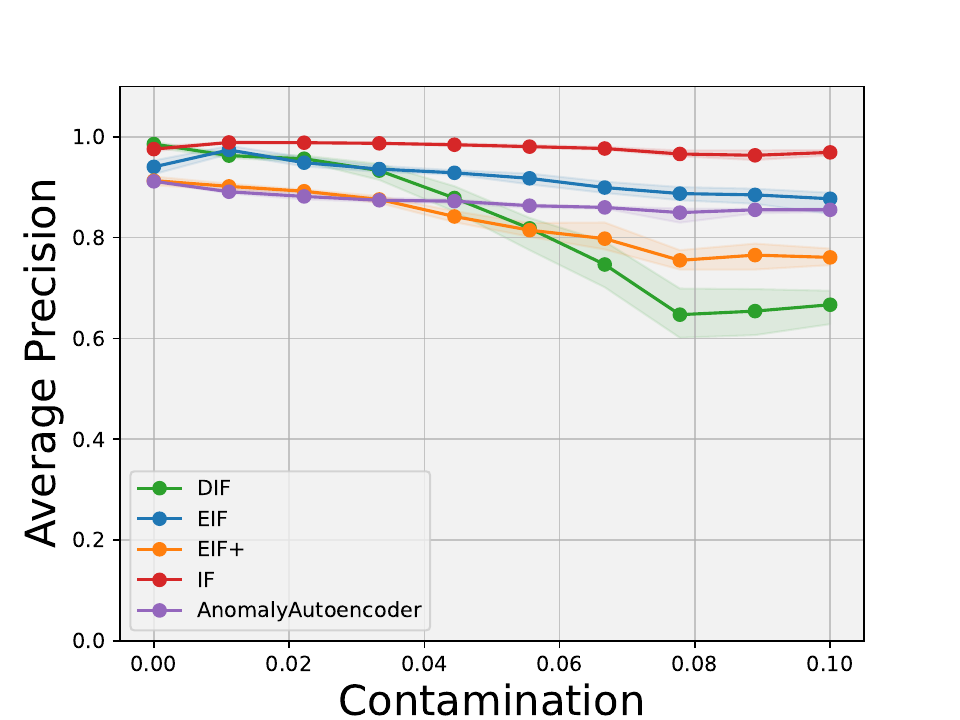}
      \caption{Models evaluation, varying the contamination levels}
      \label{fig:Shuttle_contamination_full}
    \end{subfigure}\hfil % <-- added
    \begin{subfigure}[t]{0.44\textwidth}
      \includegraphics[width=\linewidth]{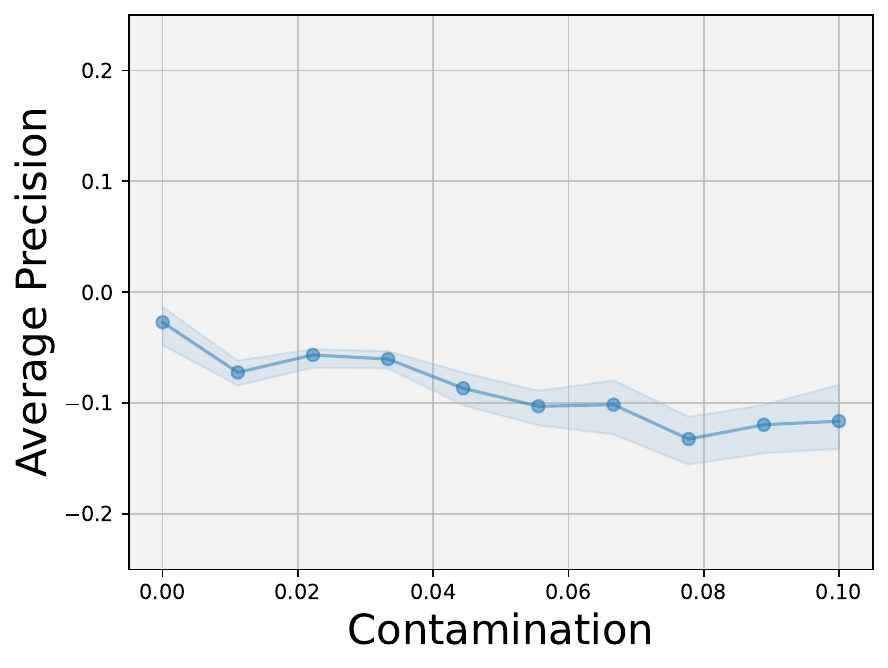}
      \caption{Difference between \EIFplus and EIF average precision}
      \label{fig:Shuttle_contaminationEIFvsEIF+}
    \end{subfigure}\hfil % <-- added
\caption{Figure \ref{fig:Shuttle_contamination_full} illustrates the average precision as the contamination level in the training set increases. Figure \ref{fig:Shuttle_contaminationEIFvsEIF+} compares the performance graphs of EIF and \EIFplus, using the difference of their scores in various contamination levels.}
\label{fig:Shuttle_contamination}
\end{figure}

\ale{A comparison between Classification reports of the AD models in Scenario I and Scenario II is reported in Table \ref{tab:Shuttle_perf}. The IF model can be considered the best according to the metric values but it is worth noticing the significant improvement of the proposed \EIFplus model passing from Scenario I to Scenario II.} 

\begin{table}[htbp]
\begin{minipage}[t]{0.46\textwidth}
\strut\vspace*{-\baselineskip}\newline
\resizebox{\textwidth}{!}{
\begin{tabular}{|c||ccc|ccc||cc|}
\toprule
\hline
&\multicolumn{3}{c|}{Scenario I}&\multicolumn{3}{c||}{Scenario II}&\multicolumn{2}{c|}{Time}\\
\hline
AD Model & Avg & Prec & ROC & Avg & Prec & ROC & fit & pred \\
& Prec &  & AUC & Prec &  & AUC &  &  \\
\hline
IF          & \textbf{0.98}& \textbf{0.96}& \textbf{0.97}& \textbf{0.98}& \textbf{0.97}& \textbf{0.98}& 0.21& \textbf{0.06}\\
EIF         & 0.90& 0.87& 0.93& 0.97& 0.95& 0.97& \textbf{0.16}& 0.54\\
EIF+        & 0.70& 0.71& 0.84& 0.91& 0.96& 0.97& 0.20& 0.36\\
DIF         & 0.54& 0.60& 0.78& \textbf{0.99}& \textbf{0.97}& \textbf{0.98}& 10.5& 9.02\\
AE & 0.90& 0.95& 0.97& 0.90& 0.94& 0.97& 19.6& 0.25\\
\hline
\end{tabular}}
\vspace{0.41cm}
\caption{Performances of 5 different Anomaly Detection models over {\ttfamily Shuttle} are compared using classical Classification metrics. Moreover, the last two columns contain the average time for a fit and predict operation. The highest metric values and the lowest execution times are highlighted in bold}\label{tab:Shuttle_perf}
\end{minipage}
\hfill
\begin{minipage}[t]{0.46\textwidth}
\strut\vspace*{-\baselineskip}\newline
\resizebox{\textwidth}{!}{
\begin{tabular}{|c||c|c|c|c||c|}
\toprule
\hline
&\multicolumn{2}{c|}{Evaluation with EIF}&\multicolumn{2}{c||}{Evaluation with \EIFplus}&\\
\hline
& Scenario I & Scenario II & Scenario I & Scenario II & Time\\

 Algorithm & $AUC_{FS}$  & $AUC_{FS}$ & $AUC_{FS}$  & $AUC_{FS}$ &  \\
\hline
DIFFI                    & -0.514& -1.487& -0.693& -1.456& 0.95\\
IF\_\approach             & \textbf{2.764}& \textbf{2.881}& \textbf{2.789}& \textbf {3.079}& \textbf{0.89}\\
EIF\_\approach            & -1.432& 0.766& 1.223& 0.315& 1.38\\
\EIFplus\_\approach       & 0.459& 0.019& 0.736& -0.131& 1.39\\
IF\_RF                   & 0.440& 0.904& 0.360& 0.648& 2.33\\
EIF\_RF                  & 1.692& 2.747& 1.733& 2.112& 2.33\\
EIF+\_RF                 & 1.904& 2.138& 1.628& 2.117& 2.33\\
\hline
\end{tabular}}
\caption{Quantitative evaluation of the effectiveness of 6 different interpretation algorithms on {\ttfamily Shuttle} through the $AUC_{FS}$ metric, introduced in \ref{sec:interpr_evaluat}. In the last column the average time taken by the different models to produce the importance scores is reported. The highest $AUC_{FS}$ and lowest Importance time values are highlighted in bold.}\label{tab:fs-tab-Shuttle}
\end{minipage}
\end{table}

\subsubsection{Importance Plots}

\ale{Similarly to the {\ttfamily Pima} dataset also in {\ttfamily Shuttle} anomalies are superimposed to the inliers distribution, as observable in the Local Scoremaps depicted in Figures \ref{fig:Local-Shuttle} and \ref{fig:Local-Shuttle-split} thus also for this dataset the explanations produced should be evaluated with care. Comparing the feature rankings produced in the Score Plots in Figure \ref{fig:Feat-imp-Shuttle} and \ref{fig:Feat-imp-Shuttle-split} a feature that should be considered as relevant is Feature 0 since it is placed in second position in both Scenario I and II. }

\begin{figure}[!ht] 
    \centering % <-- added
    \begin{subfigure}[t]{0.33\textwidth}
    \centering
      \includegraphics[width=\linewidth]{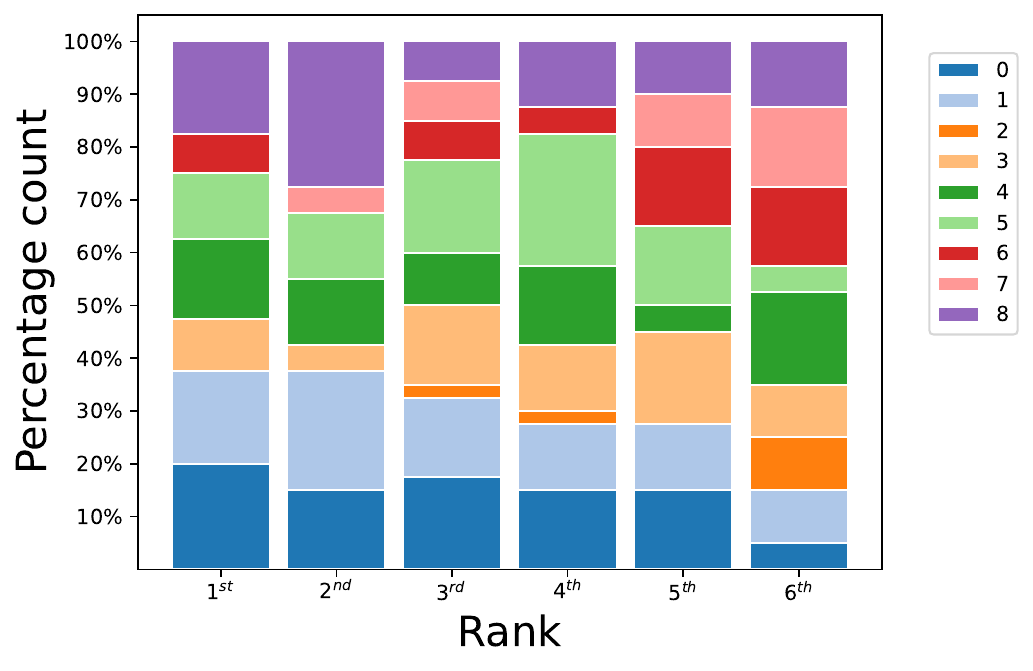}
      \caption{Bar Plot {\ttfamily Shuttle} Scenario I}
      \label{fig:GFI-Shuttle}
    \end{subfigure}\hfil % <-- added
    \begin{subfigure}[t]{0.27\textwidth}
    \centering
      \includegraphics[width=\linewidth]{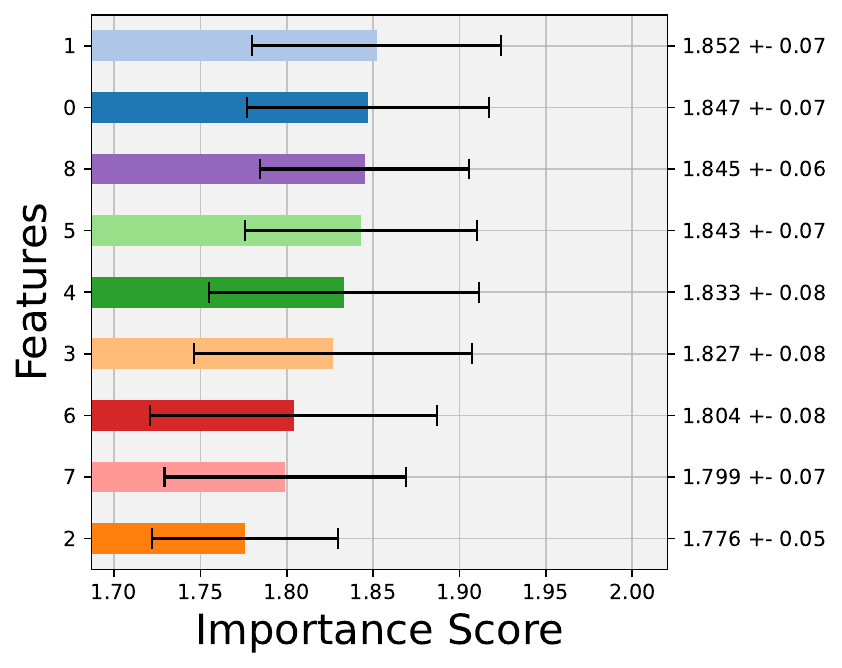}
      \caption{Score Plot {\ttfamily Shuttle} Scenario I}
      \label{fig:Feat-imp-Shuttle}
    \end{subfigure}\hfil % <-- added
    \begin{subfigure}[t]{0.28\textwidth}
    \centering
      \includegraphics[width=\linewidth]{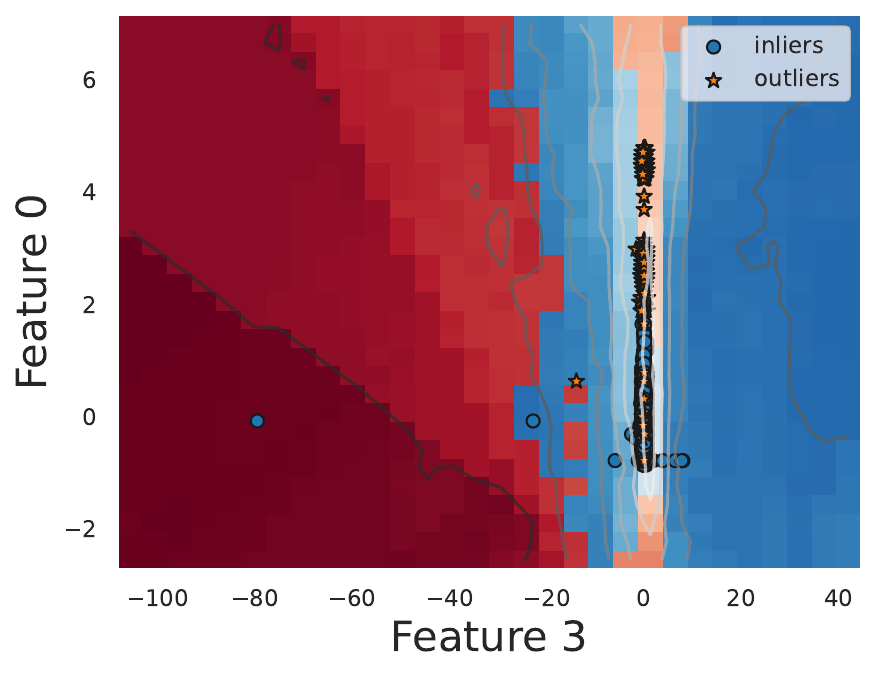}
      \caption{Scoremap {\ttfamily Shuttle} Scenario I}
      \label{fig:Local-Shuttle}
    \end{subfigure}\hfil % <-- added
    \begin{subfigure}[t]{0.33\textwidth}
    \centering
      \includegraphics[width=\linewidth]{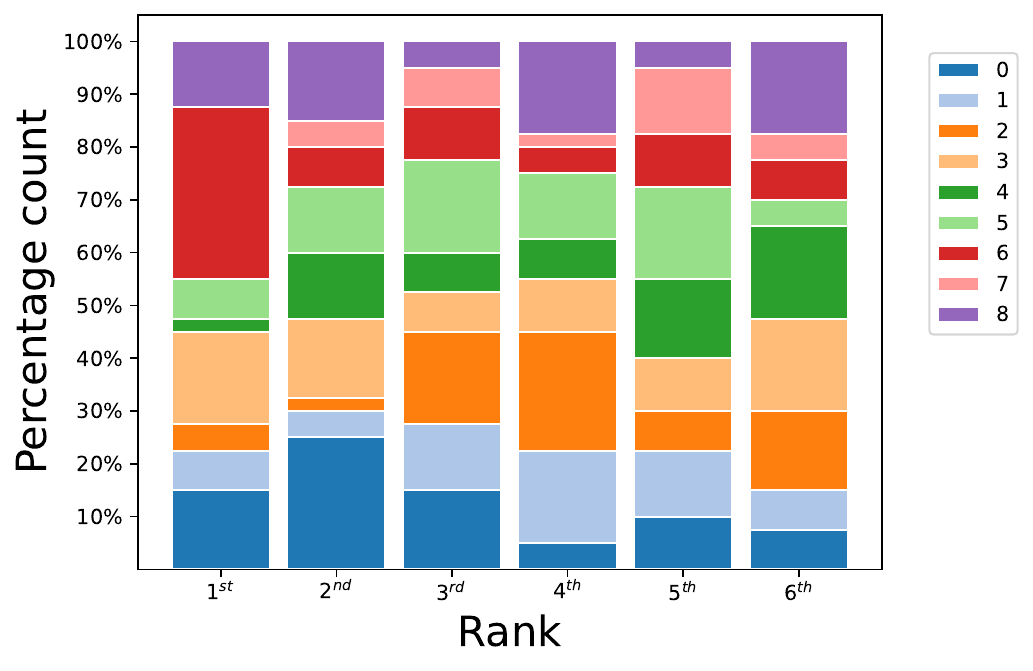}
      \caption{Bar Plot {\ttfamily Shuttle} Scenario II}
      \label{fig:GFI-Shuttle-split}
    \end{subfigure}\hfil % <-- added
    \begin{subfigure}[t]{0.27\textwidth}
    \centering
      \includegraphics[width=\linewidth]{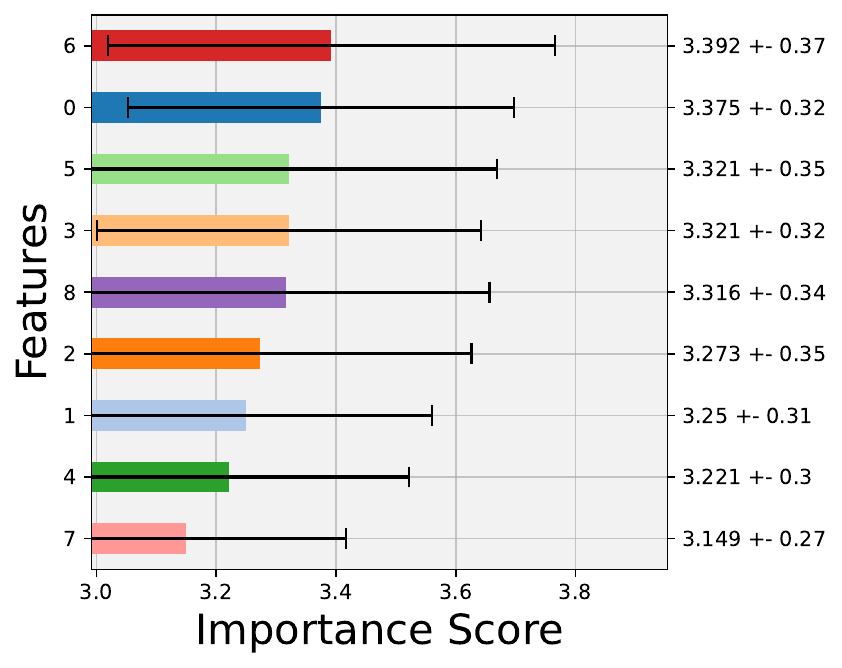}
      \caption{Score Plot {\ttfamily Shuttle} Scenario II}
      \label{fig:Feat-imp-Shuttle-split}
    \end{subfigure}\hfil % <-- added
    \begin{subfigure}[t]{0.28\textwidth}
    \centering
      \includegraphics[width=\linewidth]{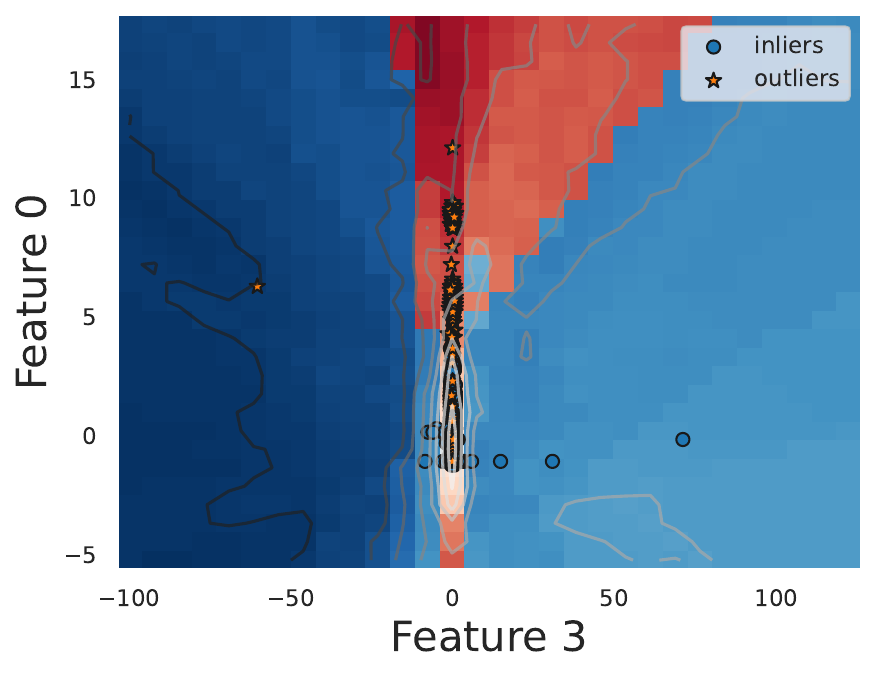}
      \caption{Scoremap {\ttfamily Shuttle} Scenario II}
      \label{fig:Local-Shuttle-split}
    \end{subfigure}\hfil % <-- added
\caption{Bar Plot, Score Plot and Scoremap for {\ttfamily Shuttle} in the two different Scenarios, using the \approach algorithm applied to the \EIFplus model.}\label{fig:interpretation-Shuttle}
\end{figure}

\subsubsection{Feature Selection} \label{sec:Shuttle-fs}

\ale{Feature Selection plots for the {\ttfamily Shuttle} dataset are grouped together in Figure \ref{fig:fs-interpretation-Shuttle}. The best results are achieved by \approach applied to IF and by the post-hoc interpretability methods exploited to explain the EIF and \EIFplus models. Both these three plots, reported in Figures \ref{fig:Feat-Sel_Shuttle_valEIF+_DIFFI_2}, \ref{fig:Feat-Sel_Shuttle_valEIF+_EIF_RandomForest_2} and \ref{fig:Feat-Sel_Shuttle_valEIF+_EIF+_RandomForest_2}, share a common behavior: as features are removed in increasing order of importance (red line) the Average Precision scores show a constant behavior while in the blue line, representing the approach in which attributes are omitted in decreasing order of importance, a significant drop in the scores can be observed passing from 5 to 4 features. A possible interpretation of this peculiar phenomenon may be related to the removal of all the relevant features leaving only the redundant and uninformative ones leading the Average Precision scores to be reduced under the value of 0.4.
On the other hand in Figures related to the \approach and \approach+ models (Figures \ref{fig:Feat-Sel_Shuttle_valEIF+_EXIFFI_2}, \ref{fig:Feat-Sel_Shuttle_valEIF+_EXIFFI+_2}) the red line presents a decreasing trend leading to small (if not negative) values of the $AUC_{FS}$ metric.}

\begin{comment}
Because of the peculiar distribution of the data points, that violates the typical properties anomalies are intended to have, post-hoc interpretation methods achieve better results than Isolation-based models. In fact in Figures \ref{fig:Feat-Sel_Shuttle_valEIF+_IF_RandomForest_2}, \ref{fig:Feat-Sel_Shuttle_valEIF+_EIF_RandomForest_2}, \ref{fig:Feat-Sel_Shuttle_valEIF+_EIF+_RandomForest_2} are associated with a constant trend in Average Precision as features are removed in increasing order of importance (red line) while precision decreases as features are excluded from the input space in decreasing order or relevance (blue line). 
\end{comment}

\begin{figure}[!ht] 
\centering
\hspace{0.05\textwidth}\textbf{IF} \hspace{0.29\textwidth} \textbf{EIF} \hspace{0.29\textwidth} \textbf{EIF+}
% First row with vertical caption on the left
\begin{minipage}{\textwidth}
    \rotatebox{90}{\parbox{15mm}{\centering \textbf{Ad-Hoc}}} % Adjust the parbox width as necessary for your caption text
    \begin{minipage}{0.95\textwidth}
        \begin{subfigure}[t]{0.30\textwidth}
            \centering
            \includegraphics[trim={0 0 3.5cm 0}, clip, width=\linewidth]{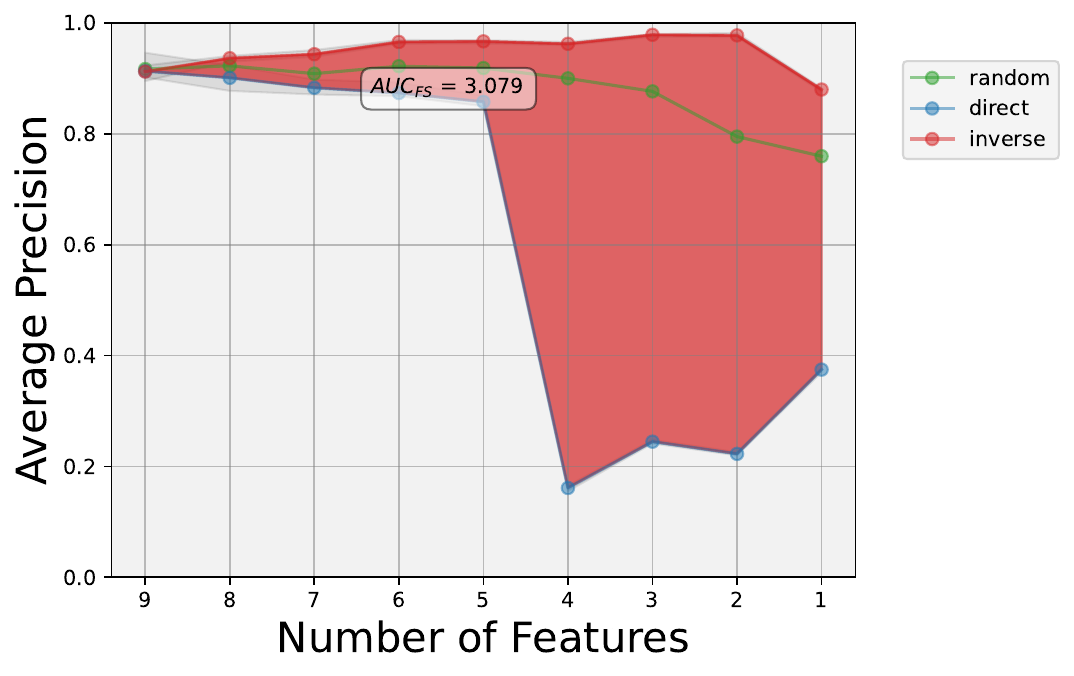}
            \caption{\approach applied to IF}
            \label{fig:Feat-Sel_Shuttle_valEIF+_DIFFI_2}
        \end{subfigure}\hfill
        \begin{subfigure}[t]{0.30\textwidth}
            \centering
            \includegraphics[trim={0 0 3.5cm 0}, clip, width=\linewidth]{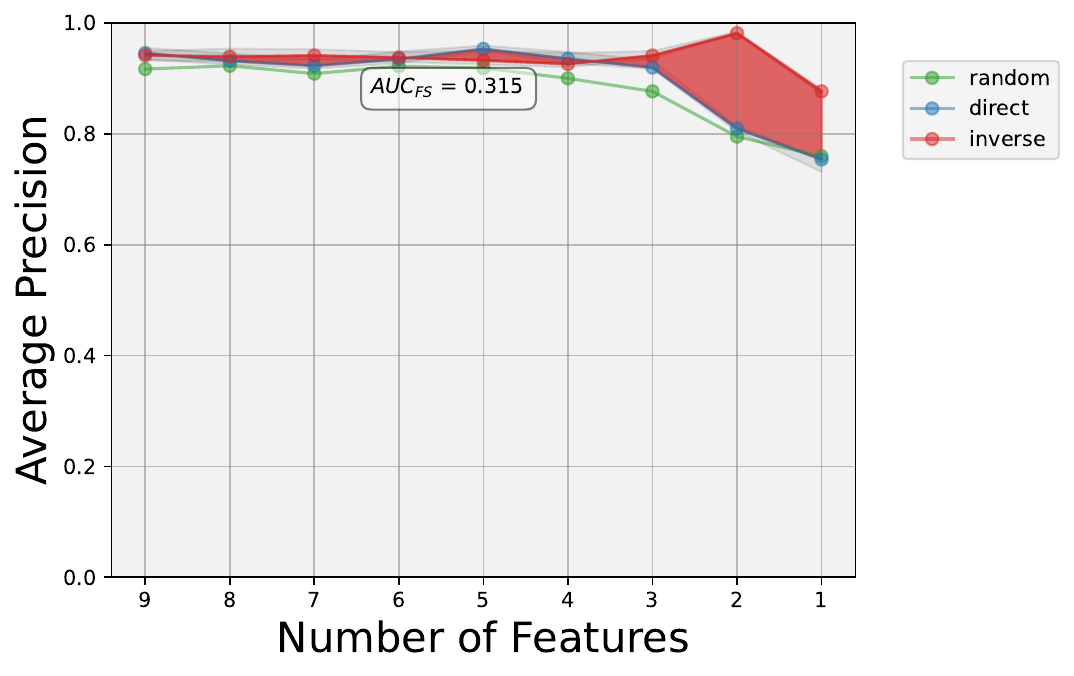}
            \caption{\approach applied to EIF}
            \label{fig:Feat-Sel_Shuttle_valEIF+_EXIFFI_2}
        \end{subfigure}\hfill
        \begin{subfigure}[t]{0.30\textwidth}
            \centering
            \includegraphics[trim={0 0 3.5cm 0}, clip, width=\linewidth]{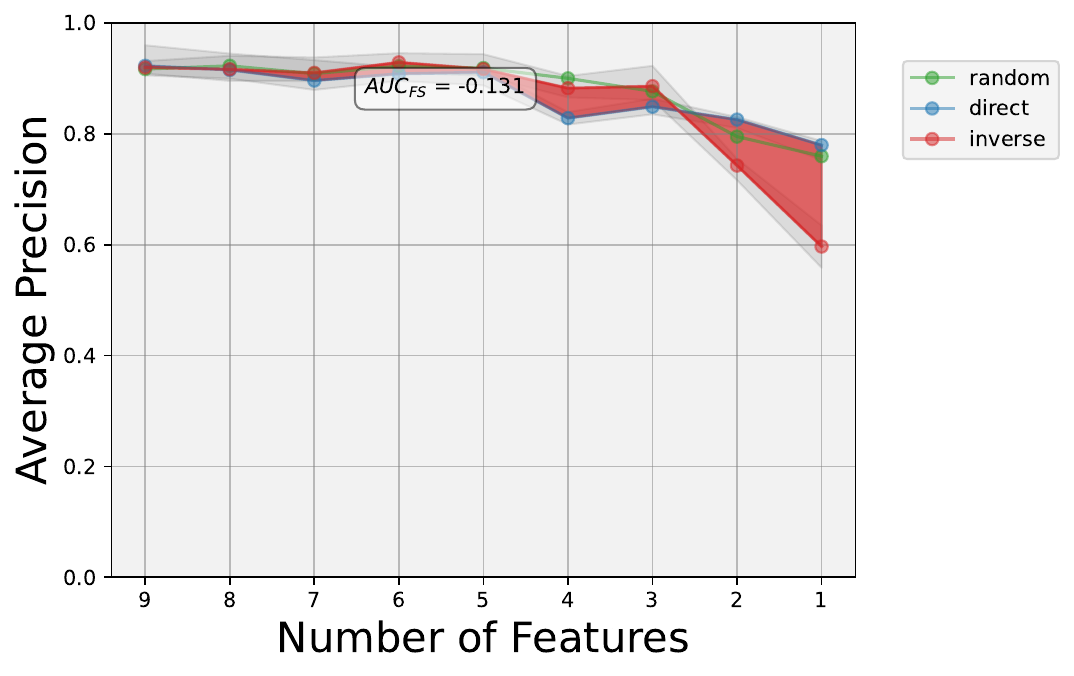}
            \caption{\approach applied to \EIFplus}
            \label{fig:Feat-Sel_Shuttle_valEIF+_EXIFFI+_2}
        \end{subfigure}
    \end{minipage}
\end{minipage}

\vspace{5mm} % Space between rows

% Second row with vertical caption on the left
\begin{minipage}{\textwidth}
    \rotatebox{90}{\parbox{15mm}{\centering \textbf{Post-Hoc}}} % Adjust as necessary
    \begin{minipage}{0.95\textwidth}
        \begin{subfigure}[t]{0.30\textwidth}
            \centering
            \includegraphics[trim={0 0 3.5cm 0}, clip, width=\linewidth]{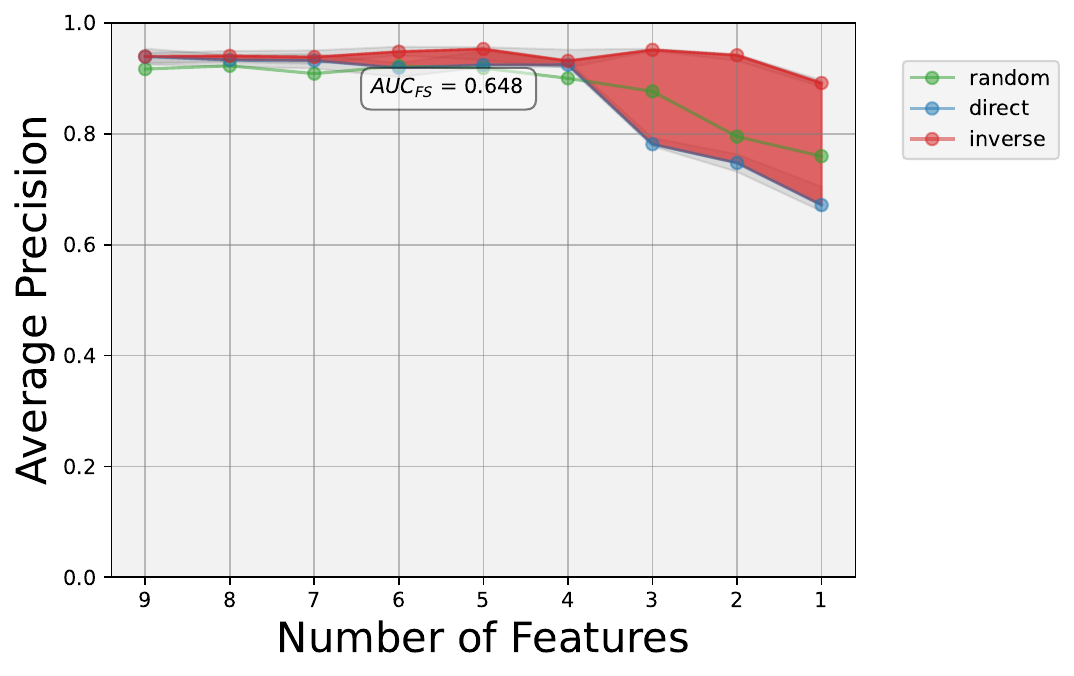}
            \caption{RandomForest fitted to IF}
            \label{fig:Feat-Sel_Shuttle_valEIF+_IF_RandomForest_2}
        \end{subfigure}\hfill
        \begin{subfigure}[t]{0.30\textwidth}
            \centering
            \includegraphics[trim={0 0 3.5cm 0}, clip, width=\linewidth]{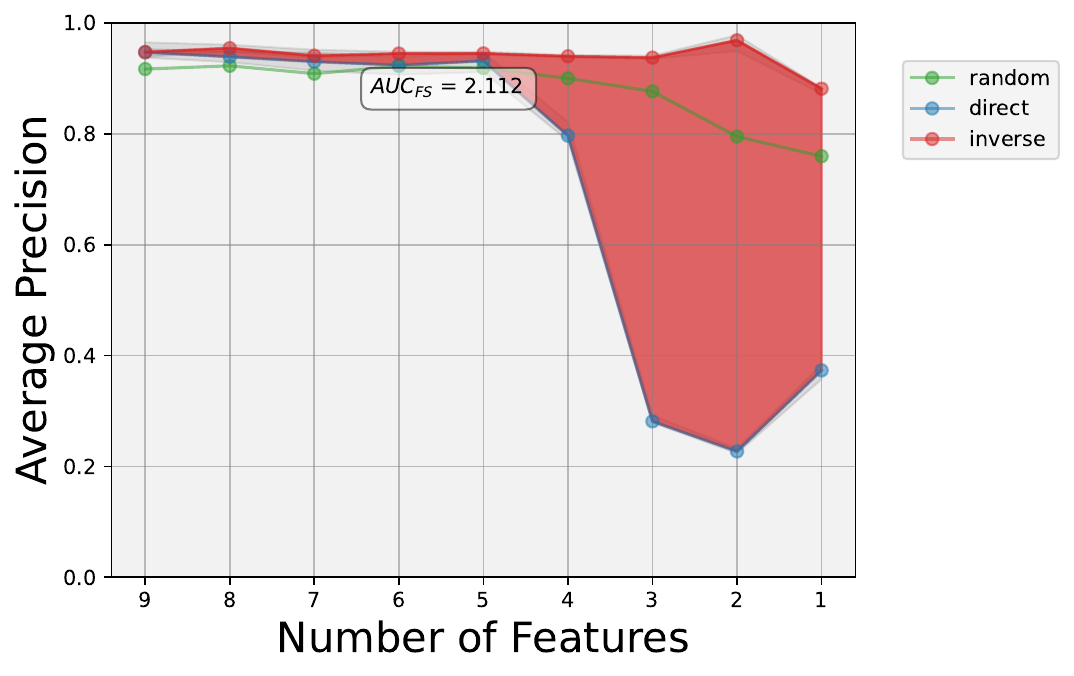}
            \caption{RandomForest fitted to EIF}
            \label{fig:Feat-Sel_Shuttle_valEIF+_EIF_RandomForest_2}
        \end{subfigure}\hfill
        \begin{subfigure}[t]{0.30\textwidth}
            \centering
            \includegraphics[trim={0 0 3.5cm 0}, clip, width=\linewidth]{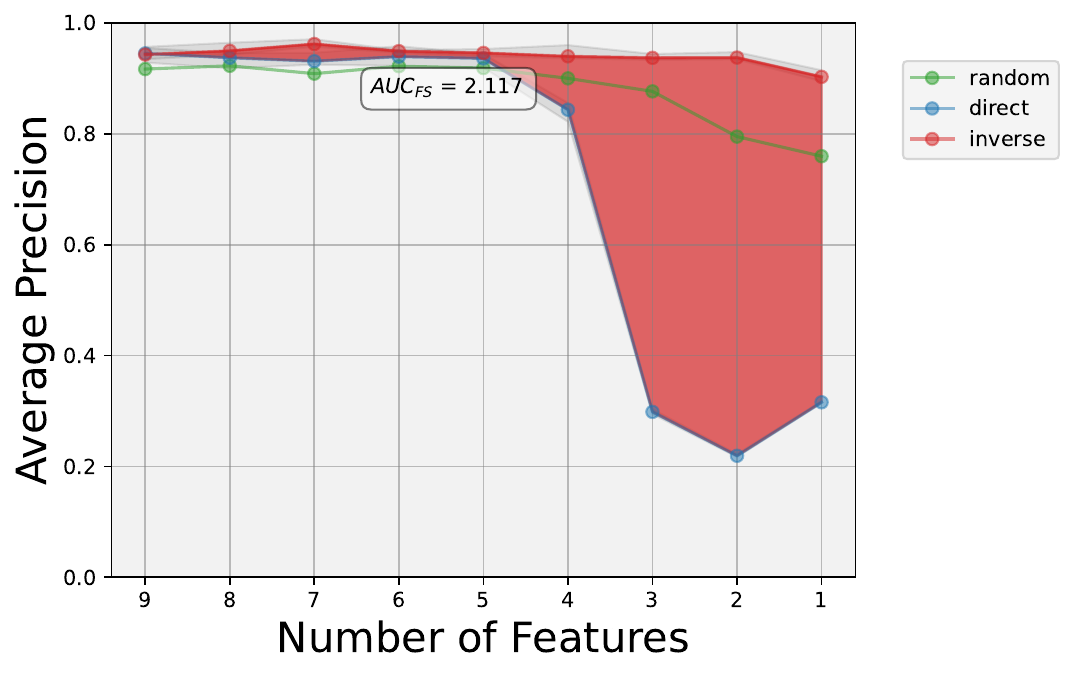}
            \caption{RandomForest fitted to \EIFplus}
            \label{fig:Feat-Sel_Shuttle_valEIF+_EIF+_RandomForest_2}
        \end{subfigure}
    \end{minipage}
\end{minipage}

\caption{Feature Selection of the different Ad-Hoc and Post-Hoc methods applied to the 3 Isolation Forest models: IF, EIF and \EIFplus. The blue line is the values of average precision, calculated with the \EIFplus model in the Scenario II, dropping the most important feature at each step, the red line is the values of average precision dropping the least important feature at each step and the green line is the value of the feature selection dropping a random feature at each step.}\label{fig:fs-interpretation-Shuttle}
\end{figure}

\ale{Table \ref{tab:fs-tab-Shuttle} contains the $AUC_{FS}$ metrics values for all the combinations of interpretation and evaluation model both for Scenario I and Scenario II. As already discussed in \ref{sec:Shuttle-fs} three models (i.e. IF\_\approach, EIF\_RandomForest and \EIFplus\_RandomForest) showcase superior quantitative outcomes. On the other hand, the $AUC_{FS}$ values of the proposed interpretation algorithms \approach and \approach+, even though faster than post-hoc methods, are lower and in some cases also negative.}

\subsection*{{\ttfamily Wine}}

\subsubsection{Performance}

\ale{The Contamination plot, depicted in Figure \ref{fig:Wine_contamination_full}, shows how the Average Precision of all the Anomaly Detection models considered diminishes as outliers are progressively included as part of the training set. \EIFplus is the model with the best metric values for low values of the contamination parameter confirming another time its effectiveness in datasets with a limited number of outliers as {\ttfamily Wine}. Moreover Figure \ref{fig:Wine_contaminationEIFvsEIF+} , that represents the difference in the Average Precision values of the EIF and \EIFplus, enhances the superiority of the proposed model with the respect to its counterpart.} 

\begin{figure}[!ht] 
    \centering % <-- added
    \begin{subfigure}[t]{0.49\textwidth}
      \includegraphics[width=\linewidth]{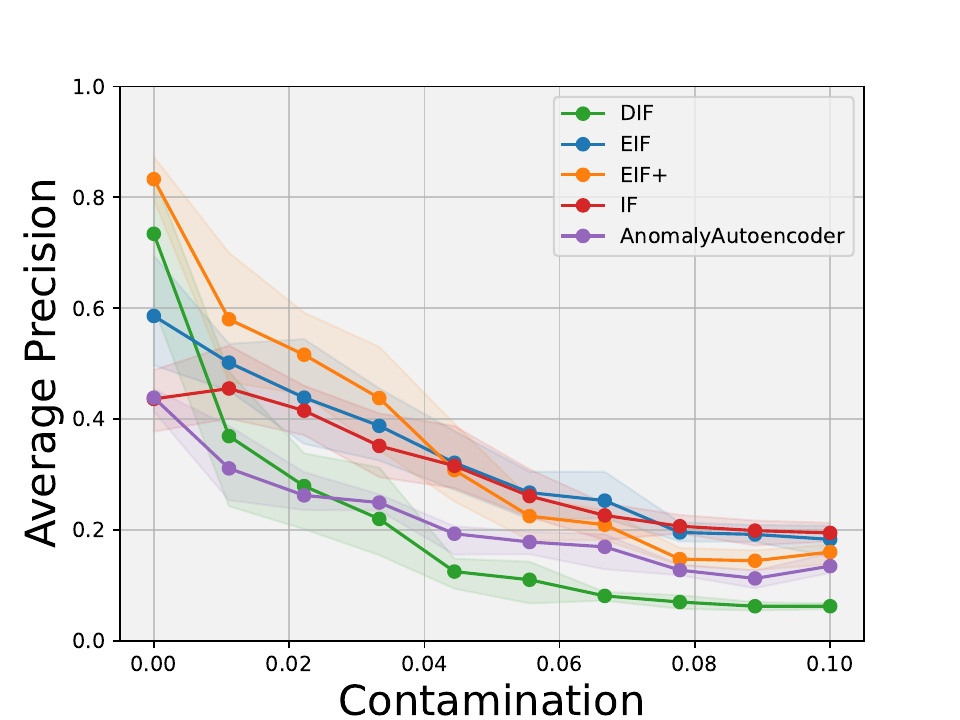}
      \caption{ }
      \label{fig:Wine_contamination_full}
    \end{subfigure}\hfil % <-- added
    \begin{subfigure}[t]{0.44\textwidth}
      \includegraphics[width=\linewidth]{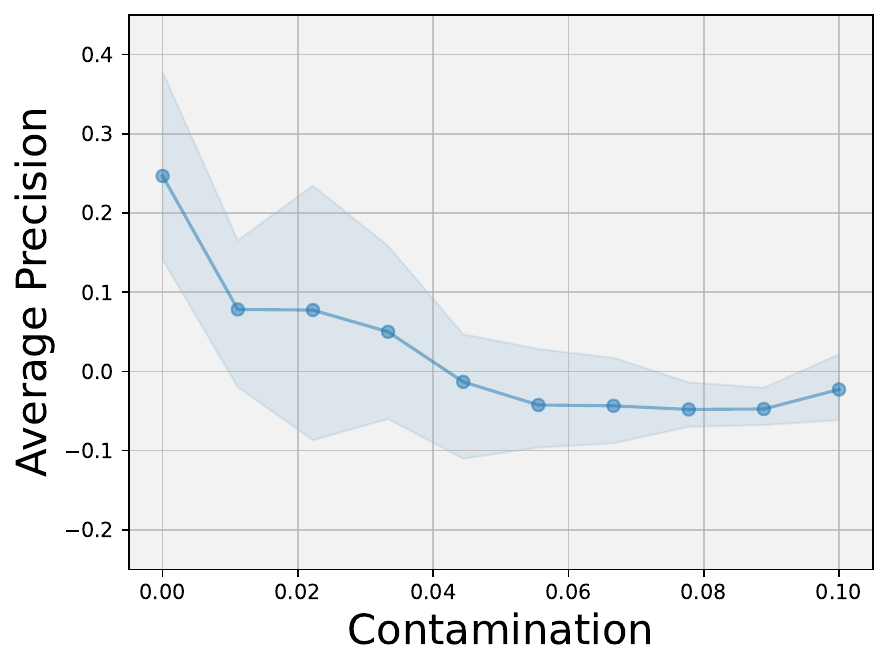}
      \caption{ }
      \label{fig:Wine_contaminationEIFvsEIF+}
    \end{subfigure}\hfil % <-- added
\caption{Fig. \ref{fig:Wine_contamination_full} Represent the average precision the more the level of contamination of the train set is increased. The Fig. \ref{fig:Wine_contaminationEIFvsEIF+} Give show specifically the graphs of the EIF and EIF+}
\label{fig:Wine_contamination}
\end{figure}

\ale{Table \ref{tab:Wine_perf}  provides a comprehensive comparison of the performances of the different methods analyzed in this study in the two different evaluation scenarios described in \ref{sec:interpr_evaluat} . In Scenario I the performances of Isolation based models (i.e. IF, EIF and \EIFplus) overcome the ones of  deep learning based approaches (i.e. DIF and Autoencoder) while in Scenario II \EIFplus stands out as the best performing model. Referring to the computational efficiency argument there is a clear separation between Isolation based and deep learning based models with the first ones being the fastest in fitting the model and providing predictions on new samples.}

\begin{table}[htbp]
\begin{minipage}[t]{0.46\textwidth}
\strut\vspace*{-\baselineskip}\newline
\resizebox{\textwidth}{!}{
\begin{tabular}{|c||ccc|ccc||cc|}
\toprule
\hline
&\multicolumn{3}{c|}{Scenario I}&\multicolumn{3}{c||}{Scenario II}&\multicolumn{2}{c|}{Time}\\
\hline
AD Model & Avg & Prec & ROC & Avg & Prec & ROC & fit & pred \\
& Prec &  & AUC & Prec &  & AUC &  & pred \\
\hline
IF          & \textbf{0.26}& \textbf{0.20}& \textbf{0.56}& 0.61& 0.50& 0.72& 0.10& \textbf{0.002}\\
EIF         & 0.21& 0.20& 0.56& 0.57& 0.60& 0.78& \textbf{0.09}& 0.005\\
EIF+        & 0.17& 0.00& 0.45& \textbf{0.79}& \textbf{0.70}& \textbf{0.83}& 0.10& \textbf{0.002}\\
DIF         & 0.07& 0.00& 0.45& 0.72& 0.70& 0.83& 0.57& 0.210\\
AE          & 0.14& 0.10& 0.51& 0.45& 0.50& 0.72& 2.13& 0.040\\
\hline
\end{tabular}}
\vspace{0.41cm}
\caption{Performances of 5 different Anomaly Detection models over {\ttfamily Wine} are compared using classical Classification metrics. Moreover the last two columns contain the average time for a fit and predict operation. The highest metric values and the lowest execution times are highlighted in bold}\label{tab:Wine_perf}
\end{minipage}
\hfill
\begin{minipage}[t]{0.46\textwidth}
\strut\vspace*{-\baselineskip}\newline
\resizebox{\textwidth}{!}{
\begin{tabular}{|c||c|c|c|c||c|}
\toprule
\hline
&\multicolumn{2}{c|}{Evaluation with EIF}&\multicolumn{2}{c||}{Evaluation with \EIFplus}&\\
\hline
& Scenario I & Scenario II & Scenario I & Scenario II & Time\\

 Algorithm & $AUC_{FS}$  & $AUC_{FS}$ & $AUC_{FS}$  & $AUC_{FS}$ &  \\
\hline
DIFFI                & 0.176& -3.799& 0.437& -3.491& 0.33\\
IF\_\approach        & \textbf{0.682}& 8.076& \textbf{0.628}& \textbf{9.401}& 0.07\\
EIF\_\approach       & 0.451& 7.122& 0.459& 8.120& \textbf{0.01}\\
\EIFplus\_\approach  & 0.127& \textbf{9.000}& 0.180& 9.25& 0.01\\
IF\_RF               & -3.093& 4.413& -2.339& 4.539& 0.18\\
EIF\_RF              & -2.415& 3.946& -1.570& 4.369& 0.18\\
EIF+\_RF             & -2.816& 4.873& -2.056& 5.642& 0.18\\
\hline
\end{tabular}
}
\caption{Quantitative evaluation of the effectiveness of 6 different interpretation algorithms on {\ttfamily Wine} through the $AUC_{FS}$ metric, introduced in \ref{sec:interpr_evaluat}. In the last column the average time taken by the different models to produce the importance scores is reported. The highest $AUC_{FS}$ and lowest Importance time values are highlighted in bold.}\label{tab:fs-tab-Wine}
\end{minipage}
\end{table}

\subsubsection{Importance Plots}

\ale{Figure \ref{fig:interpretation-Wine} provides a qualitative and quantitative evaluation of the proposed interpretation algorithm on the {\ttfamily Wine} dataset. In Scenario I \approach+ is not able to identify, as shown in \ref{fig:GFI-Wine}, an attribute dominating the others in terms of relevance for pursuing the Anomaly Detection task. On the other hand, exploiting the characteristics of \EIFplus when the training set is composed of solely inliers, feature Proline is indicated as the most relevant one in Scenario II as depicted in \ref{fig:Feat-imp-Wine-split}. The relevance of the Proline variable can be assesed observing the Local Scoremap reported in Figure \ref{fig:Local-Wine-split}.}

\begin{figure}[!ht] 
    \centering % <-- added
    \begin{subfigure}[t]{0.36\textwidth}
    \centering
      \includegraphics[width=\linewidth]{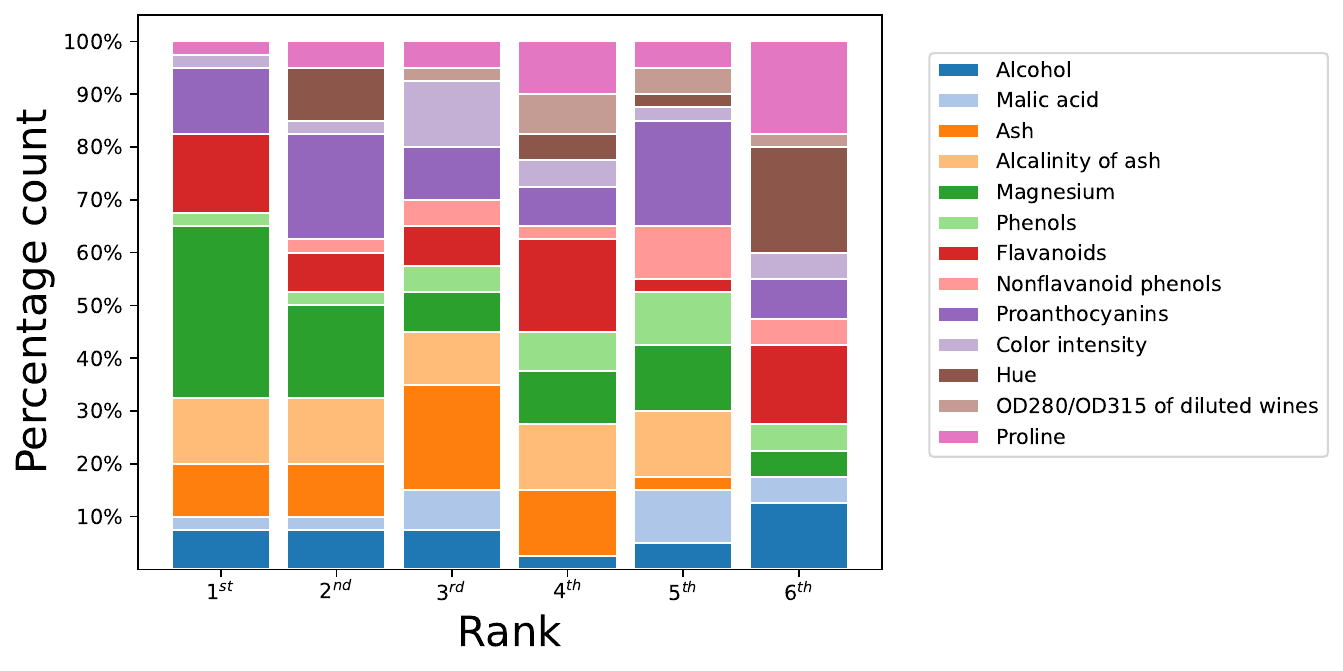}
      \caption{Bar Plot {\ttfamily Wine} Scenario I}
      \label{fig:GFI-Wine}
    \end{subfigure}\hfil % <-- added
    \begin{subfigure}[t]{0.31\textwidth}
    \centering
      \includegraphics[width=\linewidth]{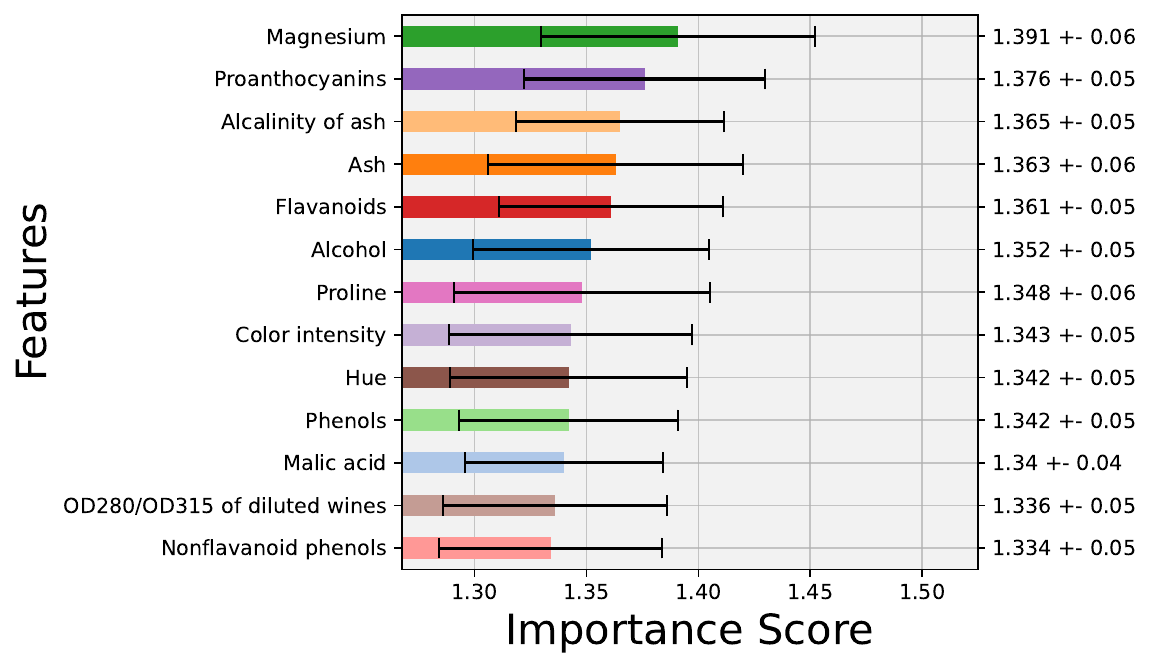}
      \caption{Score Plot {\ttfamily Wine} Scenario I}
      \label{fig:Feat-imp-Wine}
    \end{subfigure}\hfil % <-- added
    \begin{subfigure}[t]{0.23\textwidth}
    \centering
      \includegraphics[width=\linewidth]{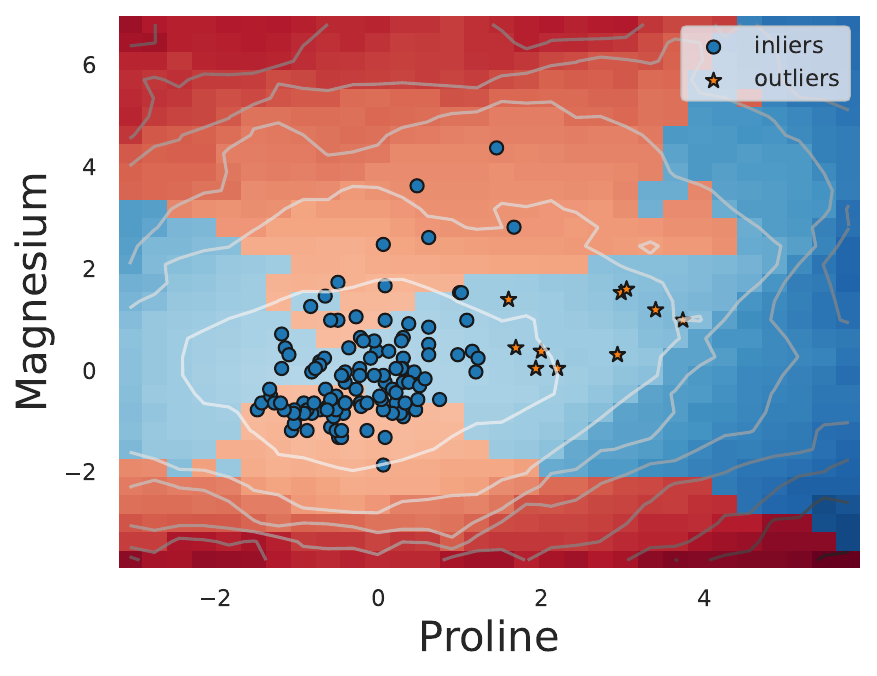}
      \caption{Scoremap {\ttfamily Wine} Scenario I}
      \label{fig:Local-Wine}
    \end{subfigure}\hfil % <-- added
    \begin{subfigure}[t]{0.36\textwidth}
    \centering
      \includegraphics[width=\linewidth]{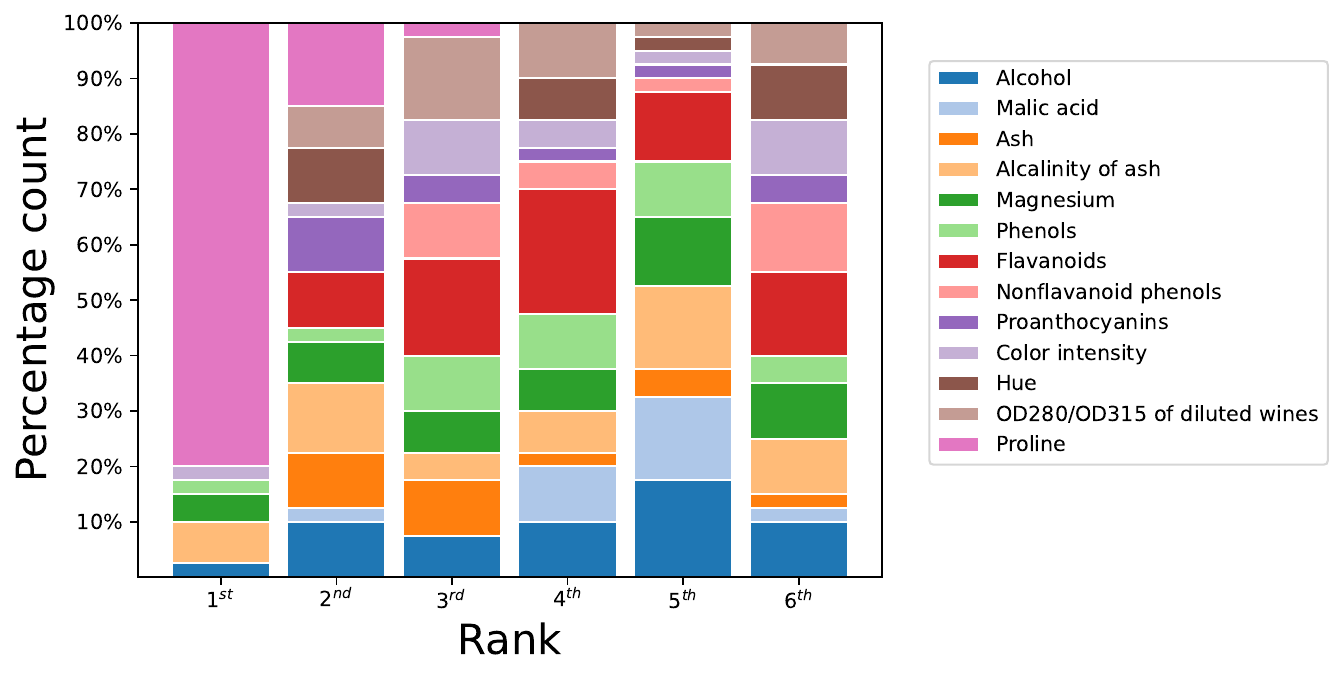}
      \caption{Bar Plot {\ttfamily Wine} Scenario II}
      \label{fig:GFI-Wine-split}
    \end{subfigure}\hfil % <-- added
    \begin{subfigure}[t]{0.31\textwidth}
    \centering
      \includegraphics[width=\linewidth]{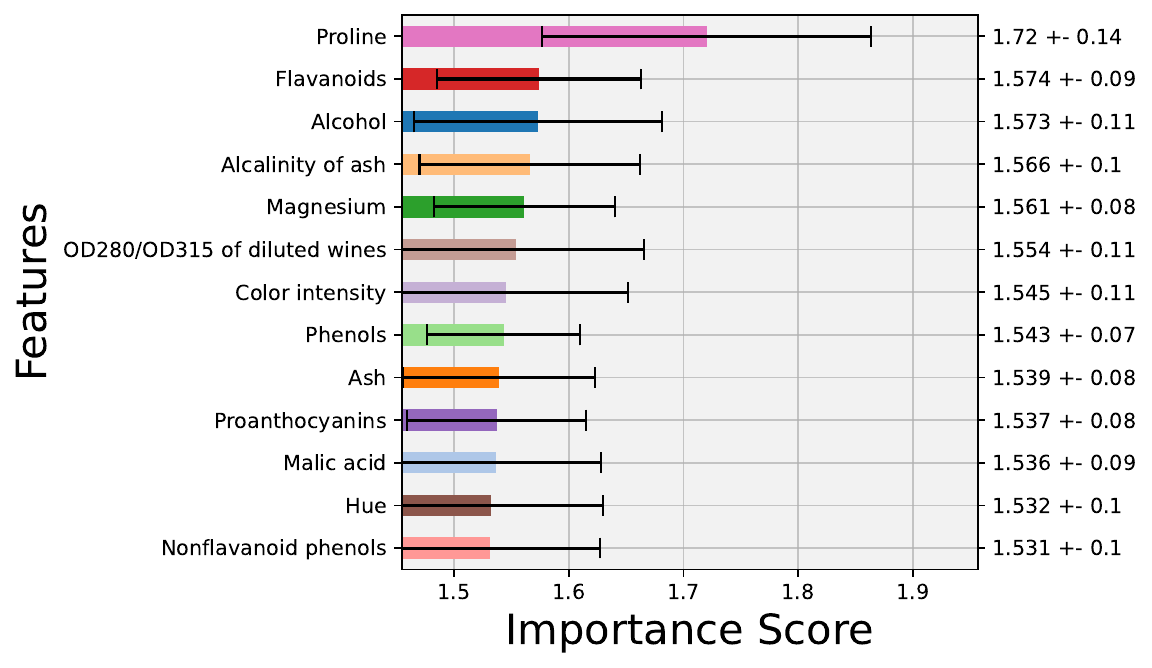}
      \caption{Score Plot {\ttfamily Wine} Scenario II}
      \label{fig:Feat-imp-Wine-split}
    \end{subfigure}\hfil % <-- added
    \begin{subfigure}[t]{0.23\textwidth}
    \centering
      \includegraphics[width=\linewidth]{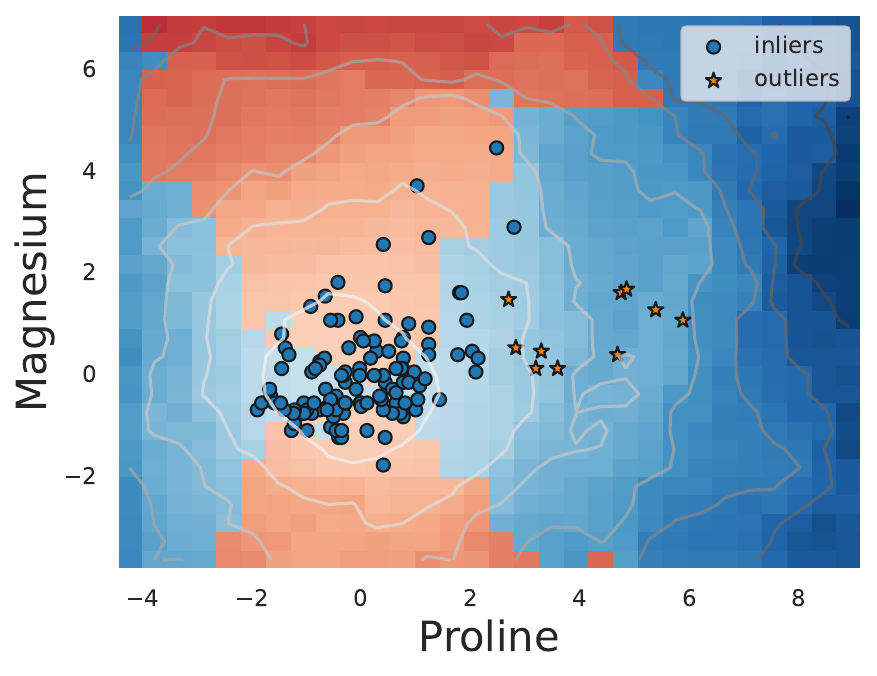}
      \caption{Scoremap {\ttfamily Wine} Scenario II}
      \label{fig:Local-Wine-split}
    \end{subfigure}\hfil % <-- added
\caption{Bar Plot, Score Plot and Scoremap for {\ttfamily Wine} in the two different Scenarios, using the \approach algorithm applied to the \EIFplus model.}\label{fig:interpretation-Wine}
\end{figure}

\subsubsection{Feature Selection}

\ale{Figure \ref{fig:fs-interpretation-Wine} shows the superiority of the \approach interpretation algorithm when applied to IF, EIF and the proposed \EIFplus as illustrated in Figures \ref{fig:Feat-Sel_Wine_valEIF+_DIFFI_2}, \ref{fig:Feat-Sel_Wine_valEIF+_EXIFFI_2} and \ref{fig:Feat-Sel_Wine_valEIF+_EXIFFI+_2}. Using the feature ranking derived from the importance scores generated by \approach, in fact, guarantees an increasing Average Precision as non relevant attributes are progressively removed from the feature space (red line) reaching almost perfect scores of 1. On the other hand following the blue line it is possible to notice an instantaneous drop in performance as the most important features are removed from the training set. Conversely the application of the RandomForest based post-hoc method produces sligthly inferior results mainly bacause of the oscillating trend observable in the blue line which demonstrates a non perfect alignment of the feature ranking with the ground truth.}

\begin{figure}[!ht] 
\centering
\hspace{0.05\textwidth}\textbf{IF} \hspace{0.29\textwidth} \textbf{EIF} \hspace{0.29\textwidth} \textbf{EIF+}
% First row with vertical caption on the left
\begin{minipage}{\textwidth}
    \rotatebox{90}{\parbox{15mm}{\centering \textbf{Ad-Hoc}}} % Adjust the parbox width as necessary for your caption text
    \begin{minipage}{0.95\textwidth}
        \begin{subfigure}[t]{0.30\textwidth}
            \centering
            \includegraphics[trim={0 0 3.5cm 0}, clip, width=\linewidth]{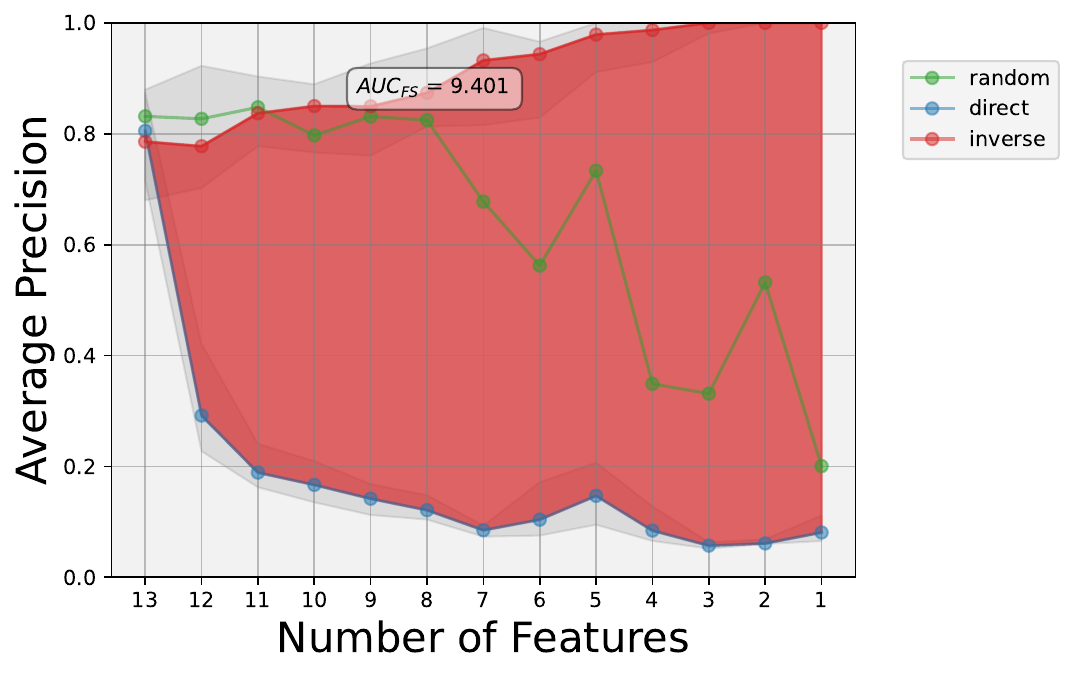}
            \caption{\approach applied to IF}
            \label{fig:Feat-Sel_Wine_valEIF+_DIFFI_2}
        \end{subfigure}\hfill
        \begin{subfigure}[t]{0.30\textwidth}
            \centering
            \includegraphics[trim={0 0 3.5cm 0}, clip, width=\linewidth]{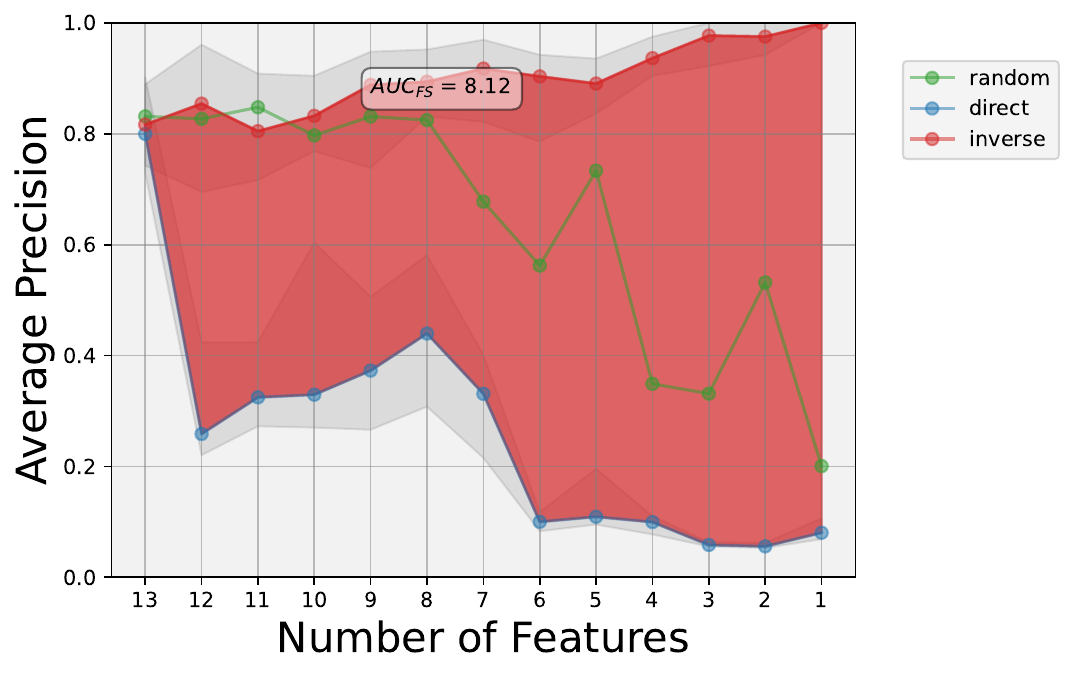}
            \caption{\approach applied to EIF}
            \label{fig:Feat-Sel_Wine_valEIF+_EXIFFI_2}
        \end{subfigure}\hfill
        \begin{subfigure}[t]{0.30\textwidth}
            \centering
            \includegraphics[trim={0 0 3.5cm 0}, clip, width=\linewidth]{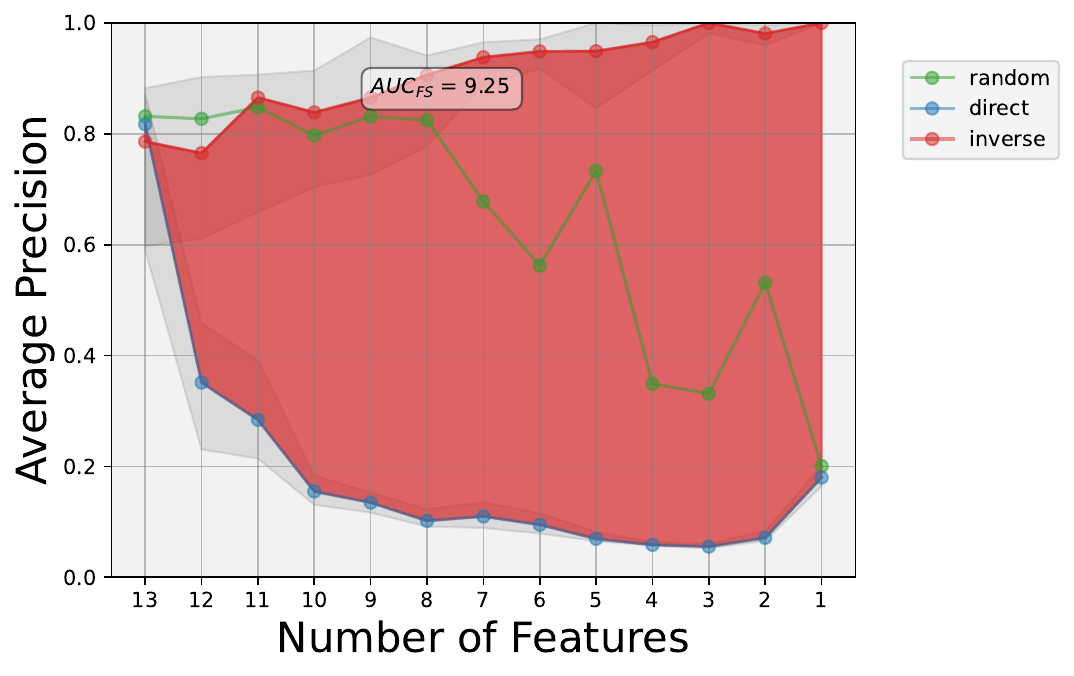}
            \caption{\approach applied to \EIFplus}
            \label{fig:Feat-Sel_Wine_valEIF+_EXIFFI+_2}
        \end{subfigure}
    \end{minipage}
\end{minipage}

\vspace{5mm} % Space between rows

% Second row with vertical caption on the left
\begin{minipage}{\textwidth}
    \rotatebox{90}{\parbox{15mm}{\centering \textbf{Post-Hoc}}} % Adjust as necessary
    \begin{minipage}{0.95\textwidth}
        \begin{subfigure}[t]{0.30\textwidth}
            \centering
            \includegraphics[trim={0 0 3.5cm 0}, clip, width=\linewidth]{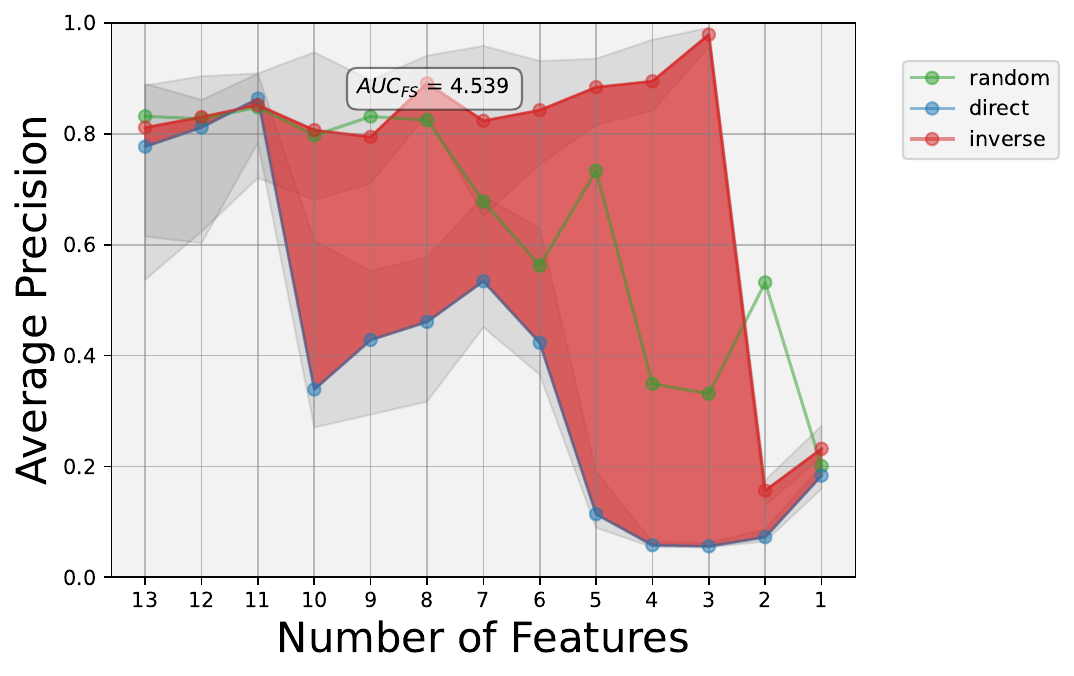}
            \caption{RandomForest fitted to IF}
            \label{fig:Feat-Sel_Wine_valEIF+_IF_RandomForest_2}
        \end{subfigure}\hfill
        \begin{subfigure}[t]{0.30\textwidth}
            \centering
            \includegraphics[trim={0 0 3.5cm 0}, clip, width=\linewidth]{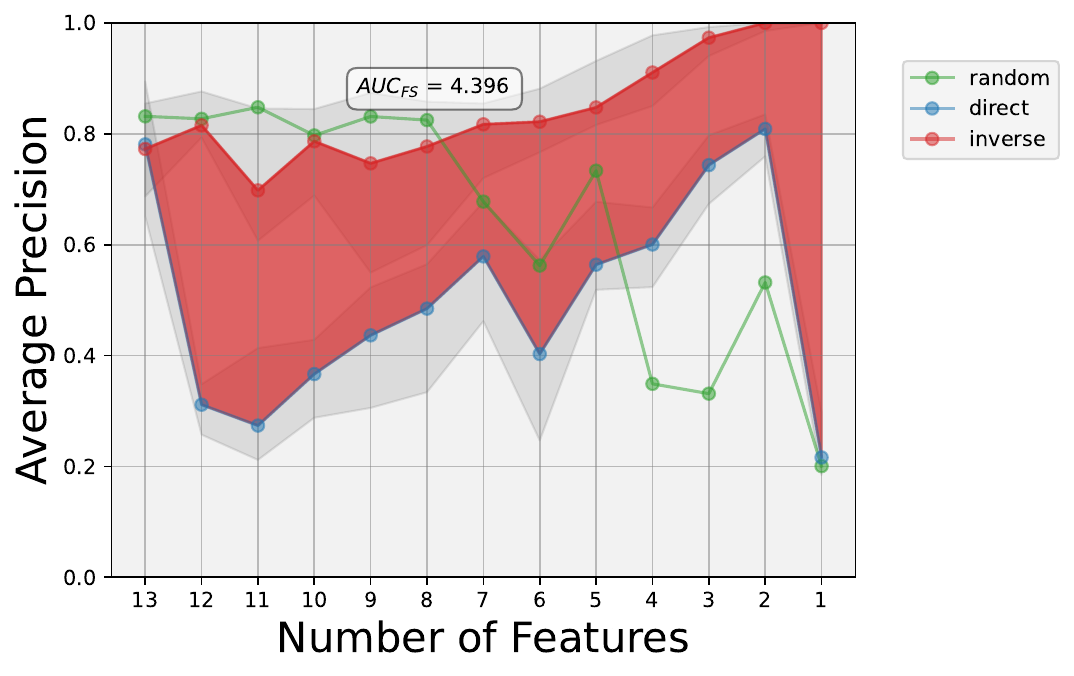}
            \caption{RandomForest fitted to EIF}
            \label{fig:Feat-Sel_Wine_valEIF+_EIF_RandomForest_2}
        \end{subfigure}\hfill
        \begin{subfigure}[t]{0.30\textwidth}
            \centering
            \includegraphics[trim={0 0 3.5cm 0}, clip, width=\linewidth]{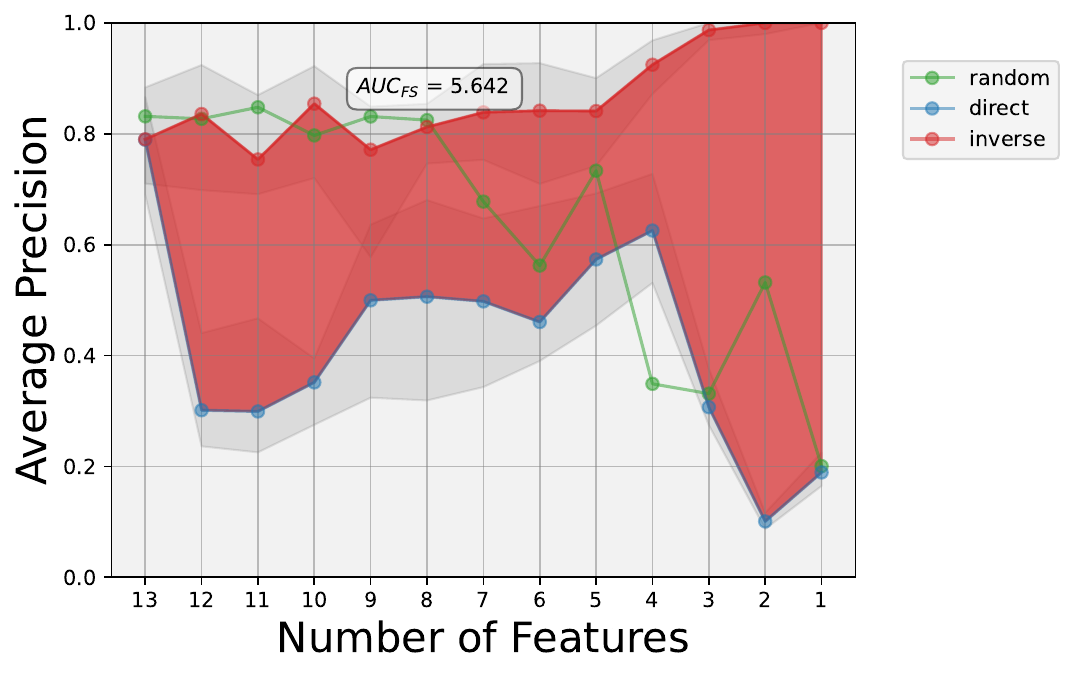}
            \caption{RandomForest fitted to \EIFplus}
            \label{fig:Feat-Sel_Wine_valEIF+_EIF+_RandomForest_2}
        \end{subfigure}
    \end{minipage}
\end{minipage}

\caption{Feature Selection of the different Ad-Hoc and Post-Hoc methods applied to the 3 Isolation Forest models: IF, EIF and \EIFplus. The blue line is the values of average precision, calculated with the \EIFplus model in the Scenario II, dropping the most important feature at each step, the red line is the values of average precision dropping the least important feature at each step and the green line is the value of the feature selection dropping a random feature at each step.}\label{fig:fs-interpretation-Wine}
\end{figure}

\ale{The summary reported in \ref{tab:fs-tab-Wine} confirm the effectiveness of the proposed approach in providing explainability to the EIF and \EIFplus AD methods surpassing DIFFI and post-hoc interpretability approaches such as Random Forest. In particular, the DIFFI interpretation algorithm is the only one producing negative $AUC_{FS}$ values in Scenario II proving its inability in producing correct feature rankings in presence of solely inliers in the training set. Moreover the ineffectiveness of this method is additionally demonstrated by the metric values associated to Scenario I (i.e. 0.176 and 0.437) that, being close to 0, represent a situation is which there is not a significant advantage in removing features in increasing or decreasing order.}

\subsection{\EIFplus: the effects of $\eta$}\label{app:eta}

\ale{In this section the results of the ablation study on the $\eta$ hyperparameter of the \EIFplus model for the datasets covered in this Appendix are reported. The {\ttfamily Yaxis} dataset, presented in \ref{sec:Yaxis}, is excluded from this analysis because of its high similarity to the {\ttfamily Xaxis} dataset that lead to essentially identical outcomes. }

\ale{The ablation study consists in evaluating the performance of the \EIFplus model, through the Average Precision metric, for 25 linearly spaced values between 0.5 and 5 of the parameter $\eta$, whose interpretation is given in \ref{sec:EIFplus}. }
\begin{figure}[!ht] 
    \centering % <-- added
    \begin{subfigure}{0.33\textwidth}
    \centering
      \includegraphics[width=\linewidth]{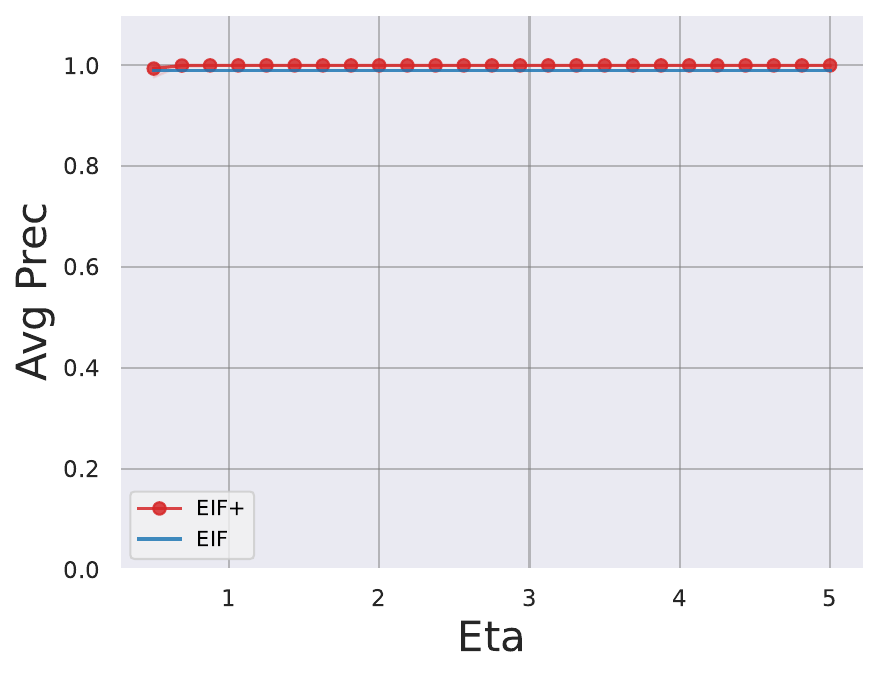}
      \caption{{\ttfamily Bisect}}
      \label{fig:ablation-Bisect}
    \end{subfigure}\hfil % <-- added
    \begin{subfigure}{0.33\textwidth}
    \centering
      \includegraphics[width=\linewidth]{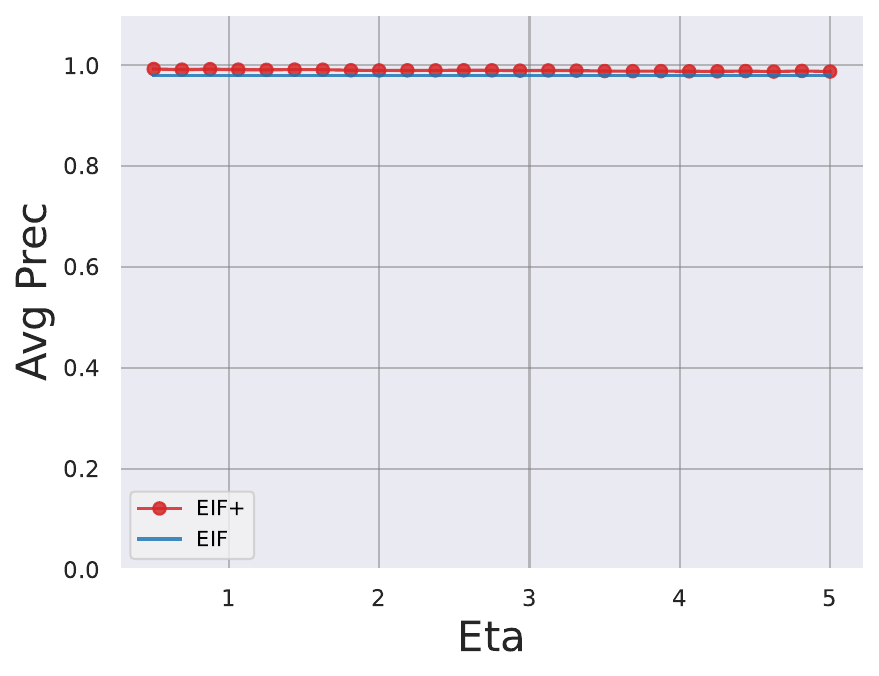}
      \caption{{\ttfamily Breastw}}
      \label{fig:ablation-Breastw}
    \end{subfigure}\hfil % <-- added
    \begin{subfigure}{0.33\textwidth}
    \centering
      \includegraphics[width=\linewidth]{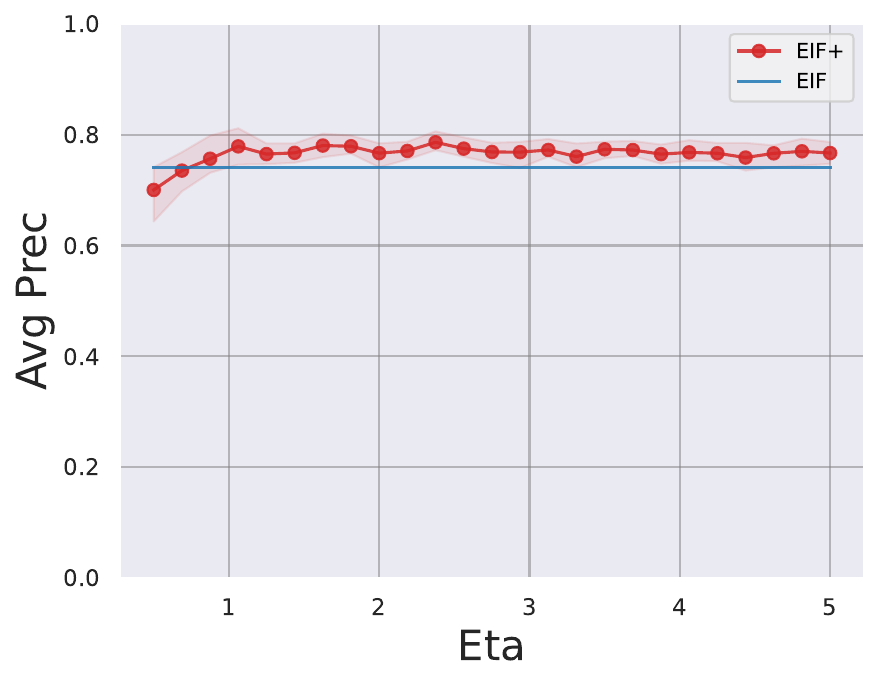}
      \caption{{\ttfamily Cardio}}
      \label{fig:ablation-Cardio}
    \end{subfigure}\hfil % <-- added
    \begin{subfigure}{0.33\textwidth}
    \centering
      \includegraphics[width=\linewidth]{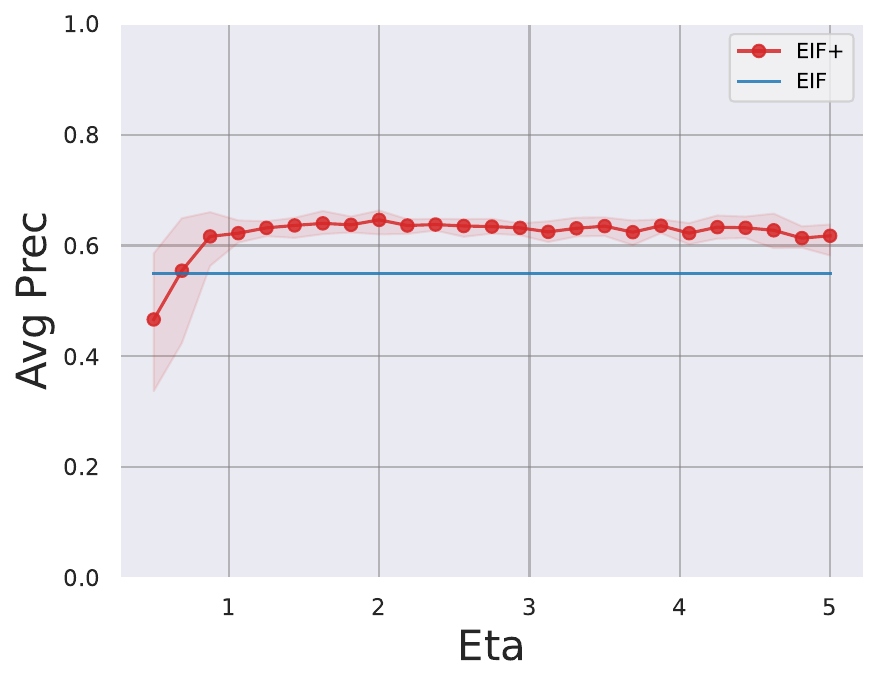}
      \caption{{\ttfamily Diabetes}}
      \label{fig:ablation-Diabetes}
    \end{subfigure}\hfil % <-- added
    \begin{subfigure}{0.33\textwidth}
    \centering
      \includegraphics[width=\linewidth]{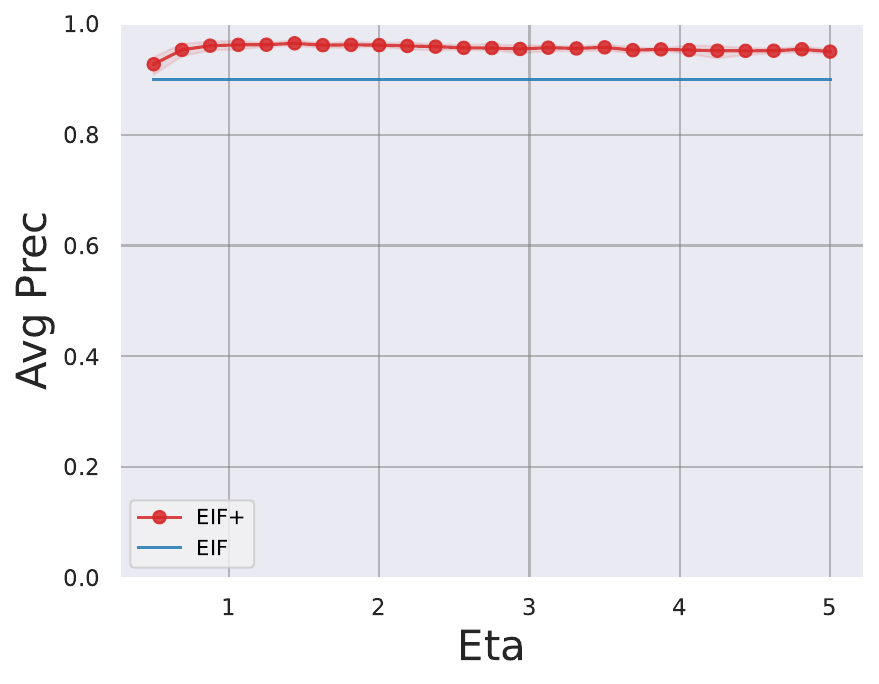}
      \caption{{\ttfamily Ionosphere}}
      \label{fig:ablation-Ionosphere}
    \end{subfigure}\hfil % <-- added
    \begin{subfigure}{0.33\textwidth}
    \centering
      \includegraphics[width=\linewidth]{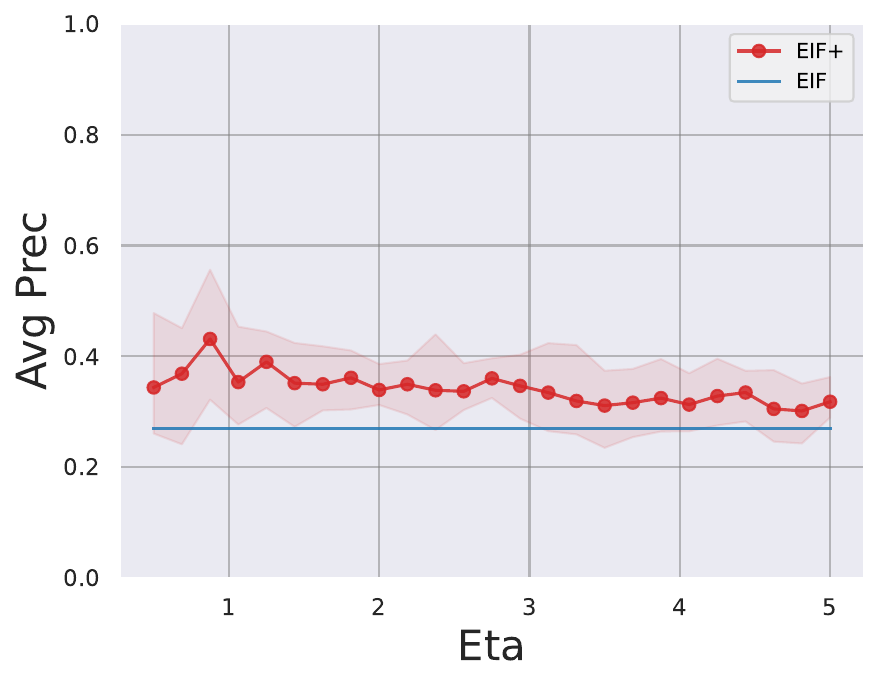}
      \caption{{\ttfamily Pendigits}}
      \label{fig:ablation-Pendigits}
    \end{subfigure}\hfil % <-- added
    \begin{subfigure}{0.33\textwidth}
    \centering
      \includegraphics[width=\linewidth]{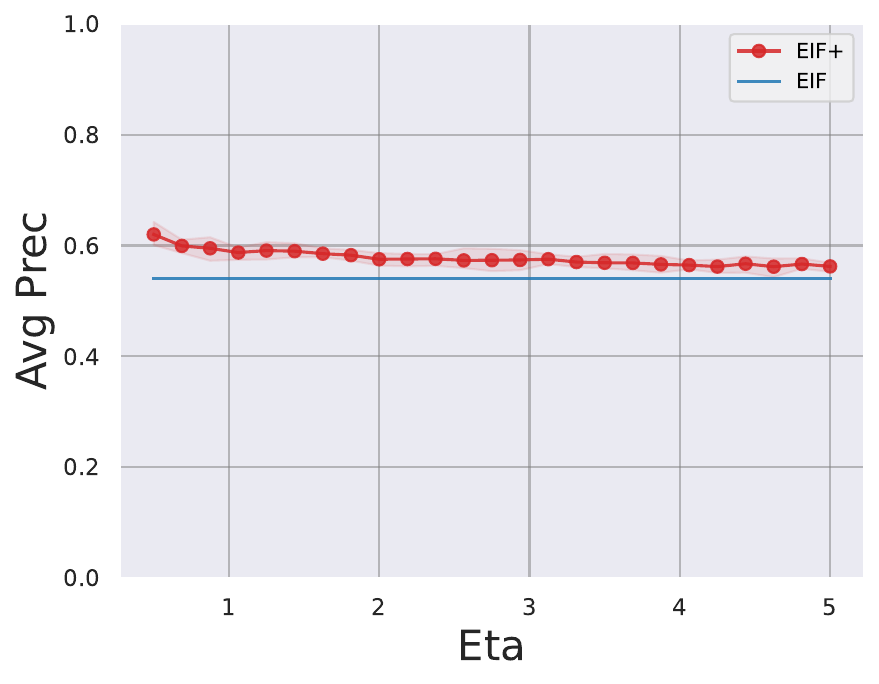}
      \caption{{\ttfamily Pima}}
      \label{fig:ablation-Pima}
    \end{subfigure}\hfil % <-- added
    \begin{subfigure}{0.33\textwidth}
    \centering
      \includegraphics[width=\linewidth]{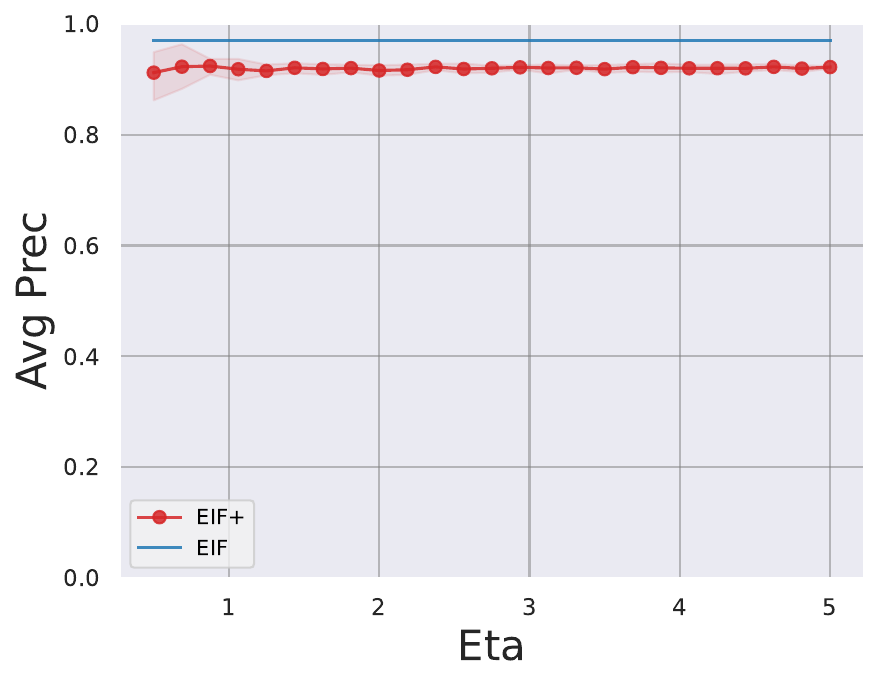}
      \caption{{\ttfamily Shuttle}}
      \label{fig:ablation-Shuttle}
    \end{subfigure}\hfil % <-- added
    \begin{subfigure}{0.33\textwidth}
    \centering
      \includegraphics[width=\linewidth]{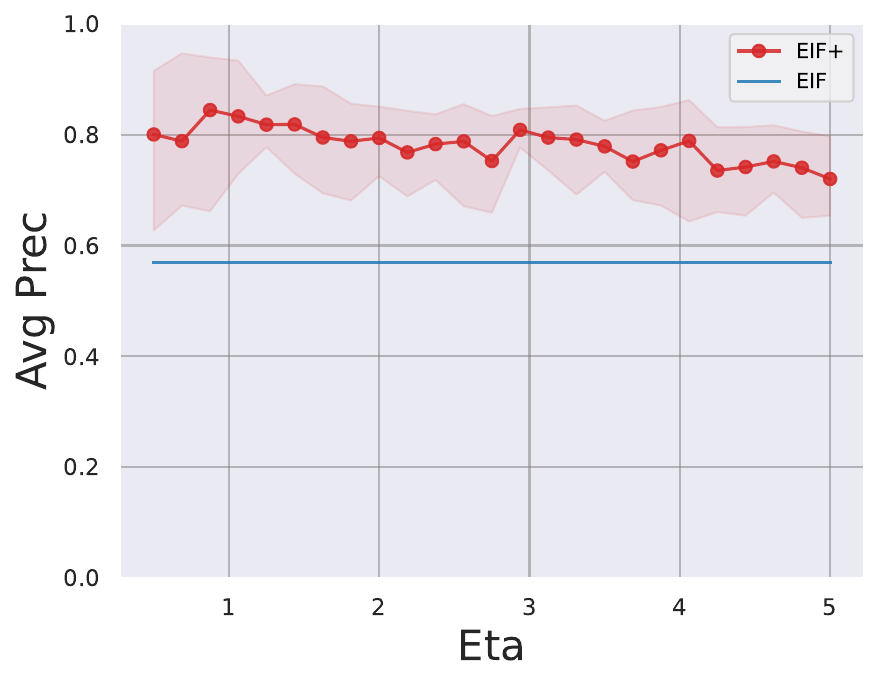}
      \caption{{\ttfamily Wine}}
      \label{fig:ablation-Wine}
    \end{subfigure}\hfil % <-- added
\caption{Exploration of how average precision changes with variations in the $\eta$ parameter.}\label{fig:ablation_appendix}
\end{figure}

\ale{After a careful observation of the plots collected in Figure \ref{fig:ablation_appendix} it is possible to conclude that for the {\ttfamily Bisect}, {\ttfamily Breastw}, {\ttfamily Ionosphere} and {\ttfamily Shuttle} the Average Precision of \EIFplus is not affected by the value of the parameter $\eta$. In fact, as it can be noticed comparing to the blue line inserted in the plot to represent the Average Precision value achieved by the EIF model, in these sets of data the improvement achieved by \EIFplus on its counterpart EIF is minimal since both models already achieve almost perfect precision scores. As a consequence the model remain unchanges independelty on the $\eta$ value since anomalies are detectable utilizing the traditional oblique cuts employed by EIF. }

\ale{For other datasets, where the data distribution is intricated and EIF-like partitions are not as effective as the novel partition approach introduced with \EIFplus, the effect of $\eta$ is more visible in the sense that there are some contained oscillations on the Average Precision values as the hyperparameter is varied. }

\ale{Concluding, comparing the diverse plots produced it is possible to infer that the optimal value for the parameter analysed in this section is highly dependent on the specific dataset structure and thus the suggested approach is to perform an hyperparameter optimization through a validation set in order to optimal value of $\eta$. }
